# Supplementary material for: Characterization of quasirandom permutations by a pattern sum
Source: arXiv:1909.11027 ancillary file (2022-07-15)
Supplement: Supplementary file 1 [file Appendices.pdf]

# Appendix 1

$$H_{1234} = \frac{1}{6 \cdot 5^6} \times \left(\begin{array}{cccccccccccccccc}
2368 & 208 & -432 & -432 & 208 & 4441 & 0 & 0 & -432 & 0 & 576 & 576 & -432 & 0 & 576 & 576 \\
208 & 1888 & 88 & -432 & -4195 & 128 & 3563 & 0 & 216 & -432 & -72 & 576 & 216 & -432 & -72 & 576 \\
-432 & 88 & 1408 & -32 & 216 & -3357 & 48 & 2601 & 0 & 288 & -432 & 0 & 0 & 288 & -432 & 0 \\
-432 & -432 & -32 & 928 & 216 & 216 & -2435 & -32 & 0 & 0 & 216 & -432 & 0 & 0 & 216 & -432 \\
208 & -4195 & 216 & 216 & 1888 & 128 & -432 & -432 & 88 & 3563 & -72 & -72 & -432 & 0 & 576 & 576 \\
4441 & 128 & -3357 & 216 & 128 & 1728 & 88 & -432 & -3357 & 88 & 3713 & -72 & 216 & -432 & -72 & 576 \\
0 & 3563 & 48 & -2435 & -432 & 88 & 1568 & 48 & 288 & -3507 & 88 & 3563 & 0 & 288 & -432 & 0 \\
0 & 0 & 2601 & -32 & -432 & -432 & 48 & 1408 & 288 & 288 & -3357 & 88 & 0 & 0 & 216 & -432 \\
-432 & 216 & 0 & 0 & 88 & -3357 & 288 & 288 & 1408 & 48 & -432 & -432 & -32 & 2601 & 0 & 0 \\
0 & -432 & 288 & 0 & 3563 & 88 & -3507 & 288 & 48 & 1568 & 88 & -432 & -2435 & 48 & 3563 & 0 \\
576 & -72 & -432 & 216 & -72 & 3713 & 88 & -3357 & -432 & 88 & 1728 & 128 & 216 & -3357 & 128 & 4441 \\
576 & 576 & 0 & -432 & -72 & -72 & 3563 & 88 & -432 & -432 & 128 & 1888 & 216 & 216 & -4195 & 208 \\
-432 & 216 & 0 & 0 & -432 & 216 & 0 & 0 & -32 & -2435 & 216 & 216 & 928 & -32 & -432 & -432 \\
0 & -432 & 288 & 0 & 0 & -432 & 288 & 0 & 2601 & 48 & -3357 & 216 & -32 & 1408 & 88 & -432 \\
576 & -72 & -432 & 216 & 576 & -72 & -432 & 216 & 0 & 3563 & 128 & -4195 & -432 & 88 & 1888 & 208 \\
576 & 576 & 0 & -432 & 576 & 576 & 0 & -432 & 0 & 0 & 4441 & 208 & -432 & -432 & 208 & 2368
\end{array}\right)$$

$$H_{1243} = \frac{1}{6 \cdot 5^6} \times \left(\begin{array}{cccccccccccccccc}
1056 & 536 & 432 & 432 & 536 & 3121 & 0 & 0 & 432 & 0 & -576 & -576 & 432 & 0 & -576 & -576 \\
536 & 640 & 432 & 432 & -3039 & 440 & 1663 & 0 & -216 & 432 & 72 & -576 & -216 & 432 & 72 & -576 \\
432 & 432 & 224 & 328 & -216 & -1629 & 344 & 433 & 0 & -288 & 432 & 0 & 0 & -288 & 432 & 0 \\
432 & 432 & 328 & -192 & -216 & -216 & -447 & 248 & 0 & 0 & -216 & 432 & 0 & 0 & -216 & 432 \\
536 & -3039 & -216 & -216 & 640 & 440 & 432 & 432 & 432 & 1663 & 72 & 72 & 432 & 0 & -576 & -576 \\
3121 & 440 & -1629 & -216 & 440 & 288 & 352 & 432 & -1629 & 352 & 569 & 72 & -216 & 432 & 72 & -576 \\
0 & 1663 & 344 & -447 & 432 & 352 & -64 & 264 & -288 & -575 & 272 & -657 & 0 & -288 & 432 & 0 \\
0 & 0 & 433 & 248 & 432 & 432 & 264 & -416 & -288 & -288 & 611 & 192 & 0 & 0 & -216 & 432 \\
432 & -216 & 0 & 0 & 432 & -1629 & -288 & -288 & 224 & 344 & 432 & 432 & 328 & 433 & 0 & 0 \\
0 & 432 & -288 & 0 & 1663 & 352 & -575 & -288 & 344 & -64 & 272 & 432 & -447 & 264 & -657 & 0 \\
-576 & 72 & 432 & -216 & 72 & 569 & 272 & 611 & 432 & 272 & -352 & 200 & -216 & 611 & 200 & -2239 \\
-576 & -576 & 0 & 432 & 72 & 72 & -657 & 192 & 432 & 432 & 200 & -640 & -216 & -216 & 2161 & 136 \\
432 & -216 & 0 & 0 & 432 & -216 & 0 & 0 & 328 & -447 & -216 & -216 & -192 & 248 & 432 & 432 \\
0 & 432 & -288 & 0 & 0 & 432 & -288 & 0 & 433 & 264 & 611 & -216 & 248 & -416 & 192 & 432 \\
-576 & 72 & 432 & -216 & -576 & 72 & 432 & -216 & 0 & -657 & 200 & 2161 & 432 & 192 & -640 & 136 \\
-576 & -576 & 0 & 432 & -576 & -576 & 0 & 432 & 0 & 0 & -2239 & 136 & 432 & 432 & 136 & -864
\end{array}\right)$$

$$H_{1324} = \frac{1}{6 \cdot 5^6} \times \left(\begin{array}{cccccccccccccccc}
-1232 & -152 & 144 & 144 & -152 & -194 & 1044 & 1044 & 144 & 1044 & 144 & 144 & 144 & 1044 & 144 & 144 \\
-152 & -848 & -56 & 144 & 350 & -88 & -550 & 1044 & -756 & 144 & 1044 & 144 & -756 & 144 & 1044 & 144 \\
144 & -56 & -464 & 40 & -756 & 738 & -24 & -162 & 144 & -756 & 144 & 1044 & 144 & -756 & 144 & 1044 \\
144 & 144 & 40 & -80 & -756 & -756 & 382 & 40 & 144 & 144 & -756 & 144 & 144 & 144 & -756 & 144 \\
-152 & 350 & -756 & -756 & -848 & -88 & 144 & 144 & -56 & -550 & 1044 & 1044 & 144 & 1044 & 144 & 144 \\
-194 & -88 & 738 & -756 & -88 & -720 & -56 & 144 & 738 & -56 & -994 & 1044 & -756 & 144 & 1044 & 144 \\
1044 & -550 & -24 & 382 & 144 & -56 & -592 & -24 & -756 & 1182 & -56 & -550 & 144 & -756 & 144 & 1044 \\
1044 & 1044 & -162 & 40 & 144 & 144 & -24 & -464 & -756 & -756 & 738 & -56 & 144 & 144 & -756 & 144 \\
144 & -756 & 144 & 144 & -56 & 738 & -756 & -756 & -464 & -24 & 144 & 144 & 40 & -162 & 1044 & 1044 \\
1044 & 144 & -756 & 144 & -550 & -56 & 1182 & -756 & -24 & -592 & -56 & 144 & 382 & -24 & -550 & 1044 \\
144 & 1044 & 144 & -756 & 1044 & -994 & -56 & 738 & 144 & -56 & -720 & -88 & -756 & 738 & -88 & -194 \\
144 & 144 & 1044 & 144 & 1044 & 1044 & -550 & -56 & 144 & 144 & -88 & -848 & -756 & -756 & 350 & -152 \\
144 & -756 & 144 & 144 & 144 & -756 & 144 & 144 & 40 & 382 & -756 & -756 & -80 & 40 & 144 & 144 \\
1044 & 144 & -756 & 144 & 1044 & 144 & -756 & 144 & -162 & -24 & 738 & -756 & 40 & -464 & -56 & 144 \\
144 & 1044 & 144 & -756 & 144 & 1044 & 144 & -756 & 1044 & -550 & -88 & 350 & 144 & -56 & -848 & -152 \\
144 & 144 & 1044 & 144 & 144 & 144 & 1044 & 144 & 1044 & 1044 & -194 & -152 & 144 & 144 & -152 & -1232
\end{array}\right)$$

$$H_{1342} = \frac{1}{6 \cdot 5^6} \times \left(\begin{array}{cccccccccccccccc}
-672 & 308 & 576 & 576 & -292 & -98 & 396 & 396 & -144 & -1044 & -144 & -144 & -144 & -1044 & -144 & -144 \\
308 & -320 & 396 & 576 & 24 & -220 & 664 & 396 & 756 & -144 & -1044 & -144 & 756 & -144 & -1044 & -144 \\
576 & 396 & 32 & 484 & -324 & -702 & -148 & 1798 & -144 & 756 & -144 & -1044 & -144 & 756 & -144 & -1044 \\
576 & 576 & 484 & 384 & -324 & -324 & -1800 & -76 & -144 & -144 & 756 & -144 & -144 & -144 & 756 & -144 \\
-292 & 24 & -324 & -324 & -800 & 260 & 576 & 576 & -324 & -356 & 36 & 36 & -144 & -1044 & -144 & -144 \\
-98 & -220 & -702 & -324 & 260 & -576 & 316 & 576 & 258 & -284 & 542 & 36 & 756 & -144 & -1044 & -144 \\
396 & 664 & -148 & -1800 & 576 & 316 & -352 & 372 & 36 & -620 & -244 & 1884 & -144 & 756 & -144 & -1044 \\
396 & 396 & 1798 & -76 & 576 & 576 & 372 & -128 & 36 & 36 & -1942 & -204 & -144 & -144 & 756 & -144 \\
-144 & 756 & -144 & -144 & -324 & 258 & 36 & 36 & -928 & 212 & 576 & 576 & -356 & -782 & -324 & -324 \\
-1044 & -144 & 756 & -144 & -356 & -284 & -620 & 36 & 212 & -832 & 236 & 576 & 660 & -348 & -36 & -324 \\
-144 & -1044 & -144 & 756 & 36 & 542 & -244 & -1942 & 576 & 236 & -736 & 260 & 396 & -82 & -340 & 1082 \\
-144 & -144 & -1044 & -144 & 36 & 36 & 1884 & -204 & 576 & 576 & 260 & -640 & 396 & 396 & -1196 & -332 \\
-144 & 756 & -144 & -144 & -144 & 756 & -144 & -144 & -356 & 660 & 396 & 396 & -1056 & 164 & 576 & 576 \\
-1044 & -144 & 756 & -144 & -1044 & -144 & 756 & -144 & -782 & -348 & -82 & 396 & 164 & -1088 & 156 & 576 \\
-144 & -1044 & -144 & 756 & -144 & -1044 & -144 & 756 & -324 & -36 & -340 & -1196 & 576 & 156 & -1120 & 148 \\
-144 & -144 & -1044 & -144 & -144 & -144 & -1044 & -144 & -324 & -324 & 1082 & -332 & 576 & 576 & 148 & -1152
\end{array}\right)$$

$$H_{1423} = \frac{1}{6 \cdot 5^6} \times \begin{pmatrix}
-672 & -292 & -144 & -144 & 308 & -98 & -1044 & -1044 & 576 & 396 & -144 & -144 & 576 & 396 & -144 & -144 \\
-292 & -800 & -324 & -144 & 24 & 260 & -356 & -1044 & -324 & 576 & 36 & -144 & -324 & 576 & 36 & -144 \\
-144 & -324 & -928 & -356 & 756 & 258 & 212 & -782 & -144 & 36 & 576 & -324 & -144 & 36 & 576 & -324 \\
-144 & -144 & -356 & -1056 & 756 & 756 & 660 & 164 & -144 & -144 & 396 & 576 & -144 & -144 & 396 & 576 \\
308 & 24 & 756 & 756 & -320 & -220 & -144 & -144 & 396 & 664 & -1044 & -1044 & 576 & 396 & -144 & -144 \\
-98 & 260 & 258 & 756 & -220 & -576 & -284 & -144 & -702 & 316 & 542 & -1044 & -324 & 576 & 36 & -144 \\
-1044 & -356 & 212 & 660 & -144 & -284 & -832 & -348 & 756 & -620 & 236 & -36 & -144 & 36 & 576 & -324 \\
-1044 & -1044 & -782 & 164 & -144 & -144 & -348 & -1088 & 756 & 756 & -82 & 156 & -144 & -144 & 396 & 576 \\
576 & -324 & -144 & -144 & 396 & -702 & 756 & 756 & 32 & -148 & -144 & -144 & 484 & 1798 & -1044 & -1044 \\
396 & 576 & 36 & -144 & 664 & 316 & -620 & 756 & -148 & -352 & -244 & -144 & -1800 & 372 & 1884 & -1044 \\
-144 & 36 & 576 & 396 & -1044 & 542 & 236 & -82 & -144 & -244 & -736 & -340 & 756 & -1942 & 260 & 1082 \\
-144 & -144 & -324 & 576 & -1044 & -1044 & -36 & 156 & -144 & -144 & -340 & -1120 & 756 & 756 & -1196 & 148 \\
576 & -324 & -144 & -144 & 576 & -324 & -144 & -144 & 484 & -1800 & 756 & 756 & 384 & -76 & -144 & -144 \\
396 & 576 & 36 & -144 & 396 & 576 & 36 & -144 & 1798 & 372 & -1942 & 756 & -76 & -128 & -204 & -144 \\
-144 & 36 & 576 & 396 & -144 & 36 & 576 & 396 & -1044 & 1884 & 260 & -1196 & -144 & -204 & -640 & -332 \\
-144 & -144 & -324 & 576 & -144 & -144 & -324 & 576 & -1044 & -1044 & 1082 & 148 & -144 & -144 & -332 & -1152
\end{pmatrix}$$

$$H_{1432} = \frac{1}{6 \cdot 5^6} \times \begin{pmatrix}
1200 & -160 & -576 & -576 & -160 & -1598 & -396 & -396 & -576 & -396 & 144 & 144 & -576 & -396 & 144 & 144 \\
-160 & 976 & -216 & -576 & 1458 & -184 & -2102 & -396 & 324 & -576 & -36 & 144 & 324 & -576 & -36 & 144 \\
-576 & -216 & 752 & -272 & 324 & 1950 & -208 & -2810 & 144 & -36 & -576 & 324 & 144 & -36 & -576 & 324 \\
-576 & -576 & -272 & 528 & 324 & 324 & 2646 & -232 & 144 & 144 & -396 & -576 & 144 & 144 & -396 & -576 \\
-160 & 1458 & 324 & 324 & 976 & -184 & -576 & -576 & -216 & -2102 & -36 & -36 & -576 & -396 & 144 & 144 \\
-1598 & -184 & 1950 & 324 & -184 & 1008 & -176 & -576 & 1950 & -176 & -2878 & -36 & 324 & -576 & -36 & 144 \\
-396 & -2102 & -208 & 2646 & -576 & -176 & 1040 & -168 & -36 & 2746 & -136 & -3642 & 144 & -36 & -576 & 324 \\
-396 & -396 & -2810 & -232 & -576 & -576 & -168 & 1072 & -36 & -36 & 3530 & -96 & 144 & 144 & -396 & -576 \\
-576 & 324 & 144 & 144 & -216 & 1950 & -36 & -36 & 752 & -208 & -576 & -576 & -272 & -2810 & 324 & 324 \\
-396 & -576 & -36 & 144 & -2102 & -176 & 2746 & -36 & -208 & 1040 & -136 & -576 & 2646 & -168 & -3642 & 324 \\
144 & -36 & -576 & -396 & -36 & -2878 & -136 & 3530 & -576 & -136 & 1328 & -64 & -396 & 3530 & -64 & -3958 \\
144 & 144 & 324 & -576 & -36 & -36 & -3642 & -96 & -576 & -576 & -64 & 1616 & -396 & -396 & 3898 & 40 \\
-576 & 324 & 144 & 144 & -576 & 324 & 144 & 144 & -272 & 2646 & -396 & -396 & 528 & -232 & -576 & -576 \\
-396 & -576 & -36 & 144 & -396 & -576 & -36 & 144 & -2810 & -168 & 3530 & -396 & -232 & 1072 & -96 & -576 \\
144 & -36 & -576 & -396 & 144 & -36 & -576 & -396 & 324 & -3642 & -64 & 3898 & -576 & -96 & 1616 & 40 \\
144 & 144 & 324 & -576 & 144 & 144 & 324 & -576 & 324 & 324 & -3958 & 40 & -576 & -576 & 40 & 2160
\end{pmatrix}$$

$$H_{2134} = \frac{1}{6 \cdot 5^6} \times \begin{pmatrix}
-864 & 136 & 432 & 432 & 136 & -2239 & 0 & 0 & 432 & 0 & -576 & -576 & 432 & 0 & -576 & -576 \\
136 & -640 & 192 & 432 & 2161 & 200 & -657 & 0 & -216 & 432 & 72 & -576 & -216 & 432 & 72 & -576 \\
432 & 192 & -416 & 248 & -216 & 611 & 264 & 433 & 0 & -288 & 432 & 0 & 0 & -288 & 432 & 0 \\
432 & 432 & 248 & -192 & -216 & -216 & -447 & 328 & 0 & 0 & -216 & 432 & 0 & 0 & -216 & 432 \\
136 & 2161 & -216 & -216 & -640 & 200 & 432 & 432 & 192 & -657 & 72 & 72 & 432 & 0 & -576 & -576 \\
-2239 & 200 & 611 & -216 & 200 & -352 & 272 & 432 & 611 & 272 & 569 & 72 & -216 & 432 & 72 & -576 \\
0 & -657 & 264 & -447 & 432 & 272 & -64 & 344 & -288 & -575 & 352 & 1663 & 0 & -288 & 432 & 0 \\
0 & 0 & 433 & 328 & 432 & 432 & 344 & 224 & -288 & -288 & -1629 & 432 & 0 & 0 & -216 & 432 \\
432 & -216 & 0 & 0 & 192 & 611 & -288 & -288 & -416 & 264 & 432 & 432 & 248 & 433 & 0 & 0 \\
0 & 432 & -288 & 0 & -657 & 272 & -575 & -288 & 264 & -64 & 352 & 432 & -447 & 344 & 1663 & 0 \\
-576 & 72 & 432 & -216 & 72 & 569 & 352 & -1629 & 432 & 352 & 288 & 440 & -216 & -1629 & 440 & 3121 \\
-576 & -576 & 0 & 432 & 72 & 72 & 1663 & 432 & 432 & 432 & 440 & 640 & -216 & -216 & -3039 & 536 \\
432 & -216 & 0 & 0 & 432 & -216 & 0 & 0 & 248 & -447 & -216 & -216 & -192 & 328 & 432 & 432 \\
0 & 432 & -288 & 0 & 0 & 432 & -288 & 0 & 433 & 344 & -1629 & -216 & 328 & 224 & 432 & 432 \\
-576 & 72 & 432 & -216 & -576 & 72 & 432 & -216 & 0 & 1663 & 440 & -3039 & 432 & 432 & 640 & 536 \\
-576 & -576 & 0 & 432 & -576 & -576 & 0 & 432 & 0 & 0 & 3121 & 536 & 432 & 432 & 536 & 1056
\end{pmatrix}$$

$$H_{2143} = \frac{1}{6 \cdot 5^6} \times \begin{pmatrix}
416 & -184 & -432 & -432 & -184 & -3235 & 0 & 0 & -432 & 0 & 576 & 576 & -432 & 0 & 576 & 576 \\
-184 & 704 & -112 & -432 & 3317 & -136 & -2125 & 0 & 216 & -432 & -72 & 576 & 216 & -432 & -72 & 576 \\
-432 & -112 & 992 & -40 & 216 & 2231 & -88 & -1411 & 0 & 288 & -432 & 0 & 0 & 288 & -432 & 0 \\
-432 & -432 & -40 & 1280 & 216 & 216 & 1541 & -40 & 0 & 0 & 216 & -432 & 0 & 0 & 216 & -432 \\
-184 & 3317 & 216 & 216 & 704 & -136 & -432 & -432 & -112 & -2125 & -72 & -72 & -432 & 0 & 576 & 576 \\
-3235 & -136 & 2231 & 216 & -136 & 800 & -112 & -432 & 2231 & -112 & -1963 & -72 & 216 & -432 & -72 & 576 \\
0 & -2125 & -88 & 1541 & -432 & -112 & 896 & -88 & 288 & 2069 & -112 & -2125 & 0 & 288 & -432 & 0 \\
0 & 0 & -1411 & -40 & -432 & -432 & -88 & 992 & 288 & 288 & 2231 & -112 & 0 & 0 & 216 & -432 \\
-432 & 216 & 0 & 0 & -112 & 2231 & 288 & 288 & 992 & -88 & -432 & -432 & -40 & -1411 & 0 & 0 \\
0 & -432 & 288 & 0 & -2125 & -112 & 2069 & 288 & -88 & 896 & -112 & -432 & 1541 & -88 & -2125 & 0 \\
576 & -72 & -432 & 216 & -72 & -1963 & -112 & 2231 & -432 & -112 & 800 & -136 & 216 & 2231 & -136 & -3235 \\
576 & 576 & 0 & -432 & -72 & -72 & -2125 & -112 & -432 & -432 & -136 & 704 & 216 & 216 & 3317 & -184 \\
-432 & 216 & 0 & 0 & -432 & 216 & 0 & 0 & -40 & 1541 & 216 & 216 & 1280 & -40 & -432 & -432 \\
0 & -432 & 288 & 0 & 0 & -432 & 288 & 0 & -1411 & -88 & 2231 & 216 & -40 & 992 & -112 & -432 \\
576 & -72 & -432 & 216 & 576 & -72 & -432 & 216 & 0 & -2125 & -136 & 3317 & -432 & -112 & 704 & -184 \\
576 & 576 & 0 & -432 & 576 & 576 & 0 & -432 & 0 & 0 & -3235 & -184 & -432 & -432 & -184 & 416
\end{pmatrix}$$

$$H_{2314} = \frac{1}{6 \cdot 5^6} \times \begin{pmatrix}
-1152 & -332 & -144 & -144 & 148 & 1082 & -1044 & -1044 & 576 & -324 & -144 & -144 & 576 & -324 & -144 & -144 \\
-332 & -640 & -204 & -144 & -1196 & 260 & 1884 & -1044 & 396 & 576 & 36 & -144 & 396 & 576 & 36 & -144 \\
-144 & -204 & -128 & -76 & 756 & -1942 & 372 & 1798 & -144 & 36 & 576 & 396 & -144 & 36 & 576 & 396 \\
-144 & -144 & -76 & 384 & 756 & 756 & -1800 & 484 & -144 & -144 & -324 & 576 & -144 & -144 & -324 & 576 \\
148 & -1196 & 756 & 756 & -1120 & -340 & -144 & -144 & 156 & -36 & -1044 & -1044 & 576 & -324 & -144 & -144 \\
1082 & 260 & -1942 & 756 & -340 & -736 & -244 & -144 & -82 & 236 & 542 & -1044 & 396 & 576 & 36 & -144 \\
-1044 & 1884 & 372 & -1800 & -144 & -244 & -352 & -148 & 756 & -620 & 316 & 664 & -144 & 36 & 576 & 396 \\
-1044 & -1044 & 1798 & 484 & -144 & -144 & -148 & 32 & 756 & 756 & -702 & 396 & -144 & -144 & -324 & 576 \\
576 & 396 & -144 & -144 & 156 & -82 & 756 & 756 & -1088 & -348 & -144 & -144 & 164 & -782 & -1044 & -1044 \\
-324 & 576 & 36 & -144 & -36 & 236 & -620 & 756 & -348 & -832 & -284 & -144 & 660 & 212 & -356 & -1044 \\
-144 & 36 & 576 & -324 & -1044 & 542 & 316 & -702 & -144 & -284 & -576 & -220 & 756 & 258 & 260 & -98 \\
-144 & -144 & 396 & 576 & -1044 & -1044 & 664 & 396 & -144 & -144 & -220 & -320 & 756 & 756 & 24 & 308 \\
576 & 396 & -144 & -144 & 576 & 396 & -144 & -144 & 164 & 660 & 756 & 756 & -1056 & -356 & -144 & -144 \\
-324 & 576 & 36 & -144 & -324 & 576 & 36 & -144 & -782 & 212 & 258 & 756 & -356 & -928 & -324 & -144 \\
-144 & 36 & 576 & -324 & -144 & 36 & 576 & -324 & -1044 & -356 & 260 & 24 & -144 & -324 & -800 & -292 \\
-144 & -144 & 396 & 576 & -144 & -144 & 396 & 576 & -1044 & -1044 & -98 & 308 & -144 & -144 & -292 & -672
\end{pmatrix}$$

$$H_{2341} = \frac{1}{6 \cdot 5^6} \times \begin{pmatrix}
528 & -232 & -576 & -576 & -272 & 2646 & -396 & -396 & -576 & 324 & 144 & 144 & -576 & 324 & 144 & 144 \\
-232 & 1072 & -96 & -576 & -2810 & -168 & 3530 & -396 & -396 & -576 & -36 & 144 & -396 & -576 & -36 & 144 \\
-576 & -96 & 1616 & 40 & 324 & -3642 & -64 & 3898 & 144 & -36 & -576 & -396 & 144 & -36 & -576 & -396 \\
-576 & -576 & 40 & 2160 & 324 & 324 & -3958 & 40 & 144 & 144 & 324 & -576 & 144 & 144 & 324 & -576 \\
-272 & -2810 & 324 & 324 & 752 & -208 & -576 & -576 & -216 & 1950 & -36 & -36 & -576 & 324 & 144 & 144 \\
2646 & -168 & -3642 & 324 & -208 & 1040 & -136 & -576 & -2102 & -176 & 2746 & -36 & -396 & -576 & -36 & 144 \\
-396 & 3530 & -64 & -3958 & -576 & -136 & 1328 & -64 & -36 & -2878 & -136 & 3530 & 144 & -36 & -576 & -396 \\
-396 & -396 & 3898 & 40 & -576 & -576 & -64 & 1616 & -36 & -36 & -3642 & -96 & 144 & 144 & 324 & -576 \\
-576 & -396 & 144 & 144 & -216 & -2102 & -36 & -36 & 976 & -184 & -576 & -576 & -160 & 1458 & 324 & 324 \\
324 & -576 & -36 & 144 & 1950 & -176 & -2878 & -36 & -184 & 1008 & -176 & -576 & -1598 & -184 & 1950 & 324 \\
144 & -36 & -576 & 324 & -36 & 2746 & -136 & -3642 & -576 & -176 & 1040 & -168 & -396 & -2102 & -208 & 2646 \\
144 & 144 & -396 & -576 & -36 & -36 & 3530 & -96 & -576 & -576 & -168 & 1072 & -396 & -396 & -2810 & -232 \\
-576 & -396 & 144 & 144 & -576 & -396 & 144 & 144 & -160 & -1598 & -396 & -396 & 1200 & -160 & -576 & -576 \\
324 & -576 & -36 & 144 & 324 & -576 & -36 & 144 & 1458 & -184 & -2102 & -396 & -160 & 976 & -216 & -576 \\
144 & -36 & -576 & 324 & 144 & -36 & -576 & 324 & 324 & 1950 & -208 & -2810 & -576 & -216 & 752 & -272 \\
144 & 144 & -396 & -576 & 144 & 144 & -396 & -576 & 324 & 324 & 2646 & -232 & -576 & -576 & -272 & 528
\end{pmatrix}$$

$$H_{2413} = \frac{1}{6 \cdot 5^6} \times \begin{pmatrix}
-1456 & -256 & 144 & 144 & -256 & 44 & 1044 & 1044 & 144 & -756 & 144 & 144 & 144 & -756 & 144 & 144 \\
-256 & -1456 & -256 & 144 & 44 & -256 & 44 & 1044 & 1044 & 144 & -756 & 144 & 1044 & 144 & -756 & 144 \\
144 & -256 & -1456 & -256 & -756 & 44 & -256 & 44 & 144 & 1044 & 144 & -756 & 144 & 1044 & 144 & -756 \\
144 & 144 & -256 & -1456 & -756 & -756 & 44 & -256 & 144 & 144 & 1044 & 144 & 144 & 144 & 1044 & 144 \\
-256 & 44 & -756 & -756 & -1456 & -256 & 144 & 144 & -256 & 44 & 1044 & 1044 & 144 & -756 & 144 & 144 \\
44 & -256 & 44 & -756 & -256 & -1456 & -256 & 144 & 44 & -256 & 44 & 1044 & 1044 & 144 & -756 & 144 \\
1044 & 44 & -256 & 44 & 144 & -256 & -1456 & -256 & -756 & 44 & -256 & 44 & 144 & 1044 & 144 & -756 \\
1044 & 1044 & 44 & -256 & 144 & 144 & -256 & -1456 & -756 & -756 & 44 & -256 & 144 & 144 & 1044 & 144 \\
144 & 1044 & 144 & 144 & -256 & 44 & -756 & -756 & -1456 & -256 & 144 & 144 & -256 & 44 & 1044 & 1044 \\
-756 & 144 & 1044 & 144 & 44 & -256 & 44 & -756 & -256 & -1456 & -256 & 144 & 44 & -256 & 44 & 1044 \\
144 & -756 & 144 & 1044 & 1044 & 44 & -256 & 44 & 144 & -256 & -1456 & -256 & -756 & 44 & -256 & 44 \\
144 & 144 & -756 & 144 & 1044 & 1044 & 44 & -256 & 144 & 144 & -256 & -1456 & -756 & -756 & 44 & -256 \\
144 & 1044 & 144 & 144 & 144 & 1044 & 144 & 144 & -256 & 44 & -756 & -756 & -1456 & -256 & 144 & 144 \\
-756 & 144 & 1044 & 144 & -756 & 144 & 1044 & 144 & 44 & -256 & 44 & -756 & -256 & -1456 & -256 & 144 \\
144 & -756 & 144 & 1044 & 144 & -756 & 144 & 1044 & 1044 & 44 & -256 & 44 & 144 & -256 & -1456 & -256 \\
144 & 144 & -756 & 144 & 144 & 144 & -756 & 144 & 1044 & 1044 & 44 & -256 & 144 & 144 & -256 & -1456
\end{pmatrix}$$

$$H_{2431} = \frac{1}{6 \cdot 5^6} \times \begin{pmatrix}
-1056 & 164 & 576 & 576 & -356 & 660 & 396 & 396 & -144 & 756 & -144 & -144 & -144 & 756 & -144 & -144 \\
164 & -1088 & 156 & 576 & -782 & -348 & -82 & 396 & -1044 & -144 & 756 & -144 & -1044 & -144 & 756 & -144 \\
576 & 156 & -1120 & 148 & -324 & -36 & -340 & -1196 & -144 & -1044 & -144 & 756 & -144 & -1044 & -144 & 756 \\
576 & 576 & 148 & -1152 & -324 & -324 & 1082 & -332 & -144 & -144 & -1044 & -144 & -144 & -144 & -1044 & -144 \\
-356 & -782 & -324 & -324 & -928 & 212 & 576 & 576 & -324 & 258 & 36 & 36 & -144 & 756 & -144 & -144 \\
660 & -348 & -36 & -324 & 212 & -832 & 236 & 576 & -356 & -284 & -620 & 36 & -1044 & -144 & 756 & -144 \\
396 & -82 & -340 & 1082 & 576 & 236 & -736 & 260 & 36 & 542 & -244 & -1942 & -144 & -1044 & -144 & 756 \\
396 & 396 & -1196 & -332 & 576 & 576 & 260 & -640 & 36 & 36 & 1884 & -204 & -144 & -144 & -1044 & -144 \\
-144 & -1044 & -144 & -144 & -324 & -356 & 36 & 36 & -800 & 260 & 576 & 576 & -292 & 24 & -324 & -324 \\
756 & -144 & -1044 & -144 & 258 & -284 & 542 & 36 & 260 & -576 & 316 & 576 & -98 & -220 & -702 & -324 \\
-144 & 756 & -144 & -1044 & 36 & -620 & -244 & 1884 & 576 & 316 & -352 & 372 & 396 & 664 & -148 & -1800 \\
-144 & -144 & 756 & -144 & 36 & 36 & -1942 & -204 & 576 & 576 & 372 & -128 & 396 & 396 & 1798 & -76 \\
-144 & -1044 & -144 & -144 & -144 & -1044 & -144 & -144 & -292 & -98 & 396 & 396 & -672 & 308 & 576 & 576 \\
756 & -144 & -1044 & -144 & 756 & -144 & -1044 & -144 & 24 & -220 & 664 & 396 & 308 & -320 & 396 & 576 \\
-144 & 756 & -144 & -1044 & -144 & 756 & -144 & -1044 & -324 & -702 & -148 & 1798 & 576 & 396 & 32 & 484 \\
-144 & -144 & 756 & -144 & -144 & -144 & 756 & -144 & -324 & -324 & -1800 & -76 & 576 & 576 & 484 & 384
\end{pmatrix}$$

$$H_{3124} = \frac{1}{6 \cdot 5^6} \times \begin{pmatrix}
-1152 & 148 & 576 & 576 & -332 & 1082 & -324 & -324 & -144 & -1044 & -144 & -144 & -144 & -1044 & -144 & -144 \\
148 & -1120 & 156 & 576 & -1196 & -340 & -36 & -324 & 756 & -144 & -1044 & -144 & 756 & -144 & -1044 & -144 \\
576 & 156 & -1088 & 164 & 396 & -82 & -348 & -782 & -144 & 756 & -144 & -1044 & -144 & 756 & -144 & -1044 \\
576 & 576 & 164 & -1056 & 396 & 396 & 660 & -356 & -144 & -144 & 756 & -144 & -144 & -144 & 756 & -144 \\
-332 & -1196 & 396 & 396 & -640 & 260 & 576 & 576 & -204 & 1884 & 36 & 36 & -144 & -1044 & -144 & -144 \\
1082 & -340 & -82 & 396 & 260 & -736 & 236 & 576 & -1942 & -244 & 542 & 36 & 756 & -144 & -1044 & -144 \\
-324 & -36 & -348 & 660 & 576 & 236 & -832 & 212 & 36 & -620 & -284 & -356 & -144 & 756 & -144 & -1044 \\
-324 & -324 & -782 & -356 & 576 & 576 & 212 & -928 & 36 & 36 & 258 & -324 & -144 & -144 & 756 & -144 \\
-144 & 756 & -144 & -144 & -204 & -1942 & 36 & 36 & -128 & 372 & 576 & 576 & -76 & 1798 & 396 & 396 \\
-1044 & -144 & 756 & -144 & 1884 & -244 & -620 & 36 & 372 & -352 & 316 & 576 & -1800 & -148 & 664 & 396 \\
-144 & -1044 & -144 & 756 & 36 & 542 & -284 & 258 & 576 & 316 & -576 & 260 & -324 & -702 & -220 & -98 \\
-144 & -144 & -1044 & -144 & 36 & 36 & -356 & -324 & 576 & 576 & 260 & -800 & -324 & -324 & 24 & -292 \\
-144 & 756 & -144 & -144 & -144 & 756 & -144 & -144 & -76 & -1800 & -324 & -324 & 384 & 484 & 576 & 576 \\
-1044 & -144 & 756 & -144 & -1044 & -144 & 756 & -144 & 1798 & -148 & -702 & -324 & 484 & 32 & 396 & 576 \\
-144 & -1044 & -144 & 756 & -144 & -1044 & -144 & 756 & 396 & 664 & -220 & 24 & 576 & 396 & -320 & 308 \\
-144 & -144 & -1044 & -144 & -144 & -144 & -1044 & -144 & 396 & 396 & -98 & -292 & 576 & 576 & 308 & -672
\end{pmatrix}$$

$$H_{3142} = \frac{1}{6 \cdot 5^6} \times \begin{pmatrix}
-1456 & -256 & 144 & 144 & -256 & 44 & -756 & -756 & 144 & 1044 & 144 & 144 & 144 & 1044 & 144 & 144 \\
-256 & -1456 & -256 & 144 & 44 & -256 & 44 & -756 & -756 & 144 & 1044 & 144 & -756 & 144 & 1044 & 144 \\
144 & -256 & -1456 & -256 & 1044 & 44 & -256 & 44 & 144 & -756 & 144 & 1044 & 144 & -756 & 144 & 1044 \\
144 & 144 & -256 & -1456 & 1044 & 1044 & 44 & -256 & 144 & 144 & -756 & 144 & 144 & 144 & -756 & 144 \\
-256 & 44 & 1044 & 1044 & -1456 & -256 & 144 & 144 & -256 & 44 & -756 & -756 & 144 & 1044 & 144 & 144 \\
44 & -256 & 44 & 1044 & -256 & -1456 & -256 & 144 & 44 & -256 & 44 & -756 & -756 & 144 & 1044 & 144 \\
-756 & 44 & -256 & 44 & 144 & -256 & -1456 & -256 & 1044 & 44 & -256 & 44 & 144 & -756 & 144 & 1044 \\
-756 & -756 & 44 & -256 & 144 & 144 & -256 & -1456 & 1044 & 1044 & 44 & -256 & 144 & 144 & -756 & 144 \\
144 & -756 & 144 & 144 & -256 & 44 & 1044 & 1044 & -1456 & -256 & 144 & 144 & -256 & 44 & -756 & -756 \\
1044 & 144 & -756 & 144 & 44 & -256 & 44 & 1044 & -256 & -1456 & -256 & 144 & 44 & -256 & 44 & -756 \\
144 & 1044 & 144 & -756 & -756 & 44 & -256 & 44 & 144 & -256 & -1456 & -256 & 1044 & 44 & -256 & 44 \\
144 & 144 & 1044 & 144 & -756 & -756 & 44 & -256 & 144 & 144 & -256 & -1456 & 1044 & 1044 & 44 & -256 \\
144 & -756 & 144 & 144 & 144 & -756 & 144 & 144 & -256 & 44 & 1044 & 1044 & -1456 & -256 & 144 & 144 \\
1044 & 144 & -756 & 144 & 1044 & 144 & -756 & 144 & 44 & -256 & 44 & 1044 & -256 & -1456 & -256 & 144 \\
144 & 1044 & 144 & -756 & 144 & 1044 & 144 & -756 & -756 & 44 & -256 & 44 & 144 & -256 & -1456 & -256 \\
144 & 144 & 1044 & 144 & 144 & 144 & 1044 & 144 & -756 & -756 & 44 & -256 & 144 & 144 & -256 & -1456
\end{pmatrix}$$

$$H_{3214} = \frac{1}{6 \cdot 5^6} \times \begin{pmatrix}
2160 & 40 & -576 & -576 & 40 & -3958 & 324 & 324 & -576 & 324 & 144 & 144 & -576 & 324 & 144 & 144 \\
40 & 1616 & -96 & -576 & 3898 & -64 & -3642 & 324 & -396 & -576 & -36 & 144 & -396 & -576 & -36 & 144 \\
-576 & -96 & 1072 & -232 & -396 & 3530 & -168 & -2810 & 144 & -36 & -576 & -396 & 144 & -36 & -576 & -396 \\
-576 & -576 & -232 & 528 & -396 & -396 & 2646 & -272 & 144 & 144 & 324 & -576 & 144 & 144 & 324 & -576 \\
40 & 3898 & -396 & -396 & 1616 & -64 & -576 & -576 & -96 & -3642 & -36 & -36 & -576 & 324 & 144 & 144 \\
-3958 & -64 & 3530 & -396 & -64 & 1328 & -136 & -576 & 3530 & -136 & -2878 & -36 & -396 & -576 & -36 & 144 \\
324 & -3642 & -168 & 2646 & -576 & -136 & 1040 & -208 & -36 & 2746 & -176 & -2102 & 144 & -36 & -576 & -396 \\
324 & 324 & -2810 & -272 & -576 & -576 & -208 & 752 & -36 & -36 & 1950 & -216 & 144 & 144 & 324 & -576 \\
-576 & -396 & 144 & 144 & -96 & 3530 & -36 & -36 & 1072 & -168 & -576 & -576 & -232 & -2810 & -396 & -396 \\
324 & -576 & -36 & 144 & -3642 & -136 & 2746 & -36 & -168 & 1040 & -176 & -576 & 2646 & -208 & -2102 & -396 \\
144 & -36 & -576 & 324 & -36 & -2878 & -176 & 1950 & -576 & -176 & 1008 & -184 & 324 & 1950 & -184 & -1598 \\
144 & 144 & -396 & -576 & -36 & -36 & -2102 & -216 & -576 & -576 & -184 & 976 & 324 & 324 & 1458 & -160 \\
-576 & -396 & 144 & 144 & -576 & -396 & 144 & 144 & -232 & 2646 & 324 & 324 & 528 & -272 & -576 & -576 \\
324 & -576 & -36 & 144 & 324 & -576 & -36 & 144 & -2810 & -208 & 1950 & 324 & -272 & 752 & -216 & -576 \\
144 & -36 & -576 & 324 & 144 & -36 & -576 & 324 & -396 & -2102 & -184 & 1458 & -576 & -216 & 976 & -160 \\
144 & 144 & -396 & -576 & 144 & 144 & -396 & -576 & -396 & -396 & -1598 & -160 & -576 & -576 & -160 & 1200
\end{pmatrix}$$

$$H_{3241} = \frac{1}{6 \cdot 5^6} \times \begin{pmatrix}
384 & -76 & -144 & -144 & 484 & -1800 & 756 & 756 & 576 & -324 & -144 & -144 & 576 & -324 & -144 & -144 \\
-76 & -128 & -204 & -144 & 1798 & 372 & -1942 & 756 & 396 & 576 & 36 & -144 & 396 & 576 & 36 & -144 \\
-144 & -204 & -640 & -332 & -1044 & 1884 & 260 & -1196 & -144 & 36 & 576 & 396 & -144 & 36 & 576 & 396 \\
-144 & -144 & -332 & -1152 & -1044 & -1044 & 1082 & 148 & -144 & -144 & -324 & 576 & -144 & -144 & -324 & 576 \\
484 & 1798 & -1044 & -1044 & 32 & -148 & -144 & -144 & 396 & -702 & 756 & 756 & 576 & -324 & -144 & -144 \\
-1800 & 372 & 1884 & -1044 & -148 & -352 & -244 & -144 & 664 & 316 & -620 & 756 & 396 & 576 & 36 & -144 \\
756 & -1942 & 260 & 1082 & -144 & -244 & -736 & -340 & -1044 & 542 & 236 & -82 & -144 & 36 & 576 & 396 \\
756 & 756 & -1196 & 148 & -144 & -144 & -340 & -1120 & -1044 & -1044 & -36 & 156 & -144 & -144 & -324 & 576 \\
576 & 396 & -144 & -144 & 396 & 664 & -1044 & -1044 & -320 & -220 & -144 & -144 & 308 & 24 & 756 & 756 \\
-324 & 576 & 36 & -144 & -702 & 316 & 542 & -1044 & -220 & -576 & -284 & -144 & -98 & 260 & 258 & 756 \\
-144 & 36 & 576 & -324 & 756 & -620 & 236 & -36 & -144 & -284 & -832 & -348 & -1044 & -356 & 212 & 660 \\
-144 & -144 & 396 & 576 & 756 & 756 & -82 & 156 & -144 & -144 & -348 & -1088 & -1044 & -1044 & -782 & 164 \\
576 & 396 & -144 & -144 & 576 & 396 & -144 & -144 & 308 & -98 & -1044 & -1044 & -672 & -292 & -144 & -144 \\
-324 & 576 & 36 & -144 & -324 & 576 & 36 & -144 & 24 & 260 & -356 & -1044 & -292 & -800 & -324 & -144 \\
-144 & 36 & 576 & -324 & -144 & 36 & 576 & -324 & 756 & 258 & 212 & -782 & -144 & -324 & -928 & -356 \\
-144 & -144 & 396 & 576 & -144 & -144 & 396 & 576 & 756 & 756 & 660 & 164 & -144 & -144 & -356 & -1056
\end{pmatrix}$$

$$H_{3412} = \frac{1}{6 \cdot 5^6} \times \begin{pmatrix}
1280 & -40 & -432 & -432 & -40 & 1541 & 216 & 216 & -432 & 216 & 0 & 0 & -432 & 216 & 0 & 0 \\
-40 & 992 & -112 & -432 & -1411 & -88 & 2231 & 216 & 0 & -432 & 288 & 0 & 0 & -432 & 288 & 0 \\
-432 & -112 & 704 & -184 & 0 & -2125 & -136 & 3317 & 576 & -72 & -432 & 216 & 576 & -72 & -432 & 216 \\
-432 & -432 & -184 & 416 & 0 & 0 & -3235 & -184 & 576 & 576 & 0 & -432 & 576 & 576 & 0 & -432 \\
-40 & -1411 & 0 & 0 & 992 & -88 & -432 & -432 & -112 & 2231 & 288 & 288 & -432 & 216 & 0 & 0 \\
1541 & -88 & -2125 & 0 & -88 & 896 & -112 & -432 & -2125 & -112 & 2069 & 288 & 0 & -432 & 288 & 0 \\
216 & 2231 & -136 & -3235 & -432 & -112 & 800 & -136 & -72 & -1963 & -112 & 2231 & 576 & -72 & -432 & 216 \\
216 & 216 & 3317 & -184 & -432 & -432 & -136 & 704 & -72 & -72 & -2125 & -112 & 576 & 576 & 0 & -432 \\
-432 & 0 & 576 & 576 & -112 & -2125 & -72 & -72 & 704 & -136 & -432 & -432 & -184 & 3317 & 216 & 216 \\
216 & -432 & -72 & 576 & 2231 & -112 & -1963 & -72 & -136 & 800 & -112 & -432 & -3235 & -136 & 2231 & 216 \\
0 & 288 & -432 & 0 & 288 & 2069 & -112 & -2125 & -432 & -112 & 896 & -88 & 0 & -2125 & -88 & 1541 \\
0 & 0 & 216 & -432 & 288 & 288 & 2231 & -112 & -432 & -432 & -88 & 992 & 0 & 0 & -1411 & -40 \\
-432 & 0 & 576 & 576 & -432 & 0 & 576 & 576 & -184 & -3235 & 0 & 0 & 416 & -184 & -432 & -432 \\
216 & -432 & -72 & 576 & 216 & -432 & -72 & 576 & 3317 & -136 & -2125 & 0 & -184 & 704 & -112 & -432 \\
0 & 288 & -432 & 0 & 0 & 288 & -432 & 0 & 216 & 2231 & -88 & -1411 & -432 & -112 & 992 & -40 \\
0 & 0 & 216 & -432 & 0 & 0 & 216 & -432 & 216 & 216 & 1541 & -40 & -432 & -432 & -40 & 1280
\end{pmatrix}$$

$$H_{3421} = \frac{1}{6 \cdot 5^6} \times \begin{pmatrix}
-192 & 248 & 432 & 432 & 328 & -447 & -216 & -216 & 432 & -216 & 0 & 0 & 432 & -216 & 0 & 0 \\
248 & -416 & 192 & 432 & 433 & 264 & 611 & -216 & 0 & 432 & -288 & 0 & 0 & 432 & -288 & 0 \\
432 & 192 & -640 & 136 & 0 & -657 & 200 & 2161 & -576 & 72 & 432 & -216 & -576 & 72 & 432 & -216 \\
432 & 432 & 136 & -864 & 0 & 0 & -2239 & 136 & -576 & -576 & 0 & 432 & -576 & -576 & 0 & 432 \\
328 & 433 & 0 & 0 & 224 & 344 & 432 & 432 & 432 & -1629 & -288 & -288 & 432 & -216 & 0 & 0 \\
-447 & 264 & -657 & 0 & 344 & -64 & 272 & 432 & 1663 & 352 & -575 & -288 & 0 & 432 & -288 & 0 \\
-216 & 611 & 200 & -2239 & 432 & 272 & -352 & 200 & 72 & 569 & 272 & 611 & -576 & 72 & 432 & -216 \\
-216 & -216 & 2161 & 136 & 432 & 432 & 200 & -640 & 72 & 72 & -657 & 192 & -576 & -576 & 0 & 432 \\
432 & 0 & -576 & -576 & 432 & 1663 & 72 & 72 & 640 & 440 & 432 & 432 & 536 & -3039 & -216 & -216 \\
-216 & 432 & 72 & -576 & -1629 & 352 & 569 & 72 & 440 & 288 & 352 & 432 & 3121 & 440 & -1629 & -216 \\
0 & -288 & 432 & 0 & -288 & -575 & 272 & -657 & 432 & 352 & -64 & 264 & 0 & 1663 & 344 & -447 \\
0 & 0 & -216 & 432 & -288 & -288 & 611 & 192 & 432 & 432 & 264 & -416 & 0 & 0 & 433 & 248 \\
432 & 0 & -576 & -576 & 432 & 0 & -576 & -576 & 536 & 3121 & 0 & 0 & 1056 & 536 & 432 & 432 \\
-216 & 432 & 72 & -576 & -216 & 432 & 72 & -576 & -3039 & 440 & 1663 & 0 & 536 & 640 & 432 & 432 \\
0 & -288 & 432 & 0 & 0 & -288 & 432 & 0 & -216 & -1629 & 344 & 433 & 432 & 432 & 224 & 328 \\
0 & 0 & -216 & 432 & 0 & 0 & -216 & 432 & -216 & -216 & -447 & 248 & 432 & 432 & 328 & -192
\end{pmatrix}$$

$$H_{4123} = \frac{1}{6 \cdot 5^6} \times \begin{pmatrix}
528 & -272 & -576 & -576 & -232 & 2646 & 324 & 324 & -576 & -396 & 144 & 144 & -576 & -396 & 144 & 144 \\
-272 & 752 & -216 & -576 & -2810 & -208 & 1950 & 324 & 324 & -576 & -36 & 144 & 324 & -576 & -36 & 144 \\
-576 & -216 & 976 & -160 & -396 & -2102 & -184 & 1458 & 144 & -36 & -576 & 324 & 144 & -36 & -576 & 324 \\
-576 & -576 & -160 & 1200 & -396 & -396 & -1598 & -160 & 144 & 144 & -396 & -576 & 144 & 144 & -396 & -576 \\
-232 & -2810 & -396 & -396 & 1072 & -168 & -576 & -576 & -96 & 3530 & -36 & -36 & -576 & -396 & 144 & 144 \\
2646 & -208 & -2102 & -396 & -168 & 1040 & -176 & -576 & -3642 & -136 & 2746 & -36 & 324 & -576 & -36 & 144 \\
324 & 1950 & -184 & -1598 & -576 & -176 & 1008 & -184 & -36 & -2878 & -176 & 1950 & 144 & -36 & -576 & 324 \\
324 & 324 & 1458 & -160 & -576 & -576 & -184 & 976 & -36 & -36 & -2102 & -216 & 144 & 144 & -396 & -576 \\
-576 & 324 & 144 & 144 & -96 & -3642 & -36 & -36 & 1616 & -64 & -576 & -576 & 40 & 3898 & -396 & -396 \\
-396 & -576 & -36 & 144 & 3530 & -136 & -2878 & -36 & -64 & 1328 & -136 & -576 & -3958 & -64 & 3530 & -396 \\
144 & -36 & -576 & -396 & -36 & 2746 & -176 & -2102 & -576 & -136 & 1040 & -208 & 324 & -3642 & -168 & 2646 \\
144 & 144 & 324 & -576 & -36 & -36 & 1950 & -216 & -576 & -576 & -208 & 752 & 324 & 324 & -2810 & -272 \\
-576 & 324 & 144 & 144 & -576 & 324 & 144 & 144 & 40 & -3958 & 324 & 324 & 2160 & 40 & -576 & -576 \\
-396 & -576 & -36 & 144 & -396 & -576 & -36 & 144 & 3898 & -64 & -3642 & 324 & 40 & 1616 & -96 & -576 \\
144 & -36 & -576 & -396 & 144 & -36 & -576 & -396 & -396 & 3530 & -168 & -2810 & -576 & -96 & 1072 & -232 \\
144 & 144 & 324 & -576 & 144 & 144 & 324 & -576 & -396 & -396 & 2646 & -272 & -576 & -576 & -232 & 528
\end{pmatrix}$$

$$H_{4132} = \frac{1}{6 \cdot 5^6} \times \begin{pmatrix} -1056 & -356 & -144 & -144 & 164 & 660 & 756 & 756 & 576 & 396 & -144 & -144 & 576 & 396 & -144 & -144 \\ -356 & -928 & -324 & -144 & -782 & 212 & 258 & 756 & -324 & 576 & 36 & -144 & -324 & 576 & 36 & -144 \\ -144 & -324 & -800 & -292 & -1044 & -356 & 260 & 24 & -144 & 36 & 576 & -324 & -144 & 36 & 576 & -324 \\ -144 & -144 & -292 & -672 & -1044 & -1044 & -98 & 308 & -144 & -144 & 396 & 576 & -144 & -144 & 396 & 576 \\ 164 & -782 & -1044 & -1044 & -1088 & -348 & -144 & -144 & 156 & -82 & 756 & 756 & 576 & 396 & -144 & -144 \\ 660 & 212 & -356 & -1044 & -348 & -832 & -284 & -144 & -36 & 236 & -620 & 756 & -324 & 576 & 36 & -144 \\ 756 & 258 & 260 & -98 & -144 & -284 & -576 & -220 & -1044 & 542 & 316 & -702 & -144 & 36 & 576 & -324 \\ 756 & 756 & 24 & 308 & -144 & -144 & -220 & -320 & -1044 & -1044 & 664 & 396 & -144 & -144 & 396 & 576 \\ 576 & -324 & -144 & -144 & 156 & -36 & -1044 & -1044 & -1120 & -340 & -144 & -144 & 148 & -1196 & 756 & 756 \\ 396 & 576 & 36 & -144 & -82 & 236 & 542 & -1044 & -340 & -736 & -244 & -144 & 1082 & 260 & -1942 & 756 \\ -144 & 36 & 576 & 396 & 756 & -620 & 316 & 664 & -144 & -244 & -352 & -148 & -1044 & 1884 & 372 & -1800 \\ -144 & -144 & -324 & 576 & 756 & 756 & -702 & 396 & -144 & -144 & -148 & 32 & -1044 & -1044 & 1798 & 484 \\ 576 & -324 & -144 & -144 & 576 & -324 & -144 & -144 & 148 & 1082 & -1044 & -1044 & -1152 & -332 & -144 & -144 \\ 396 & 576 & 36 & -144 & 396 & 576 & 36 & -144 & -1196 & 260 & 1884 & -1044 & -332 & -640 & -204 & -144 \\ -144 & 36 & 576 & 396 & -144 & 36 & 576 & 396 & 756 & -1942 & 372 & 1798 & -144 & -204 & -128 & -76 \\ -144 & -144 & -324 & 576 & -144 & -144 & -324 & 576 & 756 & 756 & -1800 & 484 & -144 & -144 & -76 & 384 \end{pmatrix}$$

$$H_{4213} = \frac{1}{6 \cdot 5^6} \times \begin{pmatrix} 384 & 484 & 576 & 576 & -76 & -1800 & -324 & -324 & -144 & 756 & -144 & -144 & -144 & 756 & -144 & -144 \\ 484 & 32 & 396 & 576 & 1798 & -148 & -702 & -324 & -1044 & -144 & 756 & -144 & -1044 & -144 & 756 & -144 \\ 576 & 396 & -320 & 308 & 396 & 664 & -220 & 24 & -144 & -1044 & -144 & 756 & -144 & -1044 & -144 & 756 \\ 576 & 576 & 308 & -672 & 396 & 396 & -98 & -292 & -144 & -144 & -1044 & -144 & -144 & -144 & -1044 & -144 \\ -76 & 1798 & 396 & 396 & -128 & 372 & 576 & 576 & -204 & -1942 & 36 & 36 & -144 & 756 & -144 & -144 \\ -1800 & -148 & 664 & 396 & 372 & -352 & 316 & 576 & 1884 & -244 & -620 & 36 & -1044 & -144 & 756 & -144 \\ -324 & -702 & -220 & -98 & 576 & 316 & -576 & 260 & 36 & 542 & -284 & 258 & -144 & -1044 & -144 & 756 \\ -324 & -324 & 24 & -292 & 576 & 576 & 260 & -800 & 36 & 36 & -356 & -324 & -144 & -144 & -1044 & -144 \\ -144 & -1044 & -144 & -144 & -204 & 1884 & 36 & 36 & -640 & 260 & 576 & 576 & -332 & -1196 & 396 & 396 \\ 756 & -144 & -1044 & -144 & -1942 & -244 & 542 & 36 & 260 & -736 & 236 & 576 & 1082 & -340 & -82 & 396 \\ -144 & 756 & -144 & -1044 & 36 & -620 & -284 & -356 & 576 & 236 & -832 & 212 & -324 & -36 & -348 & 660 \\ -144 & -144 & 756 & -144 & 36 & 36 & 258 & -324 & 576 & 576 & 212 & -928 & -324 & -324 & -782 & -356 \\ -144 & -1044 & -144 & -144 & -144 & -1044 & -144 & -144 & -332 & 1082 & -324 & -324 & -1152 & 148 & 576 & 576 \\ 756 & -144 & -1044 & -144 & 756 & -144 & -1044 & -144 & -1196 & -340 & -36 & -324 & 148 & -1120 & 156 & 576 \\ -144 & 756 & -144 & -1044 & -144 & 756 & -144 & -1044 & 396 & -82 & -348 & -782 & 576 & 156 & -1088 & 164 \\ -144 & -144 & 756 & -144 & -144 & -144 & 756 & -144 & 396 & 396 & 660 & -356 & 576 & 576 & 164 & -1056 \end{pmatrix}$$

$$H_{4231} = \frac{1}{6 \cdot 5^6} \times \begin{pmatrix} -80 & 40 & 144 & 144 & 40 & 382 & -756 & -756 & 144 & -756 & 144 & 144 & 144 & -756 & 144 & 144 \\ 40 & -464 & -56 & 144 & -162 & -24 & 738 & -756 & 1044 & 144 & -756 & 144 & 1044 & 144 & -756 & 144 \\ 144 & -56 & -848 & -152 & 1044 & -550 & -88 & 350 & 144 & 1044 & 144 & -756 & 144 & 1044 & 144 & -756 \\ 144 & 144 & -152 & -1232 & 1044 & 1044 & -194 & -152 & 144 & 144 & 1044 & 144 & 144 & 144 & 1044 & 144 \\ 40 & -162 & 1044 & 1044 & -464 & -24 & 144 & 144 & -56 & 738 & -756 & -756 & 144 & -756 & 144 & 144 \\ 382 & -24 & -550 & 1044 & -24 & -592 & -56 & 144 & -550 & -56 & 1182 & -756 & 1044 & 144 & -756 & 144 \\ -756 & 738 & -88 & -194 & 144 & -56 & -720 & -88 & 1044 & -994 & -56 & 738 & 144 & 1044 & 144 & -756 \\ -756 & -756 & 350 & -152 & 144 & 144 & -88 & -848 & 1044 & 1044 & -550 & -56 & 144 & 144 & 1044 & 144 \\ 144 & 1044 & 144 & 144 & -56 & -550 & 1044 & 1044 & -848 & -88 & 144 & 144 & -152 & 350 & -756 & -756 \\ -756 & 144 & 1044 & 144 & 738 & -56 & -994 & 1044 & -88 & -720 & -56 & 144 & -194 & -88 & 738 & -756 \\ 144 & -756 & 144 & 1044 & -756 & 1182 & -56 & -550 & 144 & -56 & -592 & -24 & 1044 & -550 & -24 & 382 \\ 144 & 144 & -756 & 144 & -756 & -756 & 738 & -56 & 144 & 144 & -24 & -464 & 1044 & 1044 & -162 & 40 \\ 144 & 1044 & 144 & 144 & 144 & 1044 & 144 & 144 & -152 & -194 & 1044 & 1044 & -1232 & -152 & 144 & 144 \\ -756 & 144 & 1044 & 144 & -756 & 144 & 1044 & 144 & 350 & -88 & -550 & 1044 & -152 & -848 & -56 & 144 \\ 144 & -756 & 144 & 1044 & 144 & -756 & 144 & 1044 & -756 & 738 & -24 & -162 & 144 & -56 & -464 & 40 \\ 144 & 144 & -756 & 144 & 144 & 144 & -756 & 144 & -756 & -756 & 382 & 40 & 144 & 144 & 40 & -80 \end{pmatrix}$$

$$H_{4312} = \frac{1}{6 \cdot 5^6} \times \begin{pmatrix} -192 & 328 & 432 & 432 & 248 & -447 & -216 & -216 & 432 & -216 & 0 & 0 & 432 & -216 & 0 & 0 \\ 328 & 224 & 432 & 432 & 433 & 344 & -1629 & -216 & 0 & 432 & -288 & 0 & 0 & 432 & -288 & 0 \\ 432 & 432 & 640 & 536 & 0 & 1663 & 440 & -3039 & -576 & 72 & 432 & -216 & -576 & 72 & 432 & -216 \\ 432 & 432 & 536 & 1056 & 0 & 0 & 3121 & 536 & -576 & -576 & 0 & 432 & -576 & -576 & 0 & 432 \\ 248 & 433 & 0 & 0 & -416 & 264 & 432 & 432 & 192 & 611 & -288 & -288 & 432 & -216 & 0 & 0 \\ -447 & 344 & 1663 & 0 & 264 & -64 & 352 & 432 & -657 & 272 & -575 & -288 & 0 & 432 & -288 & 0 \\ -216 & -1629 & 440 & 3121 & 432 & 352 & 288 & 440 & 72 & 569 & 352 & -1629 & -576 & 72 & 432 & -216 \\ -216 & -216 & -3039 & 536 & 432 & 432 & 440 & 640 & 72 & 72 & 1663 & 432 & -576 & -576 & 0 & 432 \\ 432 & 0 & -576 & -576 & 192 & -657 & 72 & 72 & -640 & 200 & 432 & 432 & 136 & 2161 & -216 & -216 \\ -216 & 432 & 72 & -576 & 611 & 272 & 569 & 72 & 200 & -352 & 272 & 432 & -2239 & 200 & 611 & -216 \\ 0 & -288 & 432 & 0 & -288 & -575 & 352 & 1663 & 432 & 272 & -64 & 344 & 0 & -657 & 264 & -447 \\ 0 & 0 & -216 & 432 & -288 & -288 & -1629 & 432 & 432 & 432 & 344 & 224 & 0 & 0 & 433 & 328 \\ 432 & 0 & -576 & -576 & 432 & 0 & -576 & -576 & 136 & -2239 & 0 & 0 & -864 & 136 & 432 & 432 \\ -216 & 432 & 72 & -576 & -216 & 432 & 72 & -576 & 2161 & 200 & -657 & 0 & 136 & -640 & 192 & 432 \\ 0 & -288 & 432 & 0 & 0 & -288 & 432 & 0 & -216 & 611 & 264 & 433 & 432 & 192 & -416 & 248 \\ 0 & 0 & -216 & 432 & 0 & 0 & -216 & 432 & -216 & -216 & -447 & 328 & 432 & 432 & 248 & -192 \end{pmatrix}$$

$$H_{4321} = \frac{1}{6 \cdot 5^6} \times \begin{pmatrix} 928 & -32 & -432 & -432 & -32 & -2435 & 216 & 216 & -432 & 216 & 0 & 0 & -432 & 216 & 0 & 0 \\ -32 & 1408 & 88 & -432 & 2601 & 48 & -3357 & 216 & 0 & -432 & 288 & 0 & 0 & -432 & 288 & 0 \\ -432 & 88 & 1888 & 208 & 0 & 3563 & 128 & -4195 & 576 & -72 & -432 & 216 & 576 & -72 & -432 & 216 \\ -432 & -432 & 208 & 2368 & 0 & 0 & 4441 & 208 & 576 & 576 & 0 & -432 & 576 & 576 & 0 & -432 \\ -32 & 2601 & 0 & 0 & 1408 & 48 & -432 & -432 & 88 & -3357 & 288 & 288 & -432 & 216 & 0 & 0 \\ -2435 & 48 & 3563 & 0 & 48 & 1568 & 88 & -432 & 3563 & 88 & -3507 & 288 & 0 & -432 & 288 & 0 \\ 216 & -3357 & 128 & 4441 & -432 & 88 & 1728 & 128 & -72 & 3713 & 88 & -3357 & 576 & -72 & -432 & 216 \\ 216 & 216 & -4195 & 208 & -432 & -432 & 128 & 1888 & -72 & -72 & 3563 & 88 & 576 & 576 & 0 & -432 \\ -432 & 0 & 576 & 576 & 88 & 3563 & -72 & -72 & 1888 & 128 & -432 & -432 & 208 & -4195 & 216 & 216 \\ 216 & -432 & -72 & 576 & -3357 & 88 & 3713 & -72 & 128 & 1728 & 88 & -432 & 4441 & 128 & -3357 & 216 \\ 0 & 288 & -432 & 0 & 288 & -3507 & 88 & 3563 & -432 & 88 & 1568 & 48 & 0 & 3563 & 48 & -2435 \\ 0 & 0 & 216 & -432 & 288 & 288 & -3357 & 88 & -432 & -432 & 48 & 1408 & 0 & 0 & 2601 & -32 \\ -432 & 0 & 576 & 576 & -432 & 0 & 576 & 576 & 208 & 4441 & 0 & 0 & 2368 & 208 & -432 & -432 \\ 216 & -432 & -72 & 576 & 216 & -432 & -72 & 576 & -4195 & 128 & 3563 & 0 & 208 & 1888 & 88 & -432 \\ 0 & 288 & -432 & 0 & 0 & 288 & -432 & 0 & 216 & -3357 & 48 & 2601 & -432 & 88 & 1408 & -32 \\ 0 & 0 & 216 & -432 & 0 & 0 & 216 & -432 & 216 & 216 & -2435 & -32 & -432 & -432 & -32 & 928 \end{pmatrix}$$

# Appendix 2

$\mathbf{S} = \{\mathbf{1234}, \mathbf{2143}, \mathbf{3412}, \mathbf{4321}\}, \lambda_{max} = 0.136488, \lambda_{min} = 0.009351$

$$H_S = \frac{1}{6 \cdot 5^6} \times \begin{pmatrix}
4992 & -48 & -1728 & -1728 & -48 & 312 & 432 & 432 & -1728 & 432 & 1152 & 1152 & -1728 & 432 & 1152 & 1152 \\
-48 & 4992 & -48 & -1728 & 312 & -48 & 312 & 432 & 432 & -1728 & 432 & 1152 & 432 & -1728 & 432 & 1152 \\
-1728 & -48 & 4992 & -48 & 432 & 312 & -48 & 312 & 1152 & 432 & -1728 & 432 & 1152 & 432 & -1728 & 432 \\
-1728 & -1728 & -48 & 4992 & 432 & 432 & 312 & -48 & 1152 & 1152 & 432 & -1728 & 1152 & 1152 & 432 & -1728 \\
-48 & 312 & 432 & 432 & 4992 & -48 & -1728 & -1728 & -48 & 312 & 432 & 432 & -1728 & 432 & 1152 & 1152 \\
312 & -48 & 312 & 432 & -48 & 4992 & -48 & -1728 & 312 & -48 & 312 & 432 & 432 & -1728 & 432 & 1152 \\
432 & 312 & -48 & 312 & -1728 & -48 & 4992 & -48 & 432 & 312 & -48 & 312 & 1152 & 432 & -1728 & 432 \\
432 & 432 & 312 & -48 & -1728 & -1728 & -48 & 4992 & 432 & 432 & 312 & -48 & 1152 & 1152 & 432 & -1728 \\
-1728 & 432 & 1152 & 1152 & -48 & 312 & 432 & 432 & 4992 & -48 & -1728 & -1728 & -48 & 312 & 432 & 432 \\
432 & -1728 & 432 & 1152 & 312 & -48 & 312 & 432 & -48 & 4992 & -48 & -1728 & 312 & -48 & 312 & 432 \\
1152 & 432 & -1728 & 432 & 432 & 312 & -48 & 312 & -1728 & -48 & 4992 & -48 & 432 & 312 & -48 & 312 \\
1152 & 1152 & 432 & -1728 & 432 & 432 & 312 & -48 & -1728 & -1728 & -48 & 4992 & 432 & 432 & 312 & -48 \\
-1728 & 432 & 1152 & 1152 & -1728 & 432 & 1152 & 1152 & -48 & 312 & 432 & 432 & 4992 & -48 & -1728 & -1728 \\
432 & -1728 & 432 & 1152 & 432 & -1728 & 432 & 1152 & 312 & -48 & 312 & 432 & -48 & 4992 & -48 & -1728 \\
1152 & 432 & -1728 & 432 & 1152 & 432 & -1728 & 432 & 432 & 312 & -48 & 312 & -1728 & -48 & 4992 & -48 \\
1152 & 1152 & 432 & -1728 & 1152 & 1152 & 432 & -1728 & 432 & 432 & 312 & -48 & -1728 & -1728 & -48 & 4992
\end{pmatrix}$$

$S = \{1234, 2143, 3421, 4312\}, \lambda_{max} = 0.065772, \lambda_{min} = -0.013328$

$$H_S = \frac{1}{6 \cdot 5^6} \times \begin{pmatrix}
2400 & 600 & 0 & 0 & 600 & 312 & -432 & -432 & 0 & -432 & 1152 & 1152 & 0 & -432 & 1152 & 1152 \\
600 & 2400 & 600 & 0 & -12 & 600 & 420 & -432 & 432 & 0 & -720 & 1152 & 432 & 0 & -720 & 1152 \\
0 & 600 & 2400 & 600 & 432 & -120 & 600 & 312 & -1152 & 720 & 0 & -432 & -1152 & 720 & 0 & -432 \\
0 & 0 & 600 & 2400 & 432 & 432 & -12 & 600 & -1152 & -1152 & 432 & 0 & -1152 & -1152 & 432 & 0 \\
600 & -12 & 432 & 432 & 2400 & 600 & 0 & 0 & 600 & 420 & -720 & -720 & 0 & -432 & 1152 & 1152 \\
312 & 600 & -120 & 432 & 600 & 2400 & 600 & 0 & -120 & 600 & 600 & -720 & 432 & 0 & -720 & 1152 \\
-432 & 420 & 600 & -12 & 0 & 600 & 2400 & 600 & 720 & -300 & 600 & 420 & -1152 & 720 & 0 & -432 \\
-432 & -432 & 312 & 600 & 0 & 0 & 600 & 2400 & 720 & 720 & -120 & 600 & -1152 & -1152 & 432 & 0 \\
0 & 432 & -1152 & -1152 & 600 & -120 & 720 & 720 & 2400 & 600 & 0 & 0 & 600 & 312 & -432 & -432 \\
-432 & 0 & 720 & -1152 & 420 & 600 & -300 & 720 & 600 & 2400 & 600 & 0 & -12 & 600 & 420 & -432 \\
1152 & -720 & 0 & 432 & -720 & 600 & 600 & -120 & 0 & 600 & 2400 & 600 & 432 & -120 & 600 & 312 \\
1152 & 1152 & -432 & 0 & -720 & -720 & 420 & 600 & 0 & 0 & 600 & 2400 & 432 & 432 & -12 & 600 \\
0 & 432 & -1152 & -1152 & 0 & 432 & -1152 & -1152 & 600 & -12 & 432 & 432 & 2400 & 600 & 0 & 0 \\
-432 & 0 & 720 & -1152 & -432 & 0 & 720 & -1152 & 312 & 600 & -120 & 432 & 600 & 2400 & 600 & 0 \\
1152 & -720 & 0 & 432 & 1152 & -720 & 0 & 432 & -432 & 420 & 600 & -12 & 0 & 600 & 2400 & 600 \\
1152 & 1152 & -432 & 0 & 1152 & 1152 & -432 & 0 & -432 & -432 & 312 & 600 & 0 & 0 & 600 & 2400
\end{pmatrix}$$

$S = \{1234, 2341, 3412, 4123\}, \lambda_{max} = 0.413046, \lambda_{min} = -0.220271$

$$H_S = \frac{1}{6 \cdot 5^6} \times \begin{pmatrix}
4704 & -336 & -2016 & -2016 & -336 & 11274 & 144 & 144 & -2016 & 144 & 864 & 864 & -2016 & 144 & 864 & 864 \\
-336 & 4704 & -336 & -2016 & -11226 & -336 & 11274 & 144 & 144 & -2016 & 144 & 864 & 144 & -2016 & 144 & 864 \\
-2016 & -336 & 4704 & -336 & 144 & -11226 & -336 & 11274 & 864 & 144 & -2016 & 144 & 864 & 144 & -2016 & 144 \\
-2016 & -2016 & -336 & 4704 & 144 & 144 & -11226 & -336 & 864 & 864 & 144 & -2016 & 864 & 864 & 144 & -2016 \\
-336 & -11226 & 144 & 144 & 4704 & -336 & -2016 & -2016 & -336 & 11274 & 144 & 144 & -2016 & 144 & 864 & 864 \\
11274 & -336 & -11226 & 144 & -336 & 4704 & -336 & -2016 & -11226 & -336 & 11274 & 144 & 144 & -2016 & 144 & 864 \\
144 & 11274 & -336 & -11226 & -2016 & -336 & 4704 & -336 & 144 & -11226 & -336 & 11274 & 864 & 144 & -2016 & 144 \\
144 & 144 & 11274 & -336 & -2016 & -2016 & -336 & 4704 & 144 & 144 & -11226 & -336 & 864 & 864 & 144 & -2016 \\
-2016 & 144 & 864 & 864 & -336 & -11226 & 144 & 144 & 4704 & -336 & -2016 & -2016 & -336 & 11274 & 144 & 144 \\
144 & -2016 & 144 & 864 & 11274 & -336 & -11226 & 144 & -336 & 4704 & -336 & -2016 & -11226 & -336 & 11274 & 144 \\
864 & 144 & -2016 & 144 & 144 & 11274 & -336 & -11226 & -2016 & -336 & 4704 & -336 & 144 & -11226 & -336 & 11274 \\
864 & 864 & 144 & -2016 & 144 & 144 & 11274 & -336 & -2016 & -2016 & -336 & 4704 & 144 & 144 & -11226 & -336 \\
-2016 & 144 & 864 & 864 & -2016 & 144 & 864 & 864 & -336 & -11226 & 144 & 144 & 4704 & -336 & -2016 & -2016 \\
144 & -2016 & 144 & 864 & 144 & -2016 & 144 & 864 & 11274 & -336 & -11226 & 144 & -336 & 4704 & -336 & -2016 \\
864 & 144 & -2016 & 144 & 864 & 144 & -2016 & 144 & 144 & 11274 & -336 & -11226 & -2016 & -336 & 4704 & -336 \\
864 & 864 & 144 & -2016 & 864 & 864 & 144 & -2016 & 144 & 144 & 11274 & -336 & -2016 & -2016 & -336 & 4704
\end{pmatrix}$$

$S = \{1234, 2413, 3142, 4321\}, \lambda_{max} = 0.044522, \lambda_{min} = -0.042560$

$$H_S = \frac{1}{6 \cdot 5^6} \times \begin{pmatrix}
384 & -336 & -576 & -576 & -336 & 2094 & 504 & 504 & -576 & 504 & 864 & 864 & -576 & 504 & 864 & 864 \\
-336 & 384 & -336 & -576 & -1506 & -336 & 294 & 504 & 504 & -576 & 504 & 864 & 504 & -576 & 504 & 864 \\
-576 & -336 & 384 & -336 & 504 & 294 & -336 & -1506 & 864 & 504 & -576 & 504 & 864 & 504 & -576 & 504 \\
-576 & -576 & -336 & 384 & 504 & 504 & 2094 & -336 & 864 & 864 & 504 & -576 & 864 & 864 & 504 & -576 \\
-336 & -1506 & 504 & 504 & 384 & -336 & -576 & -576 & -336 & 294 & 504 & 504 & -576 & 504 & 864 & 864 \\
2094 & -336 & 294 & 504 & -336 & 384 & -336 & -576 & 294 & -336 & 294 & 504 & 504 & -576 & 504 & 864 \\
504 & 294 & -336 & 2094 & -576 & -336 & 384 & -336 & 504 & 294 & -336 & 294 & 864 & 504 & -576 & 504 \\
504 & 504 & -1506 & -336 & -576 & -576 & -336 & 384 & 504 & 504 & 294 & -336 & 864 & 864 & 504 & -576 \\
-576 & 504 & 864 & 864 & -336 & 294 & 504 & 504 & 384 & -336 & -576 & -576 & -336 & -1506 & 504 & 504 \\
504 & -576 & 504 & 864 & 294 & -336 & 294 & 504 & -336 & 384 & -336 & -576 & 2094 & -336 & 294 & 504 \\
864 & 504 & -576 & 504 & 504 & 294 & -336 & 294 & -576 & -336 & 384 & -336 & 504 & 294 & -336 & 2094 \\
864 & 864 & 504 & -576 & 504 & 504 & 294 & -336 & -576 & -576 & -336 & 384 & 504 & 504 & -1506 & -336 \\
-576 & 504 & 864 & 864 & -576 & 504 & 864 & 864 & -336 & 2094 & 504 & 504 & 384 & -336 & -576 & -576 \\
504 & -576 & 504 & 864 & 504 & -576 & 504 & 864 & -1506 & -336 & 294 & 504 & -336 & 384 & -336 & -576 \\
864 & 504 & -576 & 504 & 864 & 504 & -576 & 504 & 504 & 294 & -336 & -1506 & -576 & -336 & 384 & -336 \\
864 & 864 & 504 & -576 & 864 & 864 & 504 & -576 & 504 & 504 & 2094 & -336 & -576 & -576 & -336 & 384
\end{pmatrix}$$

$S = \{1243, 2134, 3421, 4312\}, \lambda_{max} = 0.061073, \lambda_{min} = -0.068244$

$$H_S = \frac{1}{6 \cdot 5^6} \times \begin{pmatrix}
-192 & 1248 & 1728 & 1728 & 1248 & -12 & -432 & -432 & 1728 & -432 & -1152 & -1152 & 1728 & -432 & -1152 & -1152 \\
1248 & -192 & 1248 & 1728 & -12 & 1248 & -12 & -432 & -432 & 1728 & -432 & -1152 & -432 & 1728 & -432 & -1152 \\
1728 & 1248 & -192 & 1248 & -432 & -12 & 1248 & -12 & -1152 & -432 & 1728 & -432 & -1152 & -432 & 1728 & -432 \\
1728 & 1728 & 1248 & -192 & -432 & -432 & -12 & 1248 & -1152 & -1152 & -432 & 1728 & -1152 & -1152 & -432 & 1728 \\
1248 & -12 & -432 & -432 & -192 & 1248 & 1728 & 1728 & 1248 & -12 & -432 & -432 & 1728 & -432 & -1152 & -1152 \\
-12 & 1248 & -12 & -432 & 1248 & -192 & 1248 & 1728 & -12 & 1248 & -12 & -432 & -432 & 1728 & -432 & -1152 \\
-432 & -12 & 1248 & -12 & 1728 & 1248 & -192 & 1248 & -432 & -12 & 1248 & -12 & -1152 & -432 & 1728 & -432 \\
-432 & -432 & -12 & 1248 & 1728 & 1728 & 1248 & -192 & -432 & -432 & -12 & 1248 & -1152 & -1152 & -432 & 1728 \\
1728 & -432 & -1152 & -1152 & 1248 & -12 & -432 & -432 & -192 & 1248 & 1728 & 1728 & 1248 & -12 & -432 & -432 \\
-432 & 1728 & -432 & -1152 & -12 & 1248 & -12 & -432 & 1248 & -192 & 1248 & 1728 & -12 & 1248 & -12 & -432 \\
-1152 & -432 & 1728 & -432 & -432 & -12 & 1248 & -12 & 1728 & 1248 & -192 & 1248 & -432 & -12 & 1248 & -12 \\
-1152 & -1152 & -432 & 1728 & -432 & -432 & -12 & 1248 & 1728 & 1728 & 1248 & -192 & -432 & -432 & -12 & 1248 \\
1728 & -432 & -1152 & -1152 & 1728 & -432 & -1152 & -1152 & 1248 & -12 & -432 & -432 & -192 & 1248 & 1728 & 1728 \\
-432 & 1728 & -432 & -1152 & -432 & 1728 & -432 & -1152 & -12 & 1248 & -12 & -432 & 1248 & -192 & 1248 & 1728 \\
-1152 & -432 & 1728 & -432 & -1152 & -432 & 1728 & -432 & -432 & -12 & 1248 & -12 & 1728 & 1248 & -192 & 1248 \\
-1152 & -1152 & -432 & 1728 & -1152 & -1152 & -432 & 1728 & -432 & -432 & -12 & 1248 & 1728 & 1728 & 1248 & -192
\end{pmatrix}$$

$S = \{1243, 2314, 3421, 4132\}, \lambda_{max} = 0.100615, \lambda_{min} = -0.125342$

$$H_S = \frac{1}{6 \cdot 5^6} \times \begin{pmatrix}
-1344 & 96 & 576 & 576 & 1176 & 4416 & -504 & -504 & 2016 & -144 & -864 & -864 & 2016 & -144 & -864 & -864 \\
96 & -1344 & 96 & 576 & -4584 & 1176 & 4416 & -504 & -144 & 2016 & -144 & -864 & -144 & 2016 & -144 & -864 \\
576 & 96 & -1344 & 96 & -504 & -4584 & 1176 & 4416 & -864 & -144 & 2016 & -144 & -864 & -144 & 2016 & -144 \\
576 & 576 & 96 & -1344 & -504 & -504 & -4584 & 1176 & -864 & -864 & -144 & 2016 & -864 & -864 & -144 & 2016 \\
1176 & -4584 & -504 & -504 & -1344 & 96 & 576 & 576 & 1176 & -84 & -504 & -504 & 2016 & -144 & -864 & -864 \\
4416 & 1176 & -4584 & -504 & 96 & -1344 & 96 & 576 & -84 & 1176 & -84 & -504 & -144 & 2016 & -144 & -864 \\
-504 & 4416 & 1176 & -4584 & 576 & 96 & -1344 & 96 & -504 & -84 & 1176 & -84 & -864 & -144 & 2016 & -144 \\
-504 & -504 & 4416 & 1176 & 576 & 576 & 96 & -1344 & -504 & -504 & -84 & 1176 & -864 & -864 & -144 & 2016 \\
2016 & -144 & -864 & -864 & 1176 & -84 & -504 & -504 & -1344 & 96 & 576 & 576 & 1176 & -4584 & -504 & -504 \\
-144 & 2016 & -144 & -864 & -84 & 1176 & -84 & -504 & 96 & -1344 & 96 & 576 & 4416 & 1176 & -4584 & -504 \\
-864 & -144 & 2016 & -144 & -504 & -84 & 1176 & -84 & 576 & 96 & -1344 & 96 & -504 & 4416 & 1176 & -4584 \\
-864 & -864 & -144 & 2016 & -504 & -504 & -84 & 1176 & 576 & 576 & 96 & -1344 & -504 & -504 & 4416 & 1176 \\
2016 & -144 & -864 & -864 & 2016 & -144 & -864 & -864 & 1176 & 4416 & -504 & -504 & -1344 & 96 & 576 & 576 \\
-144 & 2016 & -144 & -864 & -144 & 2016 & -144 & -864 & -4584 & 1176 & 4416 & -504 & 96 & -1344 & 96 & 576 \\
-864 & -144 & 2016 & -144 & -864 & -144 & 2016 & -144 & -504 & -4584 & 1176 & 4416 & 576 & 96 & -1344 & 96 \\
-864 & -864 & -144 & 2016 & -864 & -864 & -144 & 2016 & -504 & -504 & -4584 & 1176 & 576 & 576 & 96 & -1344
\end{pmatrix}$$

$S = \{1324, 2143, 3412, 4231\}, \lambda_{max} = 0.044522, \lambda_{min} = -0.042560$

$$H_S = \frac{1}{6 \cdot 5^6} \times \begin{pmatrix}
384 & -336 & -576 & -576 & -336 & -1506 & 504 & 504 & -576 & 504 & 864 & 864 & -576 & 504 & 864 & 864 \\
-336 & 384 & -336 & -576 & 2094 & -336 & 294 & 504 & 504 & -576 & 504 & 864 & 504 & -576 & 504 & 864 \\
-576 & -336 & 384 & -336 & 504 & 294 & -336 & 2094 & 864 & 504 & -576 & 504 & 864 & 504 & -576 & 504 \\
-576 & -576 & -336 & 384 & 504 & 504 & -1506 & -336 & 864 & 864 & 504 & -576 & 864 & 864 & 504 & -576 \\
-336 & 2094 & 504 & 504 & 384 & -336 & -576 & -576 & -336 & 294 & 504 & 504 & -576 & 504 & 864 & 864 \\
-1506 & -336 & 294 & 504 & -336 & 384 & -336 & -576 & 294 & -336 & 294 & 504 & 504 & -576 & 504 & 864 \\
504 & 294 & -336 & -1506 & -576 & -336 & 384 & -336 & 504 & 294 & -336 & 294 & 864 & 504 & -576 & 504 \\
504 & 504 & 2094 & -336 & -576 & -576 & -336 & 384 & 504 & 504 & 294 & -336 & 864 & 864 & 504 & -576 \\
-576 & 504 & 864 & 864 & -336 & 294 & 504 & 504 & 384 & -336 & -576 & -576 & -336 & 2094 & 504 & 504 \\
504 & -576 & 504 & 864 & 294 & -336 & 294 & 504 & -336 & 384 & -336 & -576 & -1506 & -336 & 294 & 504 \\
864 & 504 & -576 & 504 & 504 & 294 & -336 & 294 & -576 & -336 & 384 & -336 & 504 & 294 & -336 & -1506 \\
864 & 864 & 504 & -576 & 504 & 504 & 294 & -336 & -576 & -576 & -336 & 384 & 504 & 504 & 2094 & -336 \\
-576 & 504 & 864 & 864 & -576 & 504 & 864 & 864 & -336 & -1506 & 504 & 504 & 384 & -336 & -576 & -576 \\
504 & -576 & 504 & 864 & 504 & -576 & 504 & 864 & 2094 & -336 & 294 & 504 & -336 & 384 & -336 & -576 \\
864 & 504 & -576 & 504 & 864 & 504 & -576 & 504 & 504 & 294 & -336 & 2094 & -576 & -336 & 384 & -336 \\
864 & 864 & 504 & -576 & 864 & 864 & 504 & -576 & 504 & 504 & -1506 & -336 & -576 & -576 & -336 & 384
\end{pmatrix}$$

$S = \{1324, 2413, 3142, 4231\}, \lambda_{max} = 0.003853, \lambda_{min} = -0.083022$

$$H_S = \frac{1}{6 \cdot 5^6} \times \begin{pmatrix}
-4224 & -624 & 576 & 576 & -624 & 276 & 576 & 576 & 576 & 576 & 576 & 576 & 576 & 576 & 576 & 576 \\
-624 & -4224 & -624 & 576 & 276 & -624 & 276 & 576 & 576 & 576 & 576 & 576 & 576 & 576 & 576 & 576 \\
576 & -624 & -4224 & -624 & 576 & 276 & -624 & 276 & 576 & 576 & 576 & 576 & 576 & 576 & 576 & 576 \\
576 & 576 & -624 & -4224 & 576 & 576 & 276 & -624 & 576 & 576 & 576 & 576 & 576 & 576 & 576 & 576 \\
-624 & 276 & 576 & 576 & -4224 & -624 & 576 & 576 & -624 & 276 & 576 & 576 & 576 & 576 & 576 & 576 \\
276 & -624 & 276 & 576 & -624 & -4224 & -624 & 576 & 276 & -624 & 276 & 576 & 576 & 576 & 576 & 576 \\
576 & 276 & -624 & 276 & 576 & -624 & -4224 & -624 & 576 & 276 & -624 & 276 & 576 & 576 & 576 & 576 \\
576 & 576 & 276 & -624 & 576 & 576 & -624 & -4224 & 576 & 576 & 276 & -624 & 576 & 576 & 576 & 576 \\
576 & 576 & 576 & 576 & -624 & 276 & 576 & 576 & -4224 & -624 & 576 & 576 & -624 & 276 & 576 & 576 \\
576 & 576 & 576 & 576 & 276 & -624 & 276 & 576 & -624 & -4224 & -624 & 576 & 276 & -624 & 276 & 576 \\
576 & 576 & 576 & 576 & 576 & 276 & -624 & 276 & 576 & -624 & -4224 & -624 & 576 & 276 & -624 & 276 \\
576 & 576 & 576 & 576 & 576 & 576 & 276 & -624 & 576 & 576 & -624 & -4224 & 576 & 576 & 276 & -624 \\
576 & 576 & 576 & 576 & 576 & 576 & 576 & 576 & -624 & 276 & 576 & 576 & -4224 & -624 & 576 & 576 \\
576 & 576 & 576 & 576 & 576 & 576 & 576 & 576 & 276 & -624 & 276 & 576 & -624 & -4224 & -624 & 576 \\
576 & 576 & 576 & 576 & 576 & 576 & 576 & 576 & 576 & 276 & -624 & 276 & 576 & -624 & -4224 & -624 \\
576 & 576 & 576 & 576 & 576 & 576 & 576 & 576 & 576 & 576 & 276 & -624 & 576 & 576 & -624 & -4224
\end{pmatrix}$$

$S = \{1324, 2413, 3241, 4132\}, \lambda_{max} = 0.059466, \lambda_{min} = -0.158926$

$$H_S = \frac{1}{6 \cdot 5^6} \times \begin{pmatrix}
-3360 & -840 & 0 & 0 & 240 & -1290 & 3600 & 3600 & 1440 & 360 & 0 & 0 & 1440 & 360 & 0 & 0 \\
-840 & -3360 & -840 & 0 & 1410 & 240 & -2190 & 3600 & 360 & 1440 & 360 & 0 & 360 & 1440 & 360 & 0 \\
0 & -840 & -3360 & -840 & -3600 & 2310 & 240 & -1290 & 0 & 360 & 1440 & 360 & 0 & 360 & 1440 & 360 \\
0 & 0 & -840 & -3360 & -3600 & -3600 & 1410 & 240 & 0 & 0 & 360 & 1440 & 0 & 0 & 360 & 1440 \\
240 & 1410 & -3600 & -3600 & -3360 & -840 & 0 & 0 & 240 & -1290 & 3600 & 3600 & 1440 & 360 & 0 & 0 \\
-1290 & 240 & 2310 & -3600 & -840 & -3360 & -840 & 0 & 1410 & 240 & -2190 & 3600 & 360 & 1440 & 360 & 0 \\
3600 & -2190 & 240 & 1410 & 0 & -840 & -3360 & -840 & -3600 & 2310 & 240 & -1290 & 0 & 360 & 1440 & 360 \\
3600 & 3600 & -1290 & 240 & 0 & 0 & -840 & -3360 & -3600 & -3600 & 1410 & 240 & 0 & 0 & 360 & 1440 \\
1440 & 360 & 0 & 0 & 240 & 1410 & -3600 & -3600 & -3360 & -840 & 0 & 0 & 240 & -1290 & 3600 & 3600 \\
360 & 1440 & 360 & 0 & -1290 & 240 & 2310 & -3600 & -840 & -3360 & -840 & 0 & 1410 & 240 & -2190 & 3600 \\
0 & 360 & 1440 & 360 & 3600 & -2190 & 240 & 1410 & 0 & -840 & -3360 & -840 & -3600 & 2310 & 240 & -1290 \\
0 & 0 & 360 & 1440 & 3600 & 3600 & -1290 & 240 & 0 & 0 & -840 & -3360 & -3600 & -3600 & 1410 & 240 \\
1440 & 360 & 0 & 0 & 1440 & 360 & 0 & 0 & 240 & 1410 & -3600 & -3600 & -3360 & -840 & 0 & 0 \\
360 & 1440 & 360 & 0 & 360 & 1440 & 360 & 0 & -1290 & 240 & 2310 & -3600 & -840 & -3360 & -840 & 0 \\
0 & 360 & 1440 & 360 & 0 & 360 & 1440 & 360 & 3600 & -2190 & 240 & 1410 & 0 & -840 & -3360 & -840 \\
0 & 0 & 360 & 1440 & 0 & 0 & 360 & 1440 & 3600 & 3600 & -1290 & 240 & 0 & 0 & -840 & -3360
\end{pmatrix}$$

$S = \{1342, 2431, 3124, 4213\}, \lambda_{max} = 0.061073, \lambda_{min} = -0.083022$

$$H_S = \frac{1}{6 \cdot 5^6} \times \begin{pmatrix}
-2496 & 1104 & 2304 & 2304 & -1056 & -156 & 144 & 144 & -576 & -576 & -576 & -576 & -576 & -576 & -576 & -576 \\
1104 & -2496 & 1104 & 2304 & -156 & -1056 & -156 & 144 & -576 & -576 & -576 & -576 & -576 & -576 & -576 & -576 \\
2304 & 1104 & -2496 & 1104 & 144 & -156 & -1056 & -156 & -576 & -576 & -576 & -576 & -576 & -576 & -576 & -576 \\
2304 & 2304 & 1104 & -2496 & 144 & 144 & -156 & -1056 & -576 & -576 & -576 & -576 & -576 & -576 & -576 & -576 \\
-1056 & -156 & 144 & 144 & -2496 & 1104 & 2304 & 2304 & -1056 & -156 & 144 & 144 & -576 & -576 & -576 & -576 \\
-156 & -1056 & -156 & 144 & 1104 & -2496 & 1104 & 2304 & -156 & -1056 & -156 & 144 & -576 & -576 & -576 & -576 \\
144 & -156 & -1056 & -156 & 2304 & 1104 & -2496 & 1104 & 144 & -156 & -1056 & -156 & -576 & -576 & -576 & -576 \\
144 & 144 & -156 & -1056 & 2304 & 2304 & 1104 & -2496 & 144 & 144 & -156 & -1056 & -576 & -576 & -576 & -576 \\
-576 & -576 & -576 & -576 & -1056 & -156 & 144 & 144 & -2496 & 1104 & 2304 & 2304 & -1056 & -156 & 144 & 144 \\
-576 & -576 & -576 & -576 & -156 & -1056 & -156 & 144 & 1104 & -2496 & 1104 & 2304 & -156 & -1056 & -156 & 144 \\
-576 & -576 & -576 & -576 & 144 & -156 & -1056 & -156 & 2304 & 1104 & -2496 & 1104 & 144 & -156 & -1056 & -156 \\
-576 & -576 & -576 & -576 & 144 & 144 & -156 & -1056 & 2304 & 2304 & 1104 & -2496 & 144 & 144 & -156 & -1056 \\
-576 & -576 & -576 & -576 & -576 & -576 & -576 & -576 & -1056 & -156 & 144 & 144 & -2496 & 1104 & 2304 & 2304 \\
-576 & -576 & -576 & -576 & -576 & -576 & -576 & -576 & -156 & -1056 & -156 & 144 & 1104 & -2496 & 1104 & 2304 \\
-576 & -576 & -576 & -576 & -576 & -576 & -576 & -576 & 144 & -156 & -1056 & -156 & 2304 & 1104 & -2496 & 1104 \\
-576 & -576 & -576 & -576 & -576 & -576 & -576 & -576 & 144 & 144 & -156 & -1056 & 2304 & 2304 & 1104 & -2496
\end{pmatrix}$$

$S = \{1342, 2431, 3214, 4123\}, \lambda_{max} = 0.052419, \lambda_{min} = -0.041944$

$$H_S = \frac{1}{6 \cdot 5^6} \times \begin{pmatrix}
960 & 240 & 0 & 0 & -840 & -750 & 1440 & 1440 & -1440 & -360 & 0 & 0 & -1440 & -360 & 0 & 0 \\
240 & 960 & 240 & 0 & 330 & -840 & -1110 & 1440 & -360 & -1440 & -360 & 0 & -360 & -1440 & -360 & 0 \\
0 & 240 & 960 & 240 & -1440 & 690 & -840 & -750 & 0 & -360 & -1440 & -360 & 0 & -360 & -1440 & -360 \\
0 & 0 & 240 & 960 & -1440 & -1440 & 330 & -840 & 0 & 0 & -360 & -1440 & 0 & 0 & -360 & -1440 \\
-840 & 330 & -1440 & -1440 & 960 & 240 & 0 & 0 & -840 & -210 & 0 & 0 & -1440 & -360 & 0 & 0 \\
-750 & -840 & 690 & -1440 & 240 & 960 & 240 & 0 & -210 & -840 & -210 & 0 & -360 & -1440 & -360 & 0 \\
1440 & -1110 & -840 & 330 & 0 & 240 & 960 & 240 & 0 & -210 & -840 & -210 & 0 & -360 & -1440 & -360 \\
1440 & 1440 & -750 & -840 & 0 & 0 & 240 & 960 & 0 & 0 & -210 & -840 & 0 & 0 & -360 & -1440 \\
-1440 & -360 & 0 & 0 & -840 & -210 & 0 & 0 & 960 & 240 & 0 & 0 & -840 & 330 & -1440 & -1440 \\
-360 & -1440 & -360 & 0 & -210 & -840 & -210 & 0 & 240 & 960 & 240 & 0 & -750 & -840 & 690 & -1440 \\
0 & -360 & -1440 & -360 & 0 & -210 & -840 & -210 & 0 & 240 & 960 & 240 & 1440 & -1110 & -840 & 330 \\
0 & 0 & -360 & -1440 & 0 & 0 & -210 & -840 & 0 & 0 & 240 & 960 & 1440 & 1440 & -750 & -840 \\
-1440 & -360 & 0 & 0 & -1440 & -360 & 0 & 0 & -840 & -750 & 1440 & 1440 & 960 & 240 & 0 & 0 \\
-360 & -1440 & -360 & 0 & -360 & -1440 & -360 & 0 & 330 & -840 & -1110 & 1440 & 240 & 960 & 240 & 0 \\
0 & -360 & -1440 & -360 & 0 & -360 & -1440 & -360 & -1440 & 690 & -840 & -750 & 0 & 240 & 960 & 240 \\
0 & 0 & -360 & -1440 & 0 & 0 & -360 & -1440 & -1440 & -1440 & 330 & -840 & 0 & 0 & 240 & 960
\end{pmatrix}$$

$S = \{1432, 2341, 3214, 4123\}, \lambda_{max} = 0.136488, \lambda_{min} = -0.046180$

$$H_S = \frac{1}{6 \cdot 5^6} \times \begin{pmatrix}
4416 & -624 & -2304 & -2304 & -624 & -264 & -144 & -144 & -2304 & -144 & 576 & 576 & -2304 & -144 & 576 & 576 \\
-624 & 4416 & -624 & -2304 & -264 & -624 & -264 & -144 & -144 & -2304 & -144 & 576 & -144 & -2304 & -144 & 576 \\
-2304 & -624 & 4416 & -624 & -144 & -264 & -624 & -264 & 576 & -144 & -2304 & -144 & 576 & -144 & -2304 & -144 \\
-2304 & -2304 & -624 & 4416 & -144 & -144 & -264 & -624 & 576 & 576 & -144 & -2304 & 576 & 576 & -144 & -2304 \\
-624 & -264 & -144 & -144 & 4416 & -624 & -2304 & -2304 & -624 & -264 & -144 & -144 & -2304 & -144 & 576 & 576 \\
-264 & -624 & -264 & -144 & -624 & 4416 & -624 & -2304 & -264 & -624 & -264 & -144 & -144 & -2304 & -144 & 576 \\
-144 & -264 & -624 & -264 & -2304 & -624 & 4416 & -624 & -144 & -264 & -624 & -264 & 576 & -144 & -2304 & -144 \\
-144 & -144 & -264 & -624 & -2304 & -2304 & -624 & 4416 & -144 & -144 & -264 & -624 & 576 & 576 & -144 & -2304 \\
-2304 & -144 & 576 & 576 & -624 & -264 & -144 & -144 & 4416 & -624 & -2304 & -2304 & -624 & -264 & -144 & -144 \\
-144 & -2304 & -144 & 576 & -264 & -624 & -264 & -144 & -624 & 4416 & -624 & -2304 & -264 & -624 & -264 & -144 \\
576 & -144 & -2304 & -144 & -144 & -264 & -624 & -264 & -2304 & -624 & 4416 & -624 & -144 & -264 & -624 & -264 \\
576 & 576 & -144 & -2304 & -144 & -144 & -264 & -624 & -2304 & -2304 & -624 & 4416 & -144 & -144 & -264 & -624 \\
-2304 & -144 & 576 & 576 & -2304 & -144 & 576 & 576 & -624 & -264 & -144 & -144 & 4416 & -624 & -2304 & -2304 \\
-144 & -2304 & -144 & 576 & -144 & -2304 & -144 & 576 & -264 & -624 & -264 & -144 & -624 & 4416 & -624 & -2304 \\
576 & -144 & -2304 & -144 & 576 & -144 & -2304 & -144 & -144 & -264 & -624 & -264 & -2304 & -624 & 4416 & -624 \\
576 & 576 & -144 & -2304 & 576 & 576 & -144 & -2304 & -144 & -144 & -264 & -624 & -2304 & -2304 & -624 & 4416
\end{pmatrix}$$

# Appendix 3

$\mathbf{S = \{1234, 1243, 2134, 2143, 3412, 3421, 4312, 4321\}}, \lambda_{max} = 0.100999, \lambda_{min} = 0.018156$

$$H_S = \frac{1}{6 \cdot 5^6} \times \begin{pmatrix}
4800 & 1200 & 0 & 0 & 1200 & 300 & 0 & 0 & 0 & 0 & 0 & 0 & 0 & 0 & 0 & 0 \\
1200 & 4800 & 1200 & 0 & 300 & 1200 & 300 & 0 & 0 & 0 & 0 & 0 & 0 & 0 & 0 & 0 \\
0 & 1200 & 4800 & 1200 & 0 & 300 & 1200 & 300 & 0 & 0 & 0 & 0 & 0 & 0 & 0 & 0 \\
0 & 0 & 1200 & 4800 & 0 & 0 & 300 & 1200 & 0 & 0 & 0 & 0 & 0 & 0 & 0 & 0 \\
1200 & 300 & 0 & 0 & 4800 & 1200 & 0 & 0 & 1200 & 300 & 0 & 0 & 0 & 0 & 0 & 0 \\
300 & 1200 & 300 & 0 & 1200 & 4800 & 1200 & 0 & 300 & 1200 & 300 & 0 & 0 & 0 & 0 & 0 \\
0 & 300 & 1200 & 300 & 0 & 1200 & 4800 & 1200 & 0 & 300 & 1200 & 300 & 0 & 0 & 0 & 0 \\
0 & 0 & 300 & 1200 & 0 & 0 & 1200 & 4800 & 0 & 0 & 300 & 1200 & 0 & 0 & 0 & 0 \\
0 & 0 & 0 & 0 & 1200 & 300 & 0 & 0 & 4800 & 1200 & 0 & 0 & 1200 & 300 & 0 & 0 \\
0 & 0 & 0 & 0 & 300 & 1200 & 300 & 0 & 1200 & 4800 & 1200 & 0 & 300 & 1200 & 300 & 0 \\
0 & 0 & 0 & 0 & 0 & 300 & 1200 & 300 & 0 & 1200 & 4800 & 1200 & 0 & 300 & 1200 & 300 \\
0 & 0 & 0 & 0 & 0 & 0 & 300 & 1200 & 0 & 0 & 1200 & 4800 & 0 & 0 & 300 & 1200 \\
0 & 0 & 0 & 0 & 0 & 0 & 0 & 0 & 1200 & 300 & 0 & 0 & 4800 & 1200 & 0 & 0 \\
0 & 0 & 0 & 0 & 0 & 0 & 0 & 0 & 300 & 1200 & 300 & 0 & 1200 & 4800 & 1200 & 0 \\
0 & 0 & 0 & 0 & 0 & 0 & 0 & 0 & 0 & 300 & 1200 & 300 & 0 & 1200 & 4800 & 1200 \\
0 & 0 & 0 & 0 & 0 & 0 & 0 & 0 & 0 & 0 & 300 & 1200 & 0 & 0 & 1200 & 4800
\end{pmatrix}$$

$S = \{1234, 1243, 2134, 2341, 3412, 3421, 4123, 4312\}, \lambda_{max} = 0.366707, \lambda_{min} = -0.264382$

$$H_S = \frac{1}{6 \cdot 5^6} \times \begin{pmatrix}
4512 & 912 & -288 & -288 & 912 & 11262 & -288 & -288 & -288 & -288 & -288 & -288 & -288 & -288 & -288 & -288 \\
912 & 4512 & 912 & -288 & -11238 & 912 & 11262 & -288 & -288 & -288 & -288 & -288 & -288 & -288 & -288 & -288 \\
-288 & 912 & 4512 & 912 & -288 & -11238 & 912 & 11262 & -288 & -288 & -288 & -288 & -288 & -288 & -288 & -288 \\
-288 & -288 & 912 & 4512 & -288 & -288 & -11238 & 912 & -288 & -288 & -288 & -288 & -288 & -288 & -288 & -288 \\
912 & -11238 & -288 & -288 & 4512 & 912 & -288 & -288 & 912 & 11262 & -288 & -288 & -288 & -288 & -288 & -288 \\
11262 & 912 & -11238 & -288 & 912 & 4512 & 912 & -288 & -11238 & 912 & 11262 & -288 & -288 & -288 & -288 & -288 \\
-288 & 11262 & 912 & -11238 & -288 & 912 & 4512 & 912 & -288 & -11238 & 912 & 11262 & -288 & -288 & -288 & -288 \\
-288 & -288 & 11262 & 912 & -288 & -288 & 912 & 4512 & -288 & -288 & -11238 & 912 & -288 & -288 & -288 & -288 \\
-288 & -288 & -288 & -288 & 912 & -11238 & -288 & -288 & 4512 & 912 & -288 & -288 & 912 & 11262 & -288 & -288 \\
-288 & -288 & -288 & -288 & 11262 & 912 & -11238 & -288 & 912 & 4512 & 912 & -288 & -11238 & 912 & 11262 & -288 \\
-288 & -288 & -288 & -288 & -288 & 11262 & 912 & -11238 & -288 & 912 & 4512 & 912 & -288 & -11238 & 912 & 11262 \\
-288 & -288 & -288 & -288 & -288 & -288 & 11262 & 912 & -288 & -288 & 912 & 4512 & -288 & -288 & -11238 & 912 \\
-288 & -288 & -288 & -288 & -288 & -288 & -288 & -288 & 912 & -11238 & -288 & -288 & 4512 & 912 & -288 & -288 \\
-288 & -288 & -288 & -288 & -288 & -288 & -288 & -288 & 11262 & 912 & -11238 & -288 & 912 & 4512 & 912 & -288 \\
-288 & -288 & -288 & -288 & -288 & -288 & -288 & -288 & -288 & 11262 & 912 & -11238 & -288 & 912 & 4512 & 912 \\
-288 & -288 & -288 & -288 & -288 & -288 & -288 & -288 & -288 & -288 & 11262 & 912 & -288 & -288 & 912 & 4512
\end{pmatrix}$$

$S = \{1234, 1243, 2134, 2413, 3142, 3421, 4312, 4321\}, \lambda_{max} = 0.075338, \lambda_{min} = -0.044522$

$$H_S = \frac{1}{6 \cdot 5^6} \times \begin{pmatrix}
192 & 912 & 1152 & 1152 & 912 & 2082 & 72 & 72 & 1152 & 72 & -288 & -288 & 1152 & 72 & -288 & -288 \\
912 & 192 & 912 & 1152 & -1518 & 912 & 282 & 72 & 72 & 1152 & 72 & -288 & 72 & 1152 & 72 & -288 \\
1152 & 912 & 192 & 912 & 72 & 282 & 912 & -1518 & -288 & 72 & 1152 & 72 & -288 & 72 & 1152 & 72 \\
1152 & 1152 & 912 & 192 & 72 & 72 & 2082 & 912 & -288 & -288 & 72 & 1152 & -288 & -288 & 72 & 1152 \\
912 & -1518 & 72 & 72 & 192 & 912 & 1152 & 1152 & 912 & 282 & 72 & 72 & 1152 & 72 & -288 & -288 \\
2082 & 912 & 282 & 72 & 912 & 192 & 912 & 1152 & 282 & 912 & 282 & 72 & 72 & 1152 & 72 & -288 \\
72 & 282 & 912 & 2082 & 1152 & 912 & 192 & 912 & 72 & 282 & 912 & 282 & -288 & 72 & 1152 & 72 \\
72 & 72 & -1518 & 912 & 1152 & 1152 & 912 & 192 & 72 & 72 & 282 & 912 & -288 & -288 & 72 & 1152 \\
1152 & 72 & -288 & -288 & 912 & 282 & 72 & 72 & 192 & 912 & 1152 & 1152 & 912 & -1518 & 72 & 72 \\
72 & 1152 & 72 & -288 & 282 & 912 & 282 & 72 & 912 & 192 & 912 & 1152 & 2082 & 912 & 282 & 72 \\
-288 & 72 & 1152 & 72 & 72 & 282 & 912 & 282 & 1152 & 912 & 192 & 912 & 72 & 282 & 912 & 2082 \\
-288 & -288 & 72 & 1152 & 72 & 72 & 282 & 912 & 1152 & 1152 & 912 & 192 & 72 & 72 & -1518 & 912 \\
1152 & 72 & -288 & -288 & 1152 & 72 & -288 & -288 & 912 & 2082 & 72 & 72 & 192 & 912 & 1152 & 1152 \\
72 & 1152 & 72 & -288 & 72 & 1152 & 72 & -288 & -1518 & 912 & 282 & 72 & 912 & 192 & 912 & 1152 \\
-288 & 72 & 1152 & 72 & -288 & 72 & 1152 & 72 & 72 & 282 & 912 & -1518 & 1152 & 912 & 192 & 912 \\
-288 & -288 & 72 & 1152 & -288 & -288 & 72 & 1152 & 72 & 72 & 2082 & 912 & 1152 & 1152 & 912 & 192
\end{pmatrix}$$

$S = \{1234, 1243, 2143, 2314, 3412, 3421, 4132, 4321\}, \lambda_{max} = 0.138691, \lambda_{min} = -0.036540$

$$H_S = \frac{1}{6 \cdot 5^6} \times \begin{pmatrix}
3648 & 48 & -1152 & -1152 & 1128 & 4728 & -72 & -72 & 288 & 288 & 288 & 288 & 288 & 288 & 288 & 288 \\
48 & 3648 & 48 & -1152 & -4272 & 1128 & 4728 & -72 & 288 & 288 & 288 & 288 & 288 & 288 & 288 & 288 \\
-1152 & 48 & 3648 & 48 & -72 & -4272 & 1128 & 4728 & 288 & 288 & 288 & 288 & 288 & 288 & 288 & 288 \\
-1152 & -1152 & 48 & 3648 & -72 & -72 & -4272 & 1128 & 288 & 288 & 288 & 288 & 288 & 288 & 288 & 288 \\
1128 & -4272 & -72 & -72 & 3648 & 48 & -1152 & -1152 & 1128 & 228 & -72 & -72 & 288 & 288 & 288 & 288 \\
4728 & 1128 & -4272 & -72 & 48 & 3648 & 48 & -1152 & 228 & 1128 & 228 & -72 & 288 & 288 & 288 & 288 \\
-72 & 4728 & 1128 & -4272 & -1152 & 48 & 3648 & 48 & -72 & 228 & 1128 & 228 & 288 & 288 & 288 & 288 \\
-72 & -72 & 4728 & 1128 & -1152 & -1152 & 48 & 3648 & -72 & -72 & 228 & 1128 & 288 & 288 & 288 & 288 \\
288 & 288 & 288 & 288 & 1128 & 228 & -72 & -72 & 3648 & 48 & -1152 & -1152 & 1128 & -4272 & -72 & -72 \\
288 & 288 & 288 & 288 & 228 & 1128 & 228 & -72 & 48 & 3648 & 48 & -1152 & 4728 & 1128 & -4272 & -72 \\
288 & 288 & 288 & 288 & -72 & 228 & 1128 & 228 & -1152 & 48 & 3648 & 48 & -72 & 4728 & 1128 & -4272 \\
288 & 288 & 288 & 288 & -72 & -72 & 228 & 1128 & -1152 & -1152 & 48 & 3648 & -72 & -72 & 4728 & 1128 \\
288 & 288 & 288 & 288 & 288 & 288 & 288 & 288 & 1128 & 4728 & -72 & -72 & 3648 & 48 & -1152 & -1152 \\
288 & 288 & 288 & 288 & 288 & 288 & 288 & 288 & -4272 & 1128 & 4728 & -72 & 48 & 3648 & 48 & -1152 \\
288 & 288 & 288 & 288 & 288 & 288 & 288 & 288 & -72 & -4272 & 1128 & 4728 & -1152 & 48 & 3648 & 48 \\
288 & 288 & 288 & 288 & 288 & 288 & 288 & 288 & -72 & -72 & -4272 & 1128 & -1152 & -1152 & 48 & 3648
\end{pmatrix}$$

$S = \{1234, 1243, 2314, 2341, 3412, 3421, 4123, 4132\}, \lambda_{max} = 0.392111, \lambda_{min} = -0.292806$

$$H_S = \frac{1}{6\cdot 5^6} \times \begin{pmatrix}
3360 & -240 & -1440 & -1440 & 840 & 15690 & -360 & -360 & 0 & 0 & 0 & 0 & 0 & 0 & 0 & 0 \\
-240 & 3360 & -240 & -1440 & -15810 & 840 & 15690 & -360 & 0 & 0 & 0 & 0 & 0 & 0 & 0 & 0 \\
-1440 & -240 & 3360 & -240 & -360 & -15810 & 840 & 15690 & 0 & 0 & 0 & 0 & 0 & 0 & 0 & 0 \\
-1440 & -1440 & -240 & 3360 & -360 & -360 & -15810 & 840 & 0 & 0 & 0 & 0 & 0 & 0 & 0 & 0 \\
840 & -15810 & -360 & -360 & 3360 & -240 & -1440 & -1440 & 840 & 11190 & -360 & -360 & 0 & 0 & 0 & 0 \\
15690 & 840 & -15810 & -360 & -240 & 3360 & -240 & -1440 & -11310 & 840 & 11190 & -360 & 0 & 0 & 0 & 0 \\
-360 & 15690 & 840 & -15810 & -1440 & -240 & 3360 & -240 & -360 & -11310 & 840 & 11190 & 0 & 0 & 0 & 0 \\
-360 & -360 & 15690 & 840 & -1440 & -1440 & -240 & 3360 & -360 & -360 & -11310 & 840 & 0 & 0 & 0 & 0 \\
0 & 0 & 0 & 0 & 840 & -11310 & -360 & -360 & 3360 & -240 & -1440 & -1440 & 840 & 6690 & -360 & -360 \\
0 & 0 & 0 & 0 & 11190 & 840 & -11310 & -360 & -240 & 3360 & -240 & -1440 & -6810 & 840 & 6690 & -360 \\
0 & 0 & 0 & 0 & -360 & 11190 & 840 & -11310 & -1440 & -240 & 3360 & -240 & -360 & -6810 & 840 & 6690 \\
0 & 0 & 0 & 0 & -360 & -360 & 11190 & 840 & -1440 & -1440 & -240 & 3360 & -360 & -360 & -6810 & 840 \\
0 & 0 & 0 & 0 & 0 & 0 & 0 & 0 & 840 & -6810 & -360 & -360 & 3360 & -240 & -1440 & -1440 \\
0 & 0 & 0 & 0 & 0 & 0 & 0 & 0 & 6690 & 840 & -6810 & -360 & -240 & 3360 & -240 & -1440 \\
0 & 0 & 0 & 0 & 0 & 0 & 0 & 0 & -360 & 6690 & 840 & -6810 & -1440 & -240 & 3360 & -240 \\
0 & 0 & 0 & 0 & 0 & 0 & 0 & 0 & -360 & -360 & 6690 & 840 & -1440 & -1440 & -240 & 3360
\end{pmatrix}$$

$S = \{1234, 1243, 2314, 2413, 3142, 3421, 4132, 4321\}, \lambda_{max} = 0.091988, \lambda_{min} = -0.108256$

$$H_S = \frac{1}{6\cdot 5^6} \times \begin{pmatrix}
-960 & -240 & 0 & 0 & 840 & 6510 & 0 & 0 & 1440 & 360 & 0 & 0 & 1440 & 360 & 0 & 0 \\
-240 & -960 & -240 & 0 & -6090 & 840 & 4710 & 0 & 360 & 1440 & 360 & 0 & 360 & 1440 & 360 & 0 \\
0 & -240 & -960 & -240 & 0 & -4290 & 840 & 2910 & 0 & 360 & 1440 & 360 & 0 & 360 & 1440 & 360 \\
0 & 0 & -240 & -960 & 0 & 0 & -2490 & 840 & 0 & 0 & 360 & 1440 & 0 & 0 & 360 & 1440 \\
840 & -6090 & 0 & 0 & -960 & -240 & 0 & 0 & 840 & 210 & 0 & 0 & 1440 & 360 & 0 & 0 \\
6510 & 840 & -4290 & 0 & -240 & -960 & -240 & 0 & 210 & 840 & 210 & 0 & 360 & 1440 & 360 & 0 \\
0 & 4710 & 840 & -2490 & 0 & -240 & -960 & -240 & 0 & 210 & 840 & 210 & 0 & 360 & 1440 & 360 \\
0 & 0 & 2910 & 840 & 0 & 0 & -240 & -960 & 0 & 0 & 210 & 840 & 0 & 0 & 360 & 1440 \\
1440 & 360 & 0 & 0 & 840 & 210 & 0 & 0 & -960 & -240 & 0 & 0 & 840 & -6090 & 0 & 0 \\
360 & 1440 & 360 & 0 & 210 & 840 & 210 & 0 & -240 & -960 & -240 & 0 & 6510 & 840 & -4290 & 0 \\
0 & 360 & 1440 & 360 & 0 & 210 & 840 & 210 & 0 & -240 & -960 & -240 & 0 & 4710 & 840 & -2490 \\
0 & 0 & 360 & 1440 & 0 & 0 & 210 & 840 & 0 & 0 & -240 & -960 & 0 & 0 & 2910 & 840 \\
1440 & 360 & 0 & 0 & 1440 & 360 & 0 & 0 & 840 & 6510 & 0 & 0 & -960 & -240 & 0 & 0 \\
360 & 1440 & 360 & 0 & 360 & 1440 & 360 & 0 & -6090 & 840 & 4710 & 0 & -240 & -960 & -240 & 0 \\
0 & 360 & 1440 & 360 & 0 & 360 & 1440 & 360 & 0 & -4290 & 840 & 2910 & 0 & -240 & -960 & -240 \\
0 & 0 & 360 & 1440 & 0 & 0 & 360 & 1440 & 0 & 0 & -2490 & 840 & 0 & 0 & -240 & -960
\end{pmatrix}$$

$S = \{1234, 1243, 2314, 2431, 3142, 3412, 4123, 4321\}, \lambda_{max} = 0.240174, \lambda_{min} = -0.153941$

$$H_S = \frac{1}{6\cdot 5^6} \times \begin{pmatrix}
2496 & -24 & -864 & -864 & -24 & 11100 & -648 & -648 & -864 & 1512 & 0 & 0 & -864 & 1512 & 0 & 0 \\
-24 & 2496 & -24 & -864 & -10788 & -24 & 7896 & -648 & -1080 & -864 & 2376 & 0 & -1080 & -864 & 2376 & 0 \\
-864 & -24 & 2496 & -24 & 1080 & -7584 & -24 & 4260 & 1152 & -1944 & -864 & 2952 & 1152 & -1944 & -864 & 2952 \\
-864 & -864 & -24 & 2496 & 1080 & 1080 & -3948 & -24 & 1152 & 1152 & -2520 & -864 & 1152 & 1152 & -2520 & -864 \\
-24 & -10788 & 1080 & 1080 & 2496 & -24 & -864 & -864 & -24 & 7896 & -1224 & -1224 & -864 & 1512 & 0 & 0 \\
11100 & -24 & -7584 & 1080 & -24 & 2496 & -24 & -864 & -7584 & -24 & 5556 & -1224 & -1080 & -864 & 2376 & 0 \\
-648 & 7896 & -24 & -3948 & -864 & -24 & 2496 & -24 & 1656 & -5244 & -24 & 2496 & 1152 & -1944 & -864 & 2952 \\
-648 & -648 & 4260 & -24 & -864 & -864 & -24 & 2496 & 1656 & 1656 & -2184 & -24 & 1152 & 1152 & -2520 & -864 \\
-864 & -1080 & 1152 & 1152 & -24 & -7584 & 1656 & 1656 & 2496 & -24 & -864 & -864 & -24 & 5340 & -2088 & -2088 \\
1512 & -864 & -1944 & 1152 & 7896 & -24 & -5244 & 1656 & -24 & 2496 & -24 & -864 & -5028 & -24 & 4296 & -2088 \\
0 & 2376 & -864 & -2520 & -1224 & 5556 & -24 & -2184 & -864 & -24 & 2496 & -24 & 2520 & -3984 & -24 & 2100 \\
0 & 0 & 2952 & -864 & -1224 & -1224 & 2496 & -24 & -864 & -864 & -24 & 2496 & 2520 & 2520 & -1788 & -24 \\
-864 & -1080 & 1152 & 1152 & -864 & -1080 & 1152 & 1152 & -24 & -5028 & 2520 & 2520 & 2496 & -24 & -864 & -864 \\
1512 & -864 & -1944 & 1152 & 1512 & -864 & -1944 & 1152 & 5340 & -24 & -3984 & 2520 & -24 & 2496 & -24 & -864 \\
0 & 2376 & -864 & -2520 & 0 & 2376 & -864 & -2520 & -2088 & 4296 & -24 & -1788 & -864 & -24 & 2496 & -24 \\
0 & 0 & 2952 & -864 & 0 & 0 & 2952 & -864 & -2088 & -2088 & 2100 & -24 & -864 & -864 & -24 & 2496
\end{pmatrix}$$

$S = \{1234, 1243, 2314, 2431, 3142, 3421, 4123, 4312\}, \lambda_{max} = 0.187928, \lambda_{min} = -0.217836$

$$H_S = \frac{1}{6\cdot 5^6} \times \begin{pmatrix}
-96 & 624 & 864 & 864 & 624 & 11100 & -1512 & -1512 & 864 & 648 & 0 & 0 & 864 & 648 & 0 & 0 \\
624 & -96 & 624 & 864 & -11112 & 624 & 8004 & -1512 & -1080 & 864 & 1224 & 0 & -1080 & 864 & 1224 & 0 \\
864 & 624 & -96 & 624 & 1080 & -8016 & 624 & 4260 & -1152 & -1656 & 864 & 2088 & -1152 & -1656 & 864 & 2088 \\
864 & 864 & 624 & -96 & 1080 & 1080 & -4272 & 624 & -1152 & -1152 & -2520 & 864 & -1152 & -1152 & -2520 & 864 \\
624 & -11112 & 1080 & 1080 & -96 & 624 & 864 & 864 & 624 & 8004 & -2376 & -2376 & 864 & 648 & 0 & 0 \\
11100 & 624 & -8016 & 1080 & 624 & -96 & 624 & 864 & -8016 & 624 & 5844 & -2376 & -1080 & 864 & 1224 & 0 \\
-1512 & 8004 & 624 & -4272 & 864 & 624 & -96 & 624 & 1944 & -5856 & 624 & 2604 & -1152 & -1656 & 864 & 2088 \\
-1512 & -1512 & 4260 & 624 & 864 & 864 & 624 & -96 & 1944 & 1944 & -2616 & 624 & -1152 & -1152 & -2520 & 864 \\
864 & -1080 & -1152 & -1152 & 624 & -8016 & 1944 & 1944 & -96 & 624 & 864 & 864 & 624 & 5340 & -2952 & -2952 \\
648 & 864 & -1656 & -1152 & 8004 & 624 & -5856 & 1944 & 624 & -96 & 624 & 864 & -5352 & 624 & 4404 & -2952 \\
0 & 1224 & 864 & -2520 & -2376 & 5844 & 624 & -2616 & 864 & 624 & -96 & 624 & 2520 & -4416 & 624 & 2100 \\
0 & 0 & 2088 & 864 & -2376 & -2376 & 2604 & 624 & 864 & 864 & 624 & -96 & 2520 & 2520 & -2112 & 624 \\
864 & -1080 & -1152 & -1152 & 864 & -1080 & -1152 & -1152 & 624 & -5352 & 2520 & 2520 & -96 & 624 & 864 & 864 \\
648 & 864 & -1656 & -1152 & 648 & 864 & -1656 & -1152 & 5340 & 624 & -4416 & 2520 & 624 & -96 & 624 & 864 \\
0 & 1224 & 864 & -2520 & 0 & 1224 & 864 & -2520 & -2952 & 4404 & 624 & -2112 & 864 & 624 & -96 & 624 \\
0 & 0 & 2088 & 864 & 0 & 0 & 2088 & 864 & -2952 & -2952 & 2100 & 624 & 864 & 864 & 624 & -96
\end{pmatrix}$$

$S = \{1234, 1324, 2143, 2341, 3412, 3421, 4132, 4213\}, \lambda_{max} = 0.207575, \lambda_{min} = -0.124072$

$$H_S = \frac{1}{6 \cdot 5^6} \times \begin{pmatrix}
2496 & -24 & -864 & -864 & -24 & 3612 & 1080 & 1080 & -864 & 2520 & 1152 & 1152 & -864 & 2520 & 1152 & 1152 \\
-24 & 2496 & -24 & -864 & -3300 & -24 & 6816 & 1080 & -2088 & -864 & 1656 & 1152 & -2088 & -864 & 1656 & 1152 \\
-864 & -24 & 2496 & -24 & -648 & -6504 & -24 & 10452 & 0 & -1224 & -864 & 1080 & 0 & -1224 & -864 & 1080 \\
-864 & -864 & -24 & 2496 & -648 & -648 & -10140 & -24 & 0 & 0 & -648 & -864 & 0 & 0 & -648 & -864 \\
-24 & -3300 & -648 & -648 & 2496 & -24 & -864 & -864 & -24 & 1416 & 1656 & 1656 & -864 & 2520 & 1152 & 1152 \\
3612 & -24 & -6504 & -648 & -24 & 2496 & -24 & -864 & -1104 & -24 & 3756 & 1656 & -2088 & -864 & 1656 & 1152 \\
1080 & 6816 & -24 & -10140 & -864 & -24 & 2496 & -24 & -1224 & -3444 & -24 & 6816 & 0 & -1224 & -864 & 1080 \\
1080 & 1080 & 10452 & -24 & -864 & -864 & -24 & 2496 & -1224 & -1224 & -6504 & -24 & 0 & 0 & -648 & -864 \\
-864 & -2088 & 0 & 0 & -24 & -1104 & -1224 & -1224 & 2496 & -24 & -864 & -864 & -24 & 372 & 2520 & 2520 \\
2520 & -864 & -1224 & 0 & 1416 & -24 & -3444 & -1224 & -24 & 2496 & -24 & -864 & -60 & -24 & 1416 & 2520 \\
1152 & 1656 & -864 & -648 & 1656 & 3756 & -24 & -6504 & -864 & -24 & 2496 & -24 & -2088 & -1104 & -24 & 3612 \\
1152 & 1152 & 1080 & -864 & 1656 & 1656 & 6816 & -24 & -864 & -864 & -24 & 2496 & -2088 & -2088 & -3300 & -24 \\
-864 & -2088 & 0 & 0 & -864 & -2088 & 0 & 0 & -24 & -60 & -2088 & -2088 & 2496 & -24 & -864 & -864 \\
2520 & -864 & -1224 & 0 & 2520 & -864 & -1224 & 0 & 372 & -24 & -1104 & -2088 & -24 & 2496 & -24 & -864 \\
1152 & 1656 & -864 & -648 & 1152 & 1656 & -864 & -648 & 2520 & 1416 & -24 & -3300 & -864 & -24 & 2496 & -24 \\
1152 & 1152 & 1080 & -864 & 1152 & 1152 & 1080 & -864 & 2520 & 2520 & 3612 & -24 & -864 & -864 & -24 & 2496
\end{pmatrix}$$

$S = \{1234, 1324, 2143, 2413, 3142, 3412, 4231, 4321\}, \lambda_{max} = 0.068244, \lambda_{min} = -0.061073$

$$H_S = \frac{1}{6 \cdot 5^6} \times \begin{pmatrix}
768 & -672 & -1152 & -1152 & -672 & 588 & 1008 & 1008 & -1152 & 1008 & 1728 & 1728 & -1152 & 1008 & 1728 & 1728 \\
-672 & 768 & -672 & -1152 & 588 & -672 & 588 & 1008 & 1008 & -1152 & 1008 & 1728 & 1008 & -1152 & 1008 & 1728 \\
-1152 & -672 & 768 & -672 & 1008 & 588 & -672 & 588 & 1728 & 1008 & -1152 & 1008 & 1728 & 1008 & -1152 & 1008 \\
-1152 & -1152 & -672 & 768 & 1008 & 1008 & 588 & -672 & 1728 & 1728 & 1008 & -1152 & 1728 & 1728 & 1008 & -1152 \\
-672 & 588 & 1008 & 1008 & 768 & -672 & -1152 & -1152 & -672 & 588 & 1008 & 1008 & -1152 & 1008 & 1728 & 1728 \\
588 & -672 & 588 & 1008 & -672 & 768 & -672 & -1152 & 588 & -672 & 588 & 1008 & 1008 & -1152 & 1008 & 1728 \\
1008 & 588 & -672 & 588 & -1152 & -672 & 768 & -672 & 1008 & 588 & -672 & 588 & 1728 & 1008 & -1152 & 1008 \\
1008 & 1008 & 588 & -672 & -1152 & -1152 & -672 & 768 & 1008 & 1008 & 588 & -672 & 1728 & 1728 & 1008 & -1152 \\
-1152 & 1008 & 1728 & 1728 & -672 & 588 & 1008 & 1008 & 768 & -672 & -1152 & -1152 & -672 & 588 & 1008 & 1008 \\
1008 & -1152 & 1008 & 1728 & 588 & -672 & 588 & 1008 & -672 & 768 & -672 & -1152 & 588 & -672 & 588 & 1008 \\
1728 & 1008 & -1152 & 1008 & 1008 & 588 & -672 & 588 & -1152 & -672 & 768 & -672 & 1008 & 588 & -672 & 588 \\
1728 & 1728 & 1008 & -1152 & 1008 & 1008 & 588 & -672 & -1152 & -1152 & -672 & 768 & 1008 & 1008 & 588 & -672 \\
-1152 & 1008 & 1728 & 1728 & -1152 & 1008 & 1728 & 1728 & -672 & 588 & 1008 & 1008 & 768 & -672 & -1152 & -1152 \\
1008 & -1152 & 1008 & 1728 & 1008 & -1152 & 1008 & 1728 & 588 & -672 & 588 & 1008 & -672 & 768 & -672 & -1152 \\
1728 & 1008 & -1152 & 1008 & 1728 & 1008 & -1152 & 1008 & 1008 & 588 & -672 & 588 & -1152 & -672 & 768 & -672 \\
1728 & 1728 & 1008 & -1152 & 1728 & 1728 & 1008 & -1152 & 1008 & 1008 & 588 & -672 & -1152 & -1152 & -672 & 768
\end{pmatrix}$$

$S = \{1234, 1324, 2143, 2413, 3142, 3421, 4231, 4312\}, \lambda_{max} = 0.055646, \lambda_{min} = -0.065486$

$$H_S = \frac{1}{6 \cdot 5^6} \times \begin{pmatrix}
-1824 & -24 & 576 & 576 & -24 & 588 & 144 & 144 & 576 & 144 & 1728 & 1728 & 576 & 144 & 1728 & 1728 \\
-24 & -1824 & -24 & 576 & 264 & -24 & 696 & 144 & 1008 & 576 & -144 & 1728 & 1008 & 576 & -144 & 1728 \\
576 & -24 & -1824 & -24 & 1008 & 156 & -24 & 588 & -576 & 1296 & 576 & 144 & -576 & 1296 & 576 & 144 \\
576 & 576 & -24 & -1824 & 1008 & 1008 & 264 & -24 & -576 & -576 & 1008 & 576 & -576 & -576 & 1008 & 576 \\
-24 & 264 & 1008 & 1008 & -1824 & -24 & 576 & 576 & -24 & 696 & -144 & -144 & 576 & 144 & 1728 & 1728 \\
588 & -24 & 156 & 1008 & -24 & -1824 & -24 & 576 & 156 & -24 & 876 & -144 & 1008 & 576 & -144 & 1728 \\
144 & 696 & -24 & 264 & 576 & -24 & -1824 & -24 & 1296 & -24 & -24 & 696 & -576 & 1296 & 576 & 144 \\
144 & 144 & 588 & -24 & 576 & 576 & -24 & -1824 & 1296 & 1296 & 156 & -24 & -576 & -576 & 1008 & 576 \\
576 & 1008 & -576 & -576 & -24 & 156 & 1296 & 1296 & -1824 & -24 & 576 & 576 & -24 & 588 & 144 & 144 \\
144 & 576 & 1296 & -576 & 696 & -24 & -24 & 1296 & -24 & -1824 & -24 & 576 & 264 & -24 & 696 & 144 \\
1728 & -144 & 576 & 1008 & -144 & 876 & -24 & 156 & 576 & -24 & -1824 & -24 & 1008 & 156 & -24 & 588 \\
1728 & 1728 & 144 & 576 & -144 & -144 & 696 & -24 & 576 & 576 & -24 & -1824 & 1008 & 1008 & 264 & -24 \\
576 & 1008 & -576 & -576 & 576 & 1008 & -576 & -576 & -24 & 264 & 1008 & 1008 & -1824 & -24 & 576 & 576 \\
144 & 576 & 1296 & -576 & 144 & 576 & 1296 & -576 & 588 & -24 & 156 & 1008 & -24 & -1824 & -24 & 576 \\
1728 & -144 & 576 & 1008 & 1728 & -144 & 576 & 1008 & 144 & 696 & -24 & 264 & 576 & -24 & -1824 & -24 \\
1728 & 1728 & 144 & 576 & 1728 & 1728 & 144 & 576 & 144 & 144 & 588 & -24 & 576 & 576 & -24 & -1824
\end{pmatrix}$$

$S = \{1234, 1324, 2143, 2413, 3241, 3412, 4132, 4321\}, \lambda_{max} = 0.144306, \lambda_{min} = -0.106412$

$$H_S = \frac{1}{6 \cdot 5^6} \times \begin{pmatrix}
1632 & -888 & -1728 & -1728 & 192 & -978 & 4032 & 4032 & -288 & 792 & 1152 & 1152 & -288 & 792 & 1152 & 1152 \\
-888 & 1632 & -888 & -1728 & 1722 & 192 & -1878 & 4032 & 792 & -288 & 792 & 1152 & 792 & -288 & 792 & 1152 \\
-1728 & -888 & 1632 & -888 & -3168 & 2622 & 192 & -978 & 1152 & 792 & -288 & 792 & 1152 & 792 & -288 & 792 \\
-1728 & -1728 & -888 & 1632 & -3168 & -3168 & 1722 & 192 & 1152 & 1152 & 792 & -288 & 1152 & 1152 & 792 & -288 \\
192 & 1722 & -3168 & -3168 & 1632 & -888 & -1728 & -1728 & 192 & -978 & 4032 & 4032 & -288 & 792 & 1152 & 1152 \\
-978 & 192 & 2622 & -3168 & -888 & 1632 & -888 & -1728 & 1722 & 192 & -1878 & 4032 & 792 & -288 & 792 & 1152 \\
4032 & -1878 & 192 & 1722 & -1728 & -888 & 1632 & -888 & -3168 & 2622 & 192 & -978 & 1152 & 792 & -288 & 792 \\
4032 & 4032 & -978 & 192 & -1728 & -1728 & -888 & 1632 & -3168 & -3168 & 1722 & 192 & 1152 & 1152 & 792 & -288 \\
-288 & 792 & 1152 & 1152 & 192 & 1722 & -3168 & -3168 & 1632 & -888 & -1728 & -1728 & 192 & -978 & 4032 & 4032 \\
792 & -288 & 792 & 1152 & -978 & 192 & 2622 & -3168 & -888 & 1632 & -888 & -1728 & 1722 & 192 & -1878 & 4032 \\
1152 & 792 & -288 & 792 & 4032 & -1878 & 192 & 1722 & -1728 & -888 & 1632 & -888 & -3168 & 2622 & 192 & -978 \\
1152 & 1152 & 792 & -288 & 4032 & 4032 & -978 & 192 & -1728 & -1728 & -888 & 1632 & -3168 & -3168 & 1722 & 192 \\
-288 & 792 & 1152 & 1152 & -288 & 792 & 1152 & 1152 & 192 & 1722 & -3168 & -3168 & 1632 & -888 & -1728 & -1728 \\
792 & -288 & 792 & 1152 & 792 & -288 & 792 & 1152 & -978 & 192 & 2622 & -3168 & -888 & 1632 & -888 & -1728 \\
1152 & 792 & -288 & 792 & 1152 & 792 & -288 & 792 & 4032 & -1878 & 192 & 1722 & -1728 & -888 & 1632 & -888 \\
1152 & 1152 & 792 & -288 & 1152 & 1152 & 792 & -288 & 4032 & 4032 & -978 & 192 & -1728 & -1728 & -888 & 1632
\end{pmatrix}$$

$S = \{1234, 1324, 2143, 2413, 3241, 3421, 4132, 4312\}, \lambda_{max} = 0.086086, \lambda_{min} = -0.115344$

$$H_S = \frac{1}{6 \cdot 5^6} \times \begin{pmatrix}
-960 & -240 & 0 & 0 & 840 & -978 & 3168 & 3168 & 1440 & -72 & 1152 & 1152 & 1440 & -72 & 1152 & 1152 \\
-240 & -960 & -240 & 0 & 1398 & 840 & -1770 & 3168 & 792 & 1440 & -360 & 1152 & 792 & 1440 & -360 & 1152 \\
0 & -240 & -960 & -240 & -3168 & 2190 & 840 & -978 & -1152 & 1080 & 1440 & -72 & -1152 & 1080 & 1440 & -72 \\
0 & 0 & -240 & -960 & -3168 & -3168 & 1398 & 840 & -1152 & -1152 & 792 & 1440 & -1152 & -1152 & 792 & 1440 \\
840 & 1398 & -3168 & -3168 & -960 & -240 & 0 & 0 & 840 & -870 & 2880 & 2880 & 1440 & -72 & 1152 & 1152 \\
-978 & 840 & 2190 & -3168 & -240 & -960 & -240 & 0 & 1290 & 840 & -1590 & 2880 & 792 & 1440 & -360 & 1152 \\
3168 & -1770 & 840 & 1398 & 0 & -240 & -960 & -240 & -2880 & 2010 & 840 & -870 & -1152 & 1080 & 1440 & -72 \\
3168 & 3168 & -978 & 840 & 0 & 0 & -240 & -960 & -2880 & -2880 & 1290 & 840 & -1152 & -1152 & 792 & 1440 \\
1440 & 792 & -1152 & -1152 & 840 & 1290 & -2880 & -2880 & -960 & -240 & 0 & 0 & 840 & -978 & 3168 & 3168 \\
-72 & 1440 & 1080 & -1152 & -870 & 840 & 2010 & -2880 & -240 & -960 & -240 & 0 & 1398 & 840 & -1770 & 3168 \\
1152 & -360 & 1440 & 792 & 2880 & -1590 & 840 & 1290 & 0 & -240 & -960 & -240 & -3168 & 2190 & 840 & -978 \\
1152 & 1152 & -72 & 1440 & 2880 & 2880 & -870 & 840 & 0 & 0 & -240 & -960 & -3168 & -3168 & 1398 & 840 \\
1440 & 792 & -1152 & -1152 & 1440 & 792 & -1152 & -1152 & 840 & 1398 & -3168 & -3168 & -960 & -240 & 0 & 0 \\
-72 & 1440 & 1080 & -1152 & -72 & 1440 & 1080 & -1152 & -978 & 840 & 2190 & -3168 & -240 & -960 & -240 & 0 \\
1152 & -360 & 1440 & 792 & 1152 & -360 & 1440 & 792 & 3168 & -1770 & 840 & 1398 & 0 & -240 & -960 & -240 \\
1152 & 1152 & -72 & 1440 & 1152 & 1152 & -72 & 1440 & 3168 & 3168 & -978 & 840 & 0 & 0 & -240 & -960
\end{pmatrix}$$

$S = \{1234, 1324, 2341, 2413, 3142, 3412, 4123, 4231\}, \lambda_{max} = 0.360474, \lambda_{min} = -0.271202$

$$H_S = \frac{1}{6 \cdot 5^6} \times \begin{pmatrix}
480 & -960 & -1440 & -1440 & -960 & 11550 & 720 & 720 & -1440 & 720 & 1440 & 1440 & -1440 & 720 & 1440 & 1440 \\
-960 & 480 & -960 & -1440 & -10950 & -960 & 11550 & 720 & 720 & -1440 & 720 & 1440 & 720 & -1440 & 720 & 1440 \\
-1440 & -960 & 480 & -960 & 720 & -10950 & -960 & 11550 & 1440 & 720 & -1440 & 720 & 1440 & 720 & -1440 & 720 \\
-1440 & -1440 & -960 & 480 & 720 & 720 & -10950 & -960 & 1440 & 1440 & 720 & -1440 & 1440 & 1440 & 720 & -1440 \\
-960 & -10950 & 720 & 720 & 480 & -960 & -1440 & -1440 & -960 & 11550 & 720 & 720 & -1440 & 720 & 1440 & 1440 \\
11550 & -960 & -10950 & 720 & -960 & 480 & -960 & -1440 & -10950 & -960 & 11550 & 720 & 720 & -1440 & 720 & 1440 \\
720 & 11550 & -960 & -10950 & -1440 & -960 & 480 & -960 & 720 & -10950 & -960 & 11550 & 1440 & 720 & -1440 & 720 \\
720 & 720 & 11550 & -960 & -1440 & -1440 & -960 & 480 & 720 & 720 & -10950 & -960 & 1440 & 1440 & 720 & -1440 \\
-1440 & 720 & 1440 & 1440 & -960 & -10950 & 720 & 720 & 480 & -960 & -1440 & -1440 & -960 & 11550 & 720 & 720 \\
720 & -1440 & 720 & 1440 & 11550 & -960 & -10950 & 720 & -960 & 480 & -960 & -1440 & -10950 & -960 & 11550 & 720 \\
1440 & 720 & -1440 & 720 & 720 & 11550 & -960 & -10950 & -1440 & -960 & 480 & -960 & 720 & -10950 & -960 & 11550 \\
1440 & 1440 & 720 & -1440 & 720 & 720 & 11550 & -960 & -1440 & -1440 & -960 & 480 & 720 & 720 & -10950 & -960 \\
-1440 & 720 & 1440 & 1440 & -1440 & 720 & 1440 & 1440 & -960 & -10950 & 720 & 720 & 480 & -960 & -1440 & -1440 \\
720 & -1440 & 720 & 1440 & 720 & -1440 & 720 & 1440 & 11550 & -960 & -10950 & 720 & -960 & 480 & -960 & -1440 \\
1440 & 720 & -1440 & 720 & 1440 & 720 & -1440 & 720 & 720 & 11550 & -960 & -10950 & -1440 & -960 & 480 & -960 \\
1440 & 1440 & 720 & -1440 & 1440 & 1440 & 720 & -1440 & 720 & 720 & 11550 & -960 & -1440 & -1440 & -960 & 480
\end{pmatrix}$$

$S = \{1234, 1324, 2341, 2413, 3142, 3421, 4132, 4213\}, \lambda_{max} = 0.129061, \lambda_{min} = -0.182374$

$$H_S = \frac{1}{6 \cdot 5^6} \times \begin{pmatrix}
-2112 & -312 & 288 & 288 & -312 & 5394 & 1152 & 1152 & 288 & 2592 & 864 & 864 & 288 & 2592 & 864 & 864 \\
-312 & -2112 & -312 & 288 & -5118 & -312 & 6798 & 1152 & -2016 & 288 & 1728 & 864 & -2016 & 288 & 1728 & 864 \\
288 & -312 & -2112 & -312 & -576 & -6522 & -312 & 8634 & -288 & -1152 & 288 & 1152 & -288 & -1152 & 288 & 1152 \\
288 & 288 & -312 & -2112 & -576 & -576 & -8358 & -312 & -288 & -288 & -576 & 288 & -288 & -288 & -576 & 288 \\
-312 & -5118 & -576 & -576 & -2112 & -312 & 288 & 288 & -312 & 1398 & 1728 & 1728 & 288 & 2592 & 864 & 864 \\
5394 & -312 & -6522 & -576 & -312 & -2112 & -312 & 288 & -1122 & -312 & 3738 & 1728 & -2016 & 288 & 1728 & 864 \\
1152 & 6798 & -312 & -8358 & 288 & -312 & -2112 & -312 & -1152 & -3462 & -312 & 6798 & -288 & -1152 & 288 & 1152 \\
1152 & 1152 & 8634 & -312 & 288 & 288 & -312 & -2112 & -1152 & -1152 & -6522 & -312 & -288 & -288 & -576 & 288 \\
288 & -2016 & -288 & -288 & -312 & -1122 & -1152 & -1152 & -2112 & -312 & 288 & 288 & -312 & -1446 & 2592 & 2592 \\
2592 & 288 & -1152 & -288 & 1398 & -312 & -3462 & -1152 & -312 & -2112 & -312 & 288 & 1722 & -312 & 1398 & 2592 \\
864 & 1728 & 288 & -576 & 1728 & 3738 & -312 & -6522 & 288 & -312 & -2112 & -312 & -2016 & -1122 & -312 & 5394 \\
864 & 864 & 1152 & 288 & 1728 & 1728 & 6798 & -312 & 288 & 288 & -312 & -2112 & -2016 & -2016 & -5118 & -312 \\
288 & -2016 & -288 & -288 & 288 & -2016 & -288 & -288 & -312 & 1722 & -2016 & -2016 & -2112 & -312 & 288 & 288 \\
2592 & 288 & -1152 & -288 & 2592 & 288 & -1152 & -288 & -1446 & -312 & -1122 & -2016 & -312 & -2112 & -312 & 288 \\
864 & 1728 & 288 & -576 & 864 & 1728 & 288 & -576 & 2592 & 1398 & -312 & -5118 & 288 & -312 & -2112 & -312 \\
864 & 864 & 1152 & 288 & 864 & 864 & 1152 & 288 & 2592 & 2592 & 5394 & -312 & 288 & 288 & -312 & -2112
\end{pmatrix}$$

$S = \{1234, 1324, 2341, 2413, 3241, 3412, 4123, 4132\}, \lambda_{max} = 0.318475, \lambda_{min} = -0.258919$

$$H_S = \frac{1}{6 \cdot 5^6} \times \begin{pmatrix}
1344 & -1176 & -2016 & -2016 & -96 & 9984 & 3744 & 3744 & -576 & 504 & 864 & 864 & -576 & 504 & 864 & 864 \\
-1176 & 1344 & -1176 & -2016 & -9816 & -96 & 9084 & 3744 & 504 & -576 & 504 & 864 & 504 & -576 & 504 & 864 \\
-2016 & -1176 & 1344 & -1176 & -3456 & -8916 & -96 & 9984 & 864 & 504 & -576 & 504 & 864 & 504 & -576 & 504 \\
-2016 & -2016 & -1176 & 1344 & -3456 & -3456 & -9816 & -96 & 864 & 864 & 504 & -576 & 864 & 864 & 504 & -576 \\
-96 & -9816 & -3456 & -3456 & 1344 & -1176 & -2016 & -2016 & -96 & 9984 & 3744 & 3744 & -576 & 504 & 864 & 864 \\
9984 & -96 & -8916 & -3456 & -1176 & 1344 & -1176 & -2016 & -9816 & -96 & 9084 & 3744 & 504 & -576 & 504 & 864 \\
3744 & 9084 & -96 & -9816 & -2016 & -1176 & 1344 & -1176 & -3456 & -8916 & -96 & 9984 & 864 & 504 & -576 & 504 \\
3744 & 3744 & 9984 & -96 & -2016 & -2016 & -1176 & 1344 & -3456 & -3456 & -9816 & -96 & 864 & 864 & 504 & -576 \\
-576 & 504 & 864 & 864 & -96 & -9816 & -3456 & -3456 & 1344 & -1176 & -2016 & -2016 & -96 & 9984 & 3744 & 3744 \\
504 & -576 & 504 & 864 & 9984 & -96 & -8916 & -3456 & -1176 & 1344 & -1176 & -2016 & -9816 & -96 & 9084 & 3744 \\
864 & 504 & -576 & 504 & 3744 & 9084 & -96 & -9816 & -2016 & -1176 & 1344 & -1176 & -3456 & -8916 & -96 & 9984 \\
864 & 864 & 504 & -576 & 3744 & 3744 & 9984 & -96 & -2016 & -2016 & -1176 & 1344 & -3456 & -3456 & -9816 & -96 \\
-576 & 504 & 864 & 864 & -576 & 504 & 864 & 864 & -96 & -9816 & -3456 & -3456 & 1344 & -1176 & -2016 & -2016 \\
504 & -576 & 504 & 864 & 504 & -576 & 504 & 864 & 9984 & -96 & -8916 & -3456 & -1176 & 1344 & -1176 & -2016 \\
864 & 504 & -576 & 504 & 864 & 504 & -576 & 504 & 3744 & 9084 & -96 & -9816 & -2016 & -1176 & 1344 & -1176 \\
864 & 864 & 504 & -576 & 864 & 864 & 504 & -576 & 3744 & 3744 & 9984 & -96 & -2016 & -2016 & -1176 & 1344
\end{pmatrix}$$

$S = \{1234, 1342, 2143, 2314, 3412, 3421, 4123, 4231\}, \lambda_{max} = 0.300121, \lambda_{min} = -0.213317$

$$H_S = \frac{1}{6 \cdot 5^6} \times \begin{pmatrix}
2496 & -24 & -864 & -864 & -24 & 6312 & -1080 & -1080 & -864 & -2520 & 1152 & 1152 & -864 & -2520 & 1152 & 1152 \\
-24 & 2496 & -24 & -864 & -6000 & -24 & 9516 & -1080 & 2952 & -864 & -1944 & 1152 & 2952 & -864 & -1944 & 1152 \\
-864 & -24 & 2496 & -24 & 1512 & -9204 & -24 & 12072 & 0 & 2376 & -864 & -1080 & 0 & 2376 & -864 & -1080 \\
-864 & -864 & -24 & 2496 & 1512 & 1512 & -11760 & -24 & 0 & 0 & 1512 & -864 & 0 & 0 & 1512 & -864 \\
-24 & -6000 & 1512 & 1512 & 2496 & -24 & -864 & -864 & -24 & 5916 & -1944 & -1944 & -864 & -2520 & 1152 & 1152 \\
6312 & -24 & -9204 & 1512 & -24 & 2496 & -24 & -864 & -5604 & -24 & 8256 & -1944 & 2952 & -864 & -1944 & 1152 \\
-1080 & 9516 & -24 & -11760 & -864 & -24 & 2496 & -24 & 2376 & -7944 & -24 & 9516 & 0 & 2376 & -864 & -1080 \\
-1080 & -1080 & 12072 & -24 & -864 & -864 & -24 & 2496 & 2376 & 2376 & -9204 & -24 & 0 & 0 & 1512 & -864 \\
-864 & 2952 & 0 & 0 & -24 & -5604 & 2376 & 2376 & 2496 & -24 & -864 & -864 & -24 & 4152 & -2520 & -2520 \\
-2520 & -864 & 2376 & 0 & 5916 & -24 & -7944 & 2376 & -24 & 2496 & -24 & -864 & -3840 & -24 & 5916 & -2520 \\
1152 & -1944 & -864 & 1512 & -1944 & 8256 & -24 & -9204 & -864 & -24 & 2496 & -24 & 2952 & -5604 & -24 & 6312 \\
1152 & 1152 & -1080 & -864 & -1944 & -1944 & 9516 & -24 & -864 & -864 & -24 & 2496 & 2952 & 2952 & -6000 & -24 \\
-864 & 2952 & 0 & 0 & -864 & 2952 & 0 & 0 & -24 & -3840 & 2952 & 2952 & 2496 & -24 & -864 & -864 \\
-2520 & -864 & 2376 & 0 & -2520 & -864 & 2376 & 0 & 4152 & -24 & -5604 & 2952 & -24 & 2496 & -24 & -864 \\
1152 & -1944 & -864 & 1512 & 1152 & -1944 & -864 & 1512 & -2520 & 5916 & -24 & -6000 & -864 & -24 & 2496 & -24 \\
1152 & 1152 & -1080 & -864 & 1152 & 1152 & -1080 & -864 & -2520 & -2520 & 6312 & -24 & -864 & -864 & -24 & 2496
\end{pmatrix}$$

$S = \{1234, 1342, 2143, 2413, 3124, 3421, 4231, 4312\}, \lambda_{max} = 0.110240, \lambda_{min} = -0.157279$

$$H_S = \frac{1}{6 \cdot 5^6} \times \begin{pmatrix}
-960 & 840 & 1440 & 1440 & -240 & 1722 & -72 & -72 & 0 & -4032 & 1152 & 1152 & 0 & -4032 & 1152 & 1152 \\
840 & -960 & 840 & 1440 & -1302 & -240 & 1830 & -72 & 4032 & 0 & -4320 & 1152 & 4032 & 0 & -4320 & 1152 \\
1440 & 840 & -960 & 840 & 792 & -1410 & -240 & 1722 & -1152 & 4320 & 0 & -4032 & -1152 & 4320 & 0 & -4032 \\
1440 & 1440 & 840 & -960 & 792 & 792 & -1302 & -240 & -1152 & -1152 & 4032 & 0 & -1152 & -1152 & 4032 & 0 \\
-240 & -1302 & 792 & 792 & -960 & 840 & 1440 & 1440 & -240 & 2730 & -360 & -360 & 0 & -4032 & 1152 & 1152 \\
1722 & -240 & -1410 & 792 & 840 & -960 & 840 & 1440 & -2310 & -240 & 2910 & -360 & 4032 & 0 & -4320 & 1152 \\
-72 & 1830 & -240 & -1302 & 1440 & 840 & -960 & 840 & 1080 & -2490 & -240 & 2730 & -1152 & 4320 & 0 & -4032 \\
-72 & -72 & 1722 & -240 & 1440 & 1440 & 840 & -960 & 1080 & 1080 & -2310 & -240 & -1152 & -1152 & 4032 & 0 \\
0 & 4032 & -1152 & -1152 & -240 & -2310 & 1080 & 1080 & -960 & 840 & 1440 & 1440 & -240 & 1722 & -72 & -72 \\
-4032 & 0 & 4320 & -1152 & 2730 & -240 & -2490 & 1080 & 840 & -960 & 840 & 1440 & -1302 & -240 & 1830 & -72 \\
1152 & -4320 & 0 & 4032 & -360 & 2910 & -240 & -2310 & 1440 & 840 & -960 & 840 & 792 & -1410 & -240 & 1722 \\
1152 & 1152 & -4032 & 0 & -360 & -360 & 2730 & -240 & 1440 & 1440 & 840 & -960 & 792 & 792 & -1302 & -240 \\
0 & 4032 & -1152 & -1152 & 0 & 4032 & -1152 & -1152 & -240 & -1302 & 792 & 792 & -960 & 840 & 1440 & 1440 \\
-4032 & 0 & 4320 & -1152 & -4032 & 0 & 4320 & -1152 & 1722 & -240 & -1410 & 792 & 840 & -960 & 840 & 1440 \\
1152 & -4320 & 0 & 4032 & 1152 & -4320 & 0 & 4032 & -72 & 1830 & -240 & -1302 & 1440 & 840 & -960 & 840 \\
1152 & 1152 & -4032 & 0 & 1152 & 1152 & -4032 & 0 & -72 & -72 & 1722 & -240 & 1440 & 1440 & 840 & -960
\end{pmatrix}$$

$S = \{1234, 1342, 2143, 2431, 3124, 3412, 4213, 4321\}, \lambda_{max} = 0.083022, \lambda_{min} = -0.061073$

$$H_S = \frac{1}{6 \cdot 5^6} \times \begin{pmatrix}
2496 & 1056 & 576 & 576 & -1104 & 156 & 576 & 576 & -2304 & -144 & 576 & 576 & -2304 & -144 & 576 & 576 \\
1056 & 2496 & 1056 & 576 & 156 & -1104 & 156 & 576 & -144 & -2304 & -144 & 576 & -144 & -2304 & -144 & 576 \\
576 & 1056 & 2496 & 1056 & 576 & 156 & -1104 & 156 & 576 & -144 & -2304 & -144 & 576 & -144 & -2304 & -144 \\
576 & 576 & 1056 & 2496 & 576 & 576 & 156 & -1104 & 576 & 576 & -144 & -2304 & 576 & 576 & -144 & -2304 \\
-1104 & 156 & 576 & 576 & 2496 & 1056 & 576 & 576 & -1104 & 156 & 576 & 576 & -2304 & -144 & 576 & 576 \\
156 & -1104 & 156 & 576 & 1056 & 2496 & 1056 & 576 & 156 & -1104 & 156 & 576 & -144 & -2304 & -144 & 576 \\
576 & 156 & -1104 & 156 & 576 & 1056 & 2496 & 1056 & 576 & 156 & -1104 & 156 & 576 & -144 & -2304 & -144 \\
576 & 576 & 156 & -1104 & 576 & 576 & 1056 & 2496 & 576 & 576 & 156 & -1104 & 576 & 576 & -144 & -2304 \\
-2304 & -144 & 576 & 576 & -1104 & 156 & 576 & 576 & 2496 & 1056 & 576 & 576 & -1104 & 156 & 576 & 576 \\
-144 & -2304 & -144 & 576 & 156 & -1104 & 156 & 576 & 1056 & 2496 & 1056 & 576 & 156 & -1104 & 156 & 576 \\
576 & -144 & -2304 & -144 & 576 & 156 & -1104 & 156 & 576 & 1056 & 2496 & 1056 & 576 & 156 & -1104 & 156 \\
576 & 576 & -144 & -2304 & 576 & 576 & 156 & -1104 & 576 & 576 & 1056 & 2496 & 576 & 576 & 156 & -1104 \\
-2304 & -144 & 576 & 576 & -2304 & -144 & 576 & 576 & -1104 & 156 & 576 & 576 & 2496 & 1056 & 576 & 576 \\
-144 & -2304 & -144 & 576 & -144 & -2304 & -144 & 576 & 156 & -1104 & 156 & 576 & 1056 & 2496 & 1056 & 576 \\
576 & -144 & -2304 & -144 & 576 & -144 & -2304 & -144 & 576 & 156 & -1104 & 156 & 576 & 1056 & 2496 & 1056 \\
576 & 576 & -144 & -2304 & 576 & 576 & -144 & -2304 & 576 & 576 & 156 & -1104 & 576 & 576 & 1056 & 2496
\end{pmatrix}$$

$S = \{1234, 1342, 2143, 2431, 3124, 3421, 4213, 4312\}, \lambda_{max} = 0.106084, \lambda_{min} = -0.057016$

$$H_S = \frac{1}{6 \cdot 5^6} \times \begin{pmatrix}
-96 & 1704 & 2304 & 2304 & -456 & 156 & -288 & -288 & -576 & -1008 & 576 & 576 & -576 & -1008 & 576 & 576 \\
1704 & -96 & 1704 & 2304 & -168 & -456 & 264 & -288 & -144 & -576 & -1296 & 576 & -144 & -576 & -1296 & 576 \\
2304 & 1704 & -96 & 1704 & 576 & -276 & -456 & 156 & -1728 & 144 & -576 & -1008 & -1728 & 144 & -576 & -1008 \\
2304 & 2304 & 1704 & -96 & 576 & 576 & -168 & -456 & -1728 & -1728 & -144 & -576 & -1728 & -1728 & -144 & -576 \\
-456 & -168 & 576 & 576 & -96 & 1704 & 2304 & 2304 & -456 & 264 & -576 & -576 & -576 & -1008 & 576 & 576 \\
156 & -456 & -276 & 576 & 1704 & -96 & 1704 & 2304 & -276 & -456 & 444 & -576 & -144 & -576 & -1296 & 576 \\
-288 & 264 & -456 & -168 & 2304 & 1704 & -96 & 1704 & 864 & -456 & -456 & 264 & -1728 & 144 & -576 & -1008 \\
-288 & -288 & 156 & -456 & 2304 & 2304 & 1704 & -96 & 864 & 864 & -276 & -456 & -1728 & -1728 & -144 & -576 \\
-576 & -144 & -1728 & -1728 & -456 & -276 & 864 & 864 & -96 & 1704 & 2304 & 2304 & -456 & 156 & -288 & -288 \\
-1008 & -576 & 144 & -1728 & 264 & -456 & -456 & 864 & 1704 & -96 & 1704 & 2304 & -168 & -456 & 264 & -288 \\
576 & -1296 & -576 & -144 & -576 & 444 & -456 & -276 & 2304 & 1704 & -96 & 1704 & 576 & -276 & -456 & 156 \\
576 & 576 & -1008 & -576 & -576 & -576 & 264 & -456 & 2304 & 2304 & 1704 & -96 & 576 & 576 & -168 & -456 \\
-576 & -144 & -1728 & -1728 & -576 & -144 & -1728 & -1728 & -456 & -168 & 576 & 576 & -96 & 1704 & 2304 & 2304 \\
-1008 & -576 & 144 & -1728 & -1008 & -576 & 144 & -1728 & 156 & -456 & -276 & 576 & 1704 & -96 & 1704 & 2304 \\
576 & -1296 & -576 & -144 & 576 & -1296 & -576 & -144 & -288 & 264 & -456 & -168 & 2304 & 1704 & -96 & 1704 \\
576 & 576 & -1008 & -576 & 576 & 576 & -1008 & -576 & -288 & -288 & 156 & -456 & 2304 & 2304 & 1704 & -96
\end{pmatrix}$$

$S = \{1234, 1342, 2143, 2431, 3214, 3412, 4123, 4321\}, \lambda_{max} = 0.174964, \lambda_{min} = -0.020800$

$$H_S = \frac{1}{6\cdot 5^6} \times \begin{pmatrix}
5952 & 192 & -1728 & -1728 & -888 & -438 & 1872 & 1872 & -3168 & 72 & 1152 & 1152 & -3168 & 72 & 1152 & 1152 \\
192 & 5952 & 192 & -1728 & 642 & -888 & -798 & 1872 & 72 & -3168 & 72 & 1152 & 72 & -3168 & 72 & 1152 \\
-1728 & 192 & 5952 & 192 & -1008 & 1002 & -888 & -438 & 1152 & 72 & -3168 & 72 & 1152 & 72 & -3168 & 72 \\
-1728 & -1728 & 192 & 5952 & -1008 & -1008 & 642 & -888 & 1152 & 1152 & 72 & -3168 & 1152 & 1152 & 72 & -3168 \\
-888 & 642 & -1008 & -1008 & 5952 & 192 & -1728 & -1728 & -888 & 102 & 432 & 432 & -3168 & 72 & 1152 & 1152 \\
-438 & -888 & 1002 & -1008 & 192 & 5952 & 192 & -1728 & 102 & -888 & 102 & 432 & 72 & -3168 & 72 & 1152 \\
1872 & -798 & -888 & 642 & -1728 & 192 & 5952 & 192 & 432 & 102 & -888 & 102 & 1152 & 72 & -3168 & 72 \\
1872 & 1872 & -438 & -888 & -1728 & -1728 & 192 & 5952 & 432 & 432 & 102 & -888 & 1152 & 1152 & 72 & -3168 \\
-3168 & 72 & 1152 & 1152 & -888 & 102 & 432 & 432 & 5952 & 192 & -1728 & -1728 & -888 & 642 & -1008 & -1008 \\
72 & -3168 & 72 & 1152 & 102 & -888 & 102 & 432 & 192 & 5952 & 192 & -1728 & -438 & -888 & 1002 & -1008 \\
1152 & 72 & -3168 & 72 & 432 & 102 & -888 & 102 & -1728 & 192 & 5952 & 192 & 1872 & -798 & -888 & 642 \\
1152 & 1152 & 72 & -3168 & 432 & 432 & 102 & -888 & -1728 & -1728 & 192 & 5952 & 1872 & 1872 & -438 & -888 \\
-3168 & 72 & 1152 & 1152 & -3168 & 72 & 1152 & 1152 & -888 & -438 & 1872 & 1872 & 5952 & 192 & -1728 & -1728 \\
72 & -3168 & 72 & 1152 & 72 & -3168 & 72 & 1152 & 642 & -888 & -798 & 1872 & 192 & 5952 & 192 & -1728 \\
1152 & 72 & -3168 & 72 & 1152 & 72 & -3168 & 72 & -1008 & 1002 & -888 & -438 & -1728 & 192 & 5952 & 192 \\
1152 & 1152 & 72 & -3168 & 1152 & 1152 & 72 & -3168 & -1008 & -1008 & 642 & -888 & -1728 & -1728 & 192 & 5952
\end{pmatrix}$$

$S = \{1234, 1342, 2143, 2431, 3214, 3421, 4123, 4312\}, \lambda_{max} = 0.097492, \lambda_{min} = -0.018209$

$$H_S = \frac{1}{6\cdot 5^6} \times \begin{pmatrix}
3360 & 840 & 0 & 0 & -240 & -438 & 1008 & 1008 & -1440 & -792 & 1152 & 1152 & -1440 & -792 & 1152 & 1152 \\
840 & 3360 & 840 & 0 & 318 & -240 & -690 & 1008 & 72 & -1440 & -1080 & 1152 & 72 & -1440 & -1080 & 1152 \\
0 & 840 & 3360 & 840 & -1008 & 570 & -240 & -438 & -1152 & 360 & -1440 & -792 & -1152 & 360 & -1440 & -792 \\
0 & 0 & 840 & 3360 & -1008 & -1008 & 318 & -240 & -1152 & -1152 & 72 & -1440 & -1152 & -1152 & 72 & -1440 \\
-240 & 318 & -1008 & -1008 & 3360 & 840 & 0 & 0 & -240 & 210 & -720 & -720 & -1440 & -792 & 1152 & 1152 \\
-438 & -240 & 570 & -1008 & 840 & 3360 & 840 & 0 & -330 & -240 & 390 & -720 & 72 & -1440 & -1080 & 1152 \\
1008 & -690 & -240 & 318 & 0 & 840 & 3360 & 840 & 720 & -510 & -240 & 210 & -1152 & 360 & -1440 & -792 \\
1008 & 1008 & -438 & -240 & 0 & 0 & 840 & 3360 & 720 & 720 & -330 & -240 & -1152 & -1152 & 72 & -1440 \\
-1440 & 72 & -1152 & -1152 & -240 & -330 & 720 & 720 & 3360 & 840 & 0 & 0 & -240 & 642 & -1872 & -1872 \\
-792 & -1440 & 360 & -1152 & 210 & -240 & -510 & 720 & 840 & 3360 & 840 & 0 & -762 & -240 & 1110 & -1872 \\
1152 & -1080 & -1440 & 72 & -720 & 390 & -240 & -330 & 0 & 840 & 3360 & 840 & 1872 & -1230 & -240 & 642 \\
1152 & 1152 & -792 & -1440 & -720 & -720 & 210 & -240 & 0 & 0 & 840 & 3360 & 1872 & 1872 & -762 & -240 \\
-1440 & 72 & -1152 & -1152 & -1440 & 72 & -1152 & -1152 & -240 & -762 & 1872 & 1872 & 3360 & 840 & 0 & 0 \\
-792 & -1440 & 360 & -1152 & -792 & -1440 & 360 & -1152 & 642 & -240 & -1230 & 1872 & 840 & 3360 & 840 & 0 \\
1152 & -1080 & -1440 & 72 & 1152 & -1080 & -1440 & 72 & -1872 & 1110 & -240 & -762 & 0 & 840 & 3360 & 840 \\
1152 & 1152 & -792 & -1440 & 1152 & 1152 & -792 & -1440 & -1872 & -1872 & 642 & -240 & 0 & 0 & 840 & 3360
\end{pmatrix}$$

$S = \{1234, 1342, 2314, 2413, 3142, 3421, 4123, 4231\}, \lambda_{max} = 0.233513, \lambda_{min} = -0.276085$

$$H_S = \frac{1}{6\cdot 5^6} \times \begin{pmatrix}
-2112 & -312 & 288 & 288 & -312 & 8094 & -1008 & -1008 & 288 & -2448 & 864 & 864 & 288 & -2448 & 864 & 864 \\
-312 & -2112 & -312 & 288 & -7818 & -312 & 9498 & -1008 & 3024 & 288 & -1872 & 864 & 3024 & 288 & -1872 & 864 \\
288 & -312 & -2112 & -312 & 1584 & -9222 & -312 & 10254 & -288 & 2448 & 288 & -1008 & -288 & 2448 & 288 & -1008 \\
288 & 288 & -312 & -2112 & 1584 & 1584 & -9978 & -312 & -288 & -288 & 1584 & 288 & -288 & -288 & 1584 & 288 \\
-312 & -7818 & 1584 & 1584 & -2112 & -312 & 288 & 288 & -312 & 5898 & -1872 & -1872 & 288 & -2448 & 864 & 864 \\
8094 & -312 & -9222 & 1584 & -312 & -2112 & -312 & 288 & -5622 & -312 & 8238 & -1872 & 3024 & 288 & -1872 & 864 \\
-1008 & 9498 & -312 & -9978 & 288 & -312 & -2112 & -312 & 2448 & -7962 & -312 & 9498 & -288 & 2448 & 288 & -1008 \\
-1008 & -1008 & 10254 & -312 & 288 & 288 & -312 & -2112 & 2448 & 2448 & -9222 & -312 & -288 & -288 & 1584 & 288 \\
288 & 3024 & -288 & -288 & -312 & -5622 & 2448 & 2448 & -2112 & -312 & 288 & 288 & -312 & 2334 & -2448 & -2448 \\
-2448 & 288 & 2448 & -288 & 5898 & -312 & -7962 & 2448 & -312 & -2112 & -312 & 288 & -2058 & -312 & 5898 & -2448 \\
864 & -1872 & 288 & 1584 & -1872 & 8238 & -312 & -9222 & 288 & -312 & -2112 & -312 & 3024 & -5622 & -312 & 8094 \\
864 & 864 & -1008 & 288 & -1872 & -1872 & 9498 & -312 & 288 & 288 & -312 & -2112 & 3024 & 3024 & -7818 & -312 \\
288 & 3024 & -288 & -288 & 288 & 3024 & -288 & -288 & -312 & -2058 & 3024 & 3024 & -2112 & -312 & 288 & 288 \\
-2448 & 288 & 2448 & -288 & -2448 & 288 & 2448 & -288 & 2334 & -312 & -5622 & 3024 & -312 & -2112 & -312 & 288 \\
864 & -1872 & 288 & 1584 & 864 & -1872 & 288 & 1584 & -2448 & 5898 & -312 & -7818 & 288 & -312 & -2112 & -312 \\
864 & 864 & -1008 & 288 & 864 & 864 & -1008 & 288 & -2448 & -2448 & 8094 & -312 & 288 & 288 & -312 & -2112
\end{pmatrix}$$

$S = \{1234, 1342, 2314, 2413, 3241, 3421, 4123, 4132\}, \lambda_{max} = 0.171623, \lambda_{min} = -0.217723$

$$H_S = \frac{1}{6\cdot 5^6} \times \begin{pmatrix}
-1248 & -528 & -288 & -288 & 552 & 6528 & 2016 & 2016 & 1152 & -2664 & 288 & 288 & 1152 & -2664 & 288 & 288 \\
-528 & -1248 & -528 & -288 & -6684 & 552 & 7032 & 2016 & 2808 & 1152 & -2088 & 288 & 2808 & 1152 & -2088 & 288 \\
-288 & -528 & -1248 & -528 & -2592 & -7188 & 552 & 8688 & -864 & 2232 & 1152 & -1224 & -864 & 2232 & 1152 & -1224 \\
-288 & -288 & -528 & -1248 & -2592 & -2592 & -8844 & 552 & -864 & -864 & 1368 & 1152 & -864 & -864 & 1368 & 1152 \\
552 & -6684 & -2592 & -2592 & -1248 & -528 & -288 & -288 & 552 & 4332 & 1152 & 1152 & 1152 & -2664 & 288 & 288 \\
6528 & 552 & -7188 & -2592 & -528 & -1248 & -528 & -288 & -4488 & 552 & 5772 & 1152 & 2808 & 1152 & -2088 & 288 \\
2016 & 7032 & 552 & -8844 & -288 & -528 & -1248 & -528 & -1728 & -5928 & 552 & 7932 & -864 & 2232 & 1152 & -1224 \\
2016 & 2016 & 8688 & 552 & -288 & -288 & -528 & -1248 & -1728 & -1728 & -8088 & 552 & -864 & -864 & 1368 & 1152 \\
1152 & 2808 & -864 & -864 & 552 & -4488 & -1728 & -1728 & -1248 & -528 & -288 & -288 & 552 & 768 & 576 & 576 \\
-2664 & 1152 & 2232 & -864 & 4332 & 552 & -5928 & -1728 & -528 & -1248 & -528 & -288 & -924 & 552 & 3432 & 576 \\
288 & -2088 & 1152 & 1368 & 1152 & 5772 & 552 & -8088 & -288 & -528 & -1248 & -528 & -1152 & -3588 & 552 & 6528 \\
288 & 288 & -1224 & 1152 & 1152 & 1152 & 7932 & 552 & -288 & -288 & -528 & -1248 & -1152 & -1152 & -6684 & 552 \\
1152 & 2808 & -864 & -864 & 1152 & 2808 & -864 & -864 & 552 & -924 & -1152 & -1152 & -1248 & -528 & -288 & -288 \\
-2664 & 1152 & 2232 & -864 & -2664 & 1152 & 2232 & -864 & 768 & 552 & -3588 & -1152 & -528 & -1248 & -528 & -288 \\
288 & -2088 & 1152 & 1368 & 288 & -2088 & 1152 & 1368 & 576 & 3432 & 552 & -6684 & -288 & -528 & -1248 & -528 \\
288 & 288 & -1224 & 1152 & 288 & 288 & -1224 & 1152 & 576 & 576 & 6528 & 552 & -288 & -288 & -528 & -1248
\end{pmatrix}$$

$S = \{1234, 1342, 2341, 2413, 3124, 3412, 4123, 4231\}, \lambda_{max} = 0.440077, \lambda_{min} = -0.348875$

$$H_S = \frac{1}{6 \cdot 5^6} \times \begin{pmatrix}
1344 & -96 & -576 & -576 & -1176 & 12684 & 504 & 504 & -2016 & -3456 & 864 & 864 & -2016 & -3456 & 864 & 864 \\
-96 & 1344 & -96 & -576 & -12516 & -1176 & 12684 & 504 & 3744 & -2016 & -3456 & 864 & 3744 & -2016 & -3456 & 864 \\
-576 & -96 & 1344 & -96 & 504 & -12516 & -1176 & 12684 & 864 & 3744 & -2016 & -3456 & 864 & 3744 & -2016 & -3456 \\
-576 & -576 & -96 & 1344 & 504 & 504 & -12516 & -1176 & 864 & 864 & 3744 & -2016 & 864 & 864 & 3744 & -2016 \\
-1176 & -12516 & 504 & 504 & 1344 & -96 & -576 & -576 & -1176 & 13584 & 504 & 504 & -2016 & -3456 & 864 & 864 \\
12684 & -1176 & -12516 & 504 & -96 & 1344 & -96 & -576 & -13416 & -1176 & 13584 & 504 & 3744 & -2016 & -3456 & 864 \\
504 & 12684 & -1176 & -12516 & -576 & -96 & 1344 & -96 & 504 & -13416 & -1176 & 13584 & 864 & 3744 & -2016 & -3456 \\
504 & 504 & 12684 & -1176 & -576 & -576 & -96 & 1344 & 504 & 504 & -13416 & -1176 & 864 & 864 & 3744 & -2016 \\
-2016 & 3744 & 864 & 864 & -1176 & -13416 & 504 & 504 & 1344 & -96 & -576 & -576 & -1176 & 12684 & 504 & 504 \\
-3456 & -2016 & 3744 & 864 & 13584 & -1176 & -13416 & 504 & -96 & 1344 & -96 & -576 & -12516 & -1176 & 12684 & 504 \\
864 & -3456 & -2016 & 3744 & 504 & 13584 & -1176 & -13416 & -576 & -96 & 1344 & -96 & 504 & -12516 & -1176 & 12684 \\
864 & 864 & -3456 & -2016 & 504 & 504 & 13584 & -1176 & -576 & -576 & -96 & 1344 & 504 & 504 & -12516 & -1176 \\
-2016 & 3744 & 864 & 864 & -2016 & 3744 & 864 & 864 & -1176 & -12516 & 504 & 504 & 1344 & -96 & -576 & -576 \\
-3456 & -2016 & 3744 & 864 & -3456 & -2016 & 3744 & 864 & 12684 & -1176 & -12516 & 504 & -96 & 1344 & -96 & -576 \\
864 & -3456 & -2016 & 3744 & 864 & -3456 & -2016 & 3744 & 504 & 12684 & -1176 & -12516 & -576 & -96 & 1344 & -96 \\
864 & 864 & -3456 & -2016 & 864 & 864 & -3456 & -2016 & 504 & 504 & 12684 & -1176 & -576 & -576 & -96 & 1344
\end{pmatrix}$$

$S = \{1234, 1342, 2341, 2413, 3124, 3421, 4132, 4213\}, \lambda_{max} = 0.193614, \lambda_{min} = -0.225969$

$$H_S = \frac{1}{6 \cdot 5^6} \times \begin{pmatrix}
-1248 & 552 & 1152 & 1152 & -528 & 6528 & 936 & 936 & -288 & -1584 & 288 & 288 & -288 & -1584 & 288 & 288 \\
552 & -1248 & 552 & 1152 & -6684 & -528 & 7932 & 936 & 1008 & -288 & -2448 & 288 & 1008 & -288 & -2448 & 288 \\
1152 & 552 & -1248 & 552 & -792 & -8088 & -528 & 9768 & -864 & 1872 & -288 & -3024 & -864 & 1872 & -288 & -3024 \\
1152 & 1152 & 552 & -1248 & -792 & -792 & -9924 & -528 & -864 & -864 & 2448 & -288 & -864 & -864 & 2448 & -288 \\
-528 & -6684 & -792 & -792 & -1248 & 552 & 1152 & 1152 & -528 & 3432 & 1512 & 1512 & -288 & -1584 & 288 & 288 \\
6528 & -528 & -8088 & -792 & 552 & -1248 & 552 & 1152 & -3588 & -528 & 5772 & 1512 & 1008 & -288 & -2448 & 288 \\
936 & 7932 & -528 & -9924 & 1152 & 552 & -1248 & 552 & -1368 & -5928 & -528 & 8832 & -864 & 1872 & -288 & -3024 \\
936 & 936 & 9768 & -528 & 1152 & 1152 & 552 & -1248 & -1368 & -1368 & -8988 & -528 & -864 & -864 & 2448 & -288 \\
-288 & 1008 & -864 & -864 & -528 & -3588 & -1368 & -1368 & -1248 & 552 & 1152 & 1152 & -528 & -312 & 2376 & 2376 \\
-1584 & -288 & 1872 & -864 & 3432 & -528 & -5928 & -1368 & 552 & -1248 & 552 & 1152 & 156 & -528 & 2532 & 2376 \\
288 & -2448 & -288 & 2448 & 1512 & 5772 & -528 & -8988 & 1152 & 552 & -1248 & 552 & -2232 & -2688 & -528 & 6528 \\
288 & 288 & -3024 & -288 & 1512 & 1512 & 8832 & -528 & 1152 & 1152 & 552 & -1248 & -2232 & -2232 & -6684 & -528 \\
-288 & 1008 & -864 & -864 & -288 & 1008 & -864 & -864 & -528 & 156 & -2232 & -2232 & -1248 & 552 & 1152 & 1152 \\
-1584 & -288 & 1872 & -864 & -1584 & -288 & 1872 & -864 & -312 & -528 & -2688 & -2232 & 552 & -1248 & 552 & 1152 \\
288 & -2448 & -288 & 2448 & 288 & -2448 & -288 & 2448 & 2376 & 2532 & -528 & -6684 & 1152 & 552 & -1248 & 552 \\
288 & 288 & -3024 & -288 & 288 & 288 & -3024 & -288 & 2376 & 2376 & 6528 & -528 & 1152 & 1152 & 552 & -1248
\end{pmatrix}$$

$S = \{1234, 1342, 2341, 2413, 3214, 3421, 4123, 4132\}, \lambda_{max} = 0.249499, \lambda_{min} = -0.163784$

$$H_S = \frac{1}{6 \cdot 5^6} \times \begin{pmatrix}
2208 & -312 & -1152 & -1152 & -312 & 5934 & 2232 & 2232 & -1152 & -1368 & 864 & 864 & -1152 & -1368 & 864 & 864 \\
-312 & 2208 & -312 & -1152 & -6198 & -312 & 6978 & 2232 & 1224 & -1152 & -2232 & 864 & 1224 & -1152 & -2232 & 864 \\
-1152 & -312 & 2208 & -312 & -2376 & -7242 & -312 & 9174 & -288 & 2088 & -1152 & -2808 & -288 & 2088 & -1152 & -2808 \\
-1152 & -1152 & -312 & 2208 & -2376 & -2376 & -9438 & -312 & -288 & -288 & 2664 & -1152 & -288 & -288 & 2664 & -1152 \\
-312 & -6198 & -2376 & -2376 & 2208 & -312 & -1152 & -1152 & -312 & 3378 & 1368 & 1368 & -1152 & -1368 & 864 & 864 \\
5934 & -312 & -7242 & -2376 & -312 & 2208 & -312 & -1152 & -3642 & -312 & 5718 & 1368 & 1224 & -1152 & -2232 & 864 \\
2232 & 6978 & -312 & -9438 & -1152 & -312 & 2208 & -312 & -1512 & -5982 & -312 & 8778 & -288 & 2088 & -1152 & -2808 \\
2232 & 2232 & 9174 & -312 & -1152 & -1152 & -312 & 2208 & -1512 & -1512 & -9042 & -312 & -288 & -288 & 2664 & -1152 \\
-1152 & 1224 & -288 & -288 & -312 & -3642 & -1512 & -1512 & 2208 & -312 & -1152 & -1152 & -312 & 174 & 792 & 792 \\
-1368 & -1152 & 2088 & -288 & 3378 & -312 & -5982 & -1512 & -312 & 2208 & -312 & -1152 & -438 & -312 & 3378 & 792 \\
864 & -2232 & -1152 & 2664 & 1368 & 5718 & -312 & -9042 & -1152 & -312 & 2208 & -312 & -936 & -3642 & -312 & 7014 \\
864 & 864 & -2808 & -1152 & 1368 & 1368 & 8778 & -312 & -1152 & -1152 & -312 & 2208 & -936 & -936 & -7278 & -312 \\
-1152 & 1224 & -288 & -288 & -1152 & 1224 & -288 & -288 & -312 & -438 & -936 & -936 & 2208 & -312 & -1152 & -1152 \\
-1368 & -1152 & 2088 & -288 & -1368 & -1152 & 2088 & -288 & 174 & -312 & -3642 & -936 & -312 & 2208 & -312 & -1152 \\
864 & -2232 & -1152 & 2664 & 864 & -2232 & -1152 & 2664 & 792 & 3378 & -312 & -7278 & -1152 & -312 & 2208 & -312 \\
864 & 864 & -2808 & -1152 & 864 & 864 & -2808 & -1152 & 792 & 792 & 7014 & -312 & -1152 & -1152 & -312 & 2208
\end{pmatrix}$$

$S = \{1234, 1342, 2341, 2431, 3124, 3412, 4123, 4213\}, \lambda_{max} = 0.363518, \lambda_{min} = -0.267719$

$$H_S = \frac{1}{6 \cdot 5^6} \times \begin{pmatrix}
2208 & 768 & 288 & 288 & -1392 & 11118 & 288 & 288 & -2592 & -432 & 288 & 288 & -2592 & -432 & 288 & 288 \\
768 & 2208 & 768 & 288 & -11382 & -1392 & 11118 & 288 & -432 & -2592 & -432 & 288 & -432 & -2592 & -432 & 288 \\
288 & 768 & 2208 & 768 & 288 & -11382 & -1392 & 11118 & 288 & -432 & -2592 & -432 & 288 & -432 & -2592 & -432 \\
288 & 288 & 768 & 2208 & 288 & 288 & -11382 & -1392 & 288 & 288 & -432 & -2592 & 288 & 288 & -432 & -2592 \\
-1392 & -11382 & 288 & 288 & 2208 & 768 & 288 & 288 & -1392 & 11118 & 288 & 288 & -2592 & -432 & 288 & 288 \\
11118 & -1392 & -11382 & 288 & 768 & 2208 & 768 & 288 & -11382 & -1392 & 11118 & 288 & -432 & -2592 & -432 & 288 \\
288 & 11118 & -1392 & -11382 & 288 & 768 & 2208 & 768 & 288 & -11382 & -1392 & 11118 & 288 & -432 & -2592 & -432 \\
288 & 288 & 11118 & -1392 & 288 & 288 & 768 & 2208 & 288 & 288 & -11382 & -1392 & 288 & 288 & -432 & -2592 \\
-2592 & -432 & 288 & 288 & -1392 & -11382 & 288 & 288 & 2208 & 768 & 288 & 288 & -1392 & 11118 & 288 & 288 \\
-432 & -2592 & -432 & 288 & 11118 & -1392 & -11382 & 288 & 768 & 2208 & 768 & 288 & -11382 & -1392 & 11118 & 288 \\
288 & -432 & -2592 & -432 & 288 & 11118 & -1392 & -11382 & 288 & 768 & 2208 & 768 & 288 & -11382 & -1392 & 11118 \\
288 & 288 & -432 & -2592 & 288 & 288 & 11118 & -1392 & 288 & 288 & 768 & 2208 & 288 & 288 & -11382 & -1392 \\
-2592 & -432 & 288 & 288 & -2592 & -432 & 288 & 288 & -1392 & -11382 & 288 & 288 & 2208 & 768 & 288 & 288 \\
-432 & -2592 & -432 & 288 & -432 & -2592 & -432 & 288 & 11118 & -1392 & -11382 & 288 & 768 & 2208 & 768 & 288 \\
288 & -432 & -2592 & -432 & 288 & -432 & -2592 & -432 & 288 & 11118 & -1392 & -11382 & 288 & 768 & 2208 & 768 \\
288 & 288 & -432 & -2592 & 288 & 288 & -432 & -2592 & 288 & 288 & 11118 & -1392 & 288 & 288 & 768 & 2208
\end{pmatrix}$$

$S = \{1234, 1342, 2413, 2431, 3124, 3142, 4213, 4321\}, \lambda_{max} = 0.037736, \lambda_{min} = -0.115342$

$$H_S = \frac{1}{6\cdot 5^6} \times \begin{pmatrix}
-2112 & 768 & 1728 & 1728 & -1392 & 1938 & 648 & 648 & -1152 & -72 & 288 & 288 & -1152 & -72 & 288 & 288 \\
768 & -2112 & 768 & 1728 & -1662 & -1392 & 138 & 648 & -72 & -1152 & -72 & 288 & -72 & -1152 & -72 & 288 \\
1728 & 768 & -2112 & 768 & 648 & 138 & -1392 & -1662 & 288 & -72 & -1152 & -72 & 288 & -72 & -1152 & -72 \\
1728 & 1728 & 768 & -2112 & 648 & 648 & 1938 & -1392 & 288 & 288 & -72 & -1152 & 288 & 288 & -72 & -1152 \\
-1392 & -1662 & 648 & 648 & -2112 & 768 & 1728 & 1728 & -1392 & 138 & 648 & 648 & -1152 & -72 & 288 & 288 \\
1938 & -1392 & 138 & 648 & 768 & -2112 & 768 & 1728 & 138 & -1392 & 138 & 648 & -72 & -1152 & -72 & 288 \\
648 & 138 & -1392 & 1938 & 1728 & 768 & -2112 & 768 & 648 & 138 & -1392 & 138 & 288 & -72 & -1152 & -72 \\
648 & 648 & -1662 & -1392 & 1728 & 1728 & 768 & -2112 & 648 & 648 & 138 & -1392 & 288 & 288 & -72 & -1152 \\
-1152 & -72 & 288 & 288 & -1392 & 138 & 648 & 648 & -2112 & 768 & 1728 & 1728 & -1392 & -1662 & 648 & 648 \\
-72 & -1152 & -72 & 288 & 138 & -1392 & 138 & 648 & 768 & -2112 & 768 & 1728 & 1938 & -1392 & 138 & 648 \\
288 & -72 & -1152 & -72 & 648 & 138 & -1392 & 138 & 1728 & 768 & -2112 & 768 & 648 & 138 & -1392 & 1938 \\
288 & 288 & -72 & -1152 & 648 & 648 & 138 & -1392 & 1728 & 1728 & 768 & -2112 & 648 & 648 & -1662 & -1392 \\
-1152 & -72 & 288 & 288 & -1152 & -72 & 288 & 288 & -1392 & 1938 & 648 & 648 & -2112 & 768 & 1728 & 1728 \\
-72 & -1152 & -72 & 288 & -72 & -1152 & -72 & 288 & -1662 & -1392 & 138 & 648 & 768 & -2112 & 768 & 1728 \\
288 & -72 & -1152 & -72 & 288 & -72 & -1152 & -72 & 648 & 138 & -1392 & -1662 & 1728 & 768 & -2112 & 768 \\
288 & 288 & -72 & -1152 & 288 & 288 & -72 & -1152 & 648 & 648 & 1938 & -1392 & 1728 & 1728 & 768 & -2112
\end{pmatrix}$$

$S = \{1234, 1342, 2413, 2431, 3142, 3214, 4123, 4321\}, \lambda_{max} = 0.082834, \lambda_{min} = -0.072228$

$$H_S = \frac{1}{6\cdot 5^6} \times \begin{pmatrix}
1344 & -96 & -576 & -576 & -1176 & 1344 & 1944 & 1944 & -2016 & 144 & 864 & 864 & -2016 & 144 & 864 & 864 \\
-96 & 1344 & -96 & -576 & -1176 & -1176 & -816 & 1944 & 144 & -2016 & 144 & 864 & 144 & -2016 & 144 & 864 \\
-576 & -96 & 1344 & -96 & -936 & 984 & -1176 & -2256 & 864 & 144 & -2016 & 144 & 864 & 144 & -2016 & 144 \\
-576 & -576 & -96 & 1344 & -936 & -936 & 2424 & -1176 & 864 & 864 & 144 & -2016 & 864 & 864 & 144 & -2016 \\
-1176 & -1176 & -936 & -936 & 1344 & -96 & -576 & -576 & -1176 & 84 & 504 & 504 & -2016 & 144 & 864 & 864 \\
1344 & -1176 & 984 & -936 & -96 & 1344 & -96 & -576 & 84 & -1176 & 84 & 504 & 144 & -2016 & 144 & 864 \\
1944 & -816 & -1176 & 2424 & -576 & -96 & 1344 & -96 & 504 & 84 & -1176 & 84 & 864 & 144 & -2016 & 144 \\
1944 & 1944 & -2256 & -1176 & -576 & -576 & -96 & 1344 & 504 & 504 & 84 & -1176 & 864 & 864 & 144 & -2016 \\
-2016 & 144 & 864 & 864 & -1176 & 84 & 504 & 504 & 1344 & -96 & -576 & -576 & -1176 & -1176 & -936 & -936 \\
144 & -2016 & 144 & 864 & 84 & -1176 & 84 & 504 & -96 & 1344 & -96 & -576 & 1344 & -1176 & 984 & -936 \\
864 & 144 & -2016 & 144 & 504 & 84 & -1176 & 84 & -576 & -96 & 1344 & -96 & 1944 & -816 & -1176 & 2424 \\
864 & 864 & 144 & -2016 & 504 & 504 & 84 & -1176 & -576 & -576 & -96 & 1344 & 1944 & 1944 & -2256 & -1176 \\
-2016 & 144 & 864 & 864 & -2016 & 144 & 864 & 864 & -1176 & 1344 & 1944 & 1944 & 1344 & -96 & -576 & -576 \\
144 & -2016 & 144 & 864 & 144 & -2016 & 144 & 864 & -1176 & -1176 & -816 & 1944 & -96 & 1344 & -96 & -576 \\
864 & 144 & -2016 & 144 & 864 & 144 & -2016 & 144 & -936 & 984 & -1176 & -2256 & -576 & -96 & 1344 & -96 \\
864 & 864 & 144 & -2016 & 864 & 864 & 144 & -2016 & -936 & -936 & 2424 & -1176 & -576 & -576 & -96 & 1344
\end{pmatrix}$$

$\mathbf{S = \{1234, 1432, 2143, 2341, 3214, 3412, 4123, 4321\}}, \lambda_{max} = 0.272976, \lambda_{min} = 0.004816$

$$H_S = \frac{1}{6\cdot 5^6} \times \begin{pmatrix}
9408 & -672 & -4032 & -4032 & -672 & 48 & 288 & 288 & -4032 & 288 & 1728 & 1728 & -4032 & 288 & 1728 & 1728 \\
-672 & 9408 & -672 & -4032 & 48 & -672 & 48 & 288 & 288 & -4032 & 288 & 1728 & 288 & -4032 & 288 & 1728 \\
-4032 & -672 & 9408 & -672 & 288 & 48 & -672 & 48 & 1728 & 288 & -4032 & 288 & 1728 & 288 & -4032 & 288 \\
-4032 & -4032 & -672 & 9408 & 288 & 288 & 48 & -672 & 1728 & 1728 & 288 & -4032 & 1728 & 1728 & 288 & -4032 \\
-672 & 48 & 288 & 288 & 9408 & -672 & -4032 & -4032 & -672 & 48 & 288 & 288 & -4032 & 288 & 1728 & 1728 \\
48 & -672 & 48 & 288 & -672 & 9408 & -672 & -4032 & 48 & -672 & 48 & 288 & 288 & -4032 & 288 & 1728 \\
288 & 48 & -672 & 48 & -4032 & -672 & 9408 & -672 & 288 & 48 & -672 & 48 & 1728 & 288 & -4032 & 288 \\
288 & 288 & 48 & -672 & -4032 & -4032 & -672 & 9408 & 288 & 288 & 48 & -672 & 1728 & 1728 & 288 & -4032 \\
-4032 & 288 & 1728 & 1728 & -672 & 48 & 288 & 288 & 9408 & -672 & -4032 & -4032 & -672 & 48 & 288 & 288 \\
288 & -4032 & 288 & 1728 & 48 & -672 & 48 & 288 & -672 & 9408 & -672 & -4032 & 48 & -672 & 48 & 288 \\
1728 & 288 & -4032 & 288 & 288 & 48 & -672 & 48 & -4032 & -672 & 9408 & -672 & 288 & 48 & -672 & 48 \\
1728 & 1728 & 288 & -4032 & 288 & 288 & 48 & -672 & -4032 & -4032 & -672 & 9408 & 288 & 288 & 48 & -672 \\
-4032 & 288 & 1728 & 1728 & -4032 & 288 & 1728 & 1728 & -672 & 48 & 288 & 288 & 9408 & -672 & -4032 & -4032 \\
288 & -4032 & 288 & 1728 & 288 & -4032 & 288 & 1728 & 48 & -672 & 48 & 288 & -672 & 9408 & -672 & -4032 \\
1728 & 288 & -4032 & 288 & 1728 & 288 & -4032 & 288 & 288 & 48 & -672 & 48 & -4032 & -672 & 9408 & -672 \\
1728 & 1728 & 288 & -4032 & 1728 & 1728 & 288 & -4032 & 288 & 288 & 48 & -672 & -4032 & -4032 & -672 & 9408
\end{pmatrix}$$

$S = \{1234, 1432, 2143, 2341, 3214, 3421, 4123, 4312\}, \lambda_{max} = 0.177081, \lambda_{min} = -0.002856$

$$H_S = \frac{1}{6\cdot 5^6} \times \begin{pmatrix}
6816 & -24 & -2304 & -2304 & -24 & 48 & -576 & -576 & -2304 & -576 & 1728 & 1728 & -2304 & -576 & 1728 & 1728 \\
-24 & 6816 & -24 & -2304 & -276 & -24 & 156 & -576 & 288 & -2304 & -864 & 1728 & 288 & -2304 & -864 & 1728 \\
-2304 & -24 & 6816 & -24 & 288 & -384 & -24 & 48 & -576 & 576 & -2304 & -576 & -576 & 576 & -2304 & -576 \\
-2304 & -2304 & -24 & 6816 & 288 & 288 & -276 & -24 & -576 & -576 & 288 & -2304 & -576 & -576 & 288 & -2304 \\
-24 & -276 & 288 & 288 & 6816 & -24 & -2304 & -2304 & -24 & 156 & -864 & -864 & -2304 & -576 & 1728 & 1728 \\
48 & -24 & -384 & 288 & -24 & 6816 & -24 & -2304 & -384 & -24 & 336 & -864 & 288 & -2304 & -864 & 1728 \\
-576 & 156 & -24 & -276 & -2304 & -24 & 6816 & -24 & 576 & -564 & -24 & 156 & -576 & 576 & -2304 & -576 \\
-576 & -576 & 48 & -24 & -2304 & -2304 & -24 & 6816 & 576 & 576 & -384 & -24 & -576 & -576 & 288 & -2304 \\
-2304 & 288 & -576 & -576 & -24 & -384 & 576 & 576 & 6816 & -24 & -2304 & -2304 & -24 & 48 & -576 & -576 \\
-576 & -2304 & 576 & -576 & 156 & -24 & -564 & 576 & -24 & 6816 & -24 & -2304 & -276 & -24 & 156 & -576 \\
1728 & -864 & -2304 & 288 & -864 & 336 & -24 & -384 & -2304 & -24 & 6816 & -24 & 288 & -384 & -24 & 48 \\
1728 & 1728 & -576 & -2304 & -864 & -864 & 156 & -24 & -2304 & -2304 & -24 & 6816 & 288 & 288 & -276 & -24 \\
-2304 & 288 & -576 & -576 & -2304 & 288 & -576 & -576 & -24 & -276 & 288 & 288 & 6816 & -24 & -2304 & -2304 \\
-576 & -2304 & 576 & -576 & -576 & -2304 & 576 & -576 & 48 & -24 & -384 & 288 & -24 & 6816 & -24 & -2304 \\
1728 & -864 & -2304 & 288 & 1728 & -864 & -2304 & 288 & -576 & 156 & -24 & -276 & -2304 & -24 & 6816 & -24 \\
1728 & 1728 & -576 & -2304 & 1728 & 1728 & -576 & -2304 & -576 & -576 & 48 & -24 & -2304 & -2304 & -24 & 6816
\end{pmatrix}$$

$S = \{1234, 1432, 2341, 2413, 3142, 3214, 4123, 4321\}, \lambda_{max} = 0.173488, \lambda_{min} = -0.030414$

$$H_S = \frac{1}{6 \cdot 5^6} \times \begin{pmatrix}
4800 & -960 & -2880 & -2880 & -960 & 1830 & 360 & 360 & -2880 & 360 & 1440 & 1440 & -2880 & 360 & 1440 & 1440 \\
-960 & 4800 & -960 & -2880 & -1770 & -960 & 30 & 360 & 360 & -2880 & 360 & 1440 & 360 & -2880 & 360 & 1440 \\
-2880 & -960 & 4800 & -960 & 360 & 30 & -960 & -1770 & 1440 & 360 & -2880 & 360 & 1440 & 360 & -2880 & 360 \\
-2880 & -2880 & -960 & 4800 & 360 & 360 & 1830 & -960 & 1440 & 1440 & 360 & -2880 & 1440 & 1440 & 360 & -2880 \\
-960 & -1770 & 360 & 360 & 4800 & -960 & -2880 & -2880 & -960 & 30 & 360 & 360 & -2880 & 360 & 1440 & 1440 \\
1830 & -960 & 30 & 360 & -960 & 4800 & -960 & -2880 & 30 & -960 & 30 & 360 & 360 & -2880 & 360 & 1440 \\
360 & 30 & -960 & 1830 & -2880 & -960 & 4800 & -960 & 360 & 30 & -960 & 30 & 1440 & 360 & -2880 & 360 \\
360 & 360 & -1770 & -960 & -2880 & -2880 & -960 & 4800 & 360 & 360 & 30 & -960 & 1440 & 1440 & 360 & -2880 \\
-2880 & 360 & 1440 & 1440 & -960 & 30 & 360 & 360 & 4800 & -960 & -2880 & -2880 & -960 & -1770 & 360 & 360 \\
360 & -2880 & 360 & 1440 & 30 & -960 & 30 & 360 & -960 & 4800 & -960 & -2880 & 1830 & -960 & 30 & 360 \\
1440 & 360 & -2880 & 360 & 360 & 30 & -960 & 30 & -2880 & -960 & 4800 & -960 & 360 & 30 & -960 & 1830 \\
1440 & 1440 & 360 & -2880 & 360 & 360 & 30 & -960 & -2880 & -2880 & -960 & 4800 & 360 & 360 & -1770 & -960 \\
-2880 & 360 & 1440 & 1440 & -2880 & 360 & 1440 & 1440 & -960 & 1830 & 360 & 360 & 4800 & -960 & -2880 & -2880 \\
360 & -2880 & 360 & 1440 & 360 & -2880 & 360 & 1440 & -1770 & -960 & 30 & 360 & -960 & 4800 & -960 & -2880 \\
1440 & 360 & -2880 & 360 & 1440 & 360 & -2880 & 360 & 360 & 30 & -960 & -1770 & -2880 & -960 & 4800 & -960 \\
1440 & 1440 & 360 & -2880 & 1440 & 1440 & 360 & -2880 & 360 & 360 & 1830 & -960 & -2880 & -2880 & -960 & 4800
\end{pmatrix}$$

$S = \{1243, 1324, 2134, 2143, 3412, 3421, 4231, 4312\}, \lambda_{max} = 0.076279, \lambda_{min} = -0.044522$

$$H_S = \frac{1}{6 \cdot 5^6} \times \begin{pmatrix}
192 & 912 & 1152 & 1152 & 912 & -1518 & 72 & 72 & 1152 & 72 & -288 & -288 & 1152 & 72 & -288 & -288 \\
912 & 192 & 912 & 1152 & 2082 & 912 & 282 & 72 & 72 & 1152 & 72 & -288 & 72 & 1152 & 72 & -288 \\
1152 & 912 & 192 & 912 & 72 & 282 & 912 & 2082 & -288 & 72 & 1152 & 72 & -288 & 72 & 1152 & 72 \\
1152 & 1152 & 912 & 192 & 72 & 72 & -1518 & 912 & -288 & -288 & 72 & 1152 & -288 & -288 & 72 & 1152 \\
912 & 2082 & 72 & 72 & 192 & 912 & 1152 & 1152 & 912 & 282 & 72 & 72 & 1152 & 72 & -288 & -288 \\
-1518 & 912 & 282 & 72 & 912 & 192 & 912 & 1152 & 282 & 912 & 282 & 72 & 72 & 1152 & 72 & -288 \\
72 & 282 & 912 & -1518 & 1152 & 912 & 192 & 912 & 72 & 282 & 912 & 282 & -288 & 72 & 1152 & 72 \\
72 & 72 & 2082 & 912 & 1152 & 1152 & 912 & 192 & 72 & 72 & 282 & 912 & -288 & -288 & 72 & 1152 \\
1152 & 72 & -288 & -288 & 912 & 282 & 72 & 72 & 192 & 912 & 1152 & 1152 & 912 & 2082 & 72 & 72 \\
72 & 1152 & 72 & -288 & 282 & 912 & 282 & 72 & 912 & 192 & 912 & 1152 & -1518 & 912 & 282 & 72 \\
-288 & 72 & 1152 & 72 & 72 & 282 & 912 & 282 & 1152 & 912 & 192 & 912 & 72 & 282 & 912 & -1518 \\
-288 & -288 & 72 & 1152 & 72 & 72 & 282 & 912 & 1152 & 1152 & 912 & 192 & 72 & 72 & 2082 & 912 \\
1152 & 72 & -288 & -288 & 1152 & 72 & -288 & -288 & 912 & -1518 & 72 & 72 & 192 & 912 & 1152 & 1152 \\
72 & 1152 & 72 & -288 & 72 & 1152 & 72 & -288 & 2082 & 912 & 282 & 72 & 912 & 192 & 912 & 1152 \\
-288 & 72 & 1152 & 72 & -288 & 72 & 1152 & 72 & 72 & 282 & 912 & 2082 & 1152 & 912 & 192 & 912 \\
-288 & -288 & 72 & 1152 & -288 & -288 & 72 & 1152 & 72 & 72 & -1518 & 912 & 1152 & 1152 & 912 & 192
\end{pmatrix}$$

$S = \{1243, 1324, 2134, 2341, 3412, 3421, 4132, 4213\}, \lambda_{max} = 0.161786, \lambda_{min} = -0.174378$

$$H_S = \frac{1}{6 \cdot 5^6} \times \begin{pmatrix}
-96 & 624 & 864 & 864 & 624 & 3288 & 1080 & 1080 & 864 & 2520 & -1152 & -1152 & 864 & 2520 & -1152 & -1152 \\
624 & -96 & 624 & 864 & -3300 & 624 & 6384 & 1080 & -2952 & 864 & 1944 & -1152 & -2952 & 864 & 1944 & -1152 \\
864 & 624 & -96 & 624 & -1512 & -6396 & 624 & 10128 & 0 & -2376 & 864 & 1080 & 0 & -2376 & 864 & 1080 \\
864 & 864 & 624 & -96 & -1512 & -1512 & -10140 & 624 & 0 & 0 & -1512 & 864 & 0 & 0 & -1512 & 864 \\
624 & -3300 & -1512 & -1512 & -96 & 624 & 864 & 864 & 624 & 984 & 1944 & 1944 & 864 & 2520 & -1152 & -1152 \\
3288 & 624 & -6396 & -1512 & 624 & -96 & 624 & 864 & -996 & 624 & 3144 & 1944 & -2952 & 864 & 1944 & -1152 \\
1080 & 6384 & 624 & -10140 & 864 & 624 & -96 & 624 & -2376 & -3156 & 624 & 6384 & 0 & -2376 & 864 & 1080 \\
1080 & 1080 & 10128 & 624 & 864 & 864 & 624 & -96 & -2376 & -2376 & -6396 & 624 & 0 & 0 & -1512 & 864 \\
864 & -2952 & 0 & 0 & 624 & -996 & -2376 & -2376 & -96 & 624 & 864 & 864 & 624 & 48 & 2520 & 2520 \\
2520 & 864 & -2376 & 0 & 984 & 624 & -3156 & -2376 & 624 & -96 & 624 & 864 & -60 & 624 & 984 & 2520 \\
-1152 & 1944 & 864 & -1512 & 1944 & 3144 & 624 & -6396 & 864 & 624 & -96 & 624 & -2952 & -996 & 624 & 3288 \\
-1152 & -1152 & 1080 & 864 & 1944 & 1944 & 6384 & 624 & 864 & 864 & 624 & -96 & -2952 & -2952 & -3300 & 624 \\
864 & -2952 & 0 & 0 & 864 & -2952 & 0 & 0 & 624 & -60 & -2952 & -2952 & -96 & 624 & 864 & 864 \\
2520 & 864 & -2376 & 0 & 2520 & 864 & -2376 & 0 & 48 & 624 & -996 & -2952 & 624 & -96 & 624 & 864 \\
-1152 & 1944 & 864 & -1512 & -1152 & 1944 & 864 & -1512 & 2520 & 984 & 624 & -3300 & 864 & 624 & -96 & 624 \\
-1152 & -1152 & 1080 & 864 & -1152 & -1152 & 1080 & 864 & 2520 & 2520 & 3288 & 624 & 864 & 864 & 624 & -96
\end{pmatrix}$$

$S = \{1243, 1324, 2134, 2413, 3142, 3421, 4231, 4312\}, \lambda_{max} = 0.046180, \lambda_{min} = -0.136488$

$$H_S = \frac{1}{6 \cdot 5^6} \times \begin{pmatrix}
-4416 & 624 & 2304 & 2304 & 624 & 264 & 144 & 144 & 2304 & 144 & -576 & -576 & 2304 & 144 & -576 & -576 \\
624 & -4416 & 624 & 2304 & 264 & 624 & 264 & 144 & 144 & 2304 & 144 & -576 & 144 & 2304 & 144 & -576 \\
2304 & 624 & -4416 & 624 & 144 & 264 & 624 & 264 & -576 & 144 & 2304 & 144 & -576 & 144 & 2304 & 144 \\
2304 & 2304 & 624 & -4416 & 144 & 144 & 264 & 624 & -576 & -576 & 144 & 2304 & -576 & -576 & 144 & 2304 \\
624 & 264 & 144 & 144 & -4416 & 624 & 2304 & 2304 & 624 & 264 & 144 & 144 & 2304 & 144 & -576 & -576 \\
264 & 624 & 264 & 144 & 624 & -4416 & 624 & 2304 & 264 & 624 & 264 & 144 & 144 & 2304 & 144 & -576 \\
144 & 264 & 624 & 264 & 2304 & 624 & -4416 & 624 & 144 & 264 & 624 & 264 & -576 & 144 & 2304 & 144 \\
144 & 144 & 264 & 624 & 2304 & 2304 & 624 & -4416 & 144 & 144 & 264 & 624 & -576 & -576 & 144 & 2304 \\
2304 & 144 & -576 & -576 & 624 & 264 & 144 & 144 & -4416 & 624 & 2304 & 2304 & 624 & 264 & 144 & 144 \\
144 & 2304 & 144 & -576 & 264 & 624 & 264 & 144 & 624 & -4416 & 624 & 2304 & 264 & 624 & 264 & 144 \\
-576 & 144 & 2304 & 144 & 144 & 264 & 624 & 264 & 2304 & 624 & -4416 & 624 & 144 & 264 & 624 & 264 \\
-576 & -576 & 144 & 2304 & 144 & 144 & 264 & 624 & 2304 & 2304 & 624 & -4416 & 144 & 144 & 264 & 624 \\
2304 & 144 & -576 & -576 & 2304 & 144 & -576 & -576 & 624 & 264 & 144 & 144 & -4416 & 624 & 2304 & 2304 \\
144 & 2304 & 144 & -576 & 144 & 2304 & 144 & -576 & 264 & 624 & 264 & 144 & 624 & -4416 & 624 & 2304 \\
-576 & 144 & 2304 & 144 & -576 & 144 & 2304 & 144 & 144 & 264 & 624 & 264 & 2304 & 624 & -4416 & 624 \\
-576 & -576 & 144 & 2304 & -576 & -576 & 144 & 2304 & 144 & 144 & 264 & 624 & 2304 & 2304 & 624 & -4416
\end{pmatrix}$$

$S = \{1243, 1324, 2134, 2413, 3241, 3421, 4132, 4312\}, \lambda_{max} = 0.070321, \lambda_{min} = -0.196705$

$$H_S = \frac{1}{6 \cdot 5^6} \times \begin{pmatrix}
-3552 & 408 & 1728 & 1728 & 1488 & -1302 & 3168 & 3168 & 3168 & -72 & -1152 & -1152 & 3168 & -72 & -1152 & -1152 \\
408 & -3552 & 408 & 1728 & 1398 & 1488 & -2202 & 3168 & -72 & 3168 & -72 & -1152 & -72 & 3168 & -72 & -1152 \\
1728 & 408 & -3552 & 408 & -4032 & 2298 & 1488 & -1302 & -1152 & -72 & 3168 & -72 & -1152 & -72 & 3168 & -72 \\
1728 & 1728 & 408 & -3552 & -4032 & -4032 & 1398 & 1488 & -1152 & -1152 & -72 & 3168 & -1152 & -1152 & -72 & 3168 \\
1488 & 1398 & -4032 & -4032 & -3552 & 408 & 1728 & 1728 & 1488 & -1302 & 3168 & 3168 & 3168 & -72 & -1152 & -1152 \\
-1302 & 1488 & 2298 & -4032 & 408 & -3552 & 408 & 1728 & 1398 & 1488 & -2202 & 3168 & -72 & 3168 & -72 & -1152 \\
3168 & -2202 & 1488 & 1398 & 1728 & 408 & -3552 & 408 & -4032 & 2298 & 1488 & -1302 & -1152 & -72 & 3168 & -72 \\
3168 & 3168 & -1302 & 1488 & 1728 & 1728 & 408 & -3552 & -4032 & -4032 & 1398 & 1488 & -1152 & -1152 & -72 & 3168 \\
3168 & -72 & -1152 & -1152 & 1488 & 1398 & -4032 & -4032 & -3552 & 408 & 1728 & 1728 & 1488 & -1302 & 3168 & 3168 \\
-72 & 3168 & -72 & -1152 & -1302 & 1488 & 2298 & -4032 & 408 & -3552 & 408 & 1728 & 1398 & 1488 & -2202 & 3168 \\
-1152 & -72 & 3168 & -72 & 3168 & -2202 & 1488 & 1398 & 1728 & 408 & -3552 & 408 & -4032 & 2298 & 1488 & -1302 \\
-1152 & -1152 & -72 & 3168 & 3168 & 3168 & -1302 & 1488 & 1728 & 1728 & 408 & -3552 & -4032 & -4032 & 1398 & 1488 \\
3168 & -72 & -1152 & -1152 & 3168 & -72 & -1152 & -1152 & 1488 & 1398 & -4032 & -4032 & -3552 & 408 & 1728 & 1728 \\
-72 & 3168 & -72 & -1152 & -72 & 3168 & -72 & -1152 & -1302 & 1488 & 2298 & -4032 & 408 & -3552 & 408 & 1728 \\
-1152 & -72 & 3168 & -72 & -1152 & -72 & 3168 & -72 & 3168 & -2202 & 1488 & 1398 & 1728 & 408 & -3552 & 408 \\
-1152 & -1152 & -72 & 3168 & -1152 & -1152 & -72 & 3168 & 3168 & 3168 & -1302 & 1488 & 1728 & 1728 & 408 & -3552
\end{pmatrix}$$

$S = \{1243, 1324, 2143, 2314, 3412, 3421, 4132, 4231\}, \lambda_{max} = 0.091988, \lambda_{min} = -0.108256$

$$H_S = \frac{1}{6 \cdot 5^6} \times \begin{pmatrix}
-960 & -240 & 0 & 0 & 840 & 2910 & 0 & 0 & 1440 & 360 & 0 & 0 & 1440 & 360 & 0 & 0 \\
-240 & -960 & -240 & 0 & -2490 & 840 & 4710 & 0 & 360 & 1440 & 360 & 0 & 360 & 1440 & 360 & 0 \\
0 & -240 & -960 & -240 & 0 & -4290 & 840 & 6510 & 0 & 360 & 1440 & 360 & 0 & 360 & 1440 & 360 \\
0 & 0 & -240 & -960 & 0 & 0 & -6090 & 840 & 0 & 0 & 360 & 1440 & 0 & 0 & 360 & 1440 \\
840 & -2490 & 0 & 0 & -960 & -240 & 0 & 0 & 840 & 210 & 0 & 0 & 1440 & 360 & 0 & 0 \\
2910 & 840 & -4290 & 0 & -240 & -960 & -240 & 0 & 210 & 840 & 210 & 0 & 360 & 1440 & 360 & 0 \\
0 & 4710 & 840 & -6090 & 0 & -240 & -960 & -240 & 0 & 210 & 840 & 210 & 0 & 360 & 1440 & 360 \\
0 & 0 & 6510 & 840 & 0 & 0 & -240 & -960 & 0 & 0 & 210 & 840 & 0 & 0 & 360 & 1440 \\
1440 & 360 & 0 & 0 & 840 & 210 & 0 & 0 & -960 & -240 & 0 & 0 & 840 & -2490 & 0 & 0 \\
360 & 1440 & 360 & 0 & 210 & 840 & 210 & 0 & -240 & -960 & -240 & 0 & 2910 & 840 & -4290 & 0 \\
0 & 360 & 1440 & 360 & 0 & 210 & 840 & 210 & 0 & -240 & -960 & -240 & 0 & 4710 & 840 & -6090 \\
0 & 0 & 360 & 1440 & 0 & 0 & 210 & 840 & 0 & 0 & -240 & -960 & 0 & 0 & 6510 & 840 \\
1440 & 360 & 0 & 0 & 1440 & 360 & 0 & 0 & 840 & 2910 & 0 & 0 & -960 & -240 & 0 & 0 \\
360 & 1440 & 360 & 0 & 360 & 1440 & 360 & 0 & -2490 & 840 & 4710 & 0 & -240 & -960 & -240 & 0 \\
0 & 360 & 1440 & 360 & 0 & 360 & 1440 & 360 & 0 & -4290 & 840 & 6510 & 0 & -240 & -960 & -240 \\
0 & 0 & 360 & 1440 & 0 & 0 & 360 & 1440 & 0 & 0 & -6090 & 840 & 0 & 0 & -240 & -960
\end{pmatrix}$$

$S = \{1243, 1324, 2143, 2431, 3214, 3421, 4132, 4312\}, \lambda_{max} = 0.216427, \lambda_{min} = -0.255944$

$$H_S = \frac{1}{6 \cdot 5^6} \times \begin{pmatrix}
-96 & 624 & 864 & 864 & 624 & -3840 & 2088 & 2088 & 864 & 2088 & 0 & 0 & 864 & 2088 & 0 & 0 \\
624 & -96 & 624 & 864 & 3828 & 624 & -5496 & 2088 & -2520 & 864 & 1224 & 0 & -2520 & 864 & 1224 & 0 \\
864 & 624 & -96 & 624 & -2520 & 5484 & 624 & -6000 & -1152 & -1656 & 864 & 648 & -1152 & -1656 & 864 & 648 \\
864 & 864 & 624 & -96 & -2520 & -2520 & 5988 & 624 & -1152 & -1152 & -1080 & 864 & -1152 & -1152 & -1080 & 864 \\
624 & 3828 & -2520 & -2520 & -96 & 624 & 864 & 864 & 624 & -5496 & 1224 & 1224 & 864 & 2088 & 0 & 0 \\
-3840 & 624 & 5484 & -2520 & 624 & -96 & 624 & 864 & 5484 & 624 & -7656 & 1224 & -2520 & 864 & 1224 & 0 \\
2088 & -5496 & 624 & 5988 & 864 & 624 & -96 & 624 & -1656 & 7644 & 624 & -9096 & -1152 & -1656 & 864 & 648 \\
2088 & 2088 & -6000 & 624 & 864 & 864 & 624 & -96 & -1656 & -1656 & 9084 & 624 & -1152 & -1152 & -1080 & 864 \\
864 & -2520 & -1152 & -1152 & 624 & 5484 & -1656 & -1656 & -96 & 624 & 864 & 864 & 624 & -6000 & 648 & 648 \\
2088 & 864 & -1656 & -1152 & -5496 & 624 & 7644 & -1656 & 624 & -96 & 624 & 864 & 5988 & 624 & -9096 & 648 \\
0 & 1224 & 864 & -1080 & 1224 & -7656 & 624 & 9084 & 864 & 624 & -96 & 624 & -1080 & 9084 & 624 & -11760 \\
0 & 0 & 648 & 864 & 1224 & 1224 & -9096 & 624 & 864 & 864 & 624 & -96 & -1080 & -1080 & 11748 & 624 \\
864 & -2520 & -1152 & -1152 & 864 & -2520 & -1152 & -1152 & 624 & 5988 & -1080 & -1080 & -96 & 624 & 864 & 864 \\
2088 & 864 & -1656 & -1152 & 2088 & 864 & -1656 & -1152 & -6000 & 624 & 9084 & -1080 & 624 & -96 & 624 & 864 \\
0 & 1224 & 864 & -1080 & 0 & 1224 & 864 & -1080 & 648 & -9096 & 624 & 11748 & 864 & 624 & -96 & 624 \\
0 & 0 & 648 & 864 & 0 & 0 & 648 & 864 & 648 & 648 & -11760 & 624 & 864 & 864 & 624 & -96
\end{pmatrix}$$

$S = \{1243, 1324, 2314, 2413, 3142, 3421, 4132, 4231\}, \lambda_{max} = 0.034918, \lambda_{min} = -0.180265$

$$H_S = \frac{1}{6 \cdot 5^6} \times \begin{pmatrix}
-5568 & -528 & 1152 & 1152 & 552 & 4692 & 72 & 72 & 2592 & 432 & -288 & -288 & 2592 & 432 & -288 & -288 \\
-528 & -5568 & -528 & 1152 & -4308 & 552 & 4692 & 72 & 432 & 2592 & 432 & -288 & 432 & 2592 & 432 & -288 \\
1152 & -528 & -5568 & -528 & 72 & -4308 & 552 & 4692 & -288 & 432 & 2592 & 432 & -288 & 432 & 2592 & 432 \\
1152 & 1152 & -528 & -5568 & 72 & 72 & -4308 & 552 & -288 & -288 & 432 & 2592 & -288 & -288 & 432 & 2592 \\
552 & -4308 & 72 & 72 & -5568 & -528 & 1152 & 1152 & 552 & 192 & 72 & 72 & 2592 & 432 & -288 & -288 \\
4692 & 552 & -4308 & 72 & -528 & -5568 & -528 & 1152 & 192 & 552 & 192 & 72 & 432 & 2592 & 432 & -288 \\
72 & 4692 & 552 & -4308 & 1152 & -528 & -5568 & -528 & 72 & 192 & 552 & 192 & -288 & 432 & 2592 & 432 \\
72 & 72 & 4692 & 552 & 1152 & 1152 & -528 & -5568 & 72 & 72 & 192 & 552 & -288 & -288 & 432 & 2592 \\
2592 & 432 & -288 & -288 & 552 & 192 & 72 & 72 & -5568 & -528 & 1152 & 1152 & 552 & -4308 & 72 & 72 \\
432 & 2592 & 432 & -288 & 192 & 552 & 192 & 72 & -528 & -5568 & -528 & 1152 & 4692 & 552 & -4308 & 72 \\
-288 & 432 & 2592 & 432 & 72 & 192 & 552 & 192 & 1152 & -528 & -5568 & -528 & 72 & 4692 & 552 & -4308 \\
-288 & -288 & 432 & 2592 & 72 & 72 & 192 & 552 & 1152 & 1152 & -528 & -5568 & 72 & 72 & 4692 & 552 \\
2592 & 432 & -288 & -288 & 2592 & 432 & -288 & -288 & 552 & 4692 & 72 & 72 & -5568 & -528 & 1152 & 1152 \\
432 & 2592 & 432 & -288 & 432 & 2592 & 432 & -288 & -4308 & 552 & 4692 & 72 & -528 & -5568 & -528 & 1152 \\
-288 & 432 & 2592 & 432 & -288 & 432 & 2592 & 432 & 72 & -4308 & 552 & 4692 & 1152 & -528 & -5568 & -528 \\
-288 & -288 & 432 & 2592 & -288 & -288 & 432 & 2592 & 72 & 72 & -4308 & 552 & 1152 & 1152 & -528 & -5568
\end{pmatrix}$$

$S = \{1243, 1324, 2314, 2431, 3142, 3412, 4123, 4231\}, \lambda_{max} = 0.166184, \lambda_{min} = -0.217873$

$$
H_S = \frac{1}{6 \cdot 5^6} \times \begin{pmatrix}
-2112 & -312 & 288 & 288 & -312 & 9282 & -576 & -576 & 288 & 1584 & -288 & -288 & 288 & 1584 & -288 & -288 \\
-312 & -2112 & -312 & 288 & -9006 & -312 & 7878 & -576 & -1008 & 288 & 2448 & -288 & -1008 & 288 & 2448 & -288 \\
288 & -312 & -2112 & -312 & 1152 & -7602 & -312 & 6042 & 864 & -1872 & 288 & 3024 & 864 & -1872 & 288 & 3024 \\
288 & 288 & -312 & -2112 & 1152 & 1152 & -5766 & -312 & 864 & 864 & -2448 & 288 & 864 & 864 & -2448 & 288 \\
-312 & -9006 & 1152 & 1152 & -2112 & -312 & 288 & 288 & -312 & 7878 & -1152 & -1152 & 288 & 1584 & -288 & -288 \\
9282 & -312 & -7602 & 1152 & -312 & -2112 & -312 & 288 & -7602 & -312 & 5538 & -1152 & -1008 & 288 & 2448 & -288 \\
-576 & 7878 & -312 & -5766 & 288 & -312 & -2112 & -312 & 1728 & -5262 & -312 & 2478 & 864 & -1872 & 288 & 3024 \\
-576 & -576 & 6042 & -312 & 288 & 288 & -312 & -2112 & 1728 & 1728 & -2202 & -312 & 864 & 864 & -2448 & 288 \\
288 & -1008 & 864 & 864 & -312 & -7602 & 1728 & 1728 & -2112 & -312 & 288 & 288 & -312 & 7122 & -2016 & -2016 \\
1584 & 288 & -1872 & 864 & 7878 & -312 & -5262 & 1728 & -312 & -2112 & -312 & 288 & -6846 & -312 & 4278 & -2016 \\
-288 & 2448 & 288 & -2448 & -1152 & 5538 & -312 & -2202 & 288 & -312 & -2112 & -312 & 2592 & -4002 & -312 & 282 \\
-288 & -288 & 3024 & 288 & -1152 & -1152 & 2478 & -312 & 288 & 288 & -312 & -2112 & 2592 & 2592 & -6 & -312 \\
288 & -1008 & 864 & 864 & 288 & -1008 & 864 & 864 & -312 & -6846 & 2592 & 2592 & -2112 & -312 & 288 & 288 \\
1584 & 288 & -1872 & 864 & 1584 & 288 & -1872 & 864 & 7122 & -312 & -4002 & 2592 & -312 & -2112 & -312 & 288 \\
-288 & 2448 & 288 & -2448 & -288 & 2448 & 288 & -2448 & -2016 & 4278 & -312 & -6 & 288 & -312 & -2112 & -312 \\
-288 & -288 & 3024 & 288 & -288 & -288 & 3024 & 288 & -2016 & -2016 & 282 & -312 & 288 & 288 & -312 & -2112
\end{pmatrix}
$$

$S = \{1243, 1324, 2314, 2431, 3142, 3421, 4132, 4213\}, \lambda_{max} = 0.076228, \lambda_{min} = -0.225154$

$$
H_S = \frac{1}{6 \cdot 5^6} \times \begin{pmatrix}
-4704 & 336 & 2016 & 2016 & 336 & 3126 & -144 & -144 & 2016 & 3456 & -864 & -864 & 2016 & 3456 & -864 & -864 \\
336 & -4704 & 336 & 2016 & -3174 & 336 & 3126 & -144 & -3744 & 2016 & 3456 & -864 & -3744 & 2016 & 3456 & -864 \\
2016 & 336 & -4704 & 336 & -144 & -3174 & 336 & 3126 & -864 & -3744 & 2016 & 3456 & -864 & -3744 & 2016 & 3456 \\
2016 & 2016 & 336 & -4704 & -144 & -144 & -3174 & 336 & -864 & -864 & -3744 & 2016 & -864 & -864 & -3744 & 2016 \\
336 & -3174 & -144 & -144 & -4704 & 336 & 2016 & 2016 & 336 & -2274 & -144 & -144 & 2016 & 3456 & -864 & -864 \\
3126 & 336 & -3174 & -144 & 336 & -4704 & 336 & 2016 & 2226 & 336 & -2274 & -144 & -3744 & 2016 & 3456 & -864 \\
-144 & 3126 & 336 & -3174 & 2016 & 336 & -4704 & 336 & -144 & 2226 & 336 & -2274 & -864 & -3744 & 2016 & 3456 \\
-144 & -144 & 3126 & 336 & 2016 & 2016 & 336 & -4704 & -144 & -144 & 2226 & 336 & -864 & -864 & -3744 & 2016 \\
2016 & -3744 & -864 & -864 & 336 & 2226 & -144 & -144 & -4704 & 336 & 2016 & 2016 & 336 & -5874 & -144 & -144 \\
3456 & 2016 & -3744 & -864 & -2274 & 336 & 2226 & -144 & 336 & -4704 & 336 & 2016 & 5826 & 336 & -5874 & -144 \\
-864 & 3456 & 2016 & -3744 & -144 & -2274 & 336 & 2226 & 2016 & 336 & -4704 & 336 & -144 & 5826 & 336 & -5874 \\
-864 & -864 & 3456 & 2016 & -144 & -144 & -2274 & 336 & 2016 & 2016 & 336 & -4704 & -144 & -144 & 5826 & 336 \\
2016 & -3744 & -864 & -864 & 2016 & -3744 & -864 & -864 & 336 & 5826 & -144 & -144 & -4704 & 336 & 2016 & 2016 \\
3456 & 2016 & -3744 & -864 & 3456 & 2016 & -3744 & -864 & -5874 & 336 & 5826 & -144 & 336 & -4704 & 336 & 2016 \\
-864 & 3456 & 2016 & -3744 & -864 & 3456 & 2016 & -3744 & -144 & -5874 & 336 & 5826 & 2016 & 336 & -4704 & 336 \\
-864 & -864 & 3456 & 2016 & -864 & -864 & 3456 & 2016 & -144 & -144 & -5874 & 336 & 2016 & 2016 & 336 & -4704
\end{pmatrix}
$$

$S = \{1243, 1324, 2314, 2431, 3241, 3412, 4123, 4132\}, \lambda_{max} = 0.141170, \lambda_{min} = -0.177243$

$$
H_S = \frac{1}{6 \cdot 5^6} \times \begin{pmatrix}
-1248 & -528 & -288 & -288 & 552 & 7716 & 2448 & 2448 & 1152 & 1368 & -864 & -864 & 1152 & 1368 & -864 & -864 \\
-528 & -1248 & -528 & -288 & -7872 & 552 & 5412 & 2448 & -1224 & 1152 & 2232 & -864 & -1224 & 1152 & 2232 & -864 \\
-288 & -528 & -1248 & -528 & -3024 & -5568 & 552 & 4476 & 288 & -2088 & 1152 & 2808 & 288 & -2088 & 1152 & 2808 \\
-288 & -288 & -528 & -1248 & -3024 & -3024 & -4632 & 552 & 288 & 288 & -2664 & 1152 & 288 & 288 & -2664 & 1152 \\
552 & -7872 & -3024 & -3024 & -1248 & -528 & -288 & -288 & 552 & 6312 & 1872 & 1872 & 1152 & 1368 & -864 & -864 \\
7716 & 552 & -5568 & -3024 & -528 & -1248 & -528 & -288 & -6468 & 552 & 3072 & 1872 & -1224 & 1152 & 2232 & -864 \\
2448 & 5412 & 552 & -4632 & -288 & -528 & -1248 & -528 & -2448 & -3228 & 552 & 912 & 288 & -2088 & 1152 & 2808 \\
2448 & 2448 & 4476 & 552 & -288 & -288 & -528 & -1248 & -2448 & -2448 & -1068 & 552 & 288 & 288 & -2664 & 1152 \\
1152 & -1224 & 288 & 288 & 552 & -6468 & -2448 & -2448 & -1248 & -528 & -288 & -288 & 552 & 5556 & 1008 & 1008 \\
1368 & 1152 & -2088 & 288 & 6312 & 552 & -3228 & -2448 & -528 & -1248 & -528 & -288 & -5712 & 552 & 1812 & 1008 \\
-864 & 2232 & 1152 & -2664 & 1872 & 3072 & 552 & -1068 & -288 & -528 & -1248 & -528 & -1584 & -1968 & 552 & -1284 \\
-864 & -864 & 2808 & 1152 & 1872 & 1872 & 912 & 552 & -288 & -288 & -528 & -1248 & -1584 & -1584 & 1128 & 552 \\
1152 & -1224 & 288 & 288 & 1152 & -1224 & 288 & 288 & 552 & -5712 & -1584 & -1584 & -1248 & -528 & -288 & -288 \\
1368 & 1152 & -2088 & 288 & 1368 & 1152 & -2088 & 288 & 5556 & 552 & -1968 & -1584 & -528 & -1248 & -528 & -288 \\
-864 & 2232 & 1152 & -2664 & -864 & 2232 & 1152 & -2664 & 1008 & 1812 & 552 & 1128 & -288 & -528 & -1248 & -528 \\
-864 & -864 & 2808 & 1152 & -864 & -864 & 2808 & 1152 & 1008 & 1008 & -1284 & 552 & -288 & -288 & -528 & -1248
\end{pmatrix}
$$

$S = \{1243, 1324, 2341, 2431, 3214, 3412, 4123, 4132\}, \lambda_{max} = 0.197456, \lambda_{min} = -0.114637$

$$
H_S = \frac{1}{6 \cdot 5^6} \times \begin{pmatrix}
2208 & -312 & -1152 & -1152 & -312 & 7122 & 2664 & 2664 & -1152 & 2664 & -288 & -288 & -1152 & 2664 & -288 & -288 \\
-312 & 2208 & -312 & -1152 & -7386 & -312 & 5358 & 2664 & -2808 & -1152 & 2088 & -288 & -2808 & -1152 & 2088 & -288 \\
-1152 & -312 & 2208 & -312 & -2808 & -5622 & -312 & 4962 & 864 & -2232 & -1152 & 1224 & 864 & -2232 & -1152 & 1224 \\
-1152 & -1152 & -312 & 2208 & -2808 & -2808 & -5226 & -312 & 864 & 864 & -1368 & -1152 & 864 & 864 & -1368 & -1152 \\
-312 & -7386 & -2808 & -2808 & 2208 & -312 & -1152 & -1152 & -312 & 5358 & 2088 & 2088 & -1152 & 2664 & -288 & -288 \\
7122 & -312 & -5622 & -2808 & -312 & 2208 & -312 & -1152 & -5622 & -312 & 3018 & 2088 & -2808 & -1152 & 2088 & -288 \\
2664 & 5358 & -312 & -5226 & -1152 & -312 & 2208 & -312 & -2232 & -3282 & -312 & 1758 & 864 & -2232 & -1152 & 1224 \\
2664 & 2664 & 4962 & -312 & -1152 & -1152 & -312 & 2208 & -2232 & -2232 & -2022 & -312 & 864 & 864 & -1368 & -1152 \\
-1152 & -2808 & 864 & 864 & -312 & -5622 & -2232 & -2232 & 2208 & -312 & -1152 & -1152 & -312 & 4962 & 1224 & 1224 \\
2664 & -1152 & -2232 & 864 & 5358 & -312 & -3282 & -2232 & -312 & 2208 & -312 & -1152 & -5226 & -312 & 1758 & 1224 \\
-288 & 2088 & -1152 & -1368 & 2088 & 3018 & -312 & -2022 & -1152 & -312 & 2208 & -312 & -1368 & -2022 & -312 & -798 \\
-288 & -288 & 1224 & -1152 & 2088 & 2088 & 1758 & -312 & -1152 & -1152 & -312 & 2208 & -1368 & -1368 & 534 & -312 \\
-1152 & -2808 & 864 & 864 & -1152 & -2808 & 864 & 864 & -312 & -5226 & -1368 & -1368 & 2208 & -312 & -1152 & -1152 \\
2664 & -1152 & -2232 & 864 & 2664 & -1152 & -2232 & 864 & 4962 & -312 & -2022 & -1368 & -312 & 2208 & -312 & -1152 \\
-288 & 2088 & -1152 & -1368 & -288 & 2088 & -1152 & -1368 & 1224 & 1758 & -312 & 534 & -1152 & -312 & 2208 & -312 \\
-288 & -288 & 1224 & -1152 & -288 & -288 & 1224 & -1152 & 1224 & 1224 & -798 & -312 & -1152 & -1152 & -312 & 2208
\end{pmatrix}
$$

$S = \{1243, 1342, 2134, 2431, 3124, 3421, 4213, 4312\}, \lambda_{max} = 0.122145, \lambda_{min} = -0.136488$

$$H_S = \frac{1}{6\cdot 5^6} \times \begin{pmatrix}
-2688 & 2352 & 4032 & 4032 & 192 & -168 & -288 & -288 & 1152 & -1008 & -1728 & -1728 & 1152 & -1008 & -1728 & -1728 \\
2352 & -2688 & 2352 & 4032 & -168 & 192 & -168 & -288 & -1008 & 1152 & -1008 & -1728 & -1008 & 1152 & -1008 & -1728 \\
4032 & 2352 & -2688 & 2352 & -288 & -168 & 192 & -168 & -1728 & -1008 & 1152 & -1008 & -1728 & -1008 & 1152 & -1008 \\
4032 & 4032 & 2352 & -2688 & -288 & -288 & -168 & 192 & -1728 & -1728 & -1008 & 1152 & -1728 & -1728 & -1008 & 1152 \\
192 & -168 & -288 & -288 & -2688 & 2352 & 4032 & 4032 & 192 & -168 & -288 & -288 & 1152 & -1008 & -1728 & -1728 \\
-168 & 192 & -168 & -288 & 2352 & -2688 & 2352 & 4032 & -168 & 192 & -168 & -288 & -1008 & 1152 & -1008 & -1728 \\
-288 & -168 & 192 & -168 & 4032 & 2352 & -2688 & 2352 & -288 & -168 & 192 & -168 & -1728 & -1008 & 1152 & -1008 \\
-288 & -288 & -168 & 192 & 4032 & 4032 & 2352 & -2688 & -288 & -288 & -168 & 192 & -1728 & -1728 & -1008 & 1152 \\
1152 & -1008 & -1728 & -1728 & 192 & -168 & -288 & -288 & -2688 & 2352 & 4032 & 4032 & 192 & -168 & -288 & -288 \\
-1008 & 1152 & -1008 & -1728 & -168 & 192 & -168 & -288 & 2352 & -2688 & 2352 & 4032 & -168 & 192 & -168 & -288 \\
-1728 & -1008 & 1152 & -1008 & -288 & -168 & 192 & -168 & 4032 & 2352 & -2688 & 2352 & -288 & -168 & 192 & -168 \\
-1728 & -1728 & -1008 & 1152 & -288 & -288 & -168 & 192 & 4032 & 4032 & 2352 & -2688 & -288 & -288 & -168 & 192 \\
1152 & -1008 & -1728 & -1728 & 1152 & -1008 & -1728 & -1728 & 192 & -168 & -288 & -288 & -2688 & 2352 & 4032 & 4032 \\
-1008 & 1152 & -1008 & -1728 & -1008 & 1152 & -1008 & -1728 & -168 & 192 & -168 & -288 & 2352 & -2688 & 2352 & 4032 \\
-1728 & -1008 & 1152 & -1008 & -1728 & -1008 & 1152 & -1008 & -288 & -168 & 192 & -168 & 4032 & 2352 & -2688 & 2352 \\
-1728 & -1728 & -1008 & 1152 & -1728 & -1728 & -1008 & 1152 & -288 & -288 & -168 & 192 & 4032 & 4032 & 2352 & -2688
\end{pmatrix}$$

$S = \{1243, 1342, 2134, 2431, 3214, 3421, 4123, 4312\}, \lambda_{max} = 0.104581, \lambda_{min} = -0.046452$

$$H_S = \frac{1}{6\cdot 5^6} \times \begin{pmatrix}
768 & 1488 & 1728 & 1728 & 408 & -762 & 1008 & 1008 & 288 & -792 & -1152 & -1152 & 288 & -792 & -1152 & -1152 \\
1488 & 768 & 1488 & 1728 & 318 & 408 & -1122 & 1008 & -792 & 288 & -792 & -1152 & -792 & 288 & -792 & -1152 \\
1728 & 1488 & 768 & 1488 & -1872 & 678 & 408 & -762 & -1152 & -792 & 288 & -792 & -1152 & -792 & 288 & -792 \\
1728 & 1728 & 1488 & 768 & -1872 & -1872 & 318 & 408 & -1152 & -1152 & -792 & 288 & -1152 & -1152 & -792 & 288 \\
408 & 318 & -1872 & -1872 & 768 & 1488 & 1728 & 1728 & 408 & -222 & -432 & -432 & 288 & -792 & -1152 & -1152 \\
-762 & 408 & 678 & -1872 & 1488 & 768 & 1488 & 1728 & -222 & 408 & -222 & -432 & -792 & 288 & -792 & -1152 \\
1008 & -1122 & 408 & 318 & 1728 & 1488 & 768 & 1488 & -432 & -222 & 408 & -222 & -1152 & -792 & 288 & -792 \\
1008 & 1008 & -762 & 408 & 1728 & 1728 & 1488 & 768 & -432 & -432 & -222 & 408 & -1152 & -1152 & -792 & 288 \\
288 & -792 & -1152 & -1152 & 408 & -222 & -432 & -432 & 768 & 1488 & 1728 & 1728 & 408 & 318 & -1872 & -1872 \\
-792 & 288 & -792 & -1152 & -222 & 408 & -222 & -432 & 1488 & 768 & 1488 & 1728 & -762 & 408 & 678 & -1872 \\
-1152 & -792 & 288 & -792 & -432 & -222 & 408 & -222 & 1728 & 1488 & 768 & 1488 & 1008 & -1122 & 408 & 318 \\
-1152 & -1152 & -792 & 288 & -432 & -432 & -222 & 408 & 1728 & 1728 & 1488 & 768 & 1008 & 1008 & -762 & 408 \\
288 & -792 & -1152 & -1152 & 288 & -792 & -1152 & -1152 & 408 & -762 & 1008 & 1008 & 768 & 1488 & 1728 & 1728 \\
-792 & 288 & -792 & -1152 & -792 & 288 & -792 & -1152 & 318 & 408 & -1122 & 1008 & 1488 & 768 & 1488 & 1728 \\
-1152 & -792 & 288 & -792 & -1152 & -792 & 288 & -792 & -1872 & 678 & 408 & -762 & 1728 & 1488 & 768 & 1488 \\
-1152 & -1152 & -792 & 288 & -1152 & -1152 & -792 & 288 & -1872 & -1872 & 318 & 408 & 1728 & 1728 & 1488 & 768
\end{pmatrix}$$

$S = \{1243, 1342, 2314, 2431, 3124, 3412, 4123, 4231\}, \lambda_{max} = 0.221432, \lambda_{min} = -0.261595$

$$H_S = \frac{1}{6\cdot 5^6} \times \begin{pmatrix}
-1248 & 552 & 1152 & 1152 & -528 & 10416 & -792 & -792 & -288 & -2592 & -864 & -864 & -288 & -2592 & -864 & -864 \\
552 & -1248 & 552 & 1152 & -10572 & -528 & 9012 & -792 & 2016 & -288 & -1728 & -864 & 2016 & -288 & -1728 & -864 \\
1152 & 552 & -1248 & 552 & 936 & -9168 & -528 & 7176 & 288 & 1152 & -288 & -1152 & 288 & 1152 & -288 & -1152 \\
1152 & 1152 & 552 & -1248 & 936 & 936 & -7332 & -528 & 288 & 288 & 576 & -288 & 288 & 288 & 576 & -288 \\
-528 & -10572 & 936 & 936 & -1248 & 552 & 1152 & 1152 & -528 & 9912 & -1368 & -1368 & -288 & -2592 & -864 & -864 \\
10416 & -528 & -9168 & 936 & 552 & -1248 & 552 & 1152 & -10068 & -528 & 7572 & -1368 & 2016 & -288 & -1728 & -864 \\
-792 & 9012 & -528 & -7332 & 1152 & 552 & -1248 & 552 & 1512 & -7728 & -528 & 4512 & 288 & 1152 & -288 & -1152 \\
-792 & -792 & 7176 & -528 & 1152 & 1152 & 552 & -1248 & 1512 & 1512 & -4668 & -528 & 288 & 288 & 576 & -288 \\
-288 & 2016 & 288 & 288 & -528 & -10068 & 1512 & 1512 & -1248 & 552 & 1152 & 1152 & -528 & 8256 & -2232 & -2232 \\
-2592 & -288 & 1152 & 288 & 9912 & -528 & -7728 & 1512 & 552 & -1248 & 552 & 1152 & -8412 & -528 & 5412 & -2232 \\
-864 & -1728 & -288 & 576 & -1368 & 7572 & -528 & -4668 & 1152 & 552 & -1248 & 552 & 2376 & -5568 & -528 & 1416 \\
-864 & -864 & -1152 & -288 & -1368 & -1368 & 4512 & -528 & 1152 & 1152 & 552 & -1248 & 2376 & 2376 & -1572 & -528 \\
-288 & 2016 & 288 & 288 & -288 & 2016 & 288 & 288 & -528 & -8412 & 2376 & 2376 & -1248 & 552 & 1152 & 1152 \\
-2592 & -288 & 1152 & 288 & -2592 & -288 & 1152 & 288 & 8256 & -528 & -5568 & 2376 & 552 & -1248 & 552 & 1152 \\
-864 & -1728 & -288 & 576 & -864 & -1728 & -288 & 576 & -2232 & 5412 & -528 & -1572 & 1152 & 552 & -1248 & 552 \\
-864 & -864 & -1152 & -288 & -864 & -864 & -1152 & -288 & -2232 & -2232 & 1416 & -528 & 1152 & 1152 & 552 & -1248
\end{pmatrix}$$

$S = \{1243, 1342, 2314, 2431, 3124, 3421, 4132, 4213\}, \lambda_{max} = 0.060445, \lambda_{min} = -0.178535$

$$H_S = \frac{1}{6\cdot 5^6} \times \begin{pmatrix}
-3840 & 1200 & 2880 & 2880 & 120 & 4260 & -360 & -360 & 1440 & -720 & -1440 & -1440 & 1440 & -720 & -1440 & -1440 \\
1200 & -3840 & 1200 & 2880 & -4740 & 120 & 4260 & -360 & -720 & 1440 & -720 & -1440 & -720 & 1440 & -720 & -1440 \\
2880 & 1200 & -3840 & 1200 & -360 & -4740 & 120 & 4260 & -1440 & -720 & 1440 & -720 & -1440 & -720 & 1440 & -720 \\
2880 & 2880 & 1200 & -3840 & -360 & -360 & -4740 & 120 & -1440 & -1440 & -720 & 1440 & -1440 & -1440 & -720 & 1440 \\
120 & -4740 & -360 & -360 & -3840 & 1200 & 2880 & 2880 & 120 & -240 & -360 & -360 & 1440 & -720 & -1440 & -1440 \\
4260 & 120 & -4740 & -360 & 1200 & -3840 & 1200 & 2880 & -240 & 120 & -240 & -360 & -720 & 1440 & -720 & -1440 \\
-360 & 4260 & 120 & -4740 & 2880 & 1200 & -3840 & 1200 & -360 & -240 & 120 & -240 & -1440 & -720 & 1440 & -720 \\
-360 & -360 & 4260 & 120 & 2880 & 2880 & 1200 & -3840 & -360 & -360 & -240 & 120 & -1440 & -1440 & -720 & 1440 \\
1440 & -720 & -1440 & -1440 & 120 & -240 & -360 & -360 & -3840 & 1200 & 2880 & 2880 & 120 & -4740 & -360 & -360 \\
-720 & 1440 & -720 & -1440 & -240 & 120 & -240 & -360 & 1200 & -3840 & 1200 & 2880 & 4260 & 120 & -4740 & -360 \\
-1440 & -720 & 1440 & -720 & -360 & -240 & 120 & -240 & 2880 & 1200 & -3840 & 1200 & -360 & 4260 & 120 & -4740 \\
-1440 & -1440 & -720 & 1440 & -360 & -360 & -240 & 120 & 2880 & 2880 & 1200 & -3840 & -360 & -360 & 4260 & 120 \\
1440 & -720 & -1440 & -1440 & 1440 & -720 & -1440 & -1440 & 120 & 4260 & -360 & -360 & -3840 & 1200 & 2880 & 2880 \\
-720 & 1440 & -720 & -1440 & -720 & 1440 & -720 & -1440 & -4740 & 120 & 4260 & -360 & 1200 & -3840 & 1200 & 2880 \\
-1440 & -720 & 1440 & -720 & -1440 & -720 & 1440 & -720 & -360 & -4740 & 120 & 4260 & 2880 & 1200 & -3840 & 1200 \\
-1440 & -1440 & -720 & 1440 & -1440 & -1440 & -720 & 1440 & -360 & -360 & -4740 & 120 & 2880 & 2880 & 1200 & -3840
\end{pmatrix}$$

$S = \{1243, 1342, 2314, 2431, 3214, 3421, 4123, 4132\}, \lambda_{max} = 0.087796, \lambda_{min} = -0.090018$

$$H_S = \frac{1}{6 \cdot 5^6} \times \begin{pmatrix}
-384 & 336 & 576 & 576 & 336 & 3666 & 936 & 936 & 576 & -504 & -864 & -864 & 576 & -504 & -864 & -864 \\
336 & -384 & 336 & 576 & -4254 & 336 & 3306 & 936 & -504 & 576 & -504 & -864 & -504 & 576 & -504 & -864 \\
576 & 336 & -384 & 336 & -1944 & -3894 & 336 & 3666 & -864 & -504 & 576 & -504 & -864 & -504 & 576 & -504 \\
576 & 576 & 336 & -384 & -1944 & -1944 & -4254 & 336 & -864 & -864 & -504 & 576 & -864 & -864 & -504 & 576 \\
336 & -4254 & -1944 & -1944 & -384 & 336 & 576 & 576 & 336 & -294 & -504 & -504 & 576 & -504 & -864 & -864 \\
3666 & 336 & -3894 & -1944 & 336 & -384 & 336 & 576 & -294 & 336 & -294 & -504 & -504 & 576 & -504 & -864 \\
936 & 3306 & 336 & -4254 & 576 & 336 & -384 & 336 & -504 & -294 & 336 & -294 & -864 & -504 & 576 & -504 \\
936 & 936 & 3666 & 336 & 576 & 576 & 336 & -384 & -504 & -504 & -294 & 336 & -864 & -864 & -504 & 576 \\
576 & -504 & -864 & -864 & 336 & -294 & -504 & -504 & -384 & 336 & 576 & 576 & 336 & -4254 & -1944 & -1944 \\
-504 & 576 & -504 & -864 & -294 & 336 & -294 & -504 & 336 & -384 & 336 & 576 & 3666 & 336 & -3894 & -1944 \\
-864 & -504 & 576 & -504 & -504 & -294 & 336 & -294 & 576 & 336 & -384 & 336 & 936 & 3306 & 336 & -4254 \\
-864 & -864 & -504 & 576 & -504 & -504 & -294 & 336 & 576 & 576 & 336 & -384 & 936 & 936 & 3666 & 336 \\
576 & -504 & -864 & -864 & 576 & -504 & -864 & -864 & 336 & 3666 & 936 & 936 & -384 & 336 & 576 & 576 \\
-504 & 576 & -504 & -864 & -504 & 576 & -504 & -864 & -4254 & 336 & 3306 & 936 & 336 & -384 & 336 & 576 \\
-864 & -504 & 576 & -504 & -864 & -504 & 576 & -504 & -1944 & -3894 & 336 & 3666 & 576 & 336 & -384 & 336 \\
-864 & -864 & -504 & 576 & -864 & -864 & -504 & 576 & -1944 & -1944 & -4254 & 336 & 576 & 576 & 336 & -384
\end{pmatrix}$$

$S = \{1243, 1432, 2134, 2341, 3214, 3421, 4123, 4312\}, \lambda_{max} = 0.083022, \lambda_{min} = -0.003853$

$$H_S = \frac{1}{6 \cdot 5^6} \times \begin{pmatrix}
4224 & 624 & -576 & -576 & 624 & -276 & -576 & -576 & -576 & -576 & -576 & -576 & -576 & -576 & -576 & -576 \\
624 & 4224 & 624 & -576 & -276 & 624 & -276 & -576 & -576 & -576 & -576 & -576 & -576 & -576 & -576 & -576 \\
-576 & 624 & 4224 & 624 & -576 & -276 & 624 & -276 & -576 & -576 & -576 & -576 & -576 & -576 & -576 & -576 \\
-576 & -576 & 624 & 4224 & -576 & -576 & -276 & 624 & -576 & -576 & -576 & -576 & -576 & -576 & -576 & -576 \\
624 & -276 & -576 & -576 & 4224 & 624 & -576 & -576 & 624 & -276 & -576 & -576 & -576 & -576 & -576 & -576 \\
-276 & 624 & -276 & -576 & 624 & 4224 & 624 & -576 & -276 & 624 & -276 & -576 & -576 & -576 & -576 & -576 \\
-576 & -276 & 624 & -276 & -576 & 624 & 4224 & 624 & -576 & -276 & 624 & -276 & -576 & -576 & -576 & -576 \\
-576 & -576 & -276 & 624 & -576 & -576 & 624 & 4224 & -576 & -576 & -276 & 624 & -576 & -576 & -576 & -576 \\
-576 & -576 & -576 & -576 & 624 & -276 & -576 & -576 & 4224 & 624 & -576 & -576 & 624 & -276 & -576 & -576 \\
-576 & -576 & -576 & -576 & -276 & 624 & -276 & -576 & 624 & 4224 & 624 & -576 & -276 & 624 & -276 & -576 \\
-576 & -576 & -576 & -576 & -576 & -276 & 624 & -276 & -576 & 624 & 4224 & 624 & -576 & -276 & 624 & -276 \\
-576 & -576 & -576 & -576 & -576 & -576 & -276 & 624 & -576 & -576 & 624 & 4224 & -576 & -576 & -276 & 624 \\
-576 & -576 & -576 & -576 & -576 & -576 & -576 & -576 & 624 & -276 & -576 & -576 & 4224 & 624 & -576 & -576 \\
-576 & -576 & -576 & -576 & -576 & -576 & -576 & -576 & -276 & 624 & -276 & -576 & 624 & 4224 & 624 & -576 \\
-576 & -576 & -576 & -576 & -576 & -576 & -576 & -576 & -576 & -276 & 624 & -276 & -576 & 624 & 4224 & 624 \\
-576 & -576 & -576 & -576 & -576 & -576 & -576 & -576 & -576 & -576 & -276 & 624 & -576 & -576 & 624 & 4224
\end{pmatrix}$$

$S = \{1243, 1432, 2314, 2341, 3124, 3412, 4123, 4231\}, \lambda_{max} = 0.292132, \lambda_{min} = -0.205639$

$$H_S = \frac{1}{6 \cdot 5^6} \times \begin{pmatrix}
2208 & -312 & -1152 & -1152 & -312 & 10902 & -2376 & -2376 & -1152 & -2376 & -288 & -288 & -1152 & -2376 & -288 & -288 \\
-312 & 2208 & -312 & -1152 & -11166 & -312 & 9858 & -2376 & 2232 & -1152 & -1512 & -288 & 2232 & -1152 & -1512 & -288 \\
-1152 & -312 & 2208 & -312 & 2232 & -10122 & -312 & 7662 & 864 & 1368 & -1152 & -936 & 864 & 1368 & -1152 & -936 \\
-1152 & -1152 & -312 & 2208 & 2232 & 2232 & -7926 & -312 & 864 & 864 & 792 & -1152 & 864 & 864 & 792 & -1152 \\
-312 & -11166 & 2232 & 2232 & 2208 & -312 & -1152 & -1152 & -312 & 9858 & -1512 & -1512 & -1152 & -2376 & -288 & -288 \\
10902 & -312 & -10122 & 2232 & -312 & 2208 & -312 & -1152 & -10122 & -312 & 7518 & -1512 & 2232 & -1152 & -1512 & -288 \\
-2376 & 9858 & -312 & -7926 & -1152 & -312 & 2208 & -312 & 1368 & -7782 & -312 & 4458 & 864 & 1368 & -1152 & -936 \\
-2376 & -2376 & 7662 & -312 & -1152 & -1152 & -312 & 2208 & 1368 & 1368 & -4722 & -312 & 864 & 864 & 792 & -1152 \\
-1152 & 2232 & 864 & 864 & -312 & -10122 & 1368 & 1368 & 2208 & -312 & -1152 & -1152 & -312 & 7662 & -936 & -936 \\
-2376 & -1152 & 1368 & 864 & 9858 & -312 & -7782 & 1368 & -312 & 2208 & -312 & -1152 & -7926 & -312 & 4458 & -936 \\
-288 & -1512 & -1152 & 792 & -1512 & 7518 & -312 & -4722 & -1152 & -312 & 2208 & -312 & 792 & -4722 & -312 & 822 \\
-288 & -288 & -936 & -1152 & -1512 & -1512 & 4458 & -312 & -1152 & -1152 & -312 & 2208 & 792 & 792 & -1086 & -312 \\
-1152 & 2232 & 864 & 864 & -1152 & 2232 & 864 & 864 & -312 & -7926 & 792 & 792 & 2208 & -312 & -1152 & -1152 \\
-2376 & -1152 & 1368 & 864 & -2376 & -1152 & 1368 & 864 & 7662 & -312 & -4722 & 792 & -312 & 2208 & -312 & -1152 \\
-288 & -1512 & -1152 & 792 & -288 & -1512 & -1152 & 792 & -936 & 4458 & -312 & -1086 & -1152 & -312 & 2208 & -312 \\
-288 & -288 & -936 & -1152 & -288 & -288 & -936 & -1152 & -936 & -936 & 822 & -312 & -1152 & -1152 & -312 & 2208
\end{pmatrix}$$

$S = \{1243, 1432, 2314, 2341, 3124, 3421, 4132, 4213\}, \lambda_{max} = 0.103242, \lambda_{min} = -0.118967$

$$H_S = \frac{1}{6 \cdot 5^6} \times \begin{pmatrix}
-384 & 336 & 576 & 576 & 336 & 4746 & -1944 & -1944 & 576 & -504 & -864 & -864 & 576 & -504 & -864 & -864 \\
336 & -384 & 336 & 576 & -5334 & 336 & 5106 & -1944 & -504 & 576 & -504 & -864 & -504 & 576 & -504 & -864 \\
576 & 336 & -384 & 336 & 936 & -5694 & 336 & 4746 & -864 & -504 & 576 & -504 & -864 & -504 & 576 & -504 \\
576 & 576 & 336 & -384 & 936 & 936 & -5334 & 336 & -864 & -864 & -504 & 576 & -864 & -864 & -504 & 576 \\
336 & -5334 & 936 & 936 & -384 & 336 & 576 & 576 & 336 & -294 & -504 & -504 & 576 & -504 & -864 & -864 \\
4746 & 336 & -5694 & 936 & 336 & -384 & 336 & 576 & -294 & 336 & -294 & -504 & -504 & 576 & -504 & -864 \\
-1944 & 5106 & 336 & -5334 & 576 & 336 & -384 & 336 & -504 & -294 & 336 & -294 & -864 & -504 & 576 & -504 \\
-1944 & -1944 & 4746 & 336 & 576 & 576 & 336 & -384 & -504 & -504 & -294 & 336 & -864 & -864 & -504 & 576 \\
576 & -504 & -864 & -864 & 336 & -294 & -504 & -504 & -384 & 336 & 576 & 576 & 336 & -5334 & 936 & 936 \\
-504 & 576 & -504 & -864 & -294 & 336 & -294 & -504 & 336 & -384 & 336 & 576 & 4746 & 336 & -5694 & 936 \\
-864 & -504 & 576 & -504 & -504 & -294 & 336 & -294 & 576 & 336 & -384 & 336 & -1944 & 5106 & 336 & -5334 \\
-864 & -864 & -504 & 576 & -504 & -504 & -294 & 336 & 576 & 576 & 336 & -384 & -1944 & -1944 & 4746 & 336 \\
576 & -504 & -864 & -864 & 576 & -504 & -864 & -864 & 336 & 4746 & -1944 & -1944 & -384 & 336 & 576 & 576 \\
-504 & 576 & -504 & -864 & -504 & 576 & -504 & -864 & -5334 & 336 & 5106 & -1944 & 336 & -384 & 336 & 576 \\
-864 & -504 & 576 & -504 & -864 & -504 & 576 & -504 & 936 & -5694 & 336 & 4746 & 576 & 336 & -384 & 336 \\
-864 & -864 & -504 & 576 & -864 & -864 & -504 & 576 & 936 & 936 & -5334 & 336 & 576 & 576 & 336 & -384
\end{pmatrix}$$

$S = \{1243, 1432, 2314, 2341, 3214, 3421, 4123, 4132\}, \lambda_{max} = 0.138457, \lambda_{min} = -0.049322$

$$H_S = \frac{1}{6 \cdot 5^6} \times \begin{pmatrix}
3072 & -528 & -1728 & -1728 & 552 & 4152 & -648 & -648 & -288 & -288 & -288 & -288 & -288 & -288 & -288 & -288 \\
-528 & 3072 & -528 & -1728 & -4848 & 552 & 4152 & -648 & -288 & -288 & -288 & -288 & -288 & -288 & -288 & -288 \\
-1728 & -528 & 3072 & -528 & -648 & -4848 & 552 & 4152 & -288 & -288 & -288 & -288 & -288 & -288 & -288 & -288 \\
-1728 & -1728 & -528 & 3072 & -648 & -648 & -4848 & 552 & -288 & -288 & -288 & -288 & -288 & -288 & -288 & -288 \\
552 & -4848 & -648 & -648 & 3072 & -528 & -1728 & -1728 & 552 & -348 & -648 & -648 & -288 & -288 & -288 & -288 \\
4152 & 552 & -4848 & -648 & -528 & 3072 & -528 & -1728 & -348 & 552 & -348 & -648 & -288 & -288 & -288 & -288 \\
-648 & 4152 & 552 & -4848 & -1728 & -528 & 3072 & -528 & -648 & -348 & 552 & -348 & -288 & -288 & -288 & -288 \\
-648 & -648 & 4152 & 552 & -1728 & -1728 & -528 & 3072 & -648 & -648 & -348 & 552 & -288 & -288 & -288 & -288 \\
-288 & -288 & -288 & -288 & 552 & -348 & -648 & -648 & 3072 & -528 & -1728 & -1728 & 552 & -4848 & -648 & -648 \\
-288 & -288 & -288 & -288 & -348 & 552 & -348 & -648 & -528 & 3072 & -528 & -1728 & 4152 & 552 & -4848 & -648 \\
-288 & -288 & -288 & -288 & -648 & -348 & 552 & -348 & -1728 & -528 & 3072 & -528 & -648 & 4152 & 552 & -4848 \\
-288 & -288 & -288 & -288 & -648 & -648 & -348 & 552 & -1728 & -1728 & -528 & 3072 & -648 & -648 & 4152 & 552 \\
-288 & -288 & -288 & -288 & -288 & -288 & -288 & -288 & 552 & 4152 & -648 & -648 & 3072 & -528 & -1728 & -1728 \\
-288 & -288 & -288 & -288 & -288 & -288 & -288 & -288 & -4848 & 552 & 4152 & -648 & -528 & 3072 & -528 & -1728 \\
-288 & -288 & -288 & -288 & -288 & -288 & -288 & -288 & -648 & -4848 & 552 & 4152 & -1728 & -528 & 3072 & -528 \\
-288 & -288 & -288 & -288 & -288 & -288 & -288 & -288 & -648 & -648 & -4848 & 552 & -1728 & -1728 & -528 & 3072
\end{pmatrix}$$

$S = \{1324, 1342, 2143, 2431, 3124, 3412, 4213, 4231\}, \lambda_{max} = 0.037736, \lambda_{min} = -0.115342$

$$H_S = \frac{1}{6 \cdot 5^6} \times \begin{pmatrix}
-2112 & 768 & 1728 & 1728 & -1392 & -1662 & 648 & 648 & -1152 & -72 & 288 & 288 & -1152 & -72 & 288 & 288 \\
768 & -2112 & 768 & 1728 & 1938 & -1392 & 138 & 648 & -72 & -1152 & -72 & 288 & -72 & -1152 & -72 & 288 \\
1728 & 768 & -2112 & 768 & 648 & 138 & -1392 & 1938 & 288 & -72 & -1152 & -72 & 288 & -72 & -1152 & -72 \\
1728 & 1728 & 768 & -2112 & 648 & 648 & -1662 & -1392 & 288 & 288 & -72 & -1152 & 288 & 288 & -72 & -1152 \\
-1392 & 1938 & 648 & 648 & -2112 & 768 & 1728 & 1728 & -1392 & 138 & 648 & 648 & -1152 & -72 & 288 & 288 \\
-1662 & -1392 & 138 & 648 & 768 & -2112 & 768 & 1728 & 138 & -1392 & 138 & 648 & -72 & -1152 & -72 & 288 \\
648 & 138 & -1392 & -1662 & 1728 & 768 & -2112 & 768 & 648 & 138 & -1392 & 138 & 288 & -72 & -1152 & -72 \\
648 & 648 & 1938 & -1392 & 1728 & 1728 & 768 & -2112 & 648 & 648 & 138 & -1392 & 288 & 288 & -72 & -1152 \\
-1152 & -72 & 288 & 288 & -1392 & 138 & 648 & 648 & -2112 & 768 & 1728 & 1728 & -1392 & 1938 & 648 & 648 \\
-72 & -1152 & -72 & 288 & 138 & -1392 & 138 & 648 & 768 & -2112 & 768 & 1728 & -1662 & -1392 & 138 & 648 \\
288 & -72 & -1152 & -72 & 648 & 138 & -1392 & 138 & 1728 & 768 & -2112 & 768 & 648 & 138 & -1392 & -1662 \\
288 & 288 & -72 & -1152 & 648 & 648 & 138 & -1392 & 1728 & 1728 & 768 & -2112 & 648 & 648 & 1938 & -1392 \\
-1152 & -72 & 288 & 288 & -1152 & -72 & 288 & 288 & -1392 & -1662 & 648 & 648 & -2112 & 768 & 1728 & 1728 \\
-72 & -1152 & -72 & 288 & -72 & -1152 & -72 & 288 & 1938 & -1392 & 138 & 648 & 768 & -2112 & 768 & 1728 \\
288 & -72 & -1152 & -72 & 288 & -72 & -1152 & -72 & 648 & 138 & -1392 & 1938 & 1728 & 768 & -2112 & 768 \\
288 & 288 & -72 & -1152 & 288 & 288 & -72 & -1152 & 648 & 648 & -1662 & -1392 & 1728 & 1728 & 768 & -2112
\end{pmatrix}$$

$S = \{1324, 1342, 2143, 2431, 3214, 3412, 4123, 4231\}, \lambda_{max} = 0.082834, \lambda_{min} = -0.072228$

$$H_S = \frac{1}{6 \cdot 5^6} \times \begin{pmatrix}
1344 & -96 & -576 & -576 & -1176 & -2256 & 1944 & 1944 & -2016 & 144 & 864 & 864 & -2016 & 144 & 864 & 864 \\
-96 & 1344 & -96 & -576 & 2424 & -1176 & -816 & 1944 & 144 & -2016 & 144 & 864 & 144 & -2016 & 144 & 864 \\
-576 & -96 & 1344 & -96 & -936 & 984 & -1176 & 1344 & 864 & 144 & -2016 & 144 & 864 & 144 & -2016 & 144 \\
-576 & -576 & -96 & 1344 & -936 & -936 & -1176 & -1176 & 864 & 864 & 144 & -2016 & 864 & 864 & 144 & -2016 \\
-1176 & 2424 & -936 & -936 & 1344 & -96 & -576 & -576 & -1176 & 84 & 504 & 504 & -2016 & 144 & 864 & 864 \\
-2256 & -1176 & 984 & -936 & -96 & 1344 & -96 & -576 & 84 & -1176 & 84 & 504 & 144 & -2016 & 144 & 864 \\
1944 & -816 & -1176 & -1176 & -576 & -96 & 1344 & -96 & 504 & 84 & -1176 & 84 & 864 & 144 & -2016 & 144 \\
1944 & 1944 & 1344 & -1176 & -576 & -576 & -96 & 1344 & 504 & 504 & 84 & -1176 & 864 & 864 & 144 & -2016 \\
-2016 & 144 & 864 & 864 & -1176 & 84 & 504 & 504 & 1344 & -96 & -576 & -576 & -1176 & 2424 & -936 & -936 \\
144 & -2016 & 144 & 864 & 84 & -1176 & 84 & 504 & -96 & 1344 & -96 & -576 & -2256 & -1176 & 984 & -936 \\
864 & 144 & -2016 & 144 & 504 & 84 & -1176 & 84 & -576 & -96 & 1344 & -96 & 1944 & -816 & -1176 & -1176 \\
864 & 864 & 144 & -2016 & 504 & 504 & 84 & -1176 & -576 & -576 & -96 & 1344 & 1944 & 1944 & 1344 & -1176 \\
-2016 & 144 & 864 & 864 & -2016 & 144 & 864 & 864 & -1176 & -2256 & 1944 & 1944 & 1344 & -96 & -576 & -576 \\
144 & -2016 & 144 & 864 & 144 & -2016 & 144 & 864 & 2424 & -1176 & -816 & 1944 & -96 & 1344 & -96 & -576 \\
864 & 144 & -2016 & 144 & 864 & 144 & -2016 & 144 & -936 & 984 & -1176 & 1344 & -576 & -96 & 1344 & -96 \\
864 & 864 & 144 & -2016 & 864 & 864 & 144 & -2016 & -936 & -936 & -1176 & -1176 & -576 & -576 & -96 & 1344
\end{pmatrix}$$

$\mathbf{S = \{1324, 1342, 2413, 2431, 3124, 3142, 4213, 4231\}}, \lambda_{max} = -0.009351, \lambda_{min} = -0.166043$

$$H_S = \frac{1}{6 \cdot 5^6} \times \begin{pmatrix}
-6720 & 480 & 2880 & 2880 & -1680 & 120 & 720 & 720 & 0 & 0 & 0 & 0 & 0 & 0 & 0 & 0 \\
480 & -6720 & 480 & 2880 & 120 & -1680 & 120 & 720 & 0 & 0 & 0 & 0 & 0 & 0 & 0 & 0 \\
2880 & 480 & -6720 & 480 & 720 & 120 & -1680 & 120 & 0 & 0 & 0 & 0 & 0 & 0 & 0 & 0 \\
2880 & 2880 & 480 & -6720 & 720 & 720 & 120 & -1680 & 0 & 0 & 0 & 0 & 0 & 0 & 0 & 0 \\
-1680 & 120 & 720 & 720 & -6720 & 480 & 2880 & 2880 & -1680 & 120 & 720 & 720 & 0 & 0 & 0 & 0 \\
120 & -1680 & 120 & 720 & 480 & -6720 & 480 & 2880 & 120 & -1680 & 120 & 720 & 0 & 0 & 0 & 0 \\
720 & 120 & -1680 & 120 & 2880 & 480 & -6720 & 480 & 720 & 120 & -1680 & 120 & 0 & 0 & 0 & 0 \\
720 & 720 & 120 & -1680 & 2880 & 2880 & 480 & -6720 & 720 & 720 & 120 & -1680 & 0 & 0 & 0 & 0 \\
0 & 0 & 0 & 0 & -1680 & 120 & 720 & 720 & -6720 & 480 & 2880 & 2880 & -1680 & 120 & 720 & 720 \\
0 & 0 & 0 & 0 & 120 & -1680 & 120 & 720 & 480 & -6720 & 480 & 2880 & 120 & -1680 & 120 & 720 \\
0 & 0 & 0 & 0 & 720 & 120 & -1680 & 120 & 2880 & 480 & -6720 & 480 & 720 & 120 & -1680 & 120 \\
0 & 0 & 0 & 0 & 720 & 720 & 120 & -1680 & 2880 & 2880 & 480 & -6720 & 720 & 720 & 120 & -1680 \\
0 & 0 & 0 & 0 & 0 & 0 & 0 & 0 & -1680 & 120 & 720 & 720 & -6720 & 480 & 2880 & 2880 \\
0 & 0 & 0 & 0 & 0 & 0 & 0 & 0 & 120 & -1680 & 120 & 720 & 480 & -6720 & 480 & 2880 \\
0 & 0 & 0 & 0 & 0 & 0 & 0 & 0 & 720 & 120 & -1680 & 120 & 2880 & 480 & -6720 & 480 \\
0 & 0 & 0 & 0 & 0 & 0 & 0 & 0 & 720 & 720 & 120 & -1680 & 2880 & 2880 & 480 & -6720
\end{pmatrix}$$

$S = \{1324, 1342, 2413, 2431, 3124, 3241, 4132, 4213\}, \lambda_{max} = 0.044170, \lambda_{min} = -0.198873$

$$H_S = \frac{1}{6 \cdot 5^6} \times \begin{pmatrix}
-5856 & 264 & 2304 & 2304 & -816 & -1446 & 3744 & 3744 & 864 & -216 & -576 & -576 & 864 & -216 & -576 & -576 \\
264 & -5856 & 264 & 2304 & 1254 & -816 & -2346 & 3744 & -216 & 864 & -216 & -576 & -216 & 864 & -216 & -576 \\
2304 & 264 & -5856 & 264 & -3456 & 2154 & -816 & -1446 & -576 & -216 & 864 & -216 & -576 & -216 & 864 & -216 \\
2304 & 2304 & 264 & -5856 & -3456 & -3456 & 1254 & -816 & -576 & -576 & -216 & 864 & -576 & -576 & -216 & 864 \\
-816 & 1254 & -3456 & -3456 & -5856 & 264 & 2304 & 2304 & -816 & -1446 & 3744 & 3744 & 864 & -216 & -576 & -576 \\
-1446 & -816 & 2154 & -3456 & 264 & -5856 & 264 & 2304 & 1254 & -816 & -2346 & 3744 & -216 & 864 & -216 & -576 \\
3744 & -2346 & -816 & 1254 & 2304 & 264 & -5856 & 264 & -3456 & 2154 & -816 & -1446 & -576 & -216 & 864 & -216 \\
3744 & 3744 & -1446 & -816 & 2304 & 2304 & 264 & -5856 & -3456 & -3456 & 1254 & -816 & -576 & -576 & -216 & 864 \\
864 & -216 & -576 & -576 & -816 & 1254 & -3456 & -3456 & -5856 & 264 & 2304 & 2304 & -816 & -1446 & 3744 & 3744 \\
-216 & 864 & -216 & -576 & -1446 & -816 & 2154 & -3456 & 264 & -5856 & 264 & 2304 & 1254 & -816 & -2346 & 3744 \\
-576 & -216 & 864 & -216 & 3744 & -2346 & -816 & 1254 & 2304 & 264 & -5856 & 264 & -3456 & 2154 & -816 & -1446 \\
-576 & -576 & -216 & 864 & 3744 & 3744 & -1446 & -816 & 2304 & 2304 & 264 & -5856 & -3456 & -3456 & 1254 & -816 \\
864 & -216 & -576 & -576 & 864 & -216 & -576 & -576 & -816 & 1254 & -3456 & -3456 & -5856 & 264 & 2304 & 2304 \\
-216 & 864 & -216 & -576 & -216 & 864 & -216 & -576 & -1446 & -816 & 2154 & -3456 & 264 & -5856 & 264 & 2304 \\
-576 & -216 & 864 & -216 & -576 & -216 & 864 & -216 & 3744 & -2346 & -816 & 1254 & 2304 & 264 & -5856 & 264 \\
-576 & -576 & -216 & 864 & -576 & -576 & -216 & 864 & 3744 & 3744 & -1446 & -816 & 2304 & 2304 & 264 & -5856
\end{pmatrix}$$

$S = \{1324, 1342, 2413, 2431, 3142, 3214, 4123, 4231\}, \lambda_{max} = 0.006345, \lambda_{min} = -0.118115$

$$H_S = \frac{1}{6 \cdot 5^6} \times \begin{pmatrix}
-3264 & -384 & 576 & 576 & -1464 & -474 & 2016 & 2016 & -864 & 216 & 576 & 576 & -864 & 216 & 576 & 576 \\
-384 & -3264 & -384 & 576 & 606 & -1464 & -834 & 2016 & 216 & -864 & 216 & 576 & 216 & -864 & 216 & 576 \\
576 & -384 & -3264 & -384 & -864 & 966 & -1464 & -474 & 576 & 216 & -864 & 216 & 576 & 216 & -864 & 216 \\
576 & 576 & -384 & -3264 & -864 & -864 & 606 & -1464 & 576 & 576 & 216 & -864 & 576 & 576 & 216 & -864 \\
-1464 & 606 & -864 & -864 & -3264 & -384 & 576 & 576 & -1464 & 66 & 576 & 576 & -864 & 216 & 576 & 576 \\
-474 & -1464 & 966 & -864 & -384 & -3264 & -384 & 576 & 66 & -1464 & 66 & 576 & 216 & -864 & 216 & 576 \\
2016 & -834 & -1464 & 606 & 576 & -384 & -3264 & -384 & 576 & 66 & -1464 & 66 & 576 & 216 & -864 & 216 \\
2016 & 2016 & -474 & -1464 & 576 & 576 & -384 & -3264 & 576 & 576 & 66 & -1464 & 576 & 576 & 216 & -864 \\
-864 & 216 & 576 & 576 & -1464 & 66 & 576 & 576 & -3264 & -384 & 576 & 576 & -1464 & 606 & -864 & -864 \\
216 & -864 & 216 & 576 & 66 & -1464 & 66 & 576 & -384 & -3264 & -384 & 576 & -474 & -1464 & 966 & -864 \\
576 & 216 & -864 & 216 & 576 & 66 & -1464 & 66 & 576 & -384 & -3264 & -384 & 2016 & -834 & -1464 & 606 \\
576 & 576 & 216 & -864 & 576 & 576 & 66 & -1464 & 576 & 576 & -384 & -3264 & 2016 & 2016 & -474 & -1464 \\
-864 & 216 & 576 & 576 & -864 & 216 & 576 & 576 & -1464 & -474 & 2016 & 2016 & -3264 & -384 & 576 & 576 \\
216 & -864 & 216 & 576 & 216 & -864 & 216 & 576 & 606 & -1464 & -834 & 2016 & -384 & -3264 & -384 & 576 \\
576 & 216 & -864 & 216 & 576 & 216 & -864 & 216 & -864 & 966 & -1464 & -474 & 576 & -384 & -3264 & -384 \\
576 & 576 & 216 & -864 & 576 & 576 & 216 & -864 & -864 & -864 & 606 & -1464 & 576 & 576 & -384 & -3264
\end{pmatrix}$$

$S = \{1324, 1342, 2413, 2431, 3214, 3241, 4123, 4132\}, \lambda_{max} = 0.090731, \lambda_{min} = -0.142057$

$$H_S = \frac{1}{6 \cdot 5^6} \times \begin{pmatrix}
-2400 & -600 & 0 & 0 & -600 & -2040 & 5040 & 5040 & 0 & 0 & 0 & 0 & 0 & 0 & 0 & 0 \\
-600 & -2400 & -600 & 0 & 1740 & -600 & -3300 & 5040 & 0 & 0 & 0 & 0 & 0 & 0 & 0 & 0 \\
0 & -600 & -2400 & -600 & -5040 & 3000 & -600 & -2040 & 0 & 0 & 0 & 0 & 0 & 0 & 0 & 0 \\
0 & 0 & -600 & -2400 & -5040 & -5040 & 1740 & -600 & 0 & 0 & 0 & 0 & 0 & 0 & 0 & 0 \\
-600 & 1740 & -5040 & -5040 & -2400 & -600 & 0 & 0 & -600 & -1500 & 3600 & 3600 & 0 & 0 & 0 & 0 \\
-2040 & -600 & 3000 & -5040 & -600 & -2400 & -600 & 0 & 1200 & -600 & -2400 & 3600 & 0 & 0 & 0 & 0 \\
5040 & -3300 & -600 & 1740 & 0 & -600 & -2400 & -600 & -3600 & 2100 & -600 & -1500 & 0 & 0 & 0 & 0 \\
5040 & 5040 & -2040 & -600 & 0 & 0 & -600 & -2400 & -3600 & -3600 & 1200 & -600 & 0 & 0 & 0 & 0 \\
0 & 0 & 0 & 0 & -600 & 1200 & -3600 & -3600 & -2400 & -600 & 0 & 0 & -600 & -960 & 2160 & 2160 \\
0 & 0 & 0 & 0 & -1500 & -600 & 2100 & -3600 & -600 & -2400 & -600 & 0 & 660 & -600 & -1500 & 2160 \\
0 & 0 & 0 & 0 & 3600 & -2400 & -600 & 1200 & 0 & -600 & -2400 & -600 & -2160 & 1200 & -600 & -960 \\
0 & 0 & 0 & 0 & 3600 & 3600 & -1500 & -600 & 0 & 0 & -600 & -2400 & -2160 & -2160 & 660 & -600 \\
0 & 0 & 0 & 0 & 0 & 0 & 0 & 0 & -600 & 660 & -2160 & -2160 & -2400 & -600 & 0 & 0 \\
0 & 0 & 0 & 0 & 0 & 0 & 0 & 0 & -960 & -600 & 1200 & -2160 & -600 & -2400 & -600 & 0 \\
0 & 0 & 0 & 0 & 0 & 0 & 0 & 0 & 2160 & -1500 & -600 & 660 & 0 & -600 & -2400 & -600 \\
0 & 0 & 0 & 0 & 0 & 0 & 0 & 0 & 2160 & 2160 & -960 & -600 & 0 & 0 & -600 & -2400
\end{pmatrix}$$

$S = \{1324, 1432, 2143, 2341, 3214, 3412, 4123, 4231\}, \lambda_{max} = 0.173488, \lambda_{min} = -0.028480$

$$H_S = \frac{1}{6 \cdot 5^6} \times \begin{pmatrix}
4800 & -960 & -2880 & -2880 & -960 & -1770 & 360 & 360 & -2880 & 360 & 1440 & 1440 & -2880 & 360 & 1440 & 1440 \\
-960 & 4800 & -960 & -2880 & 1830 & -960 & 30 & 360 & 360 & -2880 & 360 & 1440 & 360 & -2880 & 360 & 1440 \\
-2880 & -960 & 4800 & -960 & 360 & 30 & -960 & 1830 & 1440 & 360 & -2880 & 360 & 1440 & 360 & -2880 & 360 \\
-2880 & -2880 & -960 & 4800 & 360 & 360 & -1770 & -960 & 1440 & 1440 & 360 & -2880 & 1440 & 1440 & 360 & -2880 \\
-960 & 1830 & 360 & 360 & 4800 & -960 & -2880 & -2880 & -960 & 30 & 360 & 360 & -2880 & 360 & 1440 & 1440 \\
-1770 & -960 & 30 & 360 & -960 & 4800 & -960 & -2880 & 30 & -960 & 30 & 360 & 360 & -2880 & 360 & 1440 \\
360 & 30 & -960 & -1770 & -2880 & -960 & 4800 & -960 & 360 & 30 & -960 & 30 & 1440 & 360 & -2880 & 360 \\
360 & 360 & 1830 & -960 & -2880 & -2880 & -960 & 4800 & 360 & 360 & 30 & -960 & 1440 & 1440 & 360 & -2880 \\
-2880 & 360 & 1440 & 1440 & -960 & 30 & 360 & 360 & 4800 & -960 & -2880 & -2880 & -960 & 1830 & 360 & 360 \\
360 & -2880 & 360 & 1440 & 30 & -960 & 30 & 360 & -960 & 4800 & -960 & -2880 & -1770 & -960 & 30 & 360 \\
1440 & 360 & -2880 & 360 & 360 & 30 & -960 & 30 & -2880 & -960 & 4800 & -960 & 360 & 30 & -960 & -1770 \\
1440 & 1440 & 360 & -2880 & 360 & 360 & 30 & -960 & -2880 & -2880 & -960 & 4800 & 360 & 360 & 1830 & -960 \\
-2880 & 360 & 1440 & 1440 & -2880 & 360 & 1440 & 1440 & -960 & -1770 & 360 & 360 & 4800 & -960 & -2880 & -2880 \\
360 & -2880 & 360 & 1440 & 360 & -2880 & 360 & 1440 & 1830 & -960 & 30 & 360 & -960 & 4800 & -960 & -2880 \\
1440 & 360 & -2880 & 360 & 1440 & 360 & -2880 & 360 & 360 & 30 & -960 & 1830 & -2880 & -960 & 4800 & -960 \\
1440 & 1440 & 360 & -2880 & 1440 & 1440 & 360 & -2880 & 360 & 360 & -1770 & -960 & -2880 & -2880 & -960 & 4800
\end{pmatrix}$$

$S = \{1324, 1432, 2341, 2413, 3142, 3214, 4123, 4231\}, \lambda_{max} = 0.068244, \lambda_{min} = -0.061073$

$$H_S = \frac{1}{6 \cdot 5^6} \times \begin{pmatrix}
192 & -1248 & -1728 & -1728 & -1248 & 12 & 432 & 432 & -1728 & 432 & 1152 & 1152 & -1728 & 432 & 1152 & 1152 \\
-1248 & 192 & -1248 & -1728 & 12 & -1248 & 12 & 432 & 432 & -1728 & 432 & 1152 & 432 & -1728 & 432 & 1152 \\
-1728 & -1248 & 192 & -1248 & 432 & 12 & -1248 & 12 & 1152 & 432 & -1728 & 432 & 1152 & 432 & -1728 & 432 \\
-1728 & -1728 & -1248 & 192 & 432 & 432 & 12 & -1248 & 1152 & 1152 & 432 & -1728 & 1152 & 1152 & 432 & -1728 \\
-1248 & 12 & 432 & 432 & 192 & -1248 & -1728 & -1728 & -1248 & 12 & 432 & 432 & -1728 & 432 & 1152 & 1152 \\
12 & -1248 & 12 & 432 & -1248 & 192 & -1248 & -1728 & 12 & -1248 & 12 & 432 & 432 & -1728 & 432 & 1152 \\
432 & 12 & -1248 & 12 & -1728 & -1248 & 192 & -1248 & 432 & 12 & -1248 & 12 & 1152 & 432 & -1728 & 432 \\
432 & 432 & 12 & -1248 & -1728 & -1728 & -1248 & 192 & 432 & 432 & 12 & -1248 & 1152 & 1152 & 432 & -1728 \\
-1728 & 432 & 1152 & 1152 & -1248 & 12 & 432 & 432 & 192 & -1248 & -1728 & -1728 & -1248 & 12 & 432 & 432 \\
432 & -1728 & 432 & 1152 & 12 & -1248 & 12 & 432 & -1248 & 192 & -1248 & -1728 & 12 & -1248 & 12 & 432 \\
1152 & 432 & -1728 & 432 & 432 & 12 & -1248 & 12 & -1728 & -1248 & 192 & -1248 & 432 & 12 & -1248 & 12 \\
1152 & 1152 & 432 & -1728 & 432 & 432 & 12 & -1248 & -1728 & -1728 & -1248 & 192 & 432 & 432 & 12 & -1248 \\
-1728 & 432 & 1152 & 1152 & -1728 & 432 & 1152 & 1152 & -1248 & 12 & 432 & 432 & 192 & -1248 & -1728 & -1728 \\
432 & -1728 & 432 & 1152 & 432 & -1728 & 432 & 1152 & 12 & -1248 & 12 & 432 & -1248 & 192 & -1248 & -1728 \\
1152 & 432 & -1728 & 432 & 1152 & 432 & -1728 & 432 & 432 & 12 & -1248 & 12 & -1728 & -1248 & 192 & -1248 \\
1152 & 1152 & 432 & -1728 & 1152 & 1152 & 432 & -1728 & 432 & 432 & 12 & -1248 & -1728 & -1728 & -1248 & 192
\end{pmatrix}$$

$S = \{1324, 1432, 2341, 2413, 3214, 3241, 4123, 4132\}, \lambda_{max} = 0.143605, \lambda_{min} = -0.106412$

$$H_S = \frac{1}{6 \cdot 5^6} \times \begin{pmatrix}
1056 & -1464 & -2304 & -2304 & -384 & -1554 & 3456 & 3456 & -864 & 216 & 576 & 576 & -864 & 216 & 576 & 576 \\
-1464 & 1056 & -1464 & -2304 & 1146 & -384 & -2454 & 3456 & 216 & -864 & 216 & 576 & 216 & -864 & 216 & 576 \\
-2304 & -1464 & 1056 & -1464 & -3744 & 2046 & -384 & -1554 & 576 & 216 & -864 & 216 & 576 & 216 & -864 & 216 \\
-2304 & -2304 & -1464 & 1056 & -3744 & -3744 & 1146 & -384 & 576 & 576 & 216 & -864 & 576 & 576 & 216 & -864 \\
-384 & 1146 & -3744 & -3744 & 1056 & -1464 & -2304 & -2304 & -384 & -1554 & 3456 & 3456 & -864 & 216 & 576 & 576 \\
-1554 & -384 & 2046 & -3744 & -1464 & 1056 & -1464 & -2304 & 1146 & -384 & -2454 & 3456 & 216 & -864 & 216 & 576 \\
3456 & -2454 & -384 & 1146 & -2304 & -1464 & 1056 & -1464 & -3744 & 2046 & -384 & -1554 & 576 & 216 & -864 & 216 \\
3456 & 3456 & -1554 & -384 & -2304 & -2304 & -1464 & 1056 & -3744 & -3744 & 1146 & -384 & 576 & 576 & 216 & -864 \\
-864 & 216 & 576 & 576 & -384 & 1146 & -3744 & -3744 & 1056 & -1464 & -2304 & -2304 & -384 & -1554 & 3456 & 3456 \\
216 & -864 & 216 & 576 & -1554 & -384 & 2046 & -3744 & -1464 & 1056 & -1464 & -2304 & 1146 & -384 & -2454 & 3456 \\
576 & 216 & -864 & 216 & 3456 & -2454 & -384 & 1146 & -2304 & -1464 & 1056 & -1464 & -3744 & 2046 & -384 & -1554 \\
576 & 576 & 216 & -864 & 3456 & 3456 & -1554 & -384 & -2304 & -2304 & -1464 & 1056 & -3744 & -3744 & 1146 & -384 \\
-864 & 216 & 576 & 576 & -864 & 216 & 576 & 576 & -384 & 1146 & -3744 & -3744 & 1056 & -1464 & -2304 & -2304 \\
216 & -864 & 216 & 576 & 216 & -864 & 216 & 576 & -1554 & -384 & 2046 & -3744 & -1464 & 1056 & -1464 & -2304 \\
576 & 216 & -864 & 216 & 576 & 216 & -864 & 216 & 3456 & -2454 & -384 & 1146 & -2304 & -1464 & 1056 & -1464 \\
576 & 576 & 216 & -864 & 576 & 576 & 216 & -864 & 3456 & 3456 & -1554 & -384 & -2304 & -2304 & -1464 & 1056
\end{pmatrix}$$

$\mathbf{S = \{1342, 1423, 2314, 2431, 3124, 3241, 4132, 4213\}}, \lambda_{max} = -0.009351, \lambda_{min} = -0.136488$

$$H_S = \frac{1}{6 \cdot 5^6} \times \begin{pmatrix}
-4992 & 48 & 1728 & 1728 & 48 & -312 & -432 & -432 & 1728 & -432 & -1152 & -1152 & 1728 & -432 & -1152 & -1152 \\
48 & -4992 & 48 & 1728 & -312 & 48 & -312 & -432 & -432 & 1728 & -432 & -1152 & -432 & 1728 & -432 & -1152 \\
1728 & 48 & -4992 & 48 & -432 & -312 & 48 & -312 & -1152 & -432 & 1728 & -432 & -1152 & -432 & 1728 & -432 \\
1728 & 1728 & 48 & -4992 & -432 & -432 & -312 & 48 & -1152 & -1152 & -432 & 1728 & -1152 & -1152 & -432 & 1728 \\
48 & -312 & -432 & -432 & -4992 & 48 & 1728 & 1728 & 48 & -312 & -432 & -432 & 1728 & -432 & -1152 & -1152 \\
-312 & 48 & -312 & -432 & 48 & -4992 & 48 & 1728 & -312 & 48 & -312 & -432 & -432 & 1728 & -432 & -1152 \\
-432 & -312 & 48 & -312 & 1728 & 48 & -4992 & 48 & -432 & -312 & 48 & -312 & -1152 & -432 & 1728 & -432 \\
-432 & -432 & -312 & 48 & 1728 & 1728 & 48 & -4992 & -432 & -432 & -312 & 48 & -1152 & -1152 & -432 & 1728 \\
1728 & -432 & -1152 & -1152 & 48 & -312 & -432 & -432 & -4992 & 48 & 1728 & 1728 & 48 & -312 & -432 & -432 \\
-432 & 1728 & -432 & -1152 & -312 & 48 & -312 & -432 & 48 & -4992 & 48 & 1728 & -312 & 48 & -312 & -432 \\
-1152 & -432 & 1728 & -432 & -432 & -312 & 48 & -312 & 1728 & 48 & -4992 & 48 & -432 & -312 & 48 & -312 \\
-1152 & -1152 & -432 & 1728 & -432 & -432 & -312 & 48 & 1728 & 1728 & 48 & -4992 & -432 & -432 & -312 & 48 \\
1728 & -432 & -1152 & -1152 & 1728 & -432 & -1152 & -1152 & 48 & -312 & -432 & -432 & -4992 & 48 & 1728 & 1728 \\
-432 & 1728 & -432 & -1152 & -432 & 1728 & -432 & -1152 & -312 & 48 & -312 & -432 & 48 & -4992 & 48 & 1728 \\
-1152 & -432 & 1728 & -432 & -1152 & -432 & 1728 & -432 & -432 & -312 & 48 & -312 & 1728 & 48 & -4992 & 48 \\
-1152 & -1152 & -432 & 1728 & -1152 & -1152 & -432 & 1728 & -432 & -432 & -312 & 48 & 1728 & 1728 & 48 & -4992
\end{pmatrix}$$

$S = \{1342, 1423, 2314, 2431, 3214, 3241, 4123, 4132\}, \lambda_{max} = 0.040452, \lambda_{min} = -0.071812$

$$H_S = \frac{1}{6 \cdot 5^6} \times \begin{pmatrix}
-1536 & -816 & -576 & -576 & 264 & -906 & 864 & 864 & 864 & -216 & -576 & -576 & 864 & -216 & -576 & -576 \\
-816 & -1536 & -816 & -576 & 174 & 264 & -1266 & 864 & -216 & 864 & -216 & -576 & -216 & 864 & -216 & -576 \\
-576 & -816 & -1536 & -816 & -2016 & 534 & 264 & -906 & -576 & -216 & 864 & -216 & -576 & -216 & 864 & -216 \\
-576 & -576 & -816 & -1536 & -2016 & -2016 & 174 & 264 & -576 & -576 & -216 & 864 & -576 & -576 & -216 & 864 \\
264 & 174 & -2016 & -2016 & -1536 & -816 & -576 & -576 & 264 & -366 & -576 & -576 & 864 & -216 & -576 & -576 \\
-906 & 264 & 534 & -2016 & -816 & -1536 & -816 & -576 & -366 & 264 & -366 & -576 & -216 & 864 & -216 & -576 \\
864 & -1266 & 264 & 174 & -576 & -816 & -1536 & -816 & -576 & -366 & 264 & -366 & -576 & -216 & 864 & -216 \\
864 & 864 & -906 & 264 & -576 & -576 & -816 & -1536 & -576 & -576 & -366 & 264 & -576 & -576 & -216 & 864 \\
864 & -216 & -576 & -576 & 264 & -366 & -576 & -576 & -1536 & -816 & -576 & -576 & 264 & 174 & -2016 & -2016 \\
-216 & 864 & -216 & -576 & -366 & 264 & -366 & -576 & -816 & -1536 & -816 & -576 & -906 & 264 & 534 & -2016 \\
-576 & -216 & 864 & -216 & -576 & -366 & 264 & -366 & -576 & -816 & -1536 & -816 & 864 & -1266 & 264 & 174 \\
-576 & -576 & -216 & 864 & -576 & -576 & -366 & 264 & -576 & -576 & -816 & -1536 & 864 & 864 & -906 & 264 \\
864 & -216 & -576 & -576 & 864 & -216 & -576 & -576 & 264 & -906 & 864 & 864 & -1536 & -816 & -576 & -576 \\
-216 & 864 & -216 & -576 & -216 & 864 & -216 & -576 & 174 & 264 & -1266 & 864 & -816 & -1536 & -816 & -576 \\
-576 & -216 & 864 & -216 & -576 & -216 & 864 & -216 & -2016 & 534 & 264 & -906 & -576 & -816 & -1536 & -816 \\
-576 & -576 & -216 & 864 & -576 & -576 & -216 & 864 & -2016 & -2016 & 174 & 264 & -576 & -576 & -816 & -1536
\end{pmatrix}$$

$S = \{1342, 1432, 2341, 2431, 3124, 3214, 4123, 4213\}, \lambda_{max} = 0.083022, \lambda_{min} = -0.074297$

$$H_S = \frac{1}{6 \cdot 5^6} \times \begin{pmatrix}
1920 & 480 & 0 & 0 & -1680 & -420 & 0 & 0 & -2880 & -720 & 0 & 0 & -2880 & -720 & 0 & 0 \\
480 & 1920 & 480 & 0 & -420 & -1680 & -420 & 0 & -720 & -2880 & -720 & 0 & -720 & -2880 & -720 & 0 \\
0 & 480 & 1920 & 480 & 0 & -420 & -1680 & -420 & 0 & -720 & -2880 & -720 & 0 & -720 & -2880 & -720 \\
0 & 0 & 480 & 1920 & 0 & 0 & -420 & -1680 & 0 & 0 & -720 & -2880 & 0 & 0 & -720 & -2880 \\
-1680 & -420 & 0 & 0 & 1920 & 480 & 0 & 0 & -1680 & -420 & 0 & 0 & -2880 & -720 & 0 & 0 \\
-420 & -1680 & -420 & 0 & 480 & 1920 & 480 & 0 & -420 & -1680 & -420 & 0 & -720 & -2880 & -720 & 0 \\
0 & -420 & -1680 & -420 & 0 & 480 & 1920 & 480 & 0 & -420 & -1680 & -420 & 0 & -720 & -2880 & -720 \\
0 & 0 & -420 & -1680 & 0 & 0 & 480 & 1920 & 0 & 0 & -420 & -1680 & 0 & 0 & -720 & -2880 \\
-2880 & -720 & 0 & 0 & -1680 & -420 & 0 & 0 & 1920 & 480 & 0 & 0 & -1680 & -420 & 0 & 0 \\
-720 & -2880 & -720 & 0 & -420 & -1680 & -420 & 0 & 480 & 1920 & 480 & 0 & -420 & -1680 & -420 & 0 \\
0 & -720 & -2880 & -720 & 0 & -420 & -1680 & -420 & 0 & 480 & 1920 & 480 & 0 & -420 & -1680 & -420 \\
0 & 0 & -720 & -2880 & 0 & 0 & -420 & -1680 & 0 & 0 & 480 & 1920 & 0 & 0 & -420 & -1680 \\
-2880 & -720 & 0 & 0 & -2880 & -720 & 0 & 0 & -1680 & -420 & 0 & 0 & 1920 & 480 & 0 & 0 \\
-720 & -2880 & -720 & 0 & -720 & -2880 & -720 & 0 & -420 & -1680 & -420 & 0 & 480 & 1920 & 480 & 0 \\
0 & -720 & -2880 & -720 & 0 & -720 & -2880 & -720 & 0 & -420 & -1680 & -420 & 0 & 480 & 1920 & 480 \\
0 & 0 & -720 & -2880 & 0 & 0 & -720 & -2880 & 0 & 0 & -420 & -1680 & 0 & 0 & 480 & 1920
\end{pmatrix}$$

# Appendix 4

$\mathbf{S} = \{\mathbf{1234}, \mathbf{1243}, \mathbf{1324}, \mathbf{2134}, \mathbf{2143}, \mathbf{2413}, \mathbf{3142}, \mathbf{3412}, \mathbf{3421}, \mathbf{4231}, \mathbf{4312}, \mathbf{4321}\}, \lambda_{max} = 0.098304, \lambda_{min} = 0$

$$H_S = \frac{1}{6 \cdot 5^6} \times \begin{pmatrix}
576 & 576 & 576 & 576 & 576 & 576 & 576 & 576 & 576 & 576 & 576 & 576 & 576 & 576 & 576 & 576 \\
576 & 576 & 576 & 576 & 576 & 576 & 576 & 576 & 576 & 576 & 576 & 576 & 576 & 576 & 576 & 576 \\
576 & 576 & 576 & 576 & 576 & 576 & 576 & 576 & 576 & 576 & 576 & 576 & 576 & 576 & 576 & 576 \\
576 & 576 & 576 & 576 & 576 & 576 & 576 & 576 & 576 & 576 & 576 & 576 & 576 & 576 & 576 & 576 \\
576 & 576 & 576 & 576 & 576 & 576 & 576 & 576 & 576 & 576 & 576 & 576 & 576 & 576 & 576 & 576 \\
576 & 576 & 576 & 576 & 576 & 576 & 576 & 576 & 576 & 576 & 576 & 576 & 576 & 576 & 576 & 576 \\
576 & 576 & 576 & 576 & 576 & 576 & 576 & 576 & 576 & 576 & 576 & 576 & 576 & 576 & 576 & 576 \\
576 & 576 & 576 & 576 & 576 & 576 & 576 & 576 & 576 & 576 & 576 & 576 & 576 & 576 & 576 & 576 \\
576 & 576 & 576 & 576 & 576 & 576 & 576 & 576 & 576 & 576 & 576 & 576 & 576 & 576 & 576 & 576 \\
576 & 576 & 576 & 576 & 576 & 576 & 576 & 576 & 576 & 576 & 576 & 576 & 576 & 576 & 576 & 576 \\
576 & 576 & 576 & 576 & 576 & 576 & 576 & 576 & 576 & 576 & 576 & 576 & 576 & 576 & 576 & 576 \\
576 & 576 & 576 & 576 & 576 & 576 & 576 & 576 & 576 & 576 & 576 & 576 & 576 & 576 & 576 & 576 \\
576 & 576 & 576 & 576 & 576 & 576 & 576 & 576 & 576 & 576 & 576 & 576 & 576 & 576 & 576 & 576 \\
576 & 576 & 576 & 576 & 576 & 576 & 576 & 576 & 576 & 576 & 576 & 576 & 576 & 576 & 576 & 576 \\
576 & 576 & 576 & 576 & 576 & 576 & 576 & 576 & 576 & 576 & 576 & 576 & 576 & 576 & 576 & 576 \\
576 & 576 & 576 & 576 & 576 & 576 & 576 & 576 & 576 & 576 & 576 & 576 & 576 & 576 & 576 & 576
\end{pmatrix}$$

$S = \{1234, 1243, 1324, 2134, 2143, 2413, 3241, 3412, 3421, 4132, 4312, 4321\}, \lambda_{max} = 0.111466, \lambda_{min} = -0.105168$

$$H_S = \frac{1}{6 \cdot 5^6} \times \begin{pmatrix}
1440 & 360 & 0 & 0 & 1440 & -990 & 3600 & 3600 & 1440 & 360 & 0 & 0 & 1440 & 360 & 0 & 0 \\
360 & 1440 & 360 & 0 & 1710 & 1440 & -1890 & 3600 & 360 & 1440 & 360 & 0 & 360 & 1440 & 360 & 0 \\
0 & 360 & 1440 & 360 & -3600 & 2610 & 1440 & -990 & 0 & 360 & 1440 & 360 & 0 & 360 & 1440 & 360 \\
0 & 0 & 360 & 1440 & -3600 & -3600 & 1710 & 1440 & 0 & 0 & 360 & 1440 & 0 & 0 & 360 & 1440 \\
1440 & 1710 & -3600 & -3600 & 1440 & 360 & 0 & 0 & 1440 & -990 & 3600 & 3600 & 1440 & 360 & 0 & 0 \\
-990 & 1440 & 2610 & -3600 & 360 & 1440 & 360 & 0 & 1710 & 1440 & -1890 & 3600 & 360 & 1440 & 360 & 0 \\
3600 & -1890 & 1440 & 1710 & 0 & 360 & 1440 & 360 & -3600 & 2610 & 1440 & -990 & 0 & 360 & 1440 & 360 \\
3600 & 3600 & -990 & 1440 & 0 & 0 & 360 & 1440 & -3600 & -3600 & 1710 & 1440 & 0 & 0 & 360 & 1440 \\
1440 & 360 & 0 & 0 & 1440 & 1710 & -3600 & -3600 & 1440 & 360 & 0 & 0 & 1440 & -990 & 3600 & 3600 \\
360 & 1440 & 360 & 0 & -990 & 1440 & 2610 & -3600 & 360 & 1440 & 360 & 0 & 1710 & 1440 & -1890 & 3600 \\
0 & 360 & 1440 & 360 & 3600 & -1890 & 1440 & 1710 & 0 & 360 & 1440 & 360 & -3600 & 2610 & 1440 & -990 \\
0 & 0 & 360 & 1440 & 3600 & 3600 & -990 & 1440 & 0 & 0 & 360 & 1440 & -3600 & -3600 & 1710 & 1440 \\
1440 & 360 & 0 & 0 & 1440 & 360 & 0 & 0 & 1440 & 1710 & -3600 & -3600 & 1440 & 360 & 0 & 0 \\
360 & 1440 & 360 & 0 & 360 & 1440 & 360 & 0 & -990 & 1440 & 2610 & -3600 & 360 & 1440 & 360 & 0 \\
0 & 360 & 1440 & 360 & 0 & 360 & 1440 & 360 & 3600 & -1890 & 1440 & 1710 & 0 & 360 & 1440 & 360 \\
0 & 0 & 360 & 1440 & 0 & 0 & 360 & 1440 & 3600 & 3600 & -990 & 1440 & 0 & 0 & 360 & 1440
\end{pmatrix}$$

$S = \{1234, 1243, 1324, 2134, 2341, 2413, 3142, 3412, 3421, 4123, 4231, 4312\}, \lambda_{max} = 0.616484, \lambda_{min} = -0.315971$

$$H_S = \frac{1}{6 \cdot 5^6} \times \begin{pmatrix}
288 & 288 & 288 & 288 & 288 & 11538 & 288 & 288 & 288 & 288 & 288 & 288 & 288 & 288 & 288 & 288 \\
288 & 288 & 288 & 288 & -10962 & 288 & 11538 & 288 & 288 & 288 & 288 & 288 & 288 & 288 & 288 & 288 \\
288 & 288 & 288 & 288 & 288 & -10962 & 288 & 11538 & 288 & 288 & 288 & 288 & 288 & 288 & 288 & 288 \\
288 & 288 & 288 & 288 & 288 & 288 & -10962 & 288 & 288 & 288 & 288 & 288 & 288 & 288 & 288 & 288 \\
288 & -10962 & 288 & 288 & 288 & 288 & 288 & 288 & 288 & 11538 & 288 & 288 & 288 & 288 & 288 & 288 \\
11538 & 288 & -10962 & 288 & 288 & 288 & 288 & 288 & -10962 & 288 & 11538 & 288 & 288 & 288 & 288 & 288 \\
288 & 11538 & 288 & -10962 & 288 & 288 & 288 & 288 & 288 & -10962 & 288 & 11538 & 288 & 288 & 288 & 288 \\
288 & 288 & 11538 & 288 & 288 & 288 & 288 & 288 & 288 & 288 & -10962 & 288 & 288 & 288 & 288 & 288 \\
288 & 288 & 288 & 288 & 288 & -10962 & 288 & 288 & 288 & 288 & 288 & 288 & 288 & 11538 & 288 & 288 \\
288 & 288 & 288 & 288 & 11538 & 288 & -10962 & 288 & 288 & 288 & 288 & 288 & -10962 & 288 & 11538 & 288 \\
288 & 288 & 288 & 288 & 288 & 11538 & 288 & -10962 & 288 & 288 & 288 & 288 & 288 & -10962 & 288 & 11538 \\
288 & 288 & 288 & 288 & 288 & 288 & 11538 & 288 & 288 & 288 & 288 & 288 & 288 & 288 & -10962 & 288 \\
288 & 288 & 288 & 288 & 288 & 288 & 288 & 288 & 288 & -10962 & 288 & 288 & 288 & 288 & 288 & 288 \\
288 & 288 & 288 & 288 & 288 & 288 & 288 & 288 & 11538 & 288 & -10962 & 288 & 288 & 288 & 288 & 288 \\
288 & 288 & 288 & 288 & 288 & 288 & 288 & 288 & 288 & 11538 & 288 & -10962 & 288 & 288 & 288 & 288 \\
288 & 288 & 288 & 288 & 288 & 288 & 288 & 288 & 288 & 288 & 11538 & 288 & 288 & 288 & 288 & 288
\end{pmatrix}$$

$S = \{1234, 1243, 1324, 2134, 2341, 2413, 3142, 3412, 3421, 4132, 4213, 4321\}, \lambda_{max} = 0.159228, \lambda_{min} = -0.175436$

$$H_S = \frac{1}{6 \cdot 5^6} \times \begin{pmatrix}
288 & 288 & 288 & 288 & 288 & 5382 & 1584 & 1584 & 288 & 3024 & -288 & -288 & 288 & 3024 & -288 & -288 \\
288 & 288 & 288 & 288 & -4806 & 288 & 6678 & 1584 & -2448 & 288 & 2448 & -288 & -2448 & 288 & 2448 & -288 \\
288 & 288 & 288 & 288 & -1008 & -6102 & 288 & 8622 & 864 & -1872 & 288 & 1584 & 864 & -1872 & 288 & 1584 \\
288 & 288 & 288 & 288 & -1008 & -1008 & -8046 & 288 & 864 & 864 & -1008 & 288 & 864 & 864 & -1008 & 288 \\
288 & -4806 & -1008 & -1008 & 288 & 288 & 288 & 288 & 288 & 1278 & 2448 & 2448 & 288 & 3024 & -288 & -288 \\
5382 & 288 & -6102 & -1008 & 288 & 288 & 288 & 288 & -702 & 288 & 3438 & 2448 & -2448 & 288 & 2448 & -288 \\
1584 & 6678 & 288 & -8046 & 288 & 288 & 288 & 288 & -1872 & -2862 & 288 & 6678 & 864 & -1872 & 288 & 1584 \\
1584 & 1584 & 8622 & 288 & 288 & 288 & 288 & 288 & -1872 & -1872 & -6102 & 288 & 864 & 864 & -1008 & 288 \\
288 & -2448 & 864 & 864 & 288 & -702 & -1872 & -1872 & 288 & 288 & 288 & 288 & 288 & -1458 & 3024 & 3024 \\
3024 & 288 & -1872 & 864 & 1278 & 288 & -2862 & -1872 & 288 & 288 & 288 & 288 & 2034 & 288 & 1278 & 3024 \\
-288 & 2448 & 288 & -1008 & 2448 & 3438 & 288 & -6102 & 288 & 288 & 288 & 288 & -2448 & -702 & 288 & 5382 \\
-288 & -288 & 1584 & 288 & 2448 & 2448 & 6678 & 288 & 288 & 288 & 288 & 288 & -2448 & -2448 & -4806 & 288 \\
288 & -2448 & 864 & 864 & 288 & -2448 & 864 & 864 & 288 & 2034 & -2448 & -2448 & 288 & 288 & 288 & 288 \\
3024 & 288 & -1872 & 864 & 3024 & 288 & -1872 & 864 & -1458 & 288 & -702 & -2448 & 288 & 288 & 288 & 288 \\
-288 & 2448 & 288 & -1008 & -288 & 2448 & 288 & -1008 & 3024 & 1278 & 288 & -4806 & 288 & 288 & 288 & 288 \\
-288 & -288 & 1584 & 288 & -288 & -288 & 1584 & 288 & 3024 & 3024 & 5382 & 288 & 288 & 288 & 288 & 288
\end{pmatrix}$$

$S = \{1234, 1243, 1324, 2134, 2341, 2413, 3241, 3412, 3421, 4123, 4132, 4312\}, \lambda_{max} = 0.282791, \lambda_{min} = -0.279046$

$$H_S = \frac{1}{6 \cdot 5^6} \times \begin{pmatrix}
1152 & 72 & -288 & -288 & 1152 & 9972 & 3312 & 3312 & 1152 & 72 & -288 & -288 & 1152 & 72 & -288 & -288 \\
72 & 1152 & 72 & -288 & -9828 & 1152 & 9072 & 3312 & 72 & 1152 & 72 & -288 & 72 & 1152 & 72 & -288 \\
-288 & 72 & 1152 & 72 & -3888 & -8928 & 1152 & 9972 & -288 & 72 & 1152 & 72 & -288 & 72 & 1152 & 72 \\
-288 & -288 & 72 & 1152 & -3888 & -3888 & -9828 & 1152 & -288 & -288 & 72 & 1152 & -288 & -288 & 72 & 1152 \\
1152 & -9828 & -3888 & -3888 & 1152 & 72 & -288 & -288 & 1152 & 9972 & 3312 & 3312 & 1152 & 72 & -288 & -288 \\
9972 & 1152 & -8928 & -3888 & 72 & 1152 & 72 & -288 & -9828 & 1152 & 9072 & 3312 & 72 & 1152 & 72 & -288 \\
3312 & 9072 & 1152 & -9828 & -288 & 72 & 1152 & 72 & -3888 & -8928 & 1152 & 9972 & -288 & 72 & 1152 & 72 \\
3312 & 3312 & 9972 & 1152 & -288 & -288 & 72 & 1152 & -3888 & -3888 & -9828 & 1152 & -288 & -288 & 72 & 1152 \\
1152 & 72 & -288 & -288 & 1152 & -9828 & -3888 & -3888 & 1152 & 72 & -288 & -288 & 1152 & 9972 & 3312 & 3312 \\
72 & 1152 & 72 & -288 & 9972 & 1152 & -8928 & -3888 & 72 & 1152 & 72 & -288 & -9828 & 1152 & 9072 & 3312 \\
-288 & 72 & 1152 & 72 & 3312 & 9072 & 1152 & -9828 & -288 & 72 & 1152 & 72 & -3888 & -8928 & 1152 & 9972 \\
-288 & -288 & 72 & 1152 & 3312 & 3312 & 9972 & 1152 & -288 & -288 & 72 & 1152 & -3888 & -3888 & -9828 & 1152 \\
1152 & 72 & -288 & -288 & 1152 & 72 & -288 & -288 & 1152 & -9828 & -3888 & -3888 & 1152 & 72 & -288 & -288 \\
72 & 1152 & 72 & -288 & 72 & 1152 & 72 & -288 & 9972 & 1152 & -8928 & -3888 & 72 & 1152 & 72 & -288 \\
-288 & 72 & 1152 & 72 & -288 & 72 & 1152 & 72 & 3312 & 9072 & 1152 & -9828 & -288 & 72 & 1152 & 72 \\
-288 & -288 & 72 & 1152 & -288 & -288 & 72 & 1152 & 3312 & 3312 & 9972 & 1152 & -288 & -288 & 72 & 1152
\end{pmatrix}$$

$S = \{1234, 1243, 1324, 2143, 2314, 2413, 3142, 3412, 3421, 4132, 4231, 4321\}, \lambda_{max} = 0.086137, \lambda_{min} = -0.090020$

$$H_S = \frac{1}{6 \cdot 5^6} \times \begin{pmatrix}
-576 & -576 & -576 & -576 & 504 & 5004 & 504 & 504 & 864 & 864 & 864 & 864 & 864 & 864 & 864 & 864 \\
-576 & -576 & -576 & -576 & -3996 & 504 & 5004 & 504 & 864 & 864 & 864 & 864 & 864 & 864 & 864 & 864 \\
-576 & -576 & -576 & -576 & 504 & -3996 & 504 & 5004 & 864 & 864 & 864 & 864 & 864 & 864 & 864 & 864 \\
-576 & -576 & -576 & -576 & 504 & 504 & -3996 & 504 & 864 & 864 & 864 & 864 & 864 & 864 & 864 & 864 \\
504 & -3996 & 504 & 504 & -576 & -576 & -576 & -576 & 504 & 504 & 504 & 504 & 864 & 864 & 864 & 864 \\
5004 & 504 & -3996 & 504 & -576 & -576 & -576 & -576 & 504 & 504 & 504 & 504 & 864 & 864 & 864 & 864 \\
504 & 5004 & 504 & -3996 & -576 & -576 & -576 & -576 & 504 & 504 & 504 & 504 & 864 & 864 & 864 & 864 \\
504 & 504 & 5004 & 504 & -576 & -576 & -576 & -576 & 504 & 504 & 504 & 504 & 864 & 864 & 864 & 864 \\
864 & 864 & 864 & 864 & 504 & 504 & 504 & 504 & -576 & -576 & -576 & -576 & 504 & -3996 & 504 & 504 \\
864 & 864 & 864 & 864 & 504 & 504 & 504 & 504 & -576 & -576 & -576 & -576 & 5004 & 504 & -3996 & 504 \\
864 & 864 & 864 & 864 & 504 & 504 & 504 & 504 & -576 & -576 & -576 & -576 & 504 & 5004 & 504 & -3996 \\
864 & 864 & 864 & 864 & 504 & 504 & 504 & 504 & -576 & -576 & -576 & -576 & 504 & 504 & 5004 & 504 \\
864 & 864 & 864 & 864 & 864 & 864 & 864 & 864 & 504 & 5004 & 504 & 504 & -576 & -576 & -576 & -576 \\
864 & 864 & 864 & 864 & 864 & 864 & 864 & 864 & -3996 & 504 & 5004 & 504 & -576 & -576 & -576 & -576 \\
864 & 864 & 864 & 864 & 864 & 864 & 864 & 864 & 504 & -3996 & 504 & 5004 & -576 & -576 & -576 & -576 \\
864 & 864 & 864 & 864 & 864 & 864 & 864 & 864 & 504 & 504 & -3996 & 504 & -576 & -576 & -576 & -576
\end{pmatrix}$$

$S = \{1234, 1243, 1324, 2143, 2314, 2431, 3142, 3412, 3421, 4123, 4231, 4312\}, \lambda_{max} = 0.197607, \lambda_{min} = -0.197364$

$$H_S = \frac{1}{6 \cdot 5^6} \times \begin{pmatrix}
288 & 288 & 288 & 288 & 288 & 9594 & -1008 & -1008 & 288 & 1152 & 864 & 864 & 288 & 1152 & 864 & 864 \\
288 & 288 & 288 & 288 & -9018 & 288 & 8298 & -1008 & -576 & 288 & 1728 & 864 & -576 & 288 & 1728 & 864 \\
288 & 288 & 288 & 288 & 1584 & -7722 & 288 & 6354 & -288 & -1152 & 288 & 2592 & -288 & -1152 & 288 & 2592 \\
288 & 288 & 288 & 288 & 1584 & 1584 & -5778 & 288 & -288 & -288 & -2016 & 288 & -288 & -288 & -2016 & 288 \\
288 & -9018 & 1584 & 1584 & 288 & 288 & 288 & 288 & 288 & 8298 & -1872 & -1872 & 288 & 1152 & 864 & 864 \\
9594 & 288 & -7722 & 1584 & 288 & 288 & 288 & 288 & -7722 & 288 & 6138 & -1872 & -576 & 288 & 1728 & 864 \\
-1008 & 8298 & 288 & -5778 & 288 & 288 & 288 & 288 & 2448 & -5562 & 288 & 2898 & -288 & -1152 & 288 & 2592 \\
-1008 & -1008 & 6354 & 288 & 288 & 288 & 288 & 288 & 2448 & 2448 & -2322 & 288 & -288 & -288 & -2016 & 288 \\
288 & -576 & -288 & -288 & 288 & -7722 & 2448 & 2448 & 288 & 288 & 288 & 288 & 288 & 7434 & -2448 & -2448 \\
1152 & 288 & -1152 & -288 & 8298 & 288 & -5562 & 2448 & 288 & 288 & 288 & 288 & -6858 & 288 & 4698 & -2448 \\
864 & 1728 & 288 & -2016 & -1872 & 6138 & 288 & -2322 & 288 & 288 & 288 & 288 & 3024 & -4122 & 288 & 594 \\
864 & 864 & 2592 & 288 & -1872 & -1872 & 2898 & 288 & 288 & 288 & 288 & 288 & 3024 & 3024 & -18 & 288 \\
288 & -576 & -288 & -288 & 288 & -576 & -288 & -288 & 288 & -6858 & 3024 & 3024 & 288 & 288 & 288 & 288 \\
1152 & 288 & -1152 & -288 & 1152 & 288 & -1152 & -288 & 7434 & 288 & -4122 & 3024 & 288 & 288 & 288 & 288 \\
864 & 1728 & 288 & -2016 & 864 & 1728 & 288 & -2016 & -2448 & 4698 & 288 & -18 & 288 & 288 & 288 & 288 \\
864 & 864 & 2592 & 288 & 864 & 864 & 2592 & 288 & -2448 & -2448 & 594 & 288 & 288 & 288 & 288 & 288
\end{pmatrix}$$

$S = \{1234, 1243, 1324, 2143, 2314, 2431, 3142, 3412, 3421, 4132, 4213, 4321\}, \lambda_{max} = 0.170703, \lambda_{min} = -0.144478$

$$H_S = \frac{1}{6 \cdot 5^6} \times \begin{pmatrix}
288 & 288 & 288 & 288 & 288 & 3438 & 288 & 288 & 288 & 3888 & 288 & 288 & 288 & 3888 & 288 & 288 \\
288 & 288 & 288 & 288 & -2862 & 288 & 3438 & 288 & -3312 & 288 & 3888 & 288 & -3312 & 288 & 3888 & 288 \\
288 & 288 & 288 & 288 & 288 & -2862 & 288 & 3438 & 288 & -3312 & 288 & 3888 & 288 & -3312 & 288 & 3888 \\
288 & 288 & 288 & 288 & 288 & 288 & -2862 & 288 & 288 & 288 & -3312 & 288 & 288 & 288 & -3312 & 288 \\
288 & -2862 & 288 & 288 & 288 & 288 & 288 & 288 & 288 & -1962 & 288 & 288 & 288 & 3888 & 288 & 288 \\
3438 & 288 & -2862 & 288 & 288 & 288 & 288 & 288 & 2538 & 288 & -1962 & 288 & -3312 & 288 & 3888 & 288 \\
288 & 3438 & 288 & -2862 & 288 & 288 & 288 & 288 & 288 & 2538 & 288 & -1962 & 288 & -3312 & 288 & 3888 \\
288 & 288 & 3438 & 288 & 288 & 288 & 288 & 288 & 288 & 288 & 2538 & 288 & 288 & 288 & -3312 & 288 \\
288 & -3312 & 288 & 288 & 288 & 2538 & 288 & 288 & 288 & 288 & 288 & 288 & 288 & -5562 & 288 & 288 \\
3888 & 288 & -3312 & 288 & -1962 & 288 & 2538 & 288 & 288 & 288 & 288 & 288 & 6138 & 288 & -5562 & 288 \\
288 & 3888 & 288 & -3312 & 288 & -1962 & 288 & 2538 & 288 & 288 & 288 & 288 & 288 & 6138 & 288 & -5562 \\
288 & 288 & 3888 & 288 & 288 & 288 & -1962 & 288 & 288 & 288 & 288 & 288 & 288 & 288 & 6138 & 288 \\
288 & -3312 & 288 & 288 & 288 & -3312 & 288 & 288 & 288 & 6138 & 288 & 288 & 288 & 288 & 288 & 288 \\
3888 & 288 & -3312 & 288 & 3888 & 288 & -3312 & 288 & -5562 & 288 & 6138 & 288 & 288 & 288 & 288 & 288 \\
288 & 3888 & 288 & -3312 & 288 & 3888 & 288 & -3312 & 288 & -5562 & 288 & 6138 & 288 & 288 & 288 & 288 \\
288 & 288 & 3888 & 288 & 288 & 288 & 3888 & 288 & 288 & 288 & -5562 & 288 & 288 & 288 & 288 & 288
\end{pmatrix}$$

$S = \{1234, 1243, 1324, 2143, 2314, 2431, 3241, 3412, 3421, 4123, 4132, 4312\}, \lambda_{max} = 0.169430, \lambda_{min} = -0.145079$

$$H_S = \frac{1}{6 \cdot 5^6} \times \begin{pmatrix}
1152 & 72 & -288 & -288 & 1152 & 8028 & 2016 & 2016 & 1152 & 936 & 288 & 288 & 1152 & 936 & 288 & 288 \\
72 & 1152 & 72 & -288 & -7884 & 1152 & 5832 & 2016 & -792 & 1152 & 1512 & 288 & -792 & 1152 & 1512 & 288 \\
-288 & 72 & 1152 & 72 & -2592 & -5688 & 1152 & 4788 & -864 & -1368 & 1152 & 2376 & -864 & -1368 & 1152 & 2376 \\
-288 & -288 & 72 & 1152 & -2592 & -2592 & -4644 & 1152 & -864 & -864 & -2232 & 1152 & -864 & -864 & -2232 & 1152 \\
1152 & -7884 & -2592 & -2592 & 1152 & 72 & -288 & -288 & 1152 & 6732 & 1152 & 1152 & 1152 & 936 & 288 & 288 \\
8028 & 1152 & -5688 & -2592 & 72 & 1152 & 72 & -288 & -6588 & 1152 & 3672 & 1152 & -792 & 1152 & 1512 & 288 \\
2016 & 5832 & 1152 & -4644 & -288 & 72 & 1152 & 72 & -1728 & -3528 & 1152 & 1332 & -864 & -1368 & 1152 & 2376 \\
2016 & 2016 & 4788 & 1152 & -288 & -288 & 72 & 1152 & -1728 & -1728 & -1188 & 1152 & -864 & -864 & -2232 & 1152 \\
1152 & -792 & -864 & -864 & 1152 & -6588 & -1728 & -1728 & 1152 & 72 & -288 & -288 & 1152 & 5868 & 576 & 576 \\
936 & 1152 & -1368 & -864 & 6732 & 1152 & -3528 & -1728 & 72 & 1152 & 72 & -288 & -5724 & 1152 & 2232 & 576 \\
288 & 1512 & 1152 & -2232 & 1152 & 3672 & 1152 & -1188 & -288 & 72 & 1152 & 72 & -1152 & -2088 & 1152 & -972 \\
288 & 288 & 2376 & 1152 & 1152 & 1152 & 1332 & 1152 & -288 & -288 & 72 & 1152 & -1152 & -1152 & 1116 & 1152 \\
1152 & -792 & -864 & -864 & 1152 & -792 & -864 & -864 & 1152 & -5724 & -1152 & -1152 & 1152 & 72 & -288 & -288 \\
936 & 1152 & -1368 & -864 & 936 & 1152 & -1368 & -864 & 5868 & 1152 & -2088 & -1152 & 72 & 1152 & 72 & -288 \\
288 & 1512 & 1152 & -2232 & 288 & 1512 & 1152 & -2232 & 576 & 2232 & 1152 & 1116 & -288 & 72 & 1152 & 72 \\
288 & 288 & 2376 & 1152 & 288 & 288 & 2376 & 1152 & 576 & 576 & -972 & 1152 & -288 & -288 & 72 & 1152
\end{pmatrix}$$

$S = \{1234, 1243, 1324, 2143, 2341, 2431, 3214, 3412, 3421, 4123, 4132, 4312\}, \lambda_{max} = 0.224906, \lambda_{min} = -0.080572$

$$H_S = \frac{1}{6 \cdot 5^6} \times \begin{pmatrix}
4608 & 288 & -1152 & -1152 & 288 & 7434 & 2232 & 2232 & -1152 & 2232 & 864 & 864 & -1152 & 2232 & 864 & 864 \\
288 & 4608 & 288 & -1152 & -7398 & 288 & 5778 & 2232 & -2376 & -1152 & 1368 & 864 & -2376 & -1152 & 1368 & 864 \\
-1152 & 288 & 4608 & 288 & -2376 & -5742 & 288 & 5274 & -288 & -1512 & -1152 & 792 & -288 & -1512 & -1152 & 792 \\
-1152 & -1152 & 288 & 4608 & -2376 & -2376 & -5238 & 288 & -288 & -288 & -936 & -1152 & -288 & -288 & -936 & -1152 \\
288 & -7398 & -2376 & -2376 & 4608 & 288 & -1152 & -1152 & 288 & 5778 & 1368 & 1368 & -1152 & 2232 & 864 & 864 \\
7434 & 288 & -5742 & -2376 & 288 & 4608 & 288 & -1152 & -5742 & 288 & 3618 & 1368 & -2376 & -1152 & 1368 & 864 \\
2232 & 5778 & 288 & -5238 & -1152 & 288 & 4608 & 288 & -1512 & -3582 & 288 & 2178 & -288 & -1512 & -1152 & 792 \\
2232 & 2232 & 5274 & 288 & -1152 & -1152 & 288 & 4608 & -1512 & -1512 & -2142 & 288 & -288 & -288 & -936 & -1152 \\
-1152 & -2376 & -288 & -288 & 288 & -5742 & -1512 & -1512 & 4608 & 288 & -1152 & -1152 & 288 & 5274 & 792 & 792 \\
2232 & -1152 & -1512 & -288 & 5778 & 288 & -3582 & -1512 & 288 & 4608 & 288 & -1152 & -5238 & 288 & 2178 & 792 \\
864 & 1368 & -1152 & -936 & 1368 & 3618 & 288 & -2142 & -1152 & 288 & 4608 & 288 & -936 & -2142 & 288 & -486 \\
864 & 864 & 792 & -1152 & 1368 & 1368 & 2178 & 288 & -1152 & -1152 & 288 & 4608 & -936 & -936 & 522 & 288 \\
-1152 & -2376 & -288 & -288 & -1152 & -2376 & -288 & -288 & 288 & -5238 & -936 & -936 & 4608 & 288 & -1152 & -1152 \\
2232 & -1152 & -1512 & -288 & 2232 & -1152 & -1512 & -288 & 5274 & 288 & -2142 & -936 & 288 & 4608 & 288 & -1152 \\
864 & 1368 & -1152 & -936 & 864 & 1368 & -1152 & -936 & 792 & 2178 & 288 & 522 & -1152 & 288 & 4608 & 288 \\
864 & 864 & 792 & -1152 & 864 & 864 & 792 & -1152 & 792 & 792 & -486 & 288 & -1152 & -1152 & 288 & 4608
\end{pmatrix}$$

$S = \{1234, 1243, 1324, 2143, 2413, 2431, 3142, 3214, 3421, 4132, 4312, 4321\}, \lambda_{max} = 0.233822, \lambda_{min} = -0.272398$

$$H_S = \frac{1}{6 \cdot 5^6} \times \begin{pmatrix}
288 & 288 & 288 & 288 & 288 & -1746 & 2592 & 2592 & 288 & 2592 & 864 & 864 & 288 & 2592 & 864 & 864 \\
288 & 288 & 288 & 288 & 2322 & 288 & -5202 & 2592 & -2016 & 288 & 1728 & 864 & -2016 & 288 & 1728 & 864 \\
288 & 288 & 288 & 288 & -2016 & 5778 & 288 & -7506 & -288 & -1152 & 288 & 1152 & -288 & -1152 & 288 & 1152 \\
288 & 288 & 288 & 288 & -2016 & -2016 & 8082 & 288 & -288 & -288 & -576 & 288 & -288 & -288 & -576 & 288 \\
288 & 2322 & -2016 & -2016 & 288 & 288 & 288 & 288 & 288 & -5202 & 1728 & 1728 & 288 & 2592 & 864 & 864 \\
-1746 & 288 & 5778 & -2016 & 288 & 288 & 288 & 288 & 5778 & 288 & -7362 & 1728 & -2016 & 288 & 1728 & 864 \\
2592 & -5202 & 288 & 8082 & 288 & 288 & 288 & 288 & -1152 & 7938 & 288 & -8802 & -288 & -1152 & 288 & 1152 \\
2592 & 2592 & -7506 & 288 & 288 & 288 & 288 & 288 & -1152 & -1152 & 9378 & 288 & -288 & -288 & -576 & 288 \\
288 & -2016 & -288 & -288 & 288 & 5778 & -1152 & -1152 & 288 & 288 & 288 & 288 & 288 & -7506 & 1152 & 1152 \\
2592 & 288 & -1152 & -288 & -5202 & 288 & 7938 & -1152 & 288 & 288 & 288 & 288 & 8082 & 288 & -8802 & 1152 \\
864 & 1728 & 288 & -576 & 1728 & -7362 & 288 & 9378 & 288 & 288 & 288 & 288 & -576 & 9378 & 288 & -9666 \\
864 & 864 & 1152 & 288 & 1728 & 1728 & -8802 & 288 & 288 & 288 & 288 & 288 & -576 & -576 & 10242 & 288 \\
288 & -2016 & -288 & -288 & 288 & -2016 & -288 & -288 & 288 & 8082 & -576 & -576 & 288 & 288 & 288 & 288 \\
2592 & 288 & -1152 & -288 & 2592 & 288 & -1152 & -288 & -7506 & 288 & 9378 & -576 & 288 & 288 & 288 & 288 \\
864 & 1728 & 288 & -576 & 864 & 1728 & 288 & -576 & 1152 & -8802 & 288 & 10242 & 288 & 288 & 288 & 288 \\
864 & 864 & 1152 & 288 & 864 & 864 & 1152 & 288 & 1152 & 1152 & -9666 & 288 & 288 & 288 & 288 & 288
\end{pmatrix}$$

$S = \{1234, 1243, 1324, 2314, 2341, 2413, 3142, 3412, 3421, 4123, 4132, 4231\}, \lambda_{max} = 0.340363, \lambda_{min} = -0.343459$

$$H_S = \frac{1}{6 \cdot 5^6} \times \begin{pmatrix}
-864 & -864 & -864 & -864 & 216 & 15966 & 216 & 216 & 576 & 576 & 576 & 576 & 576 & 576 & 576 & 576 \\
-864 & -864 & -864 & -864 & -15534 & 216 & 15966 & 216 & 576 & 576 & 576 & 576 & 576 & 576 & 576 & 576 \\
-864 & -864 & -864 & -864 & 216 & -15534 & 216 & 15966 & 576 & 576 & 576 & 576 & 576 & 576 & 576 & 576 \\
-864 & -864 & -864 & -864 & 216 & 216 & -15534 & 216 & 576 & 576 & 576 & 576 & 576 & 576 & 576 & 576 \\
216 & -15534 & 216 & 216 & -864 & -864 & -864 & -864 & 216 & 11466 & 216 & 216 & 576 & 576 & 576 & 576 \\
15966 & 216 & -15534 & 216 & -864 & -864 & -864 & -864 & -11034 & 216 & 11466 & 216 & 576 & 576 & 576 & 576 \\
216 & 15966 & 216 & -15534 & -864 & -864 & -864 & -864 & 216 & -11034 & 216 & 11466 & 576 & 576 & 576 & 576 \\
216 & 216 & 15966 & 216 & -864 & -864 & -864 & -864 & 216 & 216 & -11034 & 216 & 576 & 576 & 576 & 576 \\
576 & 576 & 576 & 576 & 216 & -11034 & 216 & 216 & -864 & -864 & -864 & -864 & 216 & 6966 & 216 & 216 \\
576 & 576 & 576 & 576 & 11466 & 216 & -11034 & 216 & -864 & -864 & -864 & -864 & -6534 & 216 & 6966 & 216 \\
576 & 576 & 576 & 576 & 216 & 11466 & 216 & -11034 & -864 & -864 & -864 & -864 & 216 & -6534 & 216 & 6966 \\
576 & 576 & 576 & 576 & 216 & 216 & 11466 & 216 & -864 & -864 & -864 & -864 & 216 & 216 & -6534 & 216 \\
576 & 576 & 576 & 576 & 576 & 576 & 576 & 576 & 216 & -6534 & 216 & 216 & -864 & -864 & -864 & -864 \\
576 & 576 & 576 & 576 & 576 & 576 & 576 & 576 & 6966 & 216 & -6534 & 216 & -864 & -864 & -864 & -864 \\
576 & 576 & 576 & 576 & 576 & 576 & 576 & 576 & 216 & 6966 & 216 & -6534 & -864 & -864 & -864 & -864 \\
576 & 576 & 576 & 576 & 576 & 576 & 576 & 576 & 216 & 216 & 6966 & 216 & -864 & -864 & -864 & -864
\end{pmatrix}$$

$S = \{1234, 1243, 1324, 2314, 2341, 2431, 3142, 3412, 3421, 4123, 4132, 4213\}, \lambda_{max} = 0.330467, \lambda_{min} = -0.336718$

$$H_S = \frac{1}{6 \cdot 5^6} \times \begin{pmatrix}
0 & 0 & 0 & 0 & 0 & 14400 & 0 & 0 & 0 & 3600 & 0 & 0 & 0 & 3600 & 0 & 0 \\
0 & 0 & 0 & 0 & -14400 & 0 & 14400 & 0 & -3600 & 0 & 3600 & 0 & -3600 & 0 & 3600 & 0 \\
0 & 0 & 0 & 0 & 0 & -14400 & 0 & 14400 & 0 & -3600 & 0 & 3600 & 0 & -3600 & 0 & 3600 \\
0 & 0 & 0 & 0 & 0 & 0 & -14400 & 0 & 0 & 0 & -3600 & 0 & 0 & 0 & -3600 & 0 \\
0 & -14400 & 0 & 0 & 0 & 0 & 0 & 0 & 0 & 9000 & 0 & 0 & 0 & 3600 & 0 & 0 \\
14400 & 0 & -14400 & 0 & 0 & 0 & 0 & 0 & -9000 & 0 & 9000 & 0 & -3600 & 0 & 3600 & 0 \\
0 & 14400 & 0 & -14400 & 0 & 0 & 0 & 0 & 0 & -9000 & 0 & 9000 & 0 & -3600 & 0 & 3600 \\
0 & 0 & 14400 & 0 & 0 & 0 & 0 & 0 & 0 & 0 & -9000 & 0 & 0 & 0 & -3600 & 0 \\
0 & -3600 & 0 & 0 & 0 & -9000 & 0 & 0 & 0 & 0 & 0 & 0 & 0 & 5400 & 0 & 0 \\
3600 & 0 & -3600 & 0 & 9000 & 0 & -9000 & 0 & 0 & 0 & 0 & 0 & -5400 & 0 & 5400 & 0 \\
0 & 3600 & 0 & -3600 & 0 & 9000 & 0 & -9000 & 0 & 0 & 0 & 0 & 0 & -5400 & 0 & 5400 \\
0 & 0 & 3600 & 0 & 0 & 0 & 9000 & 0 & 0 & 0 & 0 & 0 & 0 & 0 & -5400 & 0 \\
0 & -3600 & 0 & 0 & 0 & -3600 & 0 & 0 & 0 & -5400 & 0 & 0 & 0 & 0 & 0 & 0 \\
3600 & 0 & -3600 & 0 & 3600 & 0 & -3600 & 0 & 5400 & 0 & -5400 & 0 & 0 & 0 & 0 & 0 \\
0 & 3600 & 0 & -3600 & 0 & 3600 & 0 & -3600 & 0 & 5400 & 0 & -5400 & 0 & 0 & 0 & 0 \\
0 & 0 & 3600 & 0 & 0 & 0 & 3600 & 0 & 0 & 0 & 5400 & 0 & 0 & 0 & 0 & 0
\end{pmatrix}$$

$S = \{1234, 1243, 1324, 2314, 2413, 2431, 3142, 3241, 3412, 4123, 4132, 4321\}, \lambda_{max} = 0.153466, \lambda_{min} = -0.181586$

$$H_S = \frac{1}{6 \cdot 5^6} \times \begin{pmatrix}
-864 & -864 & -864 & -864 & 216 & 9810 & 2952 & 2952 & 576 & 1872 & 0 & 0 & 576 & 1872 & 0 & 0 \\
-864 & -864 & -864 & -864 & -9378 & 216 & 5706 & 2952 & -720 & 576 & 2736 & 0 & -720 & 576 & 2736 & 0 \\
-864 & -864 & -864 & -864 & -2520 & -5274 & 216 & 2970 & 1152 & -1584 & 576 & 3312 & 1152 & -1584 & 576 & 3312 \\
-864 & -864 & -864 & -864 & -2520 & -2520 & -2538 & 216 & 1152 & 1152 & -2160 & 576 & 1152 & 1152 & -2160 & 576 \\
216 & -9378 & -2520 & -2520 & -864 & -864 & -864 & -864 & 216 & 6606 & 2376 & 2376 & 576 & 1872 & 0 & 0 \\
9810 & 216 & -5274 & -2520 & -864 & -864 & -864 & -864 & -6174 & 216 & 3366 & 2376 & -720 & 576 & 2736 & 0 \\
2952 & 5706 & 216 & -2538 & -864 & -864 & -864 & -864 & -1944 & -2934 & 216 & 1206 & 1152 & -1584 & 576 & 3312 \\
2952 & 2952 & 2970 & 216 & -864 & -864 & -864 & -864 & -1944 & -1944 & -774 & 216 & 1152 & 1152 & -2160 & 576 \\
576 & -720 & 1152 & 1152 & 216 & -6174 & -1944 & -1944 & -864 & -864 & -864 & -864 & 216 & 4050 & 1512 & 1512 \\
1872 & 576 & -1584 & 1152 & 6606 & 216 & -2934 & -1944 & -864 & -864 & -864 & -864 & -3618 & 216 & 2106 & 1512 \\
0 & 2736 & 576 & -2160 & 2376 & 3366 & 216 & -774 & -864 & -864 & -864 & -864 & -1080 & -1674 & 216 & 810 \\
0 & 0 & 3312 & 576 & 2376 & 2376 & 1206 & 216 & -864 & -864 & -864 & -864 & -1080 & -1080 & -378 & 216 \\
576 & -720 & 1152 & 1152 & 576 & -720 & 1152 & 1152 & 216 & -3618 & -1080 & -1080 & -864 & -864 & -864 & -864 \\
1872 & 576 & -1584 & 1152 & 1872 & 576 & -1584 & 1152 & 4050 & 216 & -1674 & -1080 & -864 & -864 & -864 & -864 \\
0 & 2736 & 576 & -2160 & 0 & 2736 & 576 & -2160 & 1512 & 2106 & 216 & -378 & -864 & -864 & -864 & -864 \\
0 & 0 & 3312 & 576 & 0 & 0 & 3312 & 576 & 1512 & 1512 & 810 & 216 & -864 & -864 & -864 & -864
\end{pmatrix}$$

$S = \{1234, 1243, 1324, 2314, 2413, 2431, 3142, 3241, 3421, 4123, 4132, 4312\}, \lambda_{max} = 0.113065, \lambda_{min} = -0.225725$

$$H_S = \frac{1}{6 \cdot 5^6} \times \begin{pmatrix}
-3456 & -216 & 864 & 864 & 864 & 9810 & 2088 & 2088 & 2304 & 1008 & 0 & 0 & 2304 & 1008 & 0 & 0 \\
-216 & -3456 & -216 & 864 & -9702 & 864 & 5814 & 2088 & -720 & 2304 & 1584 & 0 & -720 & 2304 & 1584 & 0 \\
864 & -216 & -3456 & -216 & -2520 & -5706 & 864 & 2970 & -1152 & -1296 & 2304 & 2448 & -1152 & -1296 & 2304 & 2448 \\
864 & 864 & -216 & -3456 & -2520 & -2520 & -2862 & 864 & -1152 & -1152 & -2160 & 2304 & -1152 & -1152 & -2160 & 2304 \\
864 & -9702 & -2520 & -2520 & -3456 & -216 & 864 & 864 & 864 & 6714 & 1224 & 1224 & 2304 & 1008 & 0 & 0 \\
9810 & 864 & -5706 & -2520 & -216 & -3456 & -216 & 864 & -6606 & 864 & 3654 & 1224 & -720 & 2304 & 1584 & 0 \\
2088 & 5814 & 864 & -2862 & 864 & -216 & -3456 & -216 & -1656 & -3546 & 864 & 1314 & -1152 & -1296 & 2304 & 2448 \\
2088 & 2088 & 2970 & 864 & 864 & 864 & -216 & -3456 & -1656 & -1656 & -1206 & 864 & -1152 & -1152 & -2160 & 2304 \\
2304 & -720 & -1152 & -1152 & 864 & -6606 & -1656 & -1656 & -3456 & -216 & 864 & 864 & 864 & 4050 & 648 & 648 \\
1008 & 2304 & -1296 & -1152 & 6714 & 864 & -3546 & -1656 & -216 & -3456 & -216 & 864 & -3942 & 864 & 2214 & 648 \\
0 & 1584 & 2304 & -2160 & 1224 & 3654 & 864 & -1206 & 864 & -216 & -3456 & -216 & -1080 & -2106 & 864 & 810 \\
0 & 0 & 2448 & 2304 & 1224 & 1224 & 1314 & 864 & 864 & 864 & -216 & -3456 & -1080 & -1080 & -702 & 864 \\
2304 & -720 & -1152 & -1152 & 2304 & -720 & -1152 & -1152 & 864 & -3942 & -1080 & -1080 & -3456 & -216 & 864 & 864 \\
1008 & 2304 & -1296 & -1152 & 1008 & 2304 & -1296 & -1152 & 4050 & 864 & -2106 & -1080 & -216 & -3456 & -216 & 864 \\
0 & 1584 & 2304 & -2160 & 0 & 1584 & 2304 & -2160 & 648 & 2214 & 864 & -702 & 864 & -216 & -3456 & -216 \\
0 & 0 & 2448 & 2304 & 0 & 0 & 2448 & 2304 & 648 & 648 & 810 & 864 & 864 & 864 & -216 & -3456
\end{pmatrix}$$

$S = \{1234, 1243, 1324, 2341, 2413, 2431, 3142, 3214, 3412, 4123, 4132, 4321\}, \lambda_{max} = 0.216172, \lambda_{min} = -0.133367$

$$H_S = \frac{1}{6 \cdot 5^6} \times \begin{pmatrix}
2592 & -648 & -1728 & -1728 & -648 & 9216 & 3168 & 3168 & -1728 & 3168 & 576 & 576 & -1728 & 3168 & 576 & 576 \\
-648 & 2592 & -648 & -1728 & -8892 & -648 & 5652 & 3168 & -2304 & -1728 & 2592 & 576 & -2304 & -1728 & 2592 & 576 \\
-1728 & -648 & 2592 & -648 & -2304 & -5328 & -648 & 3456 & 1728 & -1728 & -1728 & 1728 & 1728 & -1728 & -1728 & 1728 \\
-1728 & -1728 & -648 & 2592 & -2304 & -2304 & -3132 & -648 & 1728 & 1728 & -864 & -1728 & 1728 & 1728 & -864 & -1728 \\
-648 & -8892 & -2304 & -2304 & 2592 & -648 & -1728 & -1728 & -648 & 5652 & 2592 & 2592 & -1728 & 3168 & 576 & 576 \\
9216 & -648 & -5328 & -2304 & -648 & 2592 & -648 & -1728 & -5328 & -648 & 3312 & 2592 & -2304 & -1728 & 2592 & 576 \\
3168 & 5652 & -648 & -3132 & -1728 & -648 & 2592 & -648 & -1728 & -2988 & -648 & 2052 & 1728 & -1728 & -1728 & 1728 \\
3168 & 3168 & 3456 & -648 & -1728 & -1728 & -648 & 2592 & -1728 & -1728 & -1728 & -648 & 1728 & 1728 & -864 & -1728 \\
-1728 & -2304 & 1728 & 1728 & -648 & -5328 & -1728 & -1728 & 2592 & -648 & -1728 & -1728 & -648 & 3456 & 1728 & 1728 \\
3168 & -1728 & -1728 & 1728 & 5652 & -648 & -2988 & -1728 & -648 & 2592 & -648 & -1728 & -3132 & -648 & 2052 & 1728 \\
576 & 2592 & -1728 & -864 & 2592 & 3312 & -648 & -1728 & -1728 & -648 & 2592 & -648 & -864 & -1728 & -648 & 1296 \\
576 & 576 & 1728 & -1728 & 2592 & 2592 & 2052 & -648 & -1728 & -1728 & -648 & 2592 & -864 & -864 & -972 & -648 \\
-1728 & -2304 & 1728 & 1728 & -1728 & -2304 & 1728 & 1728 & -648 & -3132 & -864 & -864 & 2592 & -648 & -1728 & -1728 \\
3168 & -1728 & -1728 & 1728 & 3168 & -1728 & -1728 & 1728 & 3456 & -648 & -1728 & -864 & -648 & 2592 & -648 & -1728 \\
576 & 2592 & -1728 & -864 & 576 & 2592 & -1728 & -864 & 1728 & 2052 & -648 & -972 & -1728 & -648 & 2592 & -648 \\
576 & 576 & 1728 & -1728 & 576 & 576 & 1728 & -1728 & 1728 & 1728 & 1296 & -648 & -1728 & -1728 & -648 & 2592
\end{pmatrix}$$

$S = \{1234, 1243, 1324, 2341, 2413, 2431, 3142, 3214, 3421, 4123, 4132, 4312\}, \lambda_{max} = 0.301647, \lambda_{min} = -0.155286$

$$H_S = \frac{1}{6 \cdot 5^6} \times \begin{pmatrix}
0 & 0 & 0 & 0 & 0 & 9216 & 2304 & 2304 & 0 & 2304 & 576 & 576 & 0 & 2304 & 576 & 576 \\
0 & 0 & 0 & 0 & -9216 & 0 & 5760 & 2304 & -2304 & 0 & 1440 & 576 & -2304 & 0 & 1440 & 576 \\
0 & 0 & 0 & 0 & -2304 & -5760 & 0 & 3456 & -576 & -1440 & 0 & 864 & -576 & -1440 & 0 & 864 \\
0 & 0 & 0 & 0 & -2304 & -2304 & -3456 & 0 & -576 & -576 & -864 & 0 & -576 & -576 & -864 & 0 \\
0 & -9216 & -2304 & -2304 & 0 & 0 & 0 & 0 & 0 & 5760 & 1440 & 1440 & 0 & 2304 & 576 & 576 \\
9216 & 0 & -5760 & -2304 & 0 & 0 & 0 & 0 & -5760 & 0 & 3600 & 1440 & -2304 & 0 & 1440 & 576 \\
2304 & 5760 & 0 & -3456 & 0 & 0 & 0 & 0 & -1440 & -3600 & 0 & 2160 & -576 & -1440 & 0 & 864 \\
2304 & 2304 & 3456 & 0 & 0 & 0 & 0 & 0 & -1440 & -1440 & -2160 & 0 & -576 & -576 & -864 & 0 \\
0 & -2304 & -576 & -576 & 0 & -5760 & -1440 & -1440 & 0 & 0 & 0 & 0 & 0 & 3456 & 864 & 864 \\
2304 & 0 & -1440 & -576 & 5760 & 0 & -3600 & -1440 & 0 & 0 & 0 & 0 & -3456 & 0 & 2160 & 864 \\
576 & 1440 & 0 & -864 & 1440 & 3600 & 0 & -2160 & 0 & 0 & 0 & 0 & -864 & -2160 & 0 & 1296 \\
576 & 576 & 864 & 0 & 1440 & 1440 & 2160 & 0 & 0 & 0 & 0 & 0 & -864 & -864 & -1296 & 0 \\
0 & -2304 & -576 & -576 & 0 & -2304 & -576 & -576 & 0 & -3456 & -864 & -864 & 0 & 0 & 0 & 0 \\
2304 & 0 & -1440 & -576 & 2304 & 0 & -1440 & -576 & 3456 & 0 & -2160 & -864 & 0 & 0 & 0 & 0 \\
576 & 1440 & 0 & -864 & 576 & 1440 & 0 & -864 & 864 & 2160 & 0 & -1296 & 0 & 0 & 0 & 0 \\
576 & 576 & 864 & 0 & 576 & 576 & 864 & 0 & 864 & 864 & 1296 & 0 & 0 & 0 & 0 & 0
\end{pmatrix}$$

$\mathbf{S = \{1234, 1243, 1342, 2134, 2143, 2431, 3124, 3412, 3421, 4213, 4312, 4321\}}, \lambda_{max} = 0.141866, \lambda_{min} = 0$

$$H_S = \frac{1}{6 \cdot 5^6} \times \begin{pmatrix}
2304 & 2304 & 2304 & 2304 & 144 & 144 & 144 & 144 & -576 & -576 & -576 & -576 & -576 & -576 & -576 & -576 \\
2304 & 2304 & 2304 & 2304 & 144 & 144 & 144 & 144 & -576 & -576 & -576 & -576 & -576 & -576 & -576 & -576 \\
2304 & 2304 & 2304 & 2304 & 144 & 144 & 144 & 144 & -576 & -576 & -576 & -576 & -576 & -576 & -576 & -576 \\
2304 & 2304 & 2304 & 2304 & 144 & 144 & 144 & 144 & -576 & -576 & -576 & -576 & -576 & -576 & -576 & -576 \\
144 & 144 & 144 & 144 & 2304 & 2304 & 2304 & 2304 & 144 & 144 & 144 & 144 & -576 & -576 & -576 & -576 \\
144 & 144 & 144 & 144 & 2304 & 2304 & 2304 & 2304 & 144 & 144 & 144 & 144 & -576 & -576 & -576 & -576 \\
144 & 144 & 144 & 144 & 2304 & 2304 & 2304 & 2304 & 144 & 144 & 144 & 144 & -576 & -576 & -576 & -576 \\
144 & 144 & 144 & 144 & 2304 & 2304 & 2304 & 2304 & 144 & 144 & 144 & 144 & -576 & -576 & -576 & -576 \\
-576 & -576 & -576 & -576 & 144 & 144 & 144 & 144 & 2304 & 2304 & 2304 & 2304 & 144 & 144 & 144 & 144 \\
-576 & -576 & -576 & -576 & 144 & 144 & 144 & 144 & 2304 & 2304 & 2304 & 2304 & 144 & 144 & 144 & 144 \\
-576 & -576 & -576 & -576 & 144 & 144 & 144 & 144 & 2304 & 2304 & 2304 & 2304 & 144 & 144 & 144 & 144 \\
-576 & -576 & -576 & -576 & 144 & 144 & 144 & 144 & 2304 & 2304 & 2304 & 2304 & 144 & 144 & 144 & 144 \\
-576 & -576 & -576 & -576 & -576 & -576 & -576 & -576 & 144 & 144 & 144 & 144 & 2304 & 2304 & 2304 & 2304 \\
-576 & -576 & -576 & -576 & -576 & -576 & -576 & -576 & 144 & 144 & 144 & 144 & 2304 & 2304 & 2304 & 2304 \\
-576 & -576 & -576 & -576 & -576 & -576 & -576 & -576 & 144 & 144 & 144 & 144 & 2304 & 2304 & 2304 & 2304 \\
-576 & -576 & -576 & -576 & -576 & -576 & -576 & -576 & 144 & 144 & 144 & 144 & 2304 & 2304 & 2304 & 2304
\end{pmatrix}$$

$\mathbf{S = \{1234, 1243, 1342, 2134, 2143, 2431, 3214, 3412, 3421, 4123, 4312, 4321\}}, \lambda_{max} = 0.128209, \lambda_{min} = 0.016661$

$$H_S = \frac{1}{6 \cdot 5^6} \times \begin{pmatrix}
5760 & 1440 & 0 & 0 & 360 & -450 & 1440 & 1440 & -1440 & -360 & 0 & 0 & -1440 & -360 & 0 & 0 \\
1440 & 5760 & 1440 & 0 & 630 & 360 & -810 & 1440 & -360 & -1440 & -360 & 0 & -360 & -1440 & -360 & 0 \\
0 & 1440 & 5760 & 1440 & -1440 & 990 & 360 & -450 & 0 & -360 & -1440 & -360 & 0 & -360 & -1440 & -360 \\
0 & 0 & 1440 & 5760 & -1440 & -1440 & 630 & 360 & 0 & 0 & -360 & -1440 & 0 & 0 & -360 & -1440 \\
360 & 630 & -1440 & -1440 & 5760 & 1440 & 0 & 0 & 360 & 90 & 0 & 0 & -1440 & -360 & 0 & 0 \\
-450 & 360 & 990 & -1440 & 1440 & 5760 & 1440 & 0 & 90 & 360 & 90 & 0 & -360 & -1440 & -360 & 0 \\
1440 & -810 & 360 & 630 & 0 & 1440 & 5760 & 1440 & 0 & 90 & 360 & 90 & 0 & -360 & -1440 & -360 \\
1440 & 1440 & -450 & 360 & 0 & 0 & 1440 & 5760 & 0 & 0 & 90 & 360 & 0 & 0 & -360 & -1440 \\
-1440 & -360 & 0 & 0 & 360 & 90 & 0 & 0 & 5760 & 1440 & 0 & 0 & 360 & 630 & -1440 & -1440 \\
-360 & -1440 & -360 & 0 & 90 & 360 & 90 & 0 & 1440 & 5760 & 1440 & 0 & -450 & 360 & 990 & -1440 \\
0 & -360 & -1440 & -360 & 0 & 90 & 360 & 90 & 0 & 1440 & 5760 & 1440 & 1440 & -810 & 360 & 630 \\
0 & 0 & -360 & -1440 & 0 & 0 & 90 & 360 & 0 & 0 & 1440 & 5760 & 1440 & 1440 & -450 & 360 \\
-1440 & -360 & 0 & 0 & -1440 & -360 & 0 & 0 & 360 & -450 & 1440 & 1440 & 5760 & 1440 & 0 & 0 \\
-360 & -1440 & -360 & 0 & -360 & -1440 & -360 & 0 & 630 & 360 & -810 & 1440 & 1440 & 5760 & 1440 & 0 \\
0 & -360 & -1440 & -360 & 0 & -360 & -1440 & -360 & -1440 & 990 & 360 & -450 & 0 & 1440 & 5760 & 1440 \\
0 & 0 & -360 & -1440 & 0 & 0 & -360 & -1440 & -1440 & -1440 & 630 & 360 & 0 & 0 & 1440 & 5760
\end{pmatrix}$$

$S = \{1234, 1243, 1342, 2134, 2314, 2413, 3241, 3412, 3421, 4123, 4132, 4321\}, \lambda_{max} = 0.191897, \lambda_{min} = -0.188539$

$$H_S = \frac{1}{6 \cdot 5^6} \times \begin{pmatrix}
1152 & 72 & -288 & -288 & 1152 & 6516 & 2448 & 2448 & 1152 & -2232 & -864 & -864 & 1152 & -2232 & -864 & -864 \\
72 & 1152 & 72 & -288 & -6372 & 1152 & 6912 & 2448 & 2376 & 1152 & -1368 & -864 & 2376 & 1152 & -1368 & -864 \\
-288 & 72 & 1152 & 72 & -3024 & -6768 & 1152 & 8676 & 288 & 1512 & 1152 & -792 & 288 & 1512 & 1152 & -792 \\
-288 & -288 & 72 & 1152 & -3024 & -3024 & -8532 & 1152 & 288 & 288 & 936 & 1152 & 288 & 288 & 936 & 1152 \\
1152 & -6372 & -3024 & -3024 & 1152 & 72 & -288 & -288 & 1152 & 4212 & 1872 & 1872 & 1152 & -2232 & -864 & -864 \\
6516 & 1152 & -6768 & -3024 & 72 & 1152 & 72 & -288 & -4068 & 1152 & 5472 & 1872 & 2376 & 1152 & -1368 & -864 \\
2448 & 6912 & 1152 & -8532 & -288 & 72 & 1152 & 72 & -2448 & -5328 & 1152 & 7812 & 288 & 1512 & 1152 & -792 \\
2448 & 2448 & 8676 & 1152 & -288 & -288 & 72 & 1152 & -2448 & -2448 & -7668 & 1152 & 288 & 288 & 936 & 1152 \\
1152 & 2376 & 288 & 288 & 1152 & -4068 & -2448 & -2448 & 1152 & 72 & -288 & -288 & 1152 & 756 & 1008 & 1008 \\
-2232 & 1152 & 1512 & 288 & 4212 & 1152 & -5328 & -2448 & 72 & 1152 & 72 & -288 & -612 & 1152 & 3312 & 1008 \\
-864 & -1368 & 1152 & 936 & 1872 & 5472 & 1152 & -7668 & -288 & 72 & 1152 & 72 & -1584 & -3168 & 1152 & 6516 \\
-864 & -864 & -792 & 1152 & 1872 & 1872 & 7812 & 1152 & -288 & -288 & 72 & 1152 & -1584 & -1584 & -6372 & 1152 \\
1152 & 2376 & 288 & 288 & 1152 & 2376 & 288 & 288 & 1152 & -612 & -1584 & -1584 & 1152 & 72 & -288 & -288 \\
-2232 & 1152 & 1512 & 288 & -2232 & 1152 & 1512 & 288 & 756 & 1152 & -3168 & -1584 & 72 & 1152 & 72 & -288 \\
-864 & -1368 & 1152 & 936 & -864 & -1368 & 1152 & 936 & 1008 & 3312 & 1152 & -6372 & -288 & 72 & 1152 & 72 \\
-864 & -864 & -792 & 1152 & -864 & -864 & -792 & 1152 & 1008 & 1008 & 6516 & 1152 & -288 & -288 & 72 & 1152
\end{pmatrix}$$

$S = \{1234, 1243, 1342, 2134, 2341, 2413, 3124, 3412, 3421, 4123, 4231, 4312\}, \lambda_{max} = 0.395666, \lambda_{min} = -0.392510$

$$H_S = \frac{1}{6 \cdot 5^6} \times \begin{pmatrix} 1152 & 1152 & 1152 & 1152 & 72 & 12672 & 72 & 72 & -288 & -3888 & -288 & -288 & -288 & -3888 & -288 & -288 \\ 1152 & 1152 & 1152 & 1152 & -12528 & 72 & 12672 & 72 & 3312 & -288 & -3888 & -288 & 3312 & -288 & -3888 & -288 \\ 1152 & 1152 & 1152 & 1152 & 72 & -12528 & 72 & 12672 & -288 & 3312 & -288 & -3888 & -288 & 3312 & -288 & -3888 \\ 1152 & 1152 & 1152 & 1152 & 72 & 72 & -12528 & 72 & -288 & -288 & 3312 & -288 & -288 & -288 & 3312 & -288 \\ 72 & -12528 & 72 & 72 & 1152 & 1152 & 1152 & 1152 & 72 & 13572 & 72 & 72 & -288 & -3888 & -288 & -288 \\ 12672 & 72 & -12528 & 72 & 1152 & 1152 & 1152 & 1152 & -13428 & 72 & 13572 & 72 & 3312 & -288 & -3888 & -288 \\ 72 & 12672 & 72 & -12528 & 1152 & 1152 & 1152 & 1152 & 72 & -13428 & 72 & 13572 & -288 & 3312 & -288 & -3888 \\ 72 & 72 & 12672 & 72 & 1152 & 1152 & 1152 & 1152 & 72 & 72 & -13428 & 72 & -288 & -288 & 3312 & -288 \\ -288 & 3312 & -288 & -288 & 72 & -13428 & 72 & 72 & 1152 & 1152 & 1152 & 1152 & 72 & 12672 & 72 & 72 \\ -3888 & -288 & 3312 & -288 & 13572 & 72 & -13428 & 72 & 1152 & 1152 & 1152 & 1152 & -12528 & 72 & 12672 & 72 \\ -288 & -3888 & -288 & 3312 & 72 & 13572 & 72 & -13428 & 1152 & 1152 & 1152 & 1152 & 72 & -12528 & 72 & 12672 \\ -288 & -288 & -3888 & -288 & 72 & 72 & 13572 & 72 & 1152 & 1152 & 1152 & 1152 & 72 & 72 & -12528 & 72 \\ -288 & 3312 & -288 & -288 & -288 & 3312 & -288 & -288 & 72 & -12528 & 72 & 72 & 1152 & 1152 & 1152 & 1152 \\ -3888 & -288 & 3312 & -288 & -3888 & -288 & 3312 & -288 & 12672 & 72 & -12528 & 72 & 1152 & 1152 & 1152 & 1152 \\ -288 & -3888 & -288 & 3312 & -288 & -3888 & -288 & 3312 & 72 & 12672 & 72 & -12528 & 1152 & 1152 & 1152 & 1152 \\ -288 & -288 & -3888 & -288 & -288 & -288 & -3888 & -288 & 72 & 72 & 12672 & 72 & 1152 & 1152 & 1152 & 1152 \end{pmatrix}$$

$S = \{1234, 1243, 1342, 2134, 2341, 2413, 3124, 3412, 3421, 4132, 4213, 4321\}, \lambda_{max} = 0.218679, \lambda_{min} = -0.193620$

$$H_S = \frac{1}{6 \cdot 5^6} \times \begin{pmatrix} 1152 & 1152 & 1152 & 1152 & 72 & 6516 & 1368 & 1368 & -288 & -1152 & -864 & -864 & -288 & -1152 & -864 & -864 \\ 1152 & 1152 & 1152 & 1152 & -6372 & 72 & 7812 & 1368 & 576 & -288 & -1728 & -864 & 576 & -288 & -1728 & -864 \\ 1152 & 1152 & 1152 & 1152 & -1224 & -7668 & 72 & 9756 & 288 & 1152 & -288 & -2592 & 288 & 1152 & -288 & -2592 \\ 1152 & 1152 & 1152 & 1152 & -1224 & -1224 & -9612 & 72 & 288 & 288 & 2016 & -288 & 288 & 288 & 2016 & -288 \\ 72 & -6372 & -1224 & -1224 & 1152 & 1152 & 1152 & 1152 & 72 & 3312 & 2232 & 2232 & -288 & -1152 & -864 & -864 \\ 6516 & 72 & -7668 & -1224 & 1152 & 1152 & 1152 & 1152 & -3168 & 72 & 5472 & 2232 & 576 & -288 & -1728 & -864 \\ 1368 & 7812 & 72 & -9612 & 1152 & 1152 & 1152 & 1152 & -2088 & -5328 & 72 & 8712 & 288 & 1152 & -288 & -2592 \\ 1368 & 1368 & 9756 & 72 & 1152 & 1152 & 1152 & 1152 & -2088 & -2088 & -8568 & 72 & 288 & 288 & 2016 & -288 \\ -288 & 576 & 288 & 288 & 72 & -3168 & -2088 & -2088 & 1152 & 1152 & 1152 & 1152 & 72 & -324 & 2808 & 2808 \\ -1152 & -288 & 1152 & 288 & 3312 & 72 & -5328 & -2088 & 1152 & 1152 & 1152 & 1152 & 468 & 72 & 2412 & 2808 \\ -864 & -1728 & -288 & 2016 & 2232 & 5472 & 72 & -8568 & 1152 & 1152 & 1152 & 1152 & -2664 & -2268 & 72 & 6516 \\ -864 & -864 & -2592 & -288 & 2232 & 2232 & 8712 & 72 & 1152 & 1152 & 1152 & 1152 & -2664 & -2664 & -6372 & 72 \\ -288 & 576 & 288 & 288 & -288 & 576 & 288 & 288 & 72 & 468 & -2664 & -2664 & 1152 & 1152 & 1152 & 1152 \\ -1152 & -288 & 1152 & 288 & -1152 & -288 & 1152 & 288 & -324 & 72 & -2268 & -2664 & 1152 & 1152 & 1152 & 1152 \\ -864 & -1728 & -288 & 2016 & -864 & -1728 & -288 & 2016 & 2808 & 2412 & 72 & -6372 & 1152 & 1152 & 1152 & 1152 \\ -864 & -864 & -2592 & -288 & -864 & -864 & -2592 & -288 & 2808 & 2808 & 6516 & 72 & 1152 & 1152 & 1152 & 1152 \end{pmatrix}$$

$S = \{1234, 1243, 1342, 2134, 2341, 2413, 3214, 3412, 3421, 4123, 4132, 4321\}, \lambda_{max} = 0.270985, \lambda_{min} = -0.136397$

$$H_S = \frac{1}{6 \cdot 5^6} \times \begin{pmatrix} 4608 & 288 & -1152 & -1152 & 288 & 5922 & 2664 & 2664 & -1152 & -936 & -288 & -288 & -1152 & -936 & -288 & -288 \\ 288 & 4608 & 288 & -1152 & -5886 & 288 & 6858 & 2664 & 792 & -1152 & -1512 & -288 & 792 & -1152 & -1512 & -288 \\ -1152 & 288 & 4608 & 288 & -2808 & -6822 & 288 & 9162 & 864 & 1368 & -1152 & -2376 & 864 & 1368 & -1152 & -2376 \\ -1152 & -1152 & 288 & 4608 & -2808 & -2808 & -9126 & 288 & 864 & 864 & 2232 & -1152 & 864 & 864 & 2232 & -1152 \\ 288 & -5886 & -2808 & -2808 & 4608 & 288 & -1152 & -1152 & 288 & 3258 & 2088 & 2088 & -1152 & -936 & -288 & -288 \\ 5922 & 288 & -6822 & -2808 & 288 & 4608 & 288 & -1152 & -3222 & 288 & 5418 & 2088 & 792 & -1152 & -1512 & -288 \\ 2664 & 6858 & 288 & -9126 & -1152 & 288 & 4608 & 288 & -2232 & -5382 & 288 & 8658 & 864 & 1368 & -1152 & -2376 \\ 2664 & 2664 & 9162 & 288 & -1152 & -1152 & 288 & 4608 & -2232 & -2232 & -8622 & 288 & 864 & 864 & 2232 & -1152 \\ -1152 & 792 & 864 & 864 & 288 & -3222 & -2232 & -2232 & 4608 & 288 & -1152 & -1152 & 288 & 162 & 1224 & 1224 \\ -936 & -1152 & 1368 & 864 & 3258 & 288 & -5382 & -2232 & 288 & 4608 & 288 & -1152 & -126 & 288 & 3258 & 1224 \\ -288 & -1512 & -1152 & 2232 & 2088 & 5418 & 288 & -8622 & -1152 & 288 & 4608 & 288 & -1368 & -3222 & 288 & 7002 \\ -288 & -288 & -2376 & -1152 & 2088 & 2088 & 8658 & 288 & -1152 & -1152 & 288 & 4608 & -1368 & -1368 & -6966 & 288 \\ -1152 & 792 & 864 & 864 & -1152 & 792 & 864 & 864 & 288 & -126 & -1368 & -1368 & 4608 & 288 & -1152 & -1152 \\ -936 & -1152 & 1368 & 864 & -936 & -1152 & 1368 & 864 & 162 & 288 & -3222 & -1368 & 288 & 4608 & 288 & -1152 \\ -288 & -1512 & -1152 & 2232 & -288 & -1512 & -1152 & 2232 & 1224 & 3258 & 288 & -6966 & -1152 & 288 & 4608 & 288 \\ -288 & -288 & -2376 & -1152 & -288 & -288 & -2376 & -1152 & 1224 & 1224 & 7002 & 288 & -1152 & -1152 & 288 & 4608 \end{pmatrix}$$

$S = \{1234, 1243, 1342, 2134, 2341, 2431, 3124, 3412, 3421, 4123, 4213, 4312\}, \lambda_{max} = 0.320559, \lambda_{min} = -0.312088$

$$H_S = \frac{1}{6 \cdot 5^6} \times \begin{pmatrix} 2016 & 2016 & 2016 & 2016 & -144 & 11106 & -144 & -144 & -864 & -864 & -864 & -864 & -864 & -864 & -864 & -864 \\ 2016 & 2016 & 2016 & 2016 & -11394 & -144 & 11106 & -144 & -864 & -864 & -864 & -864 & -864 & -864 & -864 & -864 \\ 2016 & 2016 & 2016 & 2016 & -144 & -11394 & -144 & 11106 & -864 & -864 & -864 & -864 & -864 & -864 & -864 & -864 \\ 2016 & 2016 & 2016 & 2016 & -144 & -144 & -11394 & -144 & -864 & -864 & -864 & -864 & -864 & -864 & -864 & -864 \\ -144 & -11394 & -144 & -144 & 2016 & 2016 & 2016 & 2016 & -144 & 11106 & -144 & -144 & -864 & -864 & -864 & -864 \\ 11106 & -144 & -11394 & -144 & 2016 & 2016 & 2016 & 2016 & -11394 & -144 & 11106 & -144 & -864 & -864 & -864 & -864 \\ -144 & 11106 & -144 & -11394 & 2016 & 2016 & 2016 & 2016 & -144 & -11394 & -144 & 11106 & -864 & -864 & -864 & -864 \\ -144 & -144 & 11106 & -144 & 2016 & 2016 & 2016 & 2016 & -144 & -144 & -11394 & -144 & -864 & -864 & -864 & -864 \\ -864 & -864 & -864 & -864 & -144 & -11394 & -144 & -144 & 2016 & 2016 & 2016 & 2016 & -144 & 11106 & -144 & -144 \\ -864 & -864 & -864 & -864 & 11106 & -144 & -11394 & -144 & 2016 & 2016 & 2016 & 2016 & -11394 & -144 & 11106 & -144 \\ -864 & -864 & -864 & -864 & -144 & 11106 & -144 & -11394 & 2016 & 2016 & 2016 & 2016 & -144 & -11394 & -144 & 11106 \\ -864 & -864 & -864 & -864 & -144 & -144 & 11106 & -144 & 2016 & 2016 & 2016 & 2016 & -144 & -144 & -11394 & -144 \\ -864 & -864 & -864 & -864 & -864 & -864 & -864 & -864 & -144 & -11394 & -144 & -144 & 2016 & 2016 & 2016 & 2016 \\ -864 & -864 & -864 & -864 & -864 & -864 & -864 & -864 & 11106 & -144 & -11394 & -144 & 2016 & 2016 & 2016 & 2016 \\ -864 & -864 & -864 & -864 & -864 & -864 & -864 & -864 & -144 & 11106 & -144 & -11394 & 2016 & 2016 & 2016 & 2016 \\ -864 & -864 & -864 & -864 & -864 & -864 & -864 & -864 & -144 & -144 & 11106 & -144 & 2016 & 2016 & 2016 & 2016 \end{pmatrix}$$

$S = \{1234, 1243, 1342, 2134, 2413, 2431, 3124, 3142, 3421, 4213, 4312, 4321\}, \lambda_{max} = 0.094345, \lambda_{min} = -0.106988$

$$H_S = \frac{1}{6 \cdot 5^6} \times \begin{pmatrix} -2304 & 2016 & 3456 & 3456 & -144 & 1926 & 216 & 216 & 576 & -504 & -864 & -864 & 576 & -504 & -864 & -864 \\ 2016 & -2304 & 2016 & 3456 & -1674 & -144 & 126 & 216 & -504 & 576 & -504 & -864 & -504 & 576 & -504 & -864 \\ 3456 & 2016 & -2304 & 2016 & 216 & 126 & -144 & -1674 & -864 & -504 & 576 & -504 & -864 & -504 & 576 & -504 \\ 3456 & 3456 & 2016 & -2304 & 216 & 216 & 1926 & -144 & -864 & -864 & -504 & 576 & -864 & -864 & -504 & 576 \\ -144 & -1674 & 216 & 216 & -2304 & 2016 & 3456 & 3456 & -144 & 126 & 216 & 216 & 576 & -504 & -864 & -864 \\ 1926 & -144 & 126 & 216 & 2016 & -2304 & 2016 & 3456 & 126 & -144 & 126 & 216 & -504 & 576 & -504 & -864 \\ 216 & 126 & -144 & 1926 & 3456 & 2016 & -2304 & 2016 & 216 & 126 & -144 & 126 & -864 & -504 & 576 & -504 \\ 216 & 216 & -1674 & -144 & 3456 & 3456 & 2016 & -2304 & 216 & 216 & 126 & -144 & -864 & -864 & -504 & 576 \\ 576 & -504 & -864 & -864 & -144 & 126 & 216 & 216 & -2304 & 2016 & 3456 & 3456 & -144 & -1674 & 216 & 216 \\ -504 & 576 & -504 & -864 & 126 & -144 & 126 & 216 & 2016 & -2304 & 2016 & 3456 & 1926 & -144 & 126 & 216 \\ -864 & -504 & 576 & -504 & 216 & 126 & -144 & 126 & 3456 & 2016 & -2304 & 2016 & 216 & 126 & -144 & 1926 \\ -864 & -864 & -504 & 576 & 216 & 216 & 126 & -144 & 3456 & 3456 & 2016 & -2304 & 216 & 216 & -1674 & -144 \\ 576 & -504 & -864 & -864 & 576 & -504 & -864 & -864 & -144 & 1926 & 216 & 216 & -2304 & 2016 & 3456 & 3456 \\ -504 & 576 & -504 & -864 & -504 & 576 & -504 & -864 & -1674 & -144 & 126 & 216 & 2016 & -2304 & 2016 & 3456 \\ -864 & -504 & 576 & -504 & -864 & -504 & 576 & -504 & 216 & 126 & -144 & -1674 & 3456 & 2016 & -2304 & 2016 \\ -864 & -864 & -504 & 576 & -864 & -864 & -504 & 576 & 216 & 216 & 1926 & -144 & 3456 & 3456 & 2016 & -2304 \end{pmatrix}$$

$S = \{1234, 1243, 1342, 2134, 2413, 2431, 3142, 3214, 3421, 4123, 4312, 4321\}, \lambda_{max} = 0.080481, \lambda_{min} = -0.030952$

$$H_S = \frac{1}{6 \cdot 5^6} \times \begin{pmatrix} 1152 & 1152 & 1152 & 1152 & 72 & 1332 & 1512 & 1512 & -288 & -288 & -288 & -288 & -288 & -288 & -288 & -288 \\ 1152 & 1152 & 1152 & 1152 & -1188 & 72 & -828 & 1512 & -288 & -288 & -288 & -288 & -288 & -288 & -288 & -288 \\ 1152 & 1152 & 1152 & 1152 & -1368 & 972 & 72 & -2268 & -288 & -288 & -288 & -288 & -288 & -288 & -288 & -288 \\ 1152 & 1152 & 1152 & 1152 & -1368 & -1368 & 2412 & 72 & -288 & -288 & -288 & -288 & -288 & -288 & -288 & -288 \\ 72 & -1188 & -1368 & -1368 & 1152 & 1152 & 1152 & 1152 & 72 & 72 & 72 & 72 & -288 & -288 & -288 & -288 \\ 1332 & 72 & 972 & -1368 & 1152 & 1152 & 1152 & 1152 & 72 & 72 & 72 & 72 & -288 & -288 & -288 & -288 \\ 1512 & -828 & 72 & 2412 & 1152 & 1152 & 1152 & 1152 & 72 & 72 & 72 & 72 & -288 & -288 & -288 & -288 \\ 1512 & 1512 & -2268 & 72 & 1152 & 1152 & 1152 & 1152 & 72 & 72 & 72 & 72 & -288 & -288 & -288 & -288 \\ -288 & -288 & -288 & -288 & 72 & 72 & 72 & 72 & 1152 & 1152 & 1152 & 1152 & 72 & -1188 & -1368 & -1368 \\ -288 & -288 & -288 & -288 & 72 & 72 & 72 & 72 & 1152 & 1152 & 1152 & 1152 & 1332 & 72 & 972 & -1368 \\ -288 & -288 & -288 & -288 & 72 & 72 & 72 & 72 & 1152 & 1152 & 1152 & 1152 & 1512 & -828 & 72 & 2412 \\ -288 & -288 & -288 & -288 & 72 & 72 & 72 & 72 & 1152 & 1152 & 1152 & 1152 & 1512 & 1512 & -2268 & 72 \\ -288 & -288 & -288 & -288 & -288 & -288 & -288 & -288 & 72 & 1332 & 1512 & 1512 & 1152 & 1152 & 1152 & 1152 \\ -288 & -288 & -288 & -288 & -288 & -288 & -288 & -288 & -1188 & 72 & -828 & 1512 & 1152 & 1152 & 1152 & 1152 \\ -288 & -288 & -288 & -288 & -288 & -288 & -288 & -288 & -1368 & 972 & 72 & -2268 & 1152 & 1152 & 1152 & 1152 \\ -288 & -288 & -288 & -288 & -288 & -288 & -288 & -288 & -1368 & -1368 & 2412 & 72 & 1152 & 1152 & 1152 & 1152 \end{pmatrix}$$

$S = \{1234, 1243, 1342, 2143, 2314, 2431, 3124, 3412, 3421, 4123, 4231, 4312\}, \lambda_{max} = 0.262734, \lambda_{min} = -0.260013$

$$H_S = \frac{1}{6 \cdot 5^6} \times \begin{pmatrix} 1152 & 1152 & 1152 & 1152 & 72 & 10728 & -1224 & -1224 & -288 & -3024 & 288 & 288 & -288 & -3024 & 288 & 288 \\ 1152 & 1152 & 1152 & 1152 & -10584 & 72 & 9432 & -1224 & 2448 & -288 & -2448 & 288 & 2448 & -288 & -2448 & 288 \\ 1152 & 1152 & 1152 & 1152 & 1368 & -9288 & 72 & 7488 & -864 & 1872 & -288 & -1584 & -864 & 1872 & -288 & -1584 \\ 1152 & 1152 & 1152 & 1152 & 1368 & 1368 & -7344 & 72 & -864 & -864 & 1008 & -288 & -864 & -864 & 1008 & -288 \\ 72 & -10584 & 1368 & 1368 & 1152 & 1152 & 1152 & 1152 & 72 & 10332 & -2088 & -2088 & -288 & -3024 & 288 & 288 \\ 10728 & 72 & -9288 & 1368 & 1152 & 1152 & 1152 & 1152 & -10188 & 72 & 8172 & -2088 & 2448 & -288 & -2448 & 288 \\ -1224 & 9432 & 72 & -7344 & 1152 & 1152 & 1152 & 1152 & 2232 & -8028 & 72 & 4932 & -864 & 1872 & -288 & -1584 \\ -1224 & -1224 & 7488 & 72 & 1152 & 1152 & 1152 & 1152 & 2232 & 2232 & -4788 & 72 & -864 & -864 & 1008 & -288 \\ -288 & 2448 & -864 & -864 & 72 & -10188 & 2232 & 2232 & 1152 & 1152 & 1152 & 1152 & 72 & 8568 & -2664 & -2664 \\ -3024 & -288 & 1872 & -864 & 10332 & 72 & -8028 & 2232 & 1152 & 1152 & 1152 & 1152 & -8424 & 72 & 5832 & -2664 \\ 288 & -2448 & -288 & 1008 & -2088 & 8172 & 72 & -4788 & 1152 & 1152 & 1152 & 1152 & 2808 & -5688 & 72 & 1728 \\ 288 & 288 & -1584 & -288 & -2088 & -2088 & 4932 & 72 & 1152 & 1152 & 1152 & 1152 & 2808 & 2808 & -1584 & 72 \\ -288 & 2448 & -864 & -864 & -288 & 2448 & -864 & -864 & 72 & -8424 & 2808 & 2808 & 1152 & 1152 & 1152 & 1152 \\ -3024 & -288 & 1872 & -864 & -3024 & -288 & 1872 & -864 & 8568 & 72 & -5688 & 2808 & 1152 & 1152 & 1152 & 1152 \\ 288 & -2448 & -288 & 1008 & 288 & -2448 & -288 & 1008 & -2664 & 5832 & 72 & -1584 & 1152 & 1152 & 1152 & 1152 \\ 288 & 288 & -1584 & -288 & 288 & 288 & -1584 & -288 & -2664 & -2664 & 1728 & 72 & 1152 & 1152 & 1152 & 1152 \end{pmatrix}$$

$S = \{1234, 1243, 1342, 2143, 2314, 2431, 3124, 3412, 3421, 4132, 4213, 4321\}, \lambda_{max} = 0.090020, \lambda_{min} = -0.077083$

$$H_S = \frac{1}{6 \cdot 5^6} \times \begin{pmatrix} 1152 & 1152 & 1152 & 1152 & 72 & 4572 & 72 & 72 & -288 & -288 & -288 & -288 & -288 & -288 & -288 & -288 \\ 1152 & 1152 & 1152 & 1152 & -4428 & 72 & 4572 & 72 & -288 & -288 & -288 & -288 & -288 & -288 & -288 & -288 \\ 1152 & 1152 & 1152 & 1152 & 72 & -4428 & 72 & 4572 & -288 & -288 & -288 & -288 & -288 & -288 & -288 & -288 \\ 1152 & 1152 & 1152 & 1152 & 72 & 72 & -4428 & 72 & -288 & -288 & -288 & -288 & -288 & -288 & -288 & -288 \\ 72 & -4428 & 72 & 72 & 1152 & 1152 & 1152 & 1152 & 72 & 72 & 72 & 72 & -288 & -288 & -288 & -288 \\ 4572 & 72 & -4428 & 72 & 1152 & 1152 & 1152 & 1152 & 72 & 72 & 72 & 72 & -288 & -288 & -288 & -288 \\ 72 & 4572 & 72 & -4428 & 1152 & 1152 & 1152 & 1152 & 72 & 72 & 72 & 72 & -288 & -288 & -288 & -288 \\ 72 & 72 & 4572 & 72 & 1152 & 1152 & 1152 & 1152 & 72 & 72 & 72 & 72 & -288 & -288 & -288 & -288 \\ -288 & -288 & -288 & -288 & 72 & 72 & 72 & 72 & 1152 & 1152 & 1152 & 1152 & 72 & -4428 & 72 & 72 \\ -288 & -288 & -288 & -288 & 72 & 72 & 72 & 72 & 1152 & 1152 & 1152 & 1152 & 4572 & 72 & -4428 & 72 \\ -288 & -288 & -288 & -288 & 72 & 72 & 72 & 72 & 1152 & 1152 & 1152 & 1152 & 72 & 4572 & 72 & -4428 \\ -288 & -288 & -288 & -288 & 72 & 72 & 72 & 72 & 1152 & 1152 & 1152 & 1152 & 72 & 72 & 4572 & 72 \\ -288 & -288 & -288 & -288 & -288 & -288 & -288 & -288 & 72 & 4572 & 72 & 72 & 1152 & 1152 & 1152 & 1152 \\ -288 & -288 & -288 & -288 & -288 & -288 & -288 & -288 & -4428 & 72 & 4572 & 72 & 1152 & 1152 & 1152 & 1152 \\ -288 & -288 & -288 & -288 & -288 & -288 & -288 & -288 & 72 & -4428 & 72 & 4572 & 1152 & 1152 & 1152 & 1152 \\ -288 & -288 & -288 & -288 & -288 & -288 & -288 & -288 & 72 & 72 & -4428 & 72 & 1152 & 1152 & 1152 & 1152 \end{pmatrix}$$

$S = \{1234, 1243, 1342, 2143, 2314, 2431, 3214, 3412, 3421, 4123, 4132, 4321\}, \lambda_{max} = 0.146990, \lambda_{min} = -0.016780$

$$H_S = \frac{1}{6 \cdot 5^6} \times \begin{pmatrix}
4608 & 288 & -1152 & -1152 & 288 & 3978 & 1368 & 1368 & -1152 & -72 & 288 & 288 & -1152 & -72 & 288 & 288 \\
288 & 4608 & 288 & -1152 & -3942 & 288 & 3618 & 1368 & -72 & -1152 & -72 & 288 & -72 & -1152 & -72 & 288 \\
-1152 & 288 & 4608 & 288 & -1512 & -3582 & 288 & 3978 & 288 & -72 & -1152 & -72 & 288 & -72 & -1152 & -72 \\
-1152 & -1152 & 288 & 4608 & -1512 & -1512 & -3942 & 288 & 288 & 288 & -72 & -1152 & 288 & 288 & -72 & -1152 \\
288 & -3942 & -1512 & -1512 & 4608 & 288 & -1152 & -1152 & 288 & 18 & -72 & -72 & -1152 & -72 & 288 & 288 \\
3978 & 288 & -3582 & -1512 & 288 & 4608 & 288 & -1152 & 18 & 288 & 18 & -72 & -72 & -1152 & -72 & 288 \\
1368 & 3618 & 288 & -3942 & -1152 & 288 & 4608 & 288 & -72 & 18 & 288 & 18 & 288 & -72 & -1152 & -72 \\
1368 & 1368 & 3978 & 288 & -1152 & -1152 & 288 & 4608 & -72 & -72 & 18 & 288 & 288 & 288 & -72 & -1152 \\
-1152 & -72 & 288 & 288 & 288 & 18 & -72 & -72 & 4608 & 288 & -1152 & -1152 & 288 & -3942 & -1512 & -1512 \\
-72 & -1152 & -72 & 288 & 18 & 288 & 18 & -72 & 288 & 4608 & 288 & -1152 & 3978 & 288 & -3582 & -1512 \\
288 & -72 & -1152 & -72 & -72 & 18 & 288 & 18 & -1152 & 288 & 4608 & 288 & 1368 & 3618 & 288 & -3942 \\
288 & 288 & -72 & -1152 & -72 & -72 & 18 & 288 & -1152 & -1152 & 288 & 4608 & 1368 & 1368 & 3978 & 288 \\
-1152 & -72 & 288 & 288 & -1152 & -72 & 288 & 288 & 288 & 3978 & 1368 & 1368 & 4608 & 288 & -1152 & -1152 \\
-72 & -1152 & -72 & 288 & -72 & -1152 & -72 & 288 & -3942 & 288 & 3618 & 1368 & 288 & 4608 & 288 & -1152 \\
288 & -72 & -1152 & -72 & 288 & -72 & -1152 & -72 & -1512 & -3582 & 288 & 3978 & -1152 & 288 & 4608 & 288 \\
288 & 288 & -72 & -1152 & 288 & 288 & -72 & -1152 & -1512 & -1512 & -3942 & 288 & -1152 & -1152 & 288 & 4608
\end{pmatrix}$$

$S = \{1234, 1243, 1342, 2314, 2341, 2413, 3124, 3412, 3421, 4123, 4132, 4231\}, \lambda_{max} = 0.587023, \lambda_{min} = -0.411598$

$$H_S = \frac{1}{6 \cdot 5^6} \times \begin{pmatrix}
0 & 0 & 0 & 0 & 0 & 17100 & 0 & 0 & 0 & -3600 & 0 & 0 & 0 & -3600 & 0 & 0 \\
0 & 0 & 0 & 0 & -17100 & 0 & 17100 & 0 & 3600 & 0 & -3600 & 0 & 3600 & 0 & -3600 & 0 \\
0 & 0 & 0 & 0 & 0 & -17100 & 0 & 17100 & 0 & 3600 & 0 & -3600 & 0 & 3600 & 0 & -3600 \\
0 & 0 & 0 & 0 & 0 & 0 & -17100 & 0 & 0 & 0 & 3600 & 0 & 0 & 0 & 3600 & 0 \\
0 & -17100 & 0 & 0 & 0 & 0 & 0 & 0 & 0 & 13500 & 0 & 0 & 0 & -3600 & 0 & 0 \\
17100 & 0 & -17100 & 0 & 0 & 0 & 0 & 0 & -13500 & 0 & 13500 & 0 & 3600 & 0 & -3600 & 0 \\
0 & 17100 & 0 & -17100 & 0 & 0 & 0 & 0 & 0 & -13500 & 0 & 13500 & 0 & 3600 & 0 & -3600 \\
0 & 0 & 17100 & 0 & 0 & 0 & 0 & 0 & 0 & 0 & -13500 & 0 & 0 & 0 & 3600 & 0 \\
0 & 3600 & 0 & 0 & 0 & -13500 & 0 & 0 & 0 & 0 & 0 & 0 & 0 & 8100 & 0 & 0 \\
-3600 & 0 & 3600 & 0 & 13500 & 0 & -13500 & 0 & 0 & 0 & 0 & 0 & -8100 & 0 & 8100 & 0 \\
0 & -3600 & 0 & 3600 & 0 & 13500 & 0 & -13500 & 0 & 0 & 0 & 0 & 0 & -8100 & 0 & 8100 \\
0 & 0 & -3600 & 0 & 0 & 0 & 13500 & 0 & 0 & 0 & 0 & 0 & 0 & 0 & -8100 & 0 \\
0 & 3600 & 0 & 0 & 0 & 3600 & 0 & 0 & 0 & -8100 & 0 & 0 & 0 & 0 & 0 & 0 \\
-3600 & 0 & 3600 & 0 & -3600 & 0 & 3600 & 0 & 8100 & 0 & -8100 & 0 & 0 & 0 & 0 & 0 \\
0 & -3600 & 0 & 3600 & 0 & -3600 & 0 & 3600 & 0 & 8100 & 0 & -8100 & 0 & 0 & 0 & 0 \\
0 & 0 & -3600 & 0 & 0 & 0 & -3600 & 0 & 0 & 0 & 8100 & 0 & 0 & 0 & 0 & 0
\end{pmatrix}$$

$S = \{1234, 1243, 1342, 2314, 2413, 2431, 3124, 3142, 3412, 4123, 4231, 4321\}, \lambda_{max} = 0.242598, \lambda_{min} = -0.244542$

$$H_S = \frac{1}{6 \cdot 5^6} \times \begin{pmatrix}
-864 & 216 & 576 & 576 & -864 & 12510 & -288 & -288 & -864 & -2088 & 0 & 0 & -864 & -2088 & 0 & 0 \\
216 & -864 & 216 & 576 & -12078 & -864 & 9306 & -288 & 2520 & -864 & -1224 & 0 & 2520 & -864 & -1224 & 0 \\
576 & 216 & -864 & 216 & 1440 & -8874 & -864 & 5670 & 1152 & 1656 & -864 & -648 & 1152 & 1656 & -864 & -648 \\
576 & 576 & 216 & -864 & 1440 & 1440 & -5238 & -864 & 1152 & 1152 & 1080 & -864 & 1152 & 1152 & 1080 & -864 \\
-864 & -12078 & 1440 & 1440 & -864 & 216 & 576 & 576 & -864 & 10206 & -864 & -864 & -864 & -2088 & 0 & 0 \\
12510 & -864 & -8874 & 1440 & 216 & -864 & 216 & 576 & -9774 & -864 & 7866 & -864 & 2520 & -864 & -1224 & 0 \\
-288 & 9306 & -864 & -5238 & 576 & 216 & -864 & 216 & 2016 & -7434 & -864 & 4806 & 1152 & 1656 & -864 & -648 \\
-288 & -288 & 5670 & -864 & 576 & 576 & 216 & -864 & 2016 & 2016 & -4374 & -864 & 1152 & 1152 & 1080 & -864 \\
-864 & 2520 & 1152 & 1152 & -864 & -9774 & 2016 & 2016 & -864 & 216 & 576 & 576 & -864 & 6750 & -1728 & -1728 \\
-2088 & -864 & 1656 & 1152 & 10206 & -864 & -7434 & 2016 & 216 & -864 & 216 & 576 & -6318 & -864 & 5706 & -1728 \\
0 & -1224 & -864 & 1080 & -864 & 7866 & -864 & -4374 & 576 & 216 & -864 & 216 & 2880 & -5274 & -864 & 3510 \\
0 & 0 & -648 & -864 & -864 & -864 & 4806 & -864 & 576 & 576 & 216 & -864 & 2880 & 2880 & -3078 & -864 \\
-864 & 2520 & 1152 & 1152 & -864 & 2520 & 1152 & 1152 & -864 & -6318 & 2880 & 2880 & -864 & 216 & 576 & 576 \\
-2088 & -864 & 1656 & 1152 & -2088 & -864 & 1656 & 1152 & 6750 & -864 & -5274 & 2880 & 216 & -864 & 216 & 576 \\
0 & -1224 & -864 & 1080 & 0 & -1224 & -864 & 1080 & -1728 & 5706 & -864 & -3078 & 576 & 216 & -864 & 216 \\
0 & 0 & -648 & -864 & 0 & 0 & -648 & -864 & -1728 & -1728 & 3510 & -864 & 576 & 576 & 216 & -864
\end{pmatrix}$$

$S = \{1234, 1243, 1342, 2314, 2413, 2431, 3124, 3142, 3421, 4123, 4231, 4312\}, \lambda_{max} = 0.203291, \lambda_{min} = -0.327815$

$$H_S = \frac{1}{6 \cdot 5^6} \times \begin{pmatrix}
-3456 & 864 & 2304 & 2304 & -216 & 12510 & -1152 & -1152 & 864 & -2952 & 0 & 0 & 864 & -2952 & 0 & 0 \\
864 & -3456 & 864 & 2304 & -12402 & -216 & 9414 & -1152 & 2520 & 864 & -2376 & 0 & 2520 & 864 & -2376 & 0 \\
2304 & 864 & -3456 & 864 & 1440 & -9306 & -216 & 5670 & -1152 & 1944 & 864 & -1512 & -1152 & 1944 & 864 & -1512 \\
2304 & 2304 & 864 & -3456 & 1440 & 1440 & -5562 & -216 & -1152 & -1152 & 1080 & 864 & -1152 & -1152 & 1080 & 864 \\
-216 & -12402 & 1440 & 1440 & -3456 & 864 & 2304 & 2304 & -216 & 10314 & -2016 & -2016 & 864 & -2952 & 0 & 0 \\
12510 & -216 & -9306 & 1440 & 864 & -3456 & 864 & 2304 & -10206 & -216 & 8154 & -2016 & 2520 & 864 & -2376 & 0 \\
-1152 & 9414 & -216 & -5562 & 2304 & 864 & -3456 & 864 & 2304 & -8046 & -216 & 4914 & -1152 & 1944 & 864 & -1512 \\
-1152 & -1152 & 5670 & -216 & 2304 & 2304 & 864 & -3456 & 2304 & 2304 & -4806 & -216 & -1152 & -1152 & 1080 & 864 \\
864 & 2520 & -1152 & -1152 & -216 & -10206 & 2304 & 2304 & -3456 & 864 & 2304 & 2304 & -216 & 6750 & -2592 & -2592 \\
-2952 & 864 & 1944 & -1152 & 10314 & -216 & -8046 & 2304 & 864 & -3456 & 864 & 2304 & -6642 & -216 & 5814 & -2592 \\
0 & -2376 & 864 & 1080 & -2016 & 8154 & -216 & -4806 & 2304 & 864 & -3456 & 864 & 2880 & -5706 & -216 & 3510 \\
0 & 0 & -1512 & 864 & -2016 & -2016 & 4914 & -216 & 2304 & 2304 & 864 & -3456 & 2880 & 2880 & -3402 & -216 \\
864 & 2520 & -1152 & -1152 & 864 & 2520 & -1152 & -1152 & -216 & -6642 & 2880 & 2880 & -3456 & 864 & 2304 & 2304 \\
-2952 & 864 & 1944 & -1152 & -2952 & 864 & 1944 & -1152 & 6750 & -216 & -5706 & 2880 & 864 & -3456 & 864 & 2304 \\
0 & -2376 & 864 & 1080 & 0 & -2376 & 864 & 1080 & -2592 & 5814 & -216 & -3402 & 2304 & 864 & -3456 & 864 \\
0 & 0 & -1512 & 864 & 0 & 0 & -1512 & 864 & -2592 & -2592 & 3510 & -216 & 2304 & 2304 & 864 & -3456
\end{pmatrix}$$

$S = \{1234, 1243, 1342, 2314, 2413, 2431, 3124, 3142, 3421, 4132, 4213, 4321\}, \lambda_{max} = 0.048221, \lambda_{min} = -0.154921$

$$H_S = \frac{1}{6 \cdot 5^6} \times \begin{pmatrix}
-3456 & 864 & 2304 & 2304 & -216 & 6354 & 144 & 144 & 864 & -216 & -576 & -576 & 864 & -216 & -576 & -576 \\
864 & -3456 & 864 & 2304 & -6246 & -216 & 4554 & 144 & -216 & 864 & -216 & -576 & -216 & 864 & -216 & -576 \\
2304 & 864 & -3456 & 864 & 144 & -4446 & -216 & 2754 & -576 & -216 & 864 & -216 & -576 & -216 & 864 & -216 \\
2304 & 2304 & 864 & -3456 & 144 & 144 & -2646 & -216 & -576 & -576 & -216 & 864 & -576 & -576 & -216 & 864 \\
-216 & -6246 & 144 & 144 & -3456 & 864 & 2304 & 2304 & -216 & 54 & 144 & 144 & 864 & -216 & -576 & -576 \\
6354 & -216 & -4446 & 144 & 864 & -3456 & 864 & 2304 & 54 & -216 & 54 & 144 & -216 & 864 & -216 & -576 \\
144 & 4554 & -216 & -2646 & 2304 & 864 & -3456 & 864 & 144 & 54 & -216 & 54 & -576 & -216 & 864 & -216 \\
144 & 144 & 2754 & -216 & 2304 & 2304 & 864 & -3456 & 144 & 144 & 54 & -216 & -576 & -576 & -216 & 864 \\
864 & -216 & -576 & -576 & -216 & 54 & 144 & 144 & -3456 & 864 & 2304 & 2304 & -216 & -6246 & 144 & 144 \\
-216 & 864 & -216 & -576 & 54 & -216 & 54 & 144 & 864 & -3456 & 864 & 2304 & 6354 & -216 & -4446 & 144 \\
-576 & -216 & 864 & -216 & 144 & 54 & -216 & 54 & 2304 & 864 & -3456 & 864 & 144 & 4554 & -216 & -2646 \\
-576 & -576 & -216 & 864 & 144 & 144 & 54 & -216 & 2304 & 2304 & 864 & -3456 & 144 & 144 & 2754 & -216 \\
864 & -216 & -576 & -576 & 864 & -216 & -576 & -576 & -216 & 6354 & 144 & 144 & -3456 & 864 & 2304 & 2304 \\
-216 & 864 & -216 & -576 & -216 & 864 & -216 & -576 & -6246 & -216 & 4554 & 144 & 864 & -3456 & 864 & 2304 \\
-576 & -216 & 864 & -216 & -576 & -216 & 864 & -216 & 144 & -4446 & -216 & 2754 & 2304 & 864 & -3456 & 864 \\
-576 & -576 & -216 & 864 & -576 & -576 & -216 & 864 & 144 & 144 & -2646 & -216 & 2304 & 2304 & 864 & -3456
\end{pmatrix}$$

$S = \{1234, 1243, 1342, 2314, 2413, 2431, 3124, 3241, 3412, 4123, 4132, 4321\}, \lambda_{max} = 0.273073, \lambda_{min} = -0.204619$

$$H_S = \frac{1}{6 \cdot 5^6} \times \begin{pmatrix}
0 & 0 & 0 & 0 & 0 & 10944 & 2736 & 2736 & 0 & -2304 & -576 & -576 & 0 & -2304 & -576 & -576 \\
0 & 0 & 0 & 0 & -10944 & 0 & 6840 & 2736 & 2304 & 0 & -1440 & -576 & 2304 & 0 & -1440 & -576 \\
0 & 0 & 0 & 0 & -2736 & -6840 & 0 & 4104 & 576 & 1440 & 0 & -864 & 576 & 1440 & 0 & -864 \\
0 & 0 & 0 & 0 & -2736 & -2736 & -4104 & 0 & 576 & 576 & 864 & 0 & 576 & 576 & 864 & 0 \\
0 & -10944 & -2736 & -2736 & 0 & 0 & 0 & 0 & 0 & 8640 & 2160 & 2160 & 0 & -2304 & -576 & -576 \\
10944 & 0 & -6840 & -2736 & 0 & 0 & 0 & 0 & -8640 & 0 & 5400 & 2160 & 2304 & 0 & -1440 & -576 \\
2736 & 6840 & 0 & -4104 & 0 & 0 & 0 & 0 & -2160 & -5400 & 0 & 3240 & 576 & 1440 & 0 & -864 \\
2736 & 2736 & 4104 & 0 & 0 & 0 & 0 & 0 & -2160 & -2160 & -3240 & 0 & 576 & 576 & 864 & 0 \\
0 & 2304 & 576 & 576 & 0 & -8640 & -2160 & -2160 & 0 & 0 & 0 & 0 & 0 & 5184 & 1296 & 1296 \\
-2304 & 0 & 1440 & 576 & 8640 & 0 & -5400 & -2160 & 0 & 0 & 0 & 0 & -5184 & 0 & 3240 & 1296 \\
-576 & -1440 & 0 & 864 & 2160 & 5400 & 0 & -3240 & 0 & 0 & 0 & 0 & -1296 & -3240 & 0 & 1944 \\
-576 & -576 & -864 & 0 & 2160 & 2160 & 3240 & 0 & 0 & 0 & 0 & 0 & -1296 & -1296 & -1944 & 0 \\
0 & 2304 & 576 & 576 & 0 & 2304 & 576 & 576 & 0 & -5184 & -1296 & -1296 & 0 & 0 & 0 & 0 \\
-2304 & 0 & 1440 & 576 & -2304 & 0 & 1440 & 576 & 5184 & 0 & -3240 & -1296 & 0 & 0 & 0 & 0 \\
-576 & -1440 & 0 & 864 & -576 & -1440 & 0 & 864 & 1296 & 3240 & 0 & -1944 & 0 & 0 & 0 & 0 \\
-576 & -576 & -864 & 0 & -576 & -576 & -864 & 0 & 1296 & 1296 & 1944 & 0 & 0 & 0 & 0 & 0
\end{pmatrix}$$

$S = \{1234, 1243, 1342, 2314, 2413, 2431, 3124, 3241, 3421, 4123, 4132, 4312\}, \lambda_{max} = 0.159857, \lambda_{min} = -0.270465$

$$H_S = \frac{1}{6 \cdot 5^6} \times \begin{pmatrix}
-2592 & 648 & 1728 & 1728 & 648 & 10944 & 1872 & 1872 & 1728 & -3168 & -576 & -576 & 1728 & -3168 & -576 & -576 \\
648 & -2592 & 648 & 1728 & -11268 & 648 & 6948 & 1872 & 2304 & 1728 & -2592 & -576 & 2304 & 1728 & -2592 & -576 \\
1728 & 648 & -2592 & 648 & -2736 & -7272 & 648 & 4104 & -1728 & 1728 & 1728 & -1728 & -1728 & 1728 & 1728 & -1728 \\
1728 & 1728 & 648 & -2592 & -2736 & -2736 & -4428 & 648 & -1728 & -1728 & 864 & 1728 & -1728 & -1728 & 864 & 1728 \\
648 & -11268 & -2736 & -2736 & -2592 & 648 & 1728 & 1728 & 648 & 8748 & 1008 & 1008 & 1728 & -3168 & -576 & -576 \\
10944 & 648 & -7272 & -2736 & 648 & -2592 & 648 & 1728 & -9072 & 648 & 5688 & 1008 & 2304 & 1728 & -2592 & -576 \\
1872 & 6948 & 648 & -4428 & 1728 & 648 & -2592 & 648 & -1872 & -6012 & 648 & 3348 & -1728 & 1728 & 1728 & -1728 \\
1872 & 1872 & 4104 & 648 & 1728 & 1728 & 648 & -2592 & -1872 & -1872 & -3672 & 648 & -1728 & -1728 & 864 & 1728 \\
1728 & 2304 & -1728 & -1728 & 648 & -9072 & -1872 & -1872 & -2592 & 648 & 1728 & 1728 & 648 & 5184 & 432 & 432 \\
-3168 & 1728 & 1728 & -1728 & 8748 & 648 & -6012 & -1872 & 648 & -2592 & 648 & 1728 & -5508 & 648 & 3348 & 432 \\
-576 & -2592 & 1728 & 864 & 1008 & 5688 & 648 & -3672 & 1728 & 648 & -2592 & 648 & -1296 & -3672 & 648 & 1944 \\
-576 & -576 & -1728 & 1728 & 1008 & 1008 & 3348 & 648 & 1728 & 1728 & 648 & -2592 & -1296 & -1296 & -2268 & 648 \\
1728 & 2304 & -1728 & -1728 & 1728 & 2304 & -1728 & -1728 & 648 & -5508 & -1296 & -1296 & -2592 & 648 & 1728 & 1728 \\
-3168 & 1728 & 1728 & -1728 & -3168 & 1728 & 1728 & -1728 & 5184 & 648 & -3672 & -1296 & 648 & -2592 & 648 & 1728 \\
-576 & -2592 & 1728 & 864 & -576 & -2592 & 1728 & 864 & 432 & 3348 & 648 & -2268 & 1728 & 648 & -2592 & 648 \\
-576 & -576 & -1728 & 1728 & -576 & -576 & -1728 & 1728 & 432 & 432 & 1944 & 648 & 1728 & 1728 & 648 & -2592
\end{pmatrix}$$

$S = \{1234, 1243, 1342, 2314, 2413, 2431, 3142, 3214, 3421, 4123, 4132, 4321\}, \lambda_{max} = 0.149072, \lambda_{min} = -0.077220$

$$H_S = \frac{1}{6 \cdot 5^6} \times \begin{pmatrix}
0 & 0 & 0 & 0 & 0 & 5760 & 1440 & 1440 & 0 & 0 & 0 & 0 & 0 & 0 & 0 & 0 \\
0 & 0 & 0 & 0 & -5760 & 0 & 3600 & 1440 & 0 & 0 & 0 & 0 & 0 & 0 & 0 & 0 \\
0 & 0 & 0 & 0 & -1440 & -3600 & 0 & 2160 & 0 & 0 & 0 & 0 & 0 & 0 & 0 & 0 \\
0 & 0 & 0 & 0 & -1440 & -1440 & -2160 & 0 & 0 & 0 & 0 & 0 & 0 & 0 & 0 & 0 \\
0 & -5760 & -1440 & -1440 & 0 & 0 & 0 & 0 & 0 & 0 & 0 & 0 & 0 & 0 & 0 & 0 \\
5760 & 0 & -3600 & -1440 & 0 & 0 & 0 & 0 & 0 & 0 & 0 & 0 & 0 & 0 & 0 & 0 \\
1440 & 3600 & 0 & -2160 & 0 & 0 & 0 & 0 & 0 & 0 & 0 & 0 & 0 & 0 & 0 & 0 \\
1440 & 1440 & 2160 & 0 & 0 & 0 & 0 & 0 & 0 & 0 & 0 & 0 & 0 & 0 & 0 & 0 \\
0 & 0 & 0 & 0 & 0 & 0 & 0 & 0 & 0 & 0 & 0 & 0 & 0 & -5760 & -1440 & -1440 \\
0 & 0 & 0 & 0 & 0 & 0 & 0 & 0 & 0 & 0 & 0 & 0 & 5760 & 0 & -3600 & -1440 \\
0 & 0 & 0 & 0 & 0 & 0 & 0 & 0 & 0 & 0 & 0 & 0 & 1440 & 3600 & 0 & -2160 \\
0 & 0 & 0 & 0 & 0 & 0 & 0 & 0 & 0 & 0 & 0 & 0 & 1440 & 1440 & 2160 & 0 \\
0 & 0 & 0 & 0 & 0 & 0 & 0 & 0 & 0 & 5760 & 1440 & 1440 & 0 & 0 & 0 & 0 \\
0 & 0 & 0 & 0 & 0 & 0 & 0 & 0 & -5760 & 0 & 3600 & 1440 & 0 & 0 & 0 & 0 \\
0 & 0 & 0 & 0 & 0 & 0 & 0 & 0 & -1440 & -3600 & 0 & 2160 & 0 & 0 & 0 & 0 \\
0 & 0 & 0 & 0 & 0 & 0 & 0 & 0 & -1440 & -1440 & -2160 & 0 & 0 & 0 & 0 & 0
\end{pmatrix}$$

$S = \{1234, 1243, 1342, 2341, 2413, 2431, 3124, 3214, 3412, 4123, 4132, 4321\}, \lambda_{max} = 0.263856, \lambda_{min} = -0.131697$

$$H_S = \frac{1}{6\cdot 5^6} \times \begin{pmatrix} 3456 & 216 & -864 & -864 & -864 & 10350 & 2952 & 2952 & -2304 & -1008 & 0 & 0 & -2304 & -1008 & 0 & 0 \\ 216 & 3456 & 216 & -864 & -10458 & -864 & 6786 & 2952 & 720 & -2304 & -1584 & 0 & 720 & -2304 & -1584 & 0 \\ -864 & 216 & 3456 & 216 & -2520 & -6894 & -864 & 4590 & 1152 & 1296 & -2304 & -2448 & 1152 & 1296 & -2304 & -2448 \\ -864 & -864 & 216 & 3456 & -2520 & -2520 & -4698 & -864 & 1152 & 1152 & 2160 & -2304 & 1152 & 1152 & 2160 & -2304 \\ -864 & -10458 & -2520 & -2520 & 3456 & 216 & -864 & -864 & -864 & 7686 & 2376 & 2376 & -2304 & -1008 & 0 & 0 \\ 10350 & -864 & -6894 & -2520 & 216 & 3456 & 216 & -864 & -7794 & -864 & 5346 & 2376 & 720 & -2304 & -1584 & 0 \\ 2952 & 6786 & -864 & -4698 & -864 & 216 & 3456 & 216 & -1944 & -5454 & -864 & 4086 & 1152 & 1296 & -2304 & -2448 \\ 2952 & 2952 & 4590 & -864 & -864 & -864 & 216 & 3456 & -1944 & -1944 & -4194 & -864 & 1152 & 1152 & 2160 & -2304 \\ -2304 & 720 & 1152 & 1152 & -864 & -7794 & -1944 & -1944 & 3456 & 216 & -864 & -864 & -864 & 4590 & 1512 & 1512 \\ -1008 & -2304 & 1296 & 1152 & 7686 & -864 & -5454 & -1944 & 216 & 3456 & 216 & -864 & -4698 & -864 & 3186 & 1512 \\ 0 & -1584 & -2304 & 2160 & 2376 & 5346 & -864 & -4194 & -864 & 216 & 3456 & 216 & -1080 & -3294 & -864 & 2430 \\ 0 & 0 & -2448 & -2304 & 2376 & 2376 & 4086 & -864 & -864 & -864 & 216 & 3456 & -1080 & -1080 & -2538 & -864 \\ -2304 & 720 & 1152 & 1152 & -2304 & 720 & 1152 & 1152 & -864 & -4698 & -1080 & -1080 & 3456 & 216 & -864 & -864 \\ -1008 & -2304 & 1296 & 1152 & -1008 & -2304 & 1296 & 1152 & 4590 & -864 & -3294 & -1080 & 216 & 3456 & 216 & -864 \\ 0 & -1584 & -2304 & 2160 & 0 & -1584 & -2304 & 2160 & 1512 & 3186 & -864 & -2538 & -864 & 216 & 3456 & 216 \\ 0 & 0 & -2448 & -2304 & 0 & 0 & -2448 & -2304 & 1512 & 1512 & 2430 & -864 & -864 & -864 & 216 & 3456 \end{pmatrix}$$

$S = \{1234, 1243, 1342, 2341, 2413, 2431, 3124, 3214, 3421, 4123, 4132, 4312\}, \lambda_{max} = 0.209132, \lambda_{min} = -0.191790$

$$H_S = \frac{1}{6\cdot 5^6} \times \begin{pmatrix} 864 & 864 & 864 & 864 & -216 & 10350 & 2088 & 2088 & -576 & -1872 & 0 & 0 & -576 & -1872 & 0 & 0 \\ 864 & 864 & 864 & 864 & -10782 & -216 & 6894 & 2088 & 720 & -576 & -2736 & 0 & 720 & -576 & -2736 & 0 \\ 864 & 864 & 864 & 864 & -2520 & -7326 & -216 & 4590 & -1152 & 1584 & -576 & -3312 & -1152 & 1584 & -576 & -3312 \\ 864 & 864 & 864 & 864 & -2520 & -2520 & -5022 & -216 & -1152 & -1152 & 2160 & -576 & -1152 & -1152 & 2160 & -576 \\ -216 & -10782 & -2520 & -2520 & 864 & 864 & 864 & 864 & -216 & 7794 & 1224 & 1224 & -576 & -1872 & 0 & 0 \\ 10350 & -216 & -7326 & -2520 & 864 & 864 & 864 & 864 & -8226 & -216 & 5634 & 1224 & 720 & -576 & -2736 & 0 \\ 2088 & 6894 & -216 & -5022 & 864 & 864 & 864 & 864 & -1656 & -6066 & -216 & 4194 & -1152 & 1584 & -576 & -3312 \\ 2088 & 2088 & 4590 & -216 & 864 & 864 & 864 & 864 & -1656 & -1656 & -4626 & -216 & -1152 & -1152 & 2160 & -576 \\ -576 & 720 & -1152 & -1152 & -216 & -8226 & -1656 & -1656 & 864 & 864 & 864 & 864 & -216 & 4590 & 648 & 648 \\ -1872 & -576 & 1584 & -1152 & 7794 & -216 & -6066 & -1656 & 864 & 864 & 864 & 864 & -5022 & -216 & 3294 & 648 \\ 0 & -2736 & -576 & 2160 & 1224 & 5634 & -216 & -4626 & 864 & 864 & 864 & 864 & -1080 & -3726 & -216 & 2430 \\ 0 & 0 & -3312 & -576 & 1224 & 1224 & 4194 & -216 & 864 & 864 & 864 & 864 & -1080 & -1080 & -2862 & -216 \\ -576 & 720 & -1152 & -1152 & -576 & 720 & -1152 & -1152 & -216 & -5022 & -1080 & -1080 & 864 & 864 & 864 & 864 \\ -1872 & -576 & 1584 & -1152 & -1872 & -576 & 1584 & -1152 & 4590 & -216 & -3726 & -1080 & 864 & 864 & 864 & 864 \\ 0 & -2736 & -576 & 2160 & 0 & -2736 & -576 & 2160 & 648 & 3294 & -216 & -2862 & 864 & 864 & 864 & 864 \\ 0 & 0 & -3312 & -576 & 0 & 0 & -3312 & -576 & 648 & 648 & 2430 & -216 & 864 & 864 & 864 & 864 \end{pmatrix}$$

$\mathbf{S = \{1234, 1243, 1432, 2134, 2143, 2341, 3214, 3412, 3421, 4123, 4312, 4321\}}, \lambda_{max} = 0.204732, \lambda_{min} = 0.043105$

$$H_S = \frac{1}{6\cdot 5^6} \times \begin{pmatrix} 9216 & 576 & -2304 & -2304 & 576 & 36 & -144 & -144 & -2304 & -144 & 576 & 576 & -2304 & -144 & 576 & 576 \\ 576 & 9216 & 576 & -2304 & 36 & 576 & 36 & -144 & -144 & -2304 & -144 & 576 & -144 & -2304 & -144 & 576 \\ -2304 & 576 & 9216 & 576 & -144 & 36 & 576 & 36 & 576 & -144 & -2304 & -144 & 576 & -144 & -2304 & -144 \\ -2304 & -2304 & 576 & 9216 & -144 & -144 & 36 & 576 & 576 & 576 & -144 & -2304 & 576 & 576 & -144 & -2304 \\ 576 & 36 & -144 & -144 & 9216 & 576 & -2304 & -2304 & 576 & 36 & -144 & -144 & -2304 & -144 & 576 & 576 \\ 36 & 576 & 36 & -144 & 576 & 9216 & 576 & -2304 & 36 & 576 & 36 & -144 & -144 & -2304 & -144 & 576 \\ -144 & 36 & 576 & 36 & -2304 & 576 & 9216 & 576 & -144 & 36 & 576 & 36 & 576 & -144 & -2304 & -144 \\ -144 & -144 & 36 & 576 & -2304 & -2304 & 576 & 9216 & -144 & -144 & 36 & 576 & 576 & 576 & -144 & -2304 \\ -2304 & -144 & 576 & 576 & 576 & 36 & -144 & -144 & 9216 & 576 & -2304 & -2304 & 576 & 36 & -144 & -144 \\ -144 & -2304 & -144 & 576 & 36 & 576 & 36 & -144 & 576 & 9216 & 576 & -2304 & 36 & 576 & 36 & -144 \\ 576 & -144 & -2304 & -144 & -144 & 36 & 576 & 36 & -2304 & 576 & 9216 & 576 & -144 & 36 & 576 & 36 \\ 576 & 576 & -144 & -2304 & -144 & -144 & 36 & 576 & -2304 & -2304 & 576 & 9216 & -144 & -144 & 36 & 576 \\ -2304 & -144 & 576 & 576 & -2304 & -144 & 576 & 576 & 576 & 36 & -144 & -144 & 9216 & 576 & -2304 & -2304 \\ -144 & -2304 & -144 & 576 & -144 & -2304 & -144 & 576 & 36 & 576 & 36 & -144 & 576 & 9216 & 576 & -2304 \\ 576 & -144 & -2304 & -144 & 576 & -144 & -2304 & -144 & -144 & 36 & 576 & 36 & -2304 & 576 & 9216 & 576 \\ 576 & 576 & -144 & -2304 & 576 & 576 & -144 & -2304 & -144 & -144 & 36 & 576 & -2304 & -2304 & 576 & 9216 \end{pmatrix}$$

$\mathbf{S = \{1234, 1243, 1432, 2134, 2341, 2413, 3142, 3214, 3421, 4123, 4312, 4321\}}, \lambda_{max} = 0.106988, \lambda_{min} = 0.014289$

$$H_S = \frac{1}{6\cdot 5^6} \times \begin{pmatrix} 4608 & 288 & -1152 & -1152 & 288 & 1818 & -72 & -72 & -1152 & -72 & 288 & 288 & -1152 & -72 & 288 & 288 \\ 288 & 4608 & 288 & -1152 & -1782 & 288 & 18 & -72 & -72 & -1152 & -72 & 288 & -72 & -1152 & -72 & 288 \\ -1152 & 288 & 4608 & 288 & -72 & 18 & 288 & -1782 & 288 & -72 & -1152 & -72 & 288 & -72 & -1152 & -72 \\ -1152 & -1152 & 288 & 4608 & -72 & -72 & 1818 & 288 & 288 & 288 & -72 & -1152 & 288 & 288 & -72 & -1152 \\ 288 & -1782 & -72 & -72 & 4608 & 288 & -1152 & -1152 & 288 & 18 & -72 & -72 & -1152 & -72 & 288 & 288 \\ 1818 & 288 & 18 & -72 & 288 & 4608 & 288 & -1152 & 18 & 288 & 18 & -72 & -72 & -1152 & -72 & 288 \\ -72 & 18 & 288 & 1818 & -1152 & 288 & 4608 & 288 & -72 & 18 & 288 & 18 & 288 & -72 & -1152 & -72 \\ -72 & -72 & -1782 & 288 & -1152 & -1152 & 288 & 4608 & -72 & -72 & 18 & 288 & 288 & 288 & -72 & -1152 \\ -1152 & -72 & 288 & 288 & 288 & 18 & -72 & -72 & 4608 & 288 & -1152 & -1152 & 288 & -1782 & -72 & -72 \\ -72 & -1152 & -72 & 288 & 18 & 288 & 18 & -72 & 288 & 4608 & 288 & -1152 & 1818 & 288 & 18 & -72 \\ 288 & -72 & -1152 & -72 & -72 & 18 & 288 & 18 & -1152 & 288 & 4608 & 288 & -72 & 18 & 288 & 1818 \\ 288 & 288 & -72 & -1152 & -72 & -72 & 18 & 288 & -1152 & -1152 & 288 & 4608 & -72 & -72 & -1782 & 288 \\ -1152 & -72 & 288 & 288 & -1152 & -72 & 288 & 288 & 288 & 1818 & -72 & -72 & 4608 & 288 & -1152 & -1152 \\ -72 & -1152 & -72 & 288 & -72 & -1152 & -72 & 288 & -1782 & 288 & 18 & -72 & 288 & 4608 & 288 & -1152 \\ 288 & -72 & -1152 & -72 & 288 & -72 & -1152 & -72 & -72 & 18 & 288 & -1782 & -1152 & 288 & 4608 & 288 \\ 288 & 288 & -72 & -1152 & 288 & 288 & -72 & -1152 & -72 & -72 & 1818 & 288 & -1152 & -1152 & 288 & 4608 \end{pmatrix}$$

$S = \{1234, 1243, 1432, 2143, 2314, 2341, 3124, 3412, 3421, 4123, 4231, 4312\}, \lambda_{max} = 0.332871, \lambda_{min} = -0.205616$

$$H_S = \frac{1}{6 \cdot 5^6} \times \begin{pmatrix}
4608 & 288 & -1152 & -1152 & 288 & 11214 & -2808 & -2808 & -1152 & -2808 & 864 & 864 & -1152 & -2808 & 864 & 864 \\
288 & 4608 & 288 & -1152 & -11178 & 288 & 10278 & -2808 & 2664 & -1152 & -2232 & 864 & 2664 & -1152 & -2232 & 864 \\
-1152 & 288 & 4608 & 288 & 2664 & -10242 & 288 & 7974 & -288 & 2088 & -1152 & -1368 & -288 & 2088 & -1152 & -1368 \\
-1152 & -1152 & 288 & 4608 & 2664 & 2664 & -7938 & 288 & -288 & -288 & 1224 & -1152 & -288 & -288 & 1224 & -1152 \\
288 & -11178 & 2664 & 2664 & 4608 & 288 & -1152 & -1152 & 288 & 10278 & -2232 & -2232 & -1152 & -2808 & 864 & 864 \\
11214 & 288 & -10242 & 2664 & 288 & 4608 & 288 & -1152 & -10242 & 288 & 8118 & -2232 & 2664 & -1152 & -2232 & 864 \\
-2808 & 10278 & 288 & -7938 & -1152 & 288 & 4608 & 288 & 2088 & -8082 & 288 & 4878 & -288 & 2088 & -1152 & -1368 \\
-2808 & -2808 & 7974 & 288 & -1152 & -1152 & 288 & 4608 & 2088 & 2088 & -4842 & 288 & -288 & -288 & 1224 & -1152 \\
-1152 & 2664 & -288 & -288 & 288 & -10242 & 2088 & 2088 & 4608 & 288 & -1152 & -1152 & 288 & 7974 & -1368 & -1368 \\
-2808 & -1152 & 2088 & -288 & 10278 & 288 & -8082 & 2088 & 288 & 4608 & 288 & -1152 & -7938 & 288 & 4878 & -1368 \\
864 & -2232 & -1152 & 1224 & -2232 & 8118 & 288 & -4842 & -1152 & 288 & 4608 & 288 & 1224 & -4842 & 288 & 1134 \\
864 & 864 & -1368 & -1152 & -2232 & -2232 & 4878 & 288 & -1152 & -1152 & 288 & 4608 & 1224 & 1224 & -1098 & 288 \\
-1152 & 2664 & -288 & -288 & -1152 & 2664 & -288 & -288 & 288 & -7938 & 1224 & 1224 & 4608 & 288 & -1152 & -1152 \\
-2808 & -1152 & 2088 & -288 & -2808 & -1152 & 2088 & -288 & 7974 & 288 & -4842 & 1224 & 288 & 4608 & 288 & -1152 \\
864 & -2232 & -1152 & 1224 & 864 & -2232 & -1152 & 1224 & -1368 & 4878 & 288 & -1098 & -1152 & 288 & 4608 & 288 \\
864 & 864 & -1368 & -1152 & 864 & 864 & -1368 & -1152 & -1368 & -1368 & 1134 & 288 & -1152 & -1152 & 288 & 4608
\end{pmatrix}$$

$S = \{1234, 1243, 1432, 2143, 2314, 2341, 3124, 3412, 3421, 4132, 4213, 4321\}, \lambda_{max} = 0.166665, \lambda_{min} = -0.049014$

$$H_S = \frac{1}{6 \cdot 5^6} \times \begin{pmatrix}
4608 & 288 & -1152 & -1152 & 288 & 5058 & -1512 & -1512 & -1152 & -72 & 288 & 288 & -1152 & -72 & 288 & 288 \\
288 & 4608 & 288 & -1152 & -5022 & 288 & 5418 & -1512 & -72 & -1152 & -72 & 288 & -72 & -1152 & -72 & 288 \\
-1152 & 288 & 4608 & 288 & 1368 & -5382 & 288 & 5058 & 288 & -72 & -1152 & -72 & 288 & -72 & -1152 & -72 \\
-1152 & -1152 & 288 & 4608 & 1368 & 1368 & -5022 & 288 & 288 & 288 & -72 & -1152 & 288 & 288 & -72 & -1152 \\
288 & -5022 & 1368 & 1368 & 4608 & 288 & -1152 & -1152 & 288 & 18 & -72 & -72 & -1152 & -72 & 288 & 288 \\
5058 & 288 & -5382 & 1368 & 288 & 4608 & 288 & -1152 & 18 & 288 & 18 & -72 & -72 & -1152 & -72 & 288 \\
-1512 & 5418 & 288 & -5022 & -1152 & 288 & 4608 & 288 & -72 & 18 & 288 & 18 & 288 & -72 & -1152 & -72 \\
-1512 & -1512 & 5058 & 288 & -1152 & -1152 & 288 & 4608 & -72 & -72 & 18 & 288 & 288 & 288 & -72 & -1152 \\
-1152 & -72 & 288 & 288 & 288 & 18 & -72 & -72 & 4608 & 288 & -1152 & -1152 & 288 & -5022 & 1368 & 1368 \\
-72 & -1152 & -72 & 288 & 18 & 288 & 18 & -72 & 288 & 4608 & 288 & -1152 & 5058 & 288 & -5382 & 1368 \\
288 & -72 & -1152 & -72 & -72 & 18 & 288 & 18 & -1152 & 288 & 4608 & 288 & -1512 & 5418 & 288 & -5022 \\
288 & 288 & -72 & -1152 & -72 & -72 & 18 & 288 & -1152 & -1152 & 288 & 4608 & -1512 & -1512 & 5058 & 288 \\
-1152 & -72 & 288 & 288 & -1152 & -72 & 288 & 288 & 288 & 5058 & -1512 & -1512 & 4608 & 288 & -1152 & -1152 \\
-72 & -1152 & -72 & 288 & -72 & -1152 & -72 & 288 & -5022 & 288 & 5418 & -1512 & 288 & 4608 & 288 & -1152 \\
288 & -72 & -1152 & -72 & 288 & -72 & -1152 & -72 & 1368 & -5382 & 288 & 5058 & -1152 & 288 & 4608 & 288 \\
288 & 288 & -72 & -1152 & 288 & 288 & -72 & -1152 & 1368 & 1368 & -5022 & 288 & -1152 & -1152 & 288 & 4608
\end{pmatrix}$$

$\mathbf{S = \{1234, 1243, 1432, 2143, 2314, 2341, 3214, 3412, 3421, 4123, 4132, 4321\}}, \lambda_{max} = 0.237862, \lambda_{min} = 0.002798$

$$H_S = \frac{1}{6 \cdot 5^6} \times \begin{pmatrix}
8064 & -576 & -3456 & -3456 & 504 & 4464 & -216 & -216 & -2016 & 144 & 864 & 864 & -2016 & 144 & 864 & 864 \\
-576 & 8064 & -576 & -3456 & -4536 & 504 & 4464 & -216 & 144 & -2016 & 144 & 864 & 144 & -2016 & 144 & 864 \\
-3456 & -576 & 8064 & -576 & -216 & -4536 & 504 & 4464 & 864 & 144 & -2016 & 144 & 864 & 144 & -2016 & 144 \\
-3456 & -3456 & -576 & 8064 & -216 & -216 & -4536 & 504 & 864 & 864 & 144 & -2016 & 864 & 864 & 144 & -2016 \\
504 & -4536 & -216 & -216 & 8064 & -576 & -3456 & -3456 & 504 & -36 & -216 & -216 & -2016 & 144 & 864 & 864 \\
4464 & 504 & -4536 & -216 & -576 & 8064 & -576 & -3456 & -36 & 504 & -36 & -216 & 144 & -2016 & 144 & 864 \\
-216 & 4464 & 504 & -4536 & -3456 & -576 & 8064 & -576 & -216 & -36 & 504 & -36 & 864 & 144 & -2016 & 144 \\
-216 & -216 & 4464 & 504 & -3456 & -3456 & -576 & 8064 & -216 & -216 & -36 & 504 & 864 & 864 & 144 & -2016 \\
-2016 & 144 & 864 & 864 & 504 & -36 & -216 & -216 & 8064 & -576 & -3456 & -3456 & 504 & -4536 & -216 & -216 \\
144 & -2016 & 144 & 864 & -36 & 504 & -36 & -216 & -576 & 8064 & -576 & -3456 & 4464 & 504 & -4536 & -216 \\
864 & 144 & -2016 & 144 & -216 & -36 & 504 & -36 & -3456 & -576 & 8064 & -576 & -216 & 4464 & 504 & -4536 \\
864 & 864 & 144 & -2016 & -216 & -216 & -36 & 504 & -3456 & -3456 & -576 & 8064 & -216 & -216 & 4464 & 504 \\
-2016 & 144 & 864 & 864 & -2016 & 144 & 864 & 864 & 504 & 4464 & -216 & -216 & 8064 & -576 & -3456 & -3456 \\
144 & -2016 & 144 & 864 & 144 & -2016 & 144 & 864 & -4536 & 504 & 4464 & -216 & -576 & 8064 & -576 & -3456 \\
864 & 144 & -2016 & 144 & 864 & 144 & -2016 & 144 & -216 & -4536 & 504 & 4464 & -3456 & -576 & 8064 & -576 \\
864 & 864 & 144 & -2016 & 864 & 864 & 144 & -2016 & -216 & -216 & -4536 & 504 & -3456 & -3456 & -576 & 8064
\end{pmatrix}$$

$S = \{1234, 1243, 1432, 2314, 2341, 2413, 3124, 3142, 3412, 4123, 4231, 4321\}, \lambda_{max} = 0.314949, \lambda_{min} = -0.193509$

$$H_S = \frac{1}{6 \cdot 5^6} \times \begin{pmatrix}
2592 & -648 & -1728 & -1728 & -648 & 12996 & -1872 & -1872 & -1728 & -1872 & 576 & 576 & -1728 & -1872 & 576 & 576 \\
-648 & 2592 & -648 & -1728 & -12672 & -648 & 10152 & -1872 & 2736 & -1728 & -1008 & 576 & 2736 & -1728 & -1008 & 576 \\
-1728 & -648 & 2592 & -648 & 2736 & -9828 & -648 & 6156 & 1728 & 1872 & -1728 & -432 & 1728 & 1872 & -1728 & -432 \\
-1728 & -1728 & -648 & 2592 & 2736 & 2736 & -5832 & -648 & 1728 & 1728 & 1296 & -1728 & 1728 & 1728 & 1296 & -1728 \\
-648 & -12672 & 2736 & 2736 & 2592 & -648 & -1728 & -1728 & -648 & 10152 & -1008 & -1008 & -1728 & -1872 & 576 & 576 \\
12996 & -648 & -9828 & 2736 & -648 & 2592 & -648 & -1728 & -9828 & -648 & 7812 & -1008 & 2736 & -1728 & -1008 & 576 \\
-1872 & 10152 & -648 & -5832 & -1728 & -648 & 2592 & -648 & 1872 & -7488 & -648 & 4752 & 1728 & 1872 & -1728 & -432 \\
-1872 & -1872 & 6156 & -648 & -1728 & -1728 & -648 & 2592 & 1872 & 1872 & -4428 & -648 & 1728 & 1728 & 1296 & -1728 \\
-1728 & 2736 & 1728 & 1728 & -648 & -9828 & 1872 & 1872 & 2592 & -648 & -1728 & -1728 & -648 & 6156 & -432 & -432 \\
-1872 & -1728 & 1872 & 1728 & 10152 & -648 & -7488 & 1872 & -648 & 2592 & -648 & -1728 & -5832 & -648 & 4752 & -432 \\
576 & -1008 & -1728 & 1296 & -1008 & 7812 & -648 & -4428 & -1728 & -648 & 2592 & -648 & 1296 & -4428 & -648 & 2916 \\
576 & 576 & -432 & -1728 & -1008 & -1008 & 4752 & -648 & -1728 & -1728 & -648 & 2592 & 1296 & 1296 & -2592 & -648 \\
-1728 & 2736 & 1728 & 1728 & -1728 & 2736 & 1728 & 1728 & -648 & -5832 & 1296 & 1296 & 2592 & -648 & -1728 & -1728 \\
-1872 & -1728 & 1872 & 1728 & -1872 & -1728 & 1872 & 1728 & 6156 & -648 & -4428 & 1296 & -648 & 2592 & -648 & -1728 \\
576 & -1008 & -1728 & 1296 & 576 & -1008 & -1728 & 1296 & -432 & 4752 & -648 & -2592 & -1728 & -648 & 2592 & -648 \\
576 & 576 & -432 & -1728 & 576 & 576 & -432 & -1728 & -432 & -432 & 2916 & -648 & -1728 & -1728 & -648 & 2592
\end{pmatrix}$$

$S = \{1234, 1243, 1432, 2314, 2341, 2413, 3124, 3142, 3421, 4123, 4231, 4312\}, \lambda_{max} = 0.468946, \lambda_{min} = -0.269624$

$$H_S = \frac{1}{6 \cdot 5^6} \times \begin{pmatrix} 0 & 0 & 0 & 0 & 0 & 12996 & -2736 & -2736 & 0 & -2736 & 576 & 576 & 0 & -2736 & 576 & 576 \\ 0 & 0 & 0 & 0 & -12996 & 0 & 10260 & -2736 & 2736 & 0 & -2160 & 576 & 2736 & 0 & -2160 & 576 \\ 0 & 0 & 0 & 0 & 2736 & -10260 & 0 & 6156 & -576 & 2160 & 0 & -1296 & -576 & 2160 & 0 & -1296 \\ 0 & 0 & 0 & 0 & 2736 & 2736 & -6156 & 0 & -576 & -576 & 1296 & 0 & -576 & -576 & 1296 & 0 \\ 0 & -12996 & 2736 & 2736 & 0 & 0 & 0 & 0 & 0 & 10260 & -2160 & -2160 & 0 & -2736 & 576 & 576 \\ 12996 & 0 & -10260 & 2736 & 0 & 0 & 0 & 0 & -10260 & 0 & 8100 & -2160 & 2736 & 0 & -2160 & 576 \\ -2736 & 10260 & 0 & -6156 & 0 & 0 & 0 & 0 & 2160 & -8100 & 0 & 4860 & -576 & 2160 & 0 & -1296 \\ -2736 & -2736 & 6156 & 0 & 0 & 0 & 0 & 0 & 2160 & 2160 & -4860 & 0 & -576 & -576 & 1296 & 0 \\ 0 & 2736 & -576 & -576 & 0 & -10260 & 2160 & 2160 & 0 & 0 & 0 & 0 & 0 & 6156 & -1296 & -1296 \\ -2736 & 0 & 2160 & -576 & 10260 & 0 & -8100 & 2160 & 0 & 0 & 0 & 0 & -6156 & 0 & 4860 & -1296 \\ 576 & -2160 & 0 & 1296 & -2160 & 8100 & 0 & -4860 & 0 & 0 & 0 & 0 & 1296 & -4860 & 0 & 2916 \\ 576 & 576 & -1296 & 0 & -2160 & -2160 & 4860 & 0 & 0 & 0 & 0 & 0 & 1296 & 1296 & -2916 & 0 \\ 0 & 2736 & -576 & -576 & 0 & 2736 & -576 & -576 & 0 & -6156 & 1296 & 1296 & 0 & 0 & 0 & 0 \\ -2736 & 0 & 2160 & -576 & -2736 & 0 & 2160 & -576 & 6156 & 0 & -4860 & 1296 & 0 & 0 & 0 & 0 \\ 576 & -2160 & 0 & 1296 & 576 & -2160 & 0 & 1296 & -1296 & 4860 & 0 & -2916 & 0 & 0 & 0 & 0 \\ 576 & 576 & -1296 & 0 & 576 & 576 & -1296 & 0 & -1296 & -1296 & 2916 & 0 & 0 & 0 & 0 & 0 \end{pmatrix}$$

$S = \{1234, 1243, 1432, 2314, 2341, 2413, 3124, 3142, 3421, 4132, 4213, 4321\}, \lambda_{max} = 0.160495, \lambda_{min} = -0.101753$

$$H_S = \frac{1}{6 \cdot 5^6} \times \begin{pmatrix} 0 & 0 & 0 & 0 & 0 & 6840 & -1440 & -1440 & 0 & 0 & 0 & 0 & 0 & 0 & 0 & 0 \\ 0 & 0 & 0 & 0 & -6840 & 0 & 5400 & -1440 & 0 & 0 & 0 & 0 & 0 & 0 & 0 & 0 \\ 0 & 0 & 0 & 0 & 1440 & -5400 & 0 & 3240 & 0 & 0 & 0 & 0 & 0 & 0 & 0 & 0 \\ 0 & 0 & 0 & 0 & 1440 & 1440 & -3240 & 0 & 0 & 0 & 0 & 0 & 0 & 0 & 0 & 0 \\ 0 & -6840 & 1440 & 1440 & 0 & 0 & 0 & 0 & 0 & 0 & 0 & 0 & 0 & 0 & 0 & 0 \\ 6840 & 0 & -5400 & 1440 & 0 & 0 & 0 & 0 & 0 & 0 & 0 & 0 & 0 & 0 & 0 & 0 \\ -1440 & 5400 & 0 & -3240 & 0 & 0 & 0 & 0 & 0 & 0 & 0 & 0 & 0 & 0 & 0 & 0 \\ -1440 & -1440 & 3240 & 0 & 0 & 0 & 0 & 0 & 0 & 0 & 0 & 0 & 0 & 0 & 0 & 0 \\ 0 & 0 & 0 & 0 & 0 & 0 & 0 & 0 & 0 & 0 & 0 & 0 & 0 & -6840 & 1440 & 1440 \\ 0 & 0 & 0 & 0 & 0 & 0 & 0 & 0 & 0 & 0 & 0 & 0 & 6840 & 0 & -5400 & 1440 \\ 0 & 0 & 0 & 0 & 0 & 0 & 0 & 0 & 0 & 0 & 0 & 0 & -1440 & 5400 & 0 & -3240 \\ 0 & 0 & 0 & 0 & 0 & 0 & 0 & 0 & 0 & 0 & 0 & 0 & -1440 & -1440 & 3240 & 0 \\ 0 & 0 & 0 & 0 & 0 & 0 & 0 & 0 & 0 & 6840 & -1440 & -1440 & 0 & 0 & 0 & 0 \\ 0 & 0 & 0 & 0 & 0 & 0 & 0 & 0 & -6840 & 0 & 5400 & -1440 & 0 & 0 & 0 & 0 \\ 0 & 0 & 0 & 0 & 0 & 0 & 0 & 0 & 1440 & -5400 & 0 & 3240 & 0 & 0 & 0 & 0 \\ 0 & 0 & 0 & 0 & 0 & 0 & 0 & 0 & 1440 & 1440 & -3240 & 0 & 0 & 0 & 0 & 0 \end{pmatrix}$$

$S = \{1234, 1243, 1432, 2314, 2341, 2413, 3124, 3241, 3412, 4123, 4132, 4321\}, \lambda_{max} = 0.267567, \lambda_{min} = -0.159885$

$$H_S = \frac{1}{6 \cdot 5^6} \times \begin{pmatrix} 3456 & -864 & -2304 & -2304 & 216 & 11430 & 1152 & 1152 & -864 & -2088 & 0 & 0 & -864 & -2088 & 0 & 0 \\ -864 & 3456 & -864 & -2304 & -11538 & 216 & 7686 & 1152 & 2520 & -864 & -1224 & 0 & 2520 & -864 & -1224 & 0 \\ -2304 & -864 & 3456 & -864 & -1440 & -7794 & 216 & 4590 & 1152 & 1656 & -864 & -648 & 1152 & 1656 & -864 & -648 \\ -2304 & -2304 & -864 & 3456 & -1440 & -1440 & -4698 & 216 & 1152 & 1152 & 1080 & -864 & 1152 & 1152 & 1080 & -864 \\ 216 & -11538 & -1440 & -1440 & 3456 & -864 & -2304 & -2304 & 216 & 8586 & 2016 & 2016 & -864 & -2088 & 0 & 0 \\ 11430 & 216 & -7794 & -1440 & -864 & 3456 & -864 & -2304 & -8694 & 216 & 5346 & 2016 & 2520 & -864 & -1224 & 0 \\ 1152 & 7686 & 216 & -4698 & -2304 & -864 & 3456 & -864 & -2304 & -5454 & 216 & 3186 & 1152 & 1656 & -864 & -648 \\ 1152 & 1152 & 4590 & 216 & -2304 & -2304 & -864 & 3456 & -2304 & -2304 & -3294 & 216 & 1152 & 1152 & 1080 & -864 \\ -864 & 2520 & 1152 & 1152 & 216 & -8694 & -2304 & -2304 & 3456 & -864 & -2304 & -2304 & 216 & 4590 & 2592 & 2592 \\ -2088 & -864 & 1656 & 1152 & 8586 & 216 & -5454 & -2304 & -864 & 3456 & -864 & -2304 & -4698 & 216 & 2286 & 2592 \\ 0 & -1224 & -864 & 1080 & 2016 & 5346 & 216 & -3294 & -2304 & -864 & 3456 & -864 & -2880 & -2394 & 216 & 1350 \\ 0 & 0 & -648 & -864 & 2016 & 2016 & 3186 & 216 & -2304 & -2304 & -864 & 3456 & -2880 & -2880 & -1458 & 216 \\ -864 & 2520 & 1152 & 1152 & -864 & 2520 & 1152 & 1152 & 216 & -4698 & -2880 & -2880 & 3456 & -864 & -2304 & -2304 \\ -2088 & -864 & 1656 & 1152 & -2088 & -864 & 1656 & 1152 & 4590 & 216 & -2394 & -2880 & -864 & 3456 & -864 & -2304 \\ 0 & -1224 & -864 & 1080 & 0 & -1224 & -864 & 1080 & 2592 & 2286 & 216 & -1458 & -2304 & -864 & 3456 & -864 \\ 0 & 0 & -648 & -864 & 0 & 0 & -648 & -864 & 2592 & 2592 & 1350 & 216 & -2304 & -2304 & -864 & 3456 \end{pmatrix}$$

$S = \{1234, 1243, 1432, 2314, 2341, 2413, 3124, 3241, 3421, 4123, 4132, 4312\}, \lambda_{max} = 0.214579, \lambda_{min} = -0.210614$

$$H_S = \frac{1}{6 \cdot 5^6} \times \begin{pmatrix} 864 & -216 & -576 & -576 & 864 & 11430 & 288 & 288 & 864 & -2952 & 0 & 0 & 864 & -2952 & 0 & 0 \\ -216 & 864 & -216 & -576 & -11862 & 864 & 7794 & 288 & 2520 & 864 & -2376 & 0 & 2520 & 864 & -2376 & 0 \\ -576 & -216 & 864 & -216 & -1440 & -8226 & 864 & 4590 & -1152 & 1944 & 864 & -1512 & -1152 & 1944 & 864 & -1512 \\ -576 & -576 & -216 & 864 & -1440 & -1440 & -5022 & 864 & -1152 & -1152 & 1080 & 864 & -1152 & -1152 & 1080 & 864 \\ 864 & -11862 & -1440 & -1440 & 864 & -216 & -576 & -576 & 864 & 8694 & 864 & 864 & 864 & -2952 & 0 & 0 \\ 11430 & 864 & -8226 & -1440 & -216 & 864 & -216 & -576 & -9126 & 864 & 5634 & 864 & 2520 & 864 & -2376 & 0 \\ 288 & 7794 & 864 & -5022 & -576 & -216 & 864 & -216 & -2016 & -6066 & 864 & 3294 & -1152 & 1944 & 864 & -1512 \\ 288 & 288 & 4590 & 864 & -576 & -576 & -216 & 864 & -2016 & -2016 & -3726 & 864 & -1152 & -1152 & 1080 & 864 \\ 864 & 2520 & -1152 & -1152 & 864 & -9126 & -2016 & -2016 & 864 & -216 & -576 & -576 & 864 & 4590 & 1728 & 1728 \\ -2952 & 864 & 1944 & -1152 & 8694 & 864 & -6066 & -2016 & -216 & 864 & -216 & -576 & -5022 & 864 & 2394 & 1728 \\ 0 & -2376 & 864 & 1080 & 864 & 5634 & 864 & -3726 & -576 & -216 & 864 & -216 & -2880 & -2826 & 864 & 1350 \\ 0 & 0 & -1512 & 864 & 864 & 864 & 3294 & 864 & -576 & -576 & -216 & 864 & -2880 & -2880 & -1782 & 864 \\ 864 & 2520 & -1152 & -1152 & 864 & 2520 & -1152 & -1152 & 864 & -5022 & -2880 & -2880 & 864 & -216 & -576 & -576 \\ -2952 & 864 & 1944 & -1152 & -2952 & 864 & 1944 & -1152 & 4590 & 864 & -2826 & -2880 & -216 & 864 & -216 & -576 \\ 0 & -2376 & 864 & 1080 & 0 & -2376 & 864 & 1080 & 1728 & 2394 & 864 & -1782 & -576 & -216 & 864 & -216 \\ 0 & 0 & -1512 & 864 & 0 & 0 & -1512 & 864 & 1728 & 1728 & 1350 & 864 & -576 & -576 & -216 & 864 \end{pmatrix}$$

$S = \{1234, 1243, 1432, 2314, 2341, 2413, 3142, 3214, 3421, 4123, 4132, 4321\}, \lambda_{max} = 0.154921, \lambda_{min} = -0.048221$

$$H_S = \frac{1}{6 \cdot 5^6} \times \begin{pmatrix}
3456 & -864 & -2304 & -2304 & 216 & 6246 & -144 & -144 & -864 & 216 & 576 & 576 & -864 & 216 & 576 & 576 \\
-864 & 3456 & -864 & -2304 & -6354 & 216 & 4446 & -144 & 216 & -864 & 216 & 576 & 216 & -864 & 216 & 576 \\
-2304 & -864 & 3456 & -864 & -144 & -4554 & 216 & 2646 & 576 & 216 & -864 & 216 & 576 & 216 & -864 & 216 \\
-2304 & -2304 & -864 & 3456 & -144 & -144 & -2754 & 216 & 576 & 576 & 216 & -864 & 576 & 576 & 216 & -864 \\
216 & -6354 & -144 & -144 & 3456 & -864 & -2304 & -2304 & 216 & -54 & -144 & -144 & -864 & 216 & 576 & 576 \\
6246 & 216 & -4554 & -144 & -864 & 3456 & -864 & -2304 & -54 & 216 & -54 & -144 & 216 & -864 & 216 & 576 \\
-144 & 4446 & 216 & -2754 & -2304 & -864 & 3456 & -864 & -144 & -54 & 216 & -54 & 576 & 216 & -864 & 216 \\
-144 & -144 & 2646 & 216 & -2304 & -2304 & -864 & 3456 & -144 & -144 & -54 & 216 & 576 & 576 & 216 & -864 \\
-864 & 216 & 576 & 576 & 216 & -54 & -144 & -144 & 3456 & -864 & -2304 & -2304 & 216 & -6354 & -144 & -144 \\
216 & -864 & 216 & 576 & -54 & 216 & -54 & -144 & -864 & 3456 & -864 & -2304 & 6246 & 216 & -4554 & -144 \\
576 & 216 & -864 & 216 & -144 & -54 & 216 & -54 & -2304 & -864 & 3456 & -864 & -144 & 4446 & 216 & -2754 \\
576 & 576 & 216 & -864 & -144 & -144 & -54 & 216 & -2304 & -2304 & -864 & 3456 & -144 & -144 & 2646 & 216 \\
-864 & 216 & 576 & 576 & -864 & 216 & 576 & 576 & 216 & 6246 & -144 & -144 & 3456 & -864 & -2304 & -2304 \\
216 & -864 & 216 & 576 & 216 & -864 & 216 & 576 & -6354 & 216 & 4446 & -144 & -864 & 3456 & -864 & -2304 \\
576 & 216 & -864 & 216 & 576 & 216 & -864 & 216 & -144 & -4554 & 216 & 2646 & -2304 & -864 & 3456 & -864 \\
576 & 576 & 216 & -864 & 576 & 576 & 216 & -864 & -144 & -144 & -2754 & 216 & -2304 & -2304 & -864 & 3456
\end{pmatrix}$$

$S = \{1234, 1324, 1342, 2143, 2413, 2431, 3124, 3142, 3412, 4213, 4231, 4321\}, \lambda_{max} = 0.029371, \lambda_{min} = -0.141866$

$$H_S = \frac{1}{6 \cdot 5^6} \times \begin{pmatrix}
-1728 & 432 & 1152 & 1152 & -1728 & 432 & 1152 & 1152 & -1728 & 432 & 1152 & 1152 & -1728 & 432 & 1152 & 1152 \\
432 & -1728 & 432 & 1152 & 432 & -1728 & 432 & 1152 & 432 & -1728 & 432 & 1152 & 432 & -1728 & 432 & 1152 \\
1152 & 432 & -1728 & 432 & 1152 & 432 & -1728 & 432 & 1152 & 432 & -1728 & 432 & 1152 & 432 & -1728 & 432 \\
1152 & 1152 & 432 & -1728 & 1152 & 1152 & 432 & -1728 & 1152 & 1152 & 432 & -1728 & 1152 & 1152 & 432 & -1728 \\
-1728 & 432 & 1152 & 1152 & -1728 & 432 & 1152 & 1152 & -1728 & 432 & 1152 & 1152 & -1728 & 432 & 1152 & 1152 \\
432 & -1728 & 432 & 1152 & 432 & -1728 & 432 & 1152 & 432 & -1728 & 432 & 1152 & 432 & -1728 & 432 & 1152 \\
1152 & 432 & -1728 & 432 & 1152 & 432 & -1728 & 432 & 1152 & 432 & -1728 & 432 & 1152 & 432 & -1728 & 432 \\
1152 & 1152 & 432 & -1728 & 1152 & 1152 & 432 & -1728 & 1152 & 1152 & 432 & -1728 & 1152 & 1152 & 432 & -1728 \\
-1728 & 432 & 1152 & 1152 & -1728 & 432 & 1152 & 1152 & -1728 & 432 & 1152 & 1152 & -1728 & 432 & 1152 & 1152 \\
432 & -1728 & 432 & 1152 & 432 & -1728 & 432 & 1152 & 432 & -1728 & 432 & 1152 & 432 & -1728 & 432 & 1152 \\
1152 & 432 & -1728 & 432 & 1152 & 432 & -1728 & 432 & 1152 & 432 & -1728 & 432 & 1152 & 432 & -1728 & 432 \\
1152 & 1152 & 432 & -1728 & 1152 & 1152 & 432 & -1728 & 1152 & 1152 & 432 & -1728 & 1152 & 1152 & 432 & -1728 \\
-1728 & 432 & 1152 & 1152 & -1728 & 432 & 1152 & 1152 & -1728 & 432 & 1152 & 1152 & -1728 & 432 & 1152 & 1152 \\
432 & -1728 & 432 & 1152 & 432 & -1728 & 432 & 1152 & 432 & -1728 & 432 & 1152 & 432 & -1728 & 432 & 1152 \\
1152 & 432 & -1728 & 432 & 1152 & 432 & -1728 & 432 & 1152 & 432 & -1728 & 432 & 1152 & 432 & -1728 & 432 \\
1152 & 1152 & 432 & -1728 & 1152 & 1152 & 432 & -1728 & 1152 & 1152 & 432 & -1728 & 1152 & 1152 & 432 & -1728
\end{pmatrix}$$

$S = \{1234, 1324, 1342, 2143, 2413, 2431, 3124, 3142, 3421, 4213, 4231, 4312\}, \lambda_{max} = 0.028730, \lambda_{min} = -0.129431$

$$H_S = \frac{1}{6 \cdot 5^6} \times \begin{pmatrix}
-4320 & 1080 & 2880 & 2880 & -1080 & 432 & 288 & 288 & 0 & -432 & 1152 & 1152 & 0 & -432 & 1152 & 1152 \\
1080 & -4320 & 1080 & 2880 & 108 & -1080 & 540 & 288 & 432 & 0 & -720 & 1152 & 432 & 0 & -720 & 1152 \\
2880 & 1080 & -4320 & 1080 & 1152 & 0 & -1080 & 432 & -1152 & 720 & 0 & -432 & -1152 & 720 & 0 & -432 \\
2880 & 2880 & 1080 & -4320 & 1152 & 1152 & 108 & -1080 & -1152 & -1152 & 432 & 0 & -1152 & -1152 & 432 & 0 \\
-1080 & 108 & 1152 & 1152 & -4320 & 1080 & 2880 & 2880 & -1080 & 540 & 0 & 0 & 0 & -432 & 1152 & 1152 \\
432 & -1080 & 0 & 1152 & 1080 & -4320 & 1080 & 2880 & 0 & -1080 & 720 & 0 & 432 & 0 & -720 & 1152 \\
288 & 540 & -1080 & 108 & 2880 & 1080 & -4320 & 1080 & 1440 & -180 & -1080 & 540 & -1152 & 720 & 0 & -432 \\
288 & 288 & 432 & -1080 & 2880 & 2880 & 1080 & -4320 & 1440 & 1440 & 0 & -1080 & -1152 & -1152 & 432 & 0 \\
0 & 432 & -1152 & -1152 & -1080 & 0 & 1440 & 1440 & -4320 & 1080 & 2880 & 2880 & -1080 & 432 & 288 & 288 \\
-432 & 0 & 720 & -1152 & 540 & -1080 & -180 & 1440 & 1080 & -4320 & 1080 & 2880 & 108 & -1080 & 540 & 288 \\
1152 & -720 & 0 & 432 & 0 & 720 & -1080 & 0 & 2880 & 1080 & -4320 & 1080 & 1152 & 0 & -1080 & 432 \\
1152 & 1152 & -432 & 0 & 0 & 0 & 540 & -1080 & 2880 & 2880 & 1080 & -4320 & 1152 & 1152 & 108 & -1080 \\
0 & 432 & -1152 & -1152 & 0 & 432 & -1152 & -1152 & -1080 & 108 & 1152 & 1152 & -4320 & 1080 & 2880 & 2880 \\
-432 & 0 & 720 & -1152 & -432 & 0 & 720 & -1152 & 432 & -1080 & 0 & 1152 & 1080 & -4320 & 1080 & 2880 \\
1152 & -720 & 0 & 432 & 1152 & -720 & 0 & 432 & 288 & 540 & -1080 & 108 & 2880 & 1080 & -4320 & 1080 \\
1152 & 1152 & -432 & 0 & 1152 & 1152 & -432 & 0 & 288 & 288 & 432 & -1080 & 2880 & 2880 & 1080 & -4320
\end{pmatrix}$$

$S = \{1234, 1324, 1342, 2143, 2413, 2431, 3124, 3241, 3412, 4132, 4213, 4321\}, \lambda_{max} = 0.105871, \lambda_{min} = -0.111466$

$$H_S = \frac{1}{6 \cdot 5^6} \times \begin{pmatrix}
-864 & 216 & 576 & 576 & -864 & -1134 & 4176 & 4176 & -864 & 216 & 576 & 576 & -864 & 216 & 576 & 576 \\
216 & -864 & 216 & 576 & 1566 & -864 & -2034 & 4176 & 216 & -864 & 216 & 576 & 216 & -864 & 216 & 576 \\
576 & 216 & -864 & 216 & -3024 & 2466 & -864 & -1134 & 576 & 216 & -864 & 216 & 576 & 216 & -864 & 216 \\
576 & 576 & 216 & -864 & -3024 & -3024 & 1566 & -864 & 576 & 576 & 216 & -864 & 576 & 576 & 216 & -864 \\
-864 & 1566 & -3024 & -3024 & -864 & 216 & 576 & 576 & -864 & -1134 & 4176 & 4176 & -864 & 216 & 576 & 576 \\
-1134 & -864 & 2466 & -3024 & 216 & -864 & 216 & 576 & 1566 & -864 & -2034 & 4176 & 216 & -864 & 216 & 576 \\
4176 & -2034 & -864 & 1566 & 576 & 216 & -864 & 216 & -3024 & 2466 & -864 & -1134 & 576 & 216 & -864 & 216 \\
4176 & 4176 & -1134 & -864 & 576 & 576 & 216 & -864 & -3024 & -3024 & 1566 & -864 & 576 & 576 & 216 & -864 \\
-864 & 216 & 576 & 576 & -864 & 1566 & -3024 & -3024 & -864 & 216 & 576 & 576 & -864 & -1134 & 4176 & 4176 \\
216 & -864 & 216 & 576 & -1134 & -864 & 2466 & -3024 & 216 & -864 & 216 & 576 & 1566 & -864 & -2034 & 4176 \\
576 & 216 & -864 & 216 & 4176 & -2034 & -864 & 1566 & 576 & 216 & -864 & 216 & -3024 & 2466 & -864 & -1134 \\
576 & 576 & 216 & -864 & 4176 & 4176 & -1134 & -864 & 576 & 576 & 216 & -864 & -3024 & -3024 & 1566 & -864 \\
-864 & 216 & 576 & 576 & -864 & 216 & 576 & 576 & -864 & 1566 & -3024 & -3024 & -864 & 216 & 576 & 576 \\
216 & -864 & 216 & 576 & 216 & -864 & 216 & 576 & -1134 & -864 & 2466 & -3024 & 216 & -864 & 216 & 576 \\
576 & 216 & -864 & 216 & 576 & 216 & -864 & 216 & 4176 & -2034 & -864 & 1566 & 576 & 216 & -864 & 216 \\
576 & 576 & 216 & -864 & 576 & 576 & 216 & -864 & 4176 & 4176 & -1134 & -864 & 576 & 576 & 216 & -864
\end{pmatrix}$$

$S = \{1234, 1324, 1342, 2143, 2413, 2431, 3124, 3241, 3421, 4132, 4213, 4312\}, \lambda_{max} = 0.066722, \lambda_{min} = -0.162704$

$$H_S = \frac{1}{6 \cdot 5^6} \times \begin{pmatrix}
-3456 & 864 & 2304 & 2304 & -216 & -1134 & 3312 & 3312 & 864 & -648 & 576 & 576 & 864 & -648 & 576 & 576 \\
864 & -3456 & 864 & 2304 & 1242 & -216 & -1926 & 3312 & 216 & 864 & -936 & 576 & 216 & 864 & -936 & 576 \\
2304 & 864 & -3456 & 864 & -3024 & 2034 & -216 & -1134 & -1728 & 504 & 864 & -648 & -1728 & 504 & 864 & -648 \\
2304 & 2304 & 864 & -3456 & -3024 & -3024 & 1242 & -216 & -1728 & -1728 & 216 & 864 & -1728 & -1728 & 216 & 864 \\
-216 & 1242 & -3024 & -3024 & -3456 & 864 & 2304 & 2304 & -216 & -1026 & 3024 & 3024 & 864 & -648 & 576 & 576 \\
-1134 & -216 & 2034 & -3024 & 864 & -3456 & 864 & 2304 & 1134 & -216 & -1746 & 3024 & 216 & 864 & -936 & 576 \\
3312 & -1926 & -216 & 1242 & 2304 & 864 & -3456 & 864 & -2736 & 1854 & -216 & -1026 & -1728 & 504 & 864 & -648 \\
3312 & 3312 & -1134 & -216 & 2304 & 2304 & 864 & -3456 & -2736 & -2736 & 1134 & -216 & -1728 & -1728 & 216 & 864 \\
864 & 216 & -1728 & -1728 & -216 & 1134 & -2736 & -2736 & -3456 & 864 & 2304 & 2304 & -216 & -1134 & 3312 & 3312 \\
-648 & 864 & 504 & -1728 & -1026 & -216 & 1854 & -2736 & 864 & -3456 & 864 & 2304 & 1242 & -216 & -1926 & 3312 \\
576 & -936 & 864 & 216 & 3024 & -1746 & -216 & 1134 & 2304 & 864 & -3456 & 864 & -3024 & 2034 & -216 & -1134 \\
576 & 576 & -648 & 864 & 3024 & 3024 & -1026 & -216 & 2304 & 2304 & 864 & -3456 & -3024 & -3024 & 1242 & -216 \\
864 & 216 & -1728 & -1728 & 864 & 216 & -1728 & -1728 & -216 & 1242 & -3024 & -3024 & -3456 & 864 & 2304 & 2304 \\
-648 & 864 & 504 & -1728 & -648 & 864 & 504 & -1728 & -1134 & -216 & 2034 & -3024 & 864 & -3456 & 864 & 2304 \\
576 & -936 & 864 & 216 & 576 & -936 & 864 & 216 & 3312 & -1926 & -216 & 1242 & 2304 & 864 & -3456 & 864 \\
576 & 576 & -648 & 864 & 576 & 576 & -648 & 864 & 3312 & 3312 & -1134 & -216 & 2304 & 2304 & 864 & -3456
\end{pmatrix}$$

$S = \{1234, 1324, 1342, 2143, 2413, 2431, 3142, 3214, 3412, 4123, 4231, 4321\}, \lambda_{max} = 0.108526, \lambda_{min} = -0.097958$

$$H_S = \frac{1}{6 \cdot 5^6} \times \begin{pmatrix}
1728 & -432 & -1152 & -1152 & -1512 & -162 & 2448 & 2448 & -2592 & 648 & 1728 & 1728 & -2592 & 648 & 1728 & 1728 \\
-432 & 1728 & -432 & -1152 & 918 & -1512 & -522 & 2448 & 648 & -2592 & 648 & 1728 & 648 & -2592 & 648 & 1728 \\
-1152 & -432 & 1728 & -432 & -432 & 1278 & -1512 & -162 & 1728 & 648 & -2592 & 648 & 1728 & 648 & -2592 & 648 \\
-1152 & -1152 & -432 & 1728 & -432 & -432 & 918 & -1512 & 1728 & 1728 & 648 & -2592 & 1728 & 1728 & 648 & -2592 \\
-1512 & 918 & -432 & -432 & 1728 & -432 & -1152 & -1152 & -1512 & 378 & 1008 & 1008 & -2592 & 648 & 1728 & 1728 \\
-162 & -1512 & 1278 & -432 & -432 & 1728 & -432 & -1152 & 378 & -1512 & 378 & 1008 & 648 & -2592 & 648 & 1728 \\
2448 & -522 & -1512 & 918 & -1152 & -432 & 1728 & -432 & 1008 & 378 & -1512 & 378 & 1728 & 648 & -2592 & 648 \\
2448 & 2448 & -162 & -1512 & -1152 & -1152 & -432 & 1728 & 1008 & 1008 & 378 & -1512 & 1728 & 1728 & 648 & -2592 \\
-2592 & 648 & 1728 & 1728 & -1512 & 378 & 1008 & 1008 & 1728 & -432 & -1152 & -1152 & -1512 & 918 & -432 & -432 \\
648 & -2592 & 648 & 1728 & 378 & -1512 & 378 & 1008 & -432 & 1728 & -432 & -1152 & -162 & -1512 & 1278 & -432 \\
1728 & 648 & -2592 & 648 & 1008 & 378 & -1512 & 378 & -1152 & -432 & 1728 & -432 & 2448 & -522 & -1512 & 918 \\
1728 & 1728 & 648 & -2592 & 1008 & 1008 & 378 & -1512 & -1152 & -1152 & -432 & 1728 & 2448 & 2448 & -162 & -1512 \\
-2592 & 648 & 1728 & 1728 & -2592 & 648 & 1728 & 1728 & -1512 & -162 & 2448 & 2448 & 1728 & -432 & -1152 & -1152 \\
648 & -2592 & 648 & 1728 & 648 & -2592 & 648 & 1728 & 918 & -1512 & -522 & 2448 & -432 & 1728 & -432 & -1152 \\
1728 & 648 & -2592 & 648 & 1728 & 648 & -2592 & 648 & -432 & 1278 & -1512 & -162 & -1152 & -432 & 1728 & -432 \\
1728 & 1728 & 648 & -2592 & 1728 & 1728 & 648 & -2592 & -432 & -432 & 918 & -1512 & -1152 & -1152 & -432 & 1728
\end{pmatrix}$$

$S = \{1234, 1324, 1342, 2143, 2413, 2431, 3142, 3214, 3421, 4123, 4231, 4312\}, \lambda_{max} = 0.046613, \lambda_{min} = -0.086168$

$$H_S = \frac{1}{6 \cdot 5^6} \times \begin{pmatrix}
-864 & 216 & 576 & 576 & -864 & -162 & 1584 & 1584 & -864 & -216 & 1728 & 1728 & -864 & -216 & 1728 & 1728 \\
216 & -864 & 216 & 576 & 594 & -864 & -414 & 1584 & 648 & -864 & -504 & 1728 & 648 & -864 & -504 & 1728 \\
576 & 216 & -864 & 216 & -432 & 846 & -864 & -162 & -576 & 936 & -864 & -216 & -576 & 936 & -864 & -216 \\
576 & 576 & 216 & -864 & -432 & -432 & 594 & -864 & -576 & -576 & 648 & -864 & -576 & -576 & 648 & -864 \\
-864 & 594 & -432 & -432 & -864 & 216 & 576 & 576 & -864 & 486 & -144 & -144 & -864 & -216 & 1728 & 1728 \\
-162 & -864 & 846 & -432 & 216 & -864 & 216 & 576 & -54 & -864 & 666 & -144 & 648 & -864 & -504 & 1728 \\
1584 & -414 & -864 & 594 & 576 & 216 & -864 & 216 & 1296 & -234 & -864 & 486 & -576 & 936 & -864 & -216 \\
1584 & 1584 & -162 & -864 & 576 & 576 & 216 & -864 & 1296 & 1296 & -54 & -864 & -576 & -576 & 648 & -864 \\
-864 & 648 & -576 & -576 & -864 & -54 & 1296 & 1296 & -864 & 216 & 576 & 576 & -864 & 918 & -1296 & -1296 \\
-216 & -864 & 936 & -576 & 486 & -864 & -234 & 1296 & 216 & -864 & 216 & 576 & -486 & -864 & 1386 & -1296 \\
1728 & -504 & -864 & 648 & -144 & 666 & -864 & -54 & 576 & 216 & -864 & 216 & 2448 & -954 & -864 & 918 \\
1728 & 1728 & -216 & -864 & -144 & -144 & 486 & -864 & 576 & 576 & 216 & -864 & 2448 & 2448 & -486 & -864 \\
-864 & 648 & -576 & -576 & -864 & 648 & -576 & -576 & -864 & -486 & 2448 & 2448 & -864 & 216 & 576 & 576 \\
-216 & -864 & 936 & -576 & -216 & -864 & 936 & -576 & 918 & -864 & -954 & 2448 & 216 & -864 & 216 & 576 \\
1728 & -504 & -864 & 648 & 1728 & -504 & -864 & 648 & -1296 & 1386 & -864 & -486 & 576 & 216 & -864 & 216 \\
1728 & 1728 & -216 & -864 & 1728 & 1728 & -216 & -864 & -1296 & -1296 & 918 & -864 & 576 & 576 & 216 & -864
\end{pmatrix}$$

$S = \{1234, 1324, 1342, 2143, 2413, 2431, 3214, 3241, 3412, 4123, 4132, 4321\}, \lambda_{max} = 0.175679, \lambda_{min} = -0.089991$

$$H_S = \frac{1}{6 \cdot 5^6} \times \begin{pmatrix}
2592 & -648 & -1728 & -1728 & -648 & -1728 & 5472 & 5472 & -1728 & 432 & 1152 & 1152 & -1728 & 432 & 1152 & 1152 \\
-648 & 2592 & -648 & -1728 & 2052 & -648 & -2988 & 5472 & 432 & -1728 & 432 & 1152 & 432 & -1728 & 432 & 1152 \\
-1728 & -648 & 2592 & -648 & -4608 & 3312 & -648 & -1728 & 1152 & 432 & -1728 & 432 & 1152 & 432 & -1728 & 432 \\
-1728 & -1728 & -648 & 2592 & -4608 & -4608 & 2052 & -648 & 1152 & 1152 & 432 & -1728 & 1152 & 1152 & 432 & -1728 \\
-648 & 2052 & -4608 & -4608 & 2592 & -648 & -1728 & -1728 & -648 & -1188 & 4032 & 4032 & -1728 & 432 & 1152 & 1152 \\
-1728 & -648 & 3312 & -4608 & -648 & 2592 & -648 & -1728 & 1512 & -648 & -2088 & 4032 & 432 & -1728 & 432 & 1152 \\
5472 & -2988 & -648 & 2052 & -1728 & -648 & 2592 & -648 & -3168 & 2412 & -648 & -1188 & 1152 & 432 & -1728 & 432 \\
5472 & 5472 & -1728 & -648 & -1728 & -1728 & -648 & 2592 & -3168 & -3168 & 1512 & -648 & 1152 & 1152 & 432 & -1728 \\
-1728 & 432 & 1152 & 1152 & -648 & 1512 & -3168 & -3168 & 2592 & -648 & -1728 & -1728 & -648 & -648 & 2592 & 2592 \\
432 & -1728 & 432 & 1152 & -1188 & -648 & 2412 & -3168 & -648 & 2592 & -648 & -1728 & 972 & -648 & -1188 & 2592 \\
1152 & 432 & -1728 & 432 & 4032 & -2088 & -648 & 1512 & -1728 & -648 & 2592 & -648 & -1728 & 1512 & -648 & -648 \\
1152 & 1152 & 432 & -1728 & 4032 & 4032 & -1188 & -648 & -1728 & -1728 & -648 & 2592 & -1728 & -1728 & 972 & -648 \\
-1728 & 432 & 1152 & 1152 & -1728 & 432 & 1152 & 1152 & -648 & 972 & -1728 & -1728 & 2592 & -648 & -1728 & -1728 \\
432 & -1728 & 432 & 1152 & 432 & -1728 & 432 & 1152 & -648 & -648 & 1512 & -1728 & -648 & 2592 & -648 & -1728 \\
1152 & 432 & -1728 & 432 & 1152 & 432 & -1728 & 432 & 2592 & -1188 & -648 & 972 & -1728 & -648 & 2592 & -648 \\
1152 & 1152 & 432 & -1728 & 1152 & 1152 & 432 & -1728 & 2592 & 2592 & -648 & -648 & -1728 & -1728 & -648 & 2592
\end{pmatrix}$$

$S = \{1234, 1324, 1342, 2143, 2413, 2431, 3214, 3241, 3421, 4123, 4132, 4312\}, \lambda_{max} = 0.207470, \lambda_{min} = -0.105497$

$$H_S = \frac{1}{6\cdot 5^6} \times \begin{pmatrix} 0 & 0 & 0 & 0 & 0 & -1728 & 4608 & 4608 & 0 & -432 & 1152 & 1152 & 0 & -432 & 1152 & 1152 \\ 0 & 0 & 0 & 0 & 1728 & 0 & -2880 & 4608 & 432 & 0 & -720 & 1152 & 432 & 0 & -720 & 1152 \\ 0 & 0 & 0 & 0 & -4608 & 2880 & 0 & -1728 & -1152 & 720 & 0 & -432 & -1152 & 720 & 0 & -432 \\ 0 & 0 & 0 & 0 & -4608 & -4608 & 1728 & 0 & -1152 & -1152 & 432 & 0 & -1152 & -1152 & 432 & 0 \\ 0 & 1728 & -4608 & -4608 & 0 & 0 & 0 & 0 & 0 & -1080 & 2880 & 2880 & 0 & -432 & 1152 & 1152 \\ -1728 & 0 & 2880 & -4608 & 0 & 0 & 0 & 0 & 1080 & 0 & -1800 & 2880 & 432 & 0 & -720 & 1152 \\ 4608 & -2880 & 0 & 1728 & 0 & 0 & 0 & 0 & -2880 & 1800 & 0 & -1080 & -1152 & 720 & 0 & -432 \\ 4608 & 4608 & -1728 & 0 & 0 & 0 & 0 & 0 & -2880 & -2880 & 1080 & 0 & -1152 & -1152 & 432 & 0 \\ 0 & 432 & -1152 & -1152 & 0 & 1080 & -2880 & -2880 & 0 & 0 & 0 & 0 & 0 & -648 & 1728 & 1728 \\ -432 & 0 & 720 & -1152 & -1080 & 0 & 1800 & -2880 & 0 & 0 & 0 & 0 & 648 & 0 & -1080 & 1728 \\ 1152 & -720 & 0 & 432 & 2880 & -1800 & 0 & 1080 & 0 & 0 & 0 & 0 & -1728 & 1080 & 0 & -648 \\ 1152 & 1152 & -432 & 0 & 2880 & 2880 & -1080 & 0 & 0 & 0 & 0 & 0 & -1728 & -1728 & 648 & 0 \\ 0 & 432 & -1152 & -1152 & 0 & 432 & -1152 & -1152 & 0 & 648 & -1728 & -1728 & 0 & 0 & 0 & 0 \\ -432 & 0 & 720 & -1152 & -432 & 0 & 720 & -1152 & -648 & 0 & 1080 & -1728 & 0 & 0 & 0 & 0 \\ 1152 & -720 & 0 & 432 & 1152 & -720 & 0 & 432 & 1728 & -1080 & 0 & 648 & 0 & 0 & 0 & 0 \\ 1152 & 1152 & -432 & 0 & 1152 & 1152 & -432 & 0 & 1728 & 1728 & -648 & 0 & 0 & 0 & 0 & 0 \end{pmatrix}$$

$S = \{1234, 1324, 1432, 2143, 2341, 2413, 3142, 3214, 3412, 4123, 4231, 4321\}, \lambda_{max} = 0.204732, \lambda_{min} = -0.042387$

$$H_S = \frac{1}{6\cdot 5^6} \times \begin{pmatrix} 5184 & -1296 & -3456 & -3456 & -1296 & 324 & 864 & 864 & -3456 & 864 & 2304 & 2304 & -3456 & 864 & 2304 & 2304 \\ -1296 & 5184 & -1296 & -3456 & 324 & -1296 & 324 & 864 & 864 & -3456 & 864 & 2304 & 864 & -3456 & 864 & 2304 \\ -3456 & -1296 & 5184 & -1296 & 864 & 324 & -1296 & 324 & 2304 & 864 & -3456 & 864 & 2304 & 864 & -3456 & 864 \\ -3456 & -3456 & -1296 & 5184 & 864 & 864 & 324 & -1296 & 2304 & 2304 & 864 & -3456 & 2304 & 2304 & 864 & -3456 \\ -1296 & 324 & 864 & 864 & 5184 & -1296 & -3456 & -3456 & -1296 & 324 & 864 & 864 & -3456 & 864 & 2304 & 2304 \\ 324 & -1296 & 324 & 864 & -1296 & 5184 & -1296 & -3456 & 324 & -1296 & 324 & 864 & 864 & -3456 & 864 & 2304 \\ 864 & 324 & -1296 & 324 & -3456 & -1296 & 5184 & -1296 & 864 & 324 & -1296 & 324 & 2304 & 864 & -3456 & 864 \\ 864 & 864 & 324 & -1296 & -3456 & -3456 & -1296 & 5184 & 864 & 864 & 324 & -1296 & 2304 & 2304 & 864 & -3456 \\ -3456 & 864 & 2304 & 2304 & -1296 & 324 & 864 & 864 & 5184 & -1296 & -3456 & -3456 & -1296 & 324 & 864 & 864 \\ 864 & -3456 & 864 & 2304 & 324 & -1296 & 324 & 864 & -1296 & 5184 & -1296 & -3456 & 324 & -1296 & 324 & 864 \\ 2304 & 864 & -3456 & 864 & 864 & 324 & -1296 & 324 & -3456 & -1296 & 5184 & -1296 & 864 & 324 & -1296 & 324 \\ 2304 & 2304 & 864 & -3456 & 864 & 864 & 324 & -1296 & -3456 & -3456 & -1296 & 5184 & 864 & 864 & 324 & -1296 \\ -3456 & 864 & 2304 & 2304 & -3456 & 864 & 2304 & 2304 & -1296 & 324 & 864 & 864 & 5184 & -1296 & -3456 & -3456 \\ 864 & -3456 & 864 & 2304 & 864 & -3456 & 864 & 2304 & 324 & -1296 & 324 & 864 & -1296 & 5184 & -1296 & -3456 \\ 2304 & 864 & -3456 & 864 & 2304 & 864 & -3456 & 864 & 864 & 324 & -1296 & 324 & -3456 & -1296 & 5184 & -1296 \\ 2304 & 2304 & 864 & -3456 & 2304 & 2304 & 864 & -3456 & 864 & 864 & 324 & -1296 & -3456 & -3456 & -1296 & 5184 \end{pmatrix}$$

$S = \{1234, 1324, 1432, 2143, 2341, 2413, 3142, 3214, 3421, 4123, 4231, 4312\}, \lambda_{max} = 0.111963, \lambda_{min} = -0.045516$

$$H_S = \frac{1}{6\cdot 5^6} \times \begin{pmatrix} 2592 & -648 & -1728 & -1728 & -648 & 324 & 0 & 0 & -1728 & 0 & 2304 & 2304 & -1728 & 0 & 2304 & 2304 \\ -648 & 2592 & -648 & -1728 & 0 & -648 & 432 & 0 & 864 & -1728 & -288 & 2304 & 864 & -1728 & -288 & 2304 \\ -1728 & -648 & 2592 & -648 & 864 & -108 & -648 & 324 & 0 & 1152 & -1728 & 0 & 0 & 1152 & -1728 & 0 \\ -1728 & -1728 & -648 & 2592 & 864 & 864 & 0 & -648 & 0 & 0 & 864 & -1728 & 0 & 0 & 864 & -1728 \\ -648 & 0 & 864 & 864 & 2592 & -648 & -1728 & -1728 & -648 & 432 & -288 & -288 & -1728 & 0 & 2304 & 2304 \\ 324 & -648 & -108 & 864 & -648 & 2592 & -648 & -1728 & -108 & -648 & 612 & -288 & 864 & -1728 & -288 & 2304 \\ 0 & 432 & -648 & 0 & -1728 & -648 & 2592 & -648 & 1152 & -288 & -648 & 432 & 0 & 1152 & -1728 & 0 \\ 0 & 0 & 324 & -648 & -1728 & -1728 & -648 & 2592 & 1152 & 1152 & -108 & -648 & 0 & 0 & 864 & -1728 \\ -1728 & 864 & 0 & 0 & -648 & -108 & 1152 & 1152 & 2592 & -648 & -1728 & -1728 & -648 & 324 & 0 & 0 \\ 0 & -1728 & 1152 & 0 & 432 & -648 & -288 & 1152 & -648 & 2592 & -648 & -1728 & 0 & -648 & 432 & 0 \\ 2304 & -288 & -1728 & 864 & -288 & 612 & -648 & -108 & -1728 & -648 & 2592 & -648 & 864 & -108 & -648 & 324 \\ 2304 & 2304 & 0 & -1728 & -288 & -288 & 432 & -648 & -1728 & -1728 & -648 & 2592 & 864 & 864 & 0 & -648 \\ -1728 & 864 & 0 & 0 & -1728 & 864 & 0 & 0 & -648 & 0 & 864 & 864 & 2592 & -648 & -1728 & -1728 \\ 0 & -1728 & 1152 & 0 & 0 & -1728 & 1152 & 0 & 324 & -648 & -108 & 864 & -648 & 2592 & -648 & -1728 \\ 2304 & -288 & -1728 & 864 & 2304 & -288 & -1728 & 864 & 0 & 432 & -648 & 0 & -1728 & -648 & 2592 & -648 \\ 2304 & 2304 & 0 & -1728 & 2304 & 2304 & 0 & -1728 & 0 & 0 & 324 & -648 & -1728 & -1728 & -648 & 2592 \end{pmatrix}$$

$S = \{1234, 1324, 1432, 2143, 2341, 2413, 3214, 3241, 3412, 4123, 4132, 4321\}, \lambda_{max} = 0.249596, \lambda_{min} = -0.073147$

$$H_S = \frac{1}{6\cdot 5^6} \times \begin{pmatrix} 6048 & -1512 & -4032 & -4032 & -432 & -1242 & 3888 & 3888 & -2592 & 648 & 1728 & 1728 & -2592 & 648 & 1728 & 1728 \\ -1512 & 6048 & -1512 & -4032 & 1458 & -432 & -2142 & 3888 & 648 & -2592 & 648 & 1728 & 648 & -2592 & 648 & 1728 \\ -4032 & -1512 & 6048 & -1512 & -3312 & 2358 & -432 & -1242 & 1728 & 648 & -2592 & 648 & 1728 & 648 & -2592 & 648 \\ -4032 & -4032 & -1512 & 6048 & -3312 & -3312 & 1458 & -432 & 1728 & 1728 & 648 & -2592 & 1728 & 1728 & 648 & -2592 \\ -432 & 1458 & -3312 & -3312 & 6048 & -1512 & -4032 & -4032 & -432 & -1242 & 3888 & 3888 & -2592 & 648 & 1728 & 1728 \\ -1242 & -432 & 2358 & -3312 & -1512 & 6048 & -1512 & -4032 & 1458 & -432 & -2142 & 3888 & 648 & -2592 & 648 & 1728 \\ 3888 & -2142 & -432 & 1458 & -4032 & -1512 & 6048 & -1512 & -3312 & 2358 & -432 & -1242 & 1728 & 648 & -2592 & 648 \\ 3888 & 3888 & -1242 & -432 & -4032 & -4032 & -1512 & 6048 & -3312 & -3312 & 1458 & -432 & 1728 & 1728 & 648 & -2592 \\ -2592 & 648 & 1728 & 1728 & -432 & 1458 & -3312 & -3312 & 6048 & -1512 & -4032 & -4032 & -432 & -1242 & 3888 & 3888 \\ 648 & -2592 & 648 & 1728 & -1242 & -432 & 2358 & -3312 & -1512 & 6048 & -1512 & -4032 & 1458 & -432 & -2142 & 3888 \\ 1728 & 648 & -2592 & 648 & 3888 & -2142 & -432 & 1458 & -4032 & -1512 & 6048 & -1512 & -3312 & 2358 & -432 & -1242 \\ 1728 & 1728 & 648 & -2592 & 3888 & 3888 & -1242 & -432 & -4032 & -4032 & -1512 & 6048 & -3312 & -3312 & 1458 & -432 \\ -2592 & 648 & 1728 & 1728 & -2592 & 648 & 1728 & 1728 & -432 & 1458 & -3312 & -3312 & 6048 & -1512 & -4032 & -4032 \\ 648 & -2592 & 648 & 1728 & 648 & -2592 & 648 & 1728 & -1242 & -432 & 2358 & -3312 & -1512 & 6048 & -1512 & -4032 \\ 1728 & 648 & -2592 & 648 & 1728 & 648 & -2592 & 648 & 3888 & -2142 & -432 & 1458 & -4032 & -1512 & 6048 & -1512 \\ 1728 & 1728 & 648 & -2592 & 1728 & 1728 & 648 & -2592 & 3888 & 3888 & -1242 & -432 & -4032 & -4032 & -1512 & 6048 \end{pmatrix}$$

$S = \{1234, 1342, 1423, 2143, 2314, 2413, 3124, 3241, 3421, 4132, 4231, 4312\}, \lambda_{max} = 0.097927, \lambda_{min} = -0.191879$

$$H_S = \frac{1}{6 \cdot 5^6} \times \begin{pmatrix} -3456 & -216 & 864 & 864 & 864 & 1566 & -648 & -648 & 2304 & -3888 & 576 & 576 & 2304 & -3888 & 576 & 576 \\ -216 & -3456 & -216 & 864 & -1458 & 864 & 1674 & -648 & 4176 & 2304 & -4176 & 576 & 4176 & 2304 & -4176 & 576 \\ 864 & -216 & -3456 & -216 & 216 & -1566 & 864 & 1566 & -1728 & 4464 & 2304 & -3888 & -1728 & 4464 & 2304 & -3888 \\ 864 & 864 & -216 & -3456 & 216 & 216 & -1458 & 864 & -1728 & -1728 & 4176 & 2304 & -1728 & -1728 & 4176 & 2304 \\ 864 & -1458 & 216 & 216 & -3456 & -216 & 864 & 864 & 864 & 2574 & -936 & -936 & 2304 & -3888 & 576 & 576 \\ 1566 & 864 & -1566 & 216 & -216 & -3456 & -216 & 864 & -2466 & 864 & 2754 & -936 & 4176 & 2304 & -4176 & 576 \\ -648 & 1674 & 864 & -1458 & 864 & -216 & -3456 & -216 & 504 & -2646 & 864 & 2574 & -1728 & 4464 & 2304 & -3888 \\ -648 & -648 & 1566 & 864 & 864 & 864 & -216 & -3456 & 504 & 504 & -2466 & 864 & -1728 & -1728 & 4176 & 2304 \\ 2304 & 4176 & -1728 & -1728 & 864 & -2466 & 504 & 504 & -3456 & -216 & 864 & 864 & 864 & 1566 & -648 & -648 \\ -3888 & 2304 & 4464 & -1728 & 2574 & 864 & -2646 & 504 & -216 & -3456 & -216 & 864 & -1458 & 864 & 1674 & -648 \\ 576 & -4176 & 2304 & 4176 & -936 & 2754 & 864 & -2466 & 864 & -216 & -3456 & -216 & 216 & -1566 & 864 & 1566 \\ 576 & 576 & -3888 & 2304 & -936 & -936 & 2574 & 864 & 864 & 864 & -216 & -3456 & 216 & 216 & -1458 & 864 \\ 2304 & 4176 & -1728 & -1728 & 2304 & 4176 & -1728 & -1728 & 864 & -1458 & 216 & 216 & -3456 & -216 & 864 & 864 \\ -3888 & 2304 & 4464 & -1728 & -3888 & 2304 & 4464 & -1728 & 1566 & 864 & -1566 & 216 & -216 & -3456 & -216 & 864 \\ 576 & -4176 & 2304 & 4176 & 576 & -4176 & 2304 & 4176 & -648 & 1674 & 864 & -1458 & 864 & -216 & -3456 & -216 \\ 576 & 576 & -3888 & 2304 & 576 & 576 & -3888 & 2304 & -648 & -648 & 1566 & 864 & 864 & 864 & -216 & -3456 \end{pmatrix}$$

$\mathbf{S = \{1234, 1342, 1423, 2143, 2314, 2431, 3124, 3241, 3412, 4132, 4213, 4321\}}, \lambda_{max} = 0, \lambda_{min} = 0$

$$H_S = \frac{1}{6 \cdot 5^6} \times \begin{pmatrix} 0 & 0 & 0 & 0 & 0 & 0 & 0 & 0 & 0 & 0 & 0 & 0 & 0 & 0 & 0 & 0 \\ 0 & 0 & 0 & 0 & 0 & 0 & 0 & 0 & 0 & 0 & 0 & 0 & 0 & 0 & 0 & 0 \\ 0 & 0 & 0 & 0 & 0 & 0 & 0 & 0 & 0 & 0 & 0 & 0 & 0 & 0 & 0 & 0 \\ 0 & 0 & 0 & 0 & 0 & 0 & 0 & 0 & 0 & 0 & 0 & 0 & 0 & 0 & 0 & 0 \\ 0 & 0 & 0 & 0 & 0 & 0 & 0 & 0 & 0 & 0 & 0 & 0 & 0 & 0 & 0 & 0 \\ 0 & 0 & 0 & 0 & 0 & 0 & 0 & 0 & 0 & 0 & 0 & 0 & 0 & 0 & 0 & 0 \\ 0 & 0 & 0 & 0 & 0 & 0 & 0 & 0 & 0 & 0 & 0 & 0 & 0 & 0 & 0 & 0 \\ 0 & 0 & 0 & 0 & 0 & 0 & 0 & 0 & 0 & 0 & 0 & 0 & 0 & 0 & 0 & 0 \\ 0 & 0 & 0 & 0 & 0 & 0 & 0 & 0 & 0 & 0 & 0 & 0 & 0 & 0 & 0 & 0 \\ 0 & 0 & 0 & 0 & 0 & 0 & 0 & 0 & 0 & 0 & 0 & 0 & 0 & 0 & 0 & 0 \\ 0 & 0 & 0 & 0 & 0 & 0 & 0 & 0 & 0 & 0 & 0 & 0 & 0 & 0 & 0 & 0 \\ 0 & 0 & 0 & 0 & 0 & 0 & 0 & 0 & 0 & 0 & 0 & 0 & 0 & 0 & 0 & 0 \\ 0 & 0 & 0 & 0 & 0 & 0 & 0 & 0 & 0 & 0 & 0 & 0 & 0 & 0 & 0 & 0 \\ 0 & 0 & 0 & 0 & 0 & 0 & 0 & 0 & 0 & 0 & 0 & 0 & 0 & 0 & 0 & 0 \\ 0 & 0 & 0 & 0 & 0 & 0 & 0 & 0 & 0 & 0 & 0 & 0 & 0 & 0 & 0 & 0 \\ 0 & 0 & 0 & 0 & 0 & 0 & 0 & 0 & 0 & 0 & 0 & 0 & 0 & 0 & 0 & 0 \end{pmatrix}$$

$S = \{1234, 1342, 1423, 2143, 2314, 2431, 3142, 3214, 3421, 4123, 4231, 4312\}, \lambda_{max} = 0.268415, \lambda_{min} = -0.139013$

$$H_S = \frac{1}{6 \cdot 5^6} \times \begin{pmatrix} 0 & 0 & 0 & 0 & 0 & 972 & -2592 & -2592 & 0 & -432 & 1152 & 1152 & 0 & -432 & 1152 & 1152 \\ 0 & 0 & 0 & 0 & -972 & 0 & 1620 & -2592 & 432 & 0 & -720 & 1152 & 432 & 0 & -720 & 1152 \\ 0 & 0 & 0 & 0 & 2592 & -1620 & 0 & 972 & -1152 & 720 & 0 & -432 & -1152 & 720 & 0 & -432 \\ 0 & 0 & 0 & 0 & 2592 & 2592 & -972 & 0 & -1152 & -1152 & 432 & 0 & -1152 & -1152 & 432 & 0 \\ 0 & -972 & 2592 & 2592 & 0 & 0 & 0 & 0 & 0 & 1620 & -4320 & -4320 & 0 & -432 & 1152 & 1152 \\ 972 & 0 & -1620 & 2592 & 0 & 0 & 0 & 0 & -1620 & 0 & 2700 & -4320 & 432 & 0 & -720 & 1152 \\ -2592 & 1620 & 0 & -972 & 0 & 0 & 0 & 0 & 4320 & -2700 & 0 & 1620 & -1152 & 720 & 0 & -432 \\ -2592 & -2592 & 972 & 0 & 0 & 0 & 0 & 0 & 4320 & 4320 & -1620 & 0 & -1152 & -1152 & 432 & 0 \\ 0 & 432 & -1152 & -1152 & 0 & -1620 & 4320 & 4320 & 0 & 0 & 0 & 0 & 0 & 2052 & -5472 & -5472 \\ -432 & 0 & 720 & -1152 & 1620 & 0 & -2700 & 4320 & 0 & 0 & 0 & 0 & -2052 & 0 & 3420 & -5472 \\ 1152 & -720 & 0 & 432 & -4320 & 2700 & 0 & -1620 & 0 & 0 & 0 & 0 & 5472 & -3420 & 0 & 2052 \\ 1152 & 1152 & -432 & 0 & -4320 & -4320 & 1620 & 0 & 0 & 0 & 0 & 0 & 5472 & 5472 & -2052 & 0 \\ 0 & 432 & -1152 & -1152 & 0 & 432 & -1152 & -1152 & 0 & -2052 & 5472 & 5472 & 0 & 0 & 0 & 0 \\ -432 & 0 & 720 & -1152 & -432 & 0 & 720 & -1152 & 2052 & 0 & -3420 & 5472 & 0 & 0 & 0 & 0 \\ 1152 & -720 & 0 & 432 & 1152 & -720 & 0 & 432 & -5472 & 3420 & 0 & -2052 & 0 & 0 & 0 & 0 \\ 1152 & 1152 & -432 & 0 & 1152 & 1152 & -432 & 0 & -5472 & -5472 & 2052 & 0 & 0 & 0 & 0 & 0 \end{pmatrix}$$

$S = \{1234, 1342, 1423, 2143, 2314, 2431, 3214, 3241, 3412, 4123, 4132, 4321\}, \lambda_{max} = 0.108526, \lambda_{min} = -0.026756$

$$H_S = \frac{1}{6 \cdot 5^6} \times \begin{pmatrix} 3456 & -864 & -2304 & -2304 & 216 & -594 & 1296 & 1296 & -864 & 216 & 576 & 576 & -864 & 216 & 576 & 576 \\ -864 & 3456 & -864 & -2304 & 486 & 216 & -954 & 1296 & 216 & -864 & 216 & 576 & 216 & -864 & 216 & 576 \\ -2304 & -864 & 3456 & -864 & -1584 & 846 & 216 & -594 & 576 & 216 & -864 & 216 & 576 & 216 & -864 & 216 \\ -2304 & -2304 & -864 & 3456 & -1584 & -1584 & 486 & 216 & 576 & 576 & 216 & -864 & 576 & 576 & 216 & -864 \\ 216 & 486 & -1584 & -1584 & 3456 & -864 & -2304 & -2304 & 216 & -54 & -144 & -144 & -864 & 216 & 576 & 576 \\ -594 & 216 & 846 & -1584 & -864 & 3456 & -864 & -2304 & -54 & 216 & -54 & -144 & 216 & -864 & 216 & 576 \\ 1296 & -954 & 216 & 486 & -2304 & -864 & 3456 & -864 & -144 & -54 & 216 & -54 & 576 & 216 & -864 & 216 \\ 1296 & 1296 & -594 & 216 & -2304 & -2304 & -864 & 3456 & -144 & -144 & -54 & 216 & 576 & 576 & 216 & -864 \\ -864 & 216 & 576 & 576 & 216 & -54 & -144 & -144 & 3456 & -864 & -2304 & -2304 & 216 & 486 & -1584 & -1584 \\ 216 & -864 & 216 & 576 & -54 & 216 & -54 & -144 & -864 & 3456 & -864 & -2304 & -594 & 216 & 846 & -1584 \\ 576 & 216 & -864 & 216 & -144 & -54 & 216 & -54 & -2304 & -864 & 3456 & -864 & 1296 & -954 & 216 & 486 \\ 576 & 576 & 216 & -864 & -144 & -144 & -54 & 216 & -2304 & -2304 & -864 & 3456 & 1296 & 1296 & -594 & 216 \\ -864 & 216 & 576 & 576 & -864 & 216 & 576 & 576 & 216 & -594 & 1296 & 1296 & 3456 & -864 & -2304 & -2304 \\ 216 & -864 & 216 & 576 & 216 & -864 & 216 & 576 & 486 & 216 & -954 & 1296 & -864 & 3456 & -864 & -2304 \\ 576 & 216 & -864 & 216 & 576 & 216 & -864 & 216 & -1584 & 846 & 216 & -594 & -2304 & -864 & 3456 & -864 \\ 576 & 576 & 216 & -864 & 576 & 576 & 216 & -864 & -1584 & -1584 & 486 & 216 & -2304 & -2304 & -864 & 3456 \end{pmatrix}$$

$\mathbf{S = \{1234, 1342, 1423, 2314, 2413, 2431, 3124, 3142, 3241, 4132, 4213, 4321\}}, \lambda_{max} = -0.014289, \lambda_{min} = -0.106988$

$$H_S = \frac{1}{6\cdot 5^6} \times \begin{pmatrix}
-4608 & -288 & 1152 & 1152 & -288 & 1782 & 72 & 72 & 1152 & 72 & -288 & -288 & 1152 & 72 & -288 & -288 \\
-288 & -4608 & -288 & 1152 & -1818 & -288 & -18 & 72 & 72 & 1152 & 72 & -288 & 72 & 1152 & 72 & -288 \\
1152 & -288 & -4608 & -288 & 72 & -18 & -288 & -1818 & -288 & 72 & 1152 & 72 & -288 & 72 & 1152 & 72 \\
1152 & 1152 & -288 & -4608 & 72 & 72 & 1782 & -288 & -288 & -288 & 72 & 1152 & -288 & -288 & 72 & 1152 \\
-288 & -1818 & 72 & 72 & -4608 & -288 & 1152 & 1152 & -288 & -18 & 72 & 72 & 1152 & 72 & -288 & -288 \\
1782 & -288 & -18 & 72 & -288 & -4608 & -288 & 1152 & -18 & -288 & -18 & 72 & 72 & 1152 & 72 & -288 \\
72 & -18 & -288 & 1782 & 1152 & -288 & -4608 & -288 & 72 & -18 & -288 & -18 & -288 & 72 & 1152 & 72 \\
72 & 72 & -1818 & -288 & 1152 & 1152 & -288 & -4608 & 72 & 72 & -18 & -288 & -288 & -288 & 72 & 1152 \\
1152 & 72 & -288 & -288 & -288 & -18 & 72 & 72 & -4608 & -288 & 1152 & 1152 & -288 & -1818 & 72 & 72 \\
72 & 1152 & 72 & -288 & -18 & -288 & -18 & 72 & -288 & -4608 & -288 & 1152 & 1782 & -288 & -18 & 72 \\
-288 & 72 & 1152 & 72 & 72 & -18 & -288 & -18 & 1152 & -288 & -4608 & -288 & 72 & -18 & -288 & 1782 \\
-288 & -288 & 72 & 1152 & 72 & 72 & -18 & -288 & 1152 & 1152 & -288 & -4608 & 72 & 72 & -1818 & -288 \\
1152 & 72 & -288 & -288 & 1152 & 72 & -288 & -288 & -288 & 1782 & 72 & 72 & -4608 & -288 & 1152 & 1152 \\
72 & 1152 & 72 & -288 & 72 & 1152 & 72 & -288 & -1818 & -288 & -18 & 72 & -288 & -4608 & -288 & 1152 \\
-288 & 72 & 1152 & 72 & -288 & 72 & 1152 & 72 & 72 & -18 & -288 & -1818 & 1152 & -288 & -4608 & -288 \\
-288 & -288 & 72 & 1152 & -288 & -288 & 72 & 1152 & 72 & 72 & 1782 & -288 & 1152 & 1152 & -288 & -4608
\end{pmatrix}$$

$S = \{1234, 1342, 1423, 2314, 2413, 2431, 3142, 3214, 3241, 4123, 4132, 4321\}, \lambda_{max} = 0.030952, \lambda_{min} = -0.080481$

$$H_S = \frac{1}{6\cdot 5^6} \times \begin{pmatrix}
-1152 & -1152 & -1152 & -1152 & -72 & 1188 & 1368 & 1368 & 288 & 288 & 288 & 288 & 288 & 288 & 288 & 288 \\
-1152 & -1152 & -1152 & -1152 & -1332 & -72 & -972 & 1368 & 288 & 288 & 288 & 288 & 288 & 288 & 288 & 288 \\
-1152 & -1152 & -1152 & -1152 & -1512 & 828 & -72 & -2412 & 288 & 288 & 288 & 288 & 288 & 288 & 288 & 288 \\
-1152 & -1152 & -1152 & -1152 & -1512 & -1512 & 2268 & -72 & 288 & 288 & 288 & 288 & 288 & 288 & 288 & 288 \\
-72 & -1332 & -1512 & -1512 & -1152 & -1152 & -1152 & -1152 & -72 & -72 & -72 & -72 & 288 & 288 & 288 & 288 \\
1188 & -72 & 828 & -1512 & -1152 & -1152 & -1152 & -1152 & -72 & -72 & -72 & -72 & 288 & 288 & 288 & 288 \\
1368 & -972 & -72 & 2268 & -1152 & -1152 & -1152 & -1152 & -72 & -72 & -72 & -72 & 288 & 288 & 288 & 288 \\
1368 & 1368 & -2412 & -72 & -1152 & -1152 & -1152 & -1152 & -72 & -72 & -72 & -72 & 288 & 288 & 288 & 288 \\
288 & 288 & 288 & 288 & -72 & -72 & -72 & -72 & -1152 & -1152 & -1152 & -1152 & -72 & -1332 & -1512 & -1512 \\
288 & 288 & 288 & 288 & -72 & -72 & -72 & -72 & -1152 & -1152 & -1152 & -1152 & 1188 & -72 & 828 & -1512 \\
288 & 288 & 288 & 288 & -72 & -72 & -72 & -72 & -1152 & -1152 & -1152 & -1152 & 1368 & -972 & -72 & 2268 \\
288 & 288 & 288 & 288 & -72 & -72 & -72 & -72 & -1152 & -1152 & -1152 & -1152 & 1368 & 1368 & -2412 & -72 \\
288 & 288 & 288 & 288 & 288 & 288 & 288 & 288 & -72 & 1188 & 1368 & 1368 & -1152 & -1152 & -1152 & -1152 \\
288 & 288 & 288 & 288 & 288 & 288 & 288 & 288 & -1332 & -72 & -972 & 1368 & -1152 & -1152 & -1152 & -1152 \\
288 & 288 & 288 & 288 & 288 & 288 & 288 & 288 & -1512 & 828 & -72 & -2412 & -1152 & -1152 & -1152 & -1152 \\
288 & 288 & 288 & 288 & 288 & 288 & 288 & 288 & -1512 & -1512 & 2268 & -72 & -1152 & -1152 & -1152 & -1152
\end{pmatrix}$$

$S = \{1234, 1342, 1432, 2143, 2341, 2431, 3124, 3214, 3412, 4123, 4213, 4321\}, \lambda_{max} = 0.204732, \lambda_{min} = -0.042387$

$$H_S = \frac{1}{6\cdot 5^6} \times \begin{pmatrix}
6912 & 432 & -1728 & -1728 & -1728 & -108 & 432 & 432 & -4608 & -288 & 1152 & 1152 & -4608 & -288 & 1152 & 1152 \\
432 & 6912 & 432 & -1728 & -108 & -1728 & -108 & 432 & -288 & -4608 & -288 & 1152 & -288 & -4608 & -288 & 1152 \\
-1728 & 432 & 6912 & 432 & 432 & -108 & -1728 & -108 & 1152 & -288 & -4608 & -288 & 1152 & -288 & -4608 & -288 \\
-1728 & -1728 & 432 & 6912 & 432 & 432 & -108 & -1728 & 1152 & 1152 & -288 & -4608 & 1152 & 1152 & -288 & -4608 \\
-1728 & -108 & 432 & 432 & 6912 & 432 & -1728 & -1728 & -1728 & -108 & 432 & 432 & -4608 & -288 & 1152 & 1152 \\
-108 & -1728 & -108 & 432 & 432 & 6912 & 432 & -1728 & -108 & -1728 & -108 & 432 & -288 & -4608 & -288 & 1152 \\
432 & -108 & -1728 & -108 & -1728 & 432 & 6912 & 432 & 432 & -108 & -1728 & -108 & 1152 & -288 & -4608 & -288 \\
432 & 432 & -108 & -1728 & -1728 & -1728 & 432 & 6912 & 432 & 432 & -108 & -1728 & 1152 & 1152 & -288 & -4608 \\
-4608 & -288 & 1152 & 1152 & -1728 & -108 & 432 & 432 & 6912 & 432 & -1728 & -1728 & -1728 & -108 & 432 & 432 \\
-288 & -4608 & -288 & 1152 & -108 & -1728 & -108 & 432 & 432 & 6912 & 432 & -1728 & -108 & -1728 & -108 & 432 \\
1152 & -288 & -4608 & -288 & 432 & -108 & -1728 & -108 & -1728 & 432 & 6912 & 432 & 432 & -108 & -1728 & -108 \\
1152 & 1152 & -288 & -4608 & 432 & 432 & -108 & -1728 & -1728 & -1728 & 432 & 6912 & 432 & 432 & -108 & -1728 \\
-4608 & -288 & 1152 & 1152 & -4608 & -288 & 1152 & 1152 & -1728 & -108 & 432 & 432 & 6912 & 432 & -1728 & -1728 \\
-288 & -4608 & -288 & 1152 & -288 & -4608 & -288 & 1152 & -108 & -1728 & -108 & 432 & 432 & 6912 & 432 & -1728 \\
1152 & -288 & -4608 & -288 & 1152 & -288 & -4608 & -288 & 432 & -108 & -1728 & -108 & -1728 & 432 & 6912 & 432 \\
1152 & 1152 & -288 & -4608 & 1152 & 1152 & -288 & -4608 & 432 & 432 & -108 & -1728 & -1728 & -1728 & 432 & 6912
\end{pmatrix}$$

$S = \{1234, 1342, 1432, 2341, 2413, 2431, 3124, 3142, 3214, 4123, 4213, 4321\}, \lambda_{max} = 0.106988, \lambda_{min} = -0.094345$

$$H_S = \frac{1}{6\cdot 5^6} \times \begin{pmatrix}
2304 & 144 & -576 & -576 & -2016 & 1674 & 504 & 504 & -3456 & -216 & 864 & 864 & -3456 & -216 & 864 & 864 \\
144 & 2304 & 144 & -576 & -1926 & -2016 & -126 & 504 & -216 & -3456 & -216 & 864 & -216 & -3456 & -216 & 864 \\
-576 & 144 & 2304 & 144 & 504 & -126 & -2016 & -1926 & 864 & -216 & -3456 & -216 & 864 & -216 & -3456 & -216 \\
-576 & -576 & 144 & 2304 & 504 & 504 & 1674 & -2016 & 864 & 864 & -216 & -3456 & 864 & 864 & -216 & -3456 \\
-2016 & -1926 & 504 & 504 & 2304 & 144 & -576 & -576 & -2016 & -126 & 504 & 504 & -3456 & -216 & 864 & 864 \\
1674 & -2016 & -126 & 504 & 144 & 2304 & 144 & -576 & -126 & -2016 & -126 & 504 & -216 & -3456 & -216 & 864 \\
504 & -126 & -2016 & 1674 & -576 & 144 & 2304 & 144 & 504 & -126 & -2016 & -126 & 864 & -216 & -3456 & -216 \\
504 & 504 & -1926 & -2016 & -576 & -576 & 144 & 2304 & 504 & 504 & -126 & -2016 & 864 & 864 & -216 & -3456 \\
-3456 & -216 & 864 & 864 & -2016 & -126 & 504 & 504 & 2304 & 144 & -576 & -576 & -2016 & -1926 & 504 & 504 \\
-216 & -3456 & -216 & 864 & -126 & -2016 & -126 & 504 & 144 & 2304 & 144 & -576 & 1674 & -2016 & -126 & 504 \\
864 & -216 & -3456 & -216 & 504 & -126 & -2016 & -126 & -576 & 144 & 2304 & 144 & 504 & -126 & -2016 & 1674 \\
864 & 864 & -216 & -3456 & 504 & 504 & -126 & -2016 & -576 & -576 & 144 & 2304 & 504 & 504 & -1926 & -2016 \\
-3456 & -216 & 864 & 864 & -3456 & -216 & 864 & 864 & -2016 & 1674 & 504 & 504 & 2304 & 144 & -576 & -576 \\
-216 & -3456 & -216 & 864 & -216 & -3456 & -216 & 864 & -1926 & -2016 & -126 & 504 & 144 & 2304 & 144 & -576 \\
864 & -216 & -3456 & -216 & 864 & -216 & -3456 & -216 & 504 & -126 & -2016 & -1926 & -576 & 144 & 2304 & 144 \\
864 & 864 & -216 & -3456 & 864 & 864 & -216 & -3456 & 504 & 504 & 1674 & -2016 & -576 & -576 & 144 & 2304
\end{pmatrix}$$

# Appendix 5

$S = \{1234, 2143, 3412, 4321\}$

$$\sum_{\pi \in S} d(\pi, \mu[A]) = \frac{9877}{60000} < \frac{1}{6} \text{ for } A = \begin{pmatrix}
0&0&0&0&1&0&0&0&0&0&0&0&0&0&0&0&0&0&0&0\\
0&0&0&0&0&1&0&0&0&0&0&0&0&0&0&0&0&0&0&0\\
0&0&0&0&0&0&0&0&0&1&0&0&0&0&0&0&0&0&0&0\\
0&0&0&0&0&0&0&0&0&0&0&0&0&1&0&0&0&0&0&0\\
0&0&0&0&0&0&0&0&0&0&0&0&0&0&0&0&0&0&0&1\\
0&0&0&0&0&0&0&0&0&0&0&0&0&0&0&0&0&0&1&0\\
0&0&0&1&0&0&0&0&0&0&0&0&0&0&0&0&0&0&0&0\\
0&0&0&0&0&0&0&0&1&0&0&0&0&0&0&0&0&0&0&0\\
0&0&0&0&0&0&0&0&0&0&0&0&1&0&0&0&0&0&0&0\\
0&0&0&0&0&0&0&0&0&0&0&0&0&0&0&0&0&1&0&0\\
0&0&1&0&0&0&0&0&0&0&0&0&0&0&0&0&0&0&0&0\\
0&0&0&0&0&0&0&1&0&0&0&0&0&0&0&0&0&0&0&0\\
0&0&0&0&0&0&0&0&0&0&0&1&0&0&0&0&0&0&0&0\\
0&0&0&0&0&0&0&0&0&0&0&0&0&0&0&0&1&0&0&0\\
0&1&0&0&0&0&0&0&0&0&0&0&0&0&0&0&0&0&0&0\\
1&0&0&0&0&0&0&0&0&0&0&0&0&0&0&0&0&0&0&0\\
0&0&0&0&0&0&1&0&0&0&0&0&0&0&0&0&0&0&0&0\\
0&0&0&0&0&0&0&0&0&0&1&0&0&0&0&0&0&0&0&0\\
0&0&0&0&0&0&0&0&0&0&0&0&0&0&1&0&0&0&0&0\\
0&0&0&0&0&0&0&0&0&0&0&0&0&0&0&1&0&0&0&0
\end{pmatrix}$$

$S = \{1234, 1243, 1324, 2134, 2143, 2413, 3142, 3412, 3421, 4231, 4312, 4321\}$

$$\sum_{\pi \in S} d(\pi, \mu[A]) = \frac{2027}{4096} < \frac{1}{2} \text{ for } A = \begin{pmatrix}
0.0 & 0.5 & 0.0 & 0.5\\
1.0 & 0.0 & 0.0 & 0.0\\
0.0 & 0.0 & 0.5 & 0.5\\
0.0 & 0.5 & 0.5 & 0.0
\end{pmatrix}$$

$S = \{1234, 1243, 1342, 2134, 2143, 2431, 3124, 3412, 3421, 4213, 4312, 4321\}$

$$\sum_{\pi \in S} d(\pi, \mu[A]) = \frac{388411}{781250} < \frac{1}{2} \text{ for } A = \begin{pmatrix}
0.0 & 0.0 & 1.0 & 0.0 & 0.0\\
0.4 & 0.0 & 0.0 & 0.6 & 0.0\\
0.4 & 0.0 & 0.0 & 0.4 & 0.2\\
0.2 & 0.2 & 0.0 & 0.0 & 0.6\\
0.0 & 0.8 & 0.0 & 0.0 & 0.2
\end{pmatrix}$$

$S = \{1234, 1243, 1342, 2134, 2143, 2431, 3214, 3412, 3421, 4123, 4312, 4321\}$

$$\sum_{\pi \in S} d(\pi, \mu[A]) = \frac{127871}{256000} < \frac{1}{2} \text{ for } A = \begin{pmatrix}
0.0 & 0.4 & 0.0 & 0.0 & 0.0 & 0.6 & 0.0 & 0.0\\
0.0 & 0.0 & 0.6 & 0.0 & 0.0 & 0.0 & 0.4 & 0.0\\
0.4 & 0.0 & 0.0 & 0.4 & 0.0 & 0.0 & 0.0 & 0.2\\
0.2 & 0.2 & 0.0 & 0.0 & 0.2 & 0.0 & 0.0 & 0.4\\
0.0 & 0.4 & 0.0 & 0.0 & 0.0 & 0.2 & 0.2 & 0.2\\
0.4 & 0.0 & 0.0 & 0.0 & 0.4 & 0.2 & 0.0 & 0.0\\
0.0 & 0.0 & 0.0 & 0.6 & 0.4 & 0.0 & 0.0 & 0.0\\
0.0 & 0.0 & 0.4 & 0.0 & 0.0 & 0.0 & 0.4 & 0.2
\end{pmatrix}$$

$S = \{1234, 1243, 1432, 2134, 2341, 2413, 3142, 3214, 3421, 4123, 4312, 4321\}$

$$\sum_{\pi \in S} d(\pi, \mu[A]) = \frac{125}{256} < \frac{1}{2} \text{ for } A = \begin{pmatrix} 0 & 1 & 0 & 0 \\ 1 & 0 & 0 & 0 \\ 0 & 0 & 0 & 1 \\ 0 & 0 & 1 & 0 \end{pmatrix}$$

$S = \{1234, 1243, 1432, 2143, 2314, 2341, 3214, 3412, 3421, 4123, 4132, 4321\}$

$$\sum_{\pi \in S} d(\pi, \mu[A]) = \frac{321}{648} < \frac{1}{2} \text{ for } A = \begin{pmatrix} 0.0 & 0.5 & 0.0 & 0.0 & 0.5 & 0.0 \\ 0.5 & 0.0 & 0.0 & 0.5 & 0.0 & 0.0 \\ 0.0 & 0.0 & 0.5 & 0.0 & 0.0 & 0.5 \\ 0.0 & 0.5 & 0.0 & 0.0 & 0.5 & 0.0 \\ 0.0 & 0.0 & 0.5 & 0.0 & 0.0 & 0.5 \\ 0.5 & 0.0 & 0.0 & 0.5 & 0.0 & 0.0 \end{pmatrix}$$

$S = \{1234, 1342, 1423, 2143, 2314, 2431, 3124, 3241, 3412, 4132, 4213, 4321\}$

$$\sum_{\pi \in S} d(\pi, \mu[A]) = \frac{29}{64} < \frac{1}{2} \text{ for } A = \begin{pmatrix} 0 & 0 & 0 & 1 \\ 0 & 0 & 1 & 0 \\ 1 & 0 & 0 & 0 \\ 0 & 1 & 0 & 0 \end{pmatrix}$$

$S = \{1234, 1342, 1423, 2314, 2413, 2431, 3124, 3142, 3241, 4132, 4213, 4321\}$

$$\sum_{\pi \in S} d(\pi, \mu[A]) = \frac{997}{1024} < \frac{1}{2} \text{ for } A = \begin{pmatrix} 0.0 & 0.5 & 0.0 & 0.5 \\ 0.5 & 0.0 & 0.5 & 0.0 \\ 0.5 & 0.0 & 0.0 & 0.5 \\ 0.0 & 0.5 & 0.5 & 0.0 \end{pmatrix}$$
